# Supplementary material for: Biologically Inspired Dynamic Thresholds for Spiking Neural Networks
Source: arXiv:2206.04426 source file (2023-06-19)
Supplement: Supplementary file 1 [file CC_Ant_experiment_results.tex]

The training and experimental setups are the same as those used for the HalfCheetah-v3 tasks.
% Besides HalfCheetah-v3, we also use the Ant-v3 simulator, another continuous control task, for demonstrating the effectiveeness of the proposed \DTname. 

% \subsection{Experimental Setup}
% The same as the one used for HalfCheetah-v3.

% \subsection{Training Process} 
% The training process of the Ant-v3 tasks are the same as the one for HalfCheetah-v3.

\begin{figure}[ht!]
	\centering
	\includegraphics [scale=0.25]{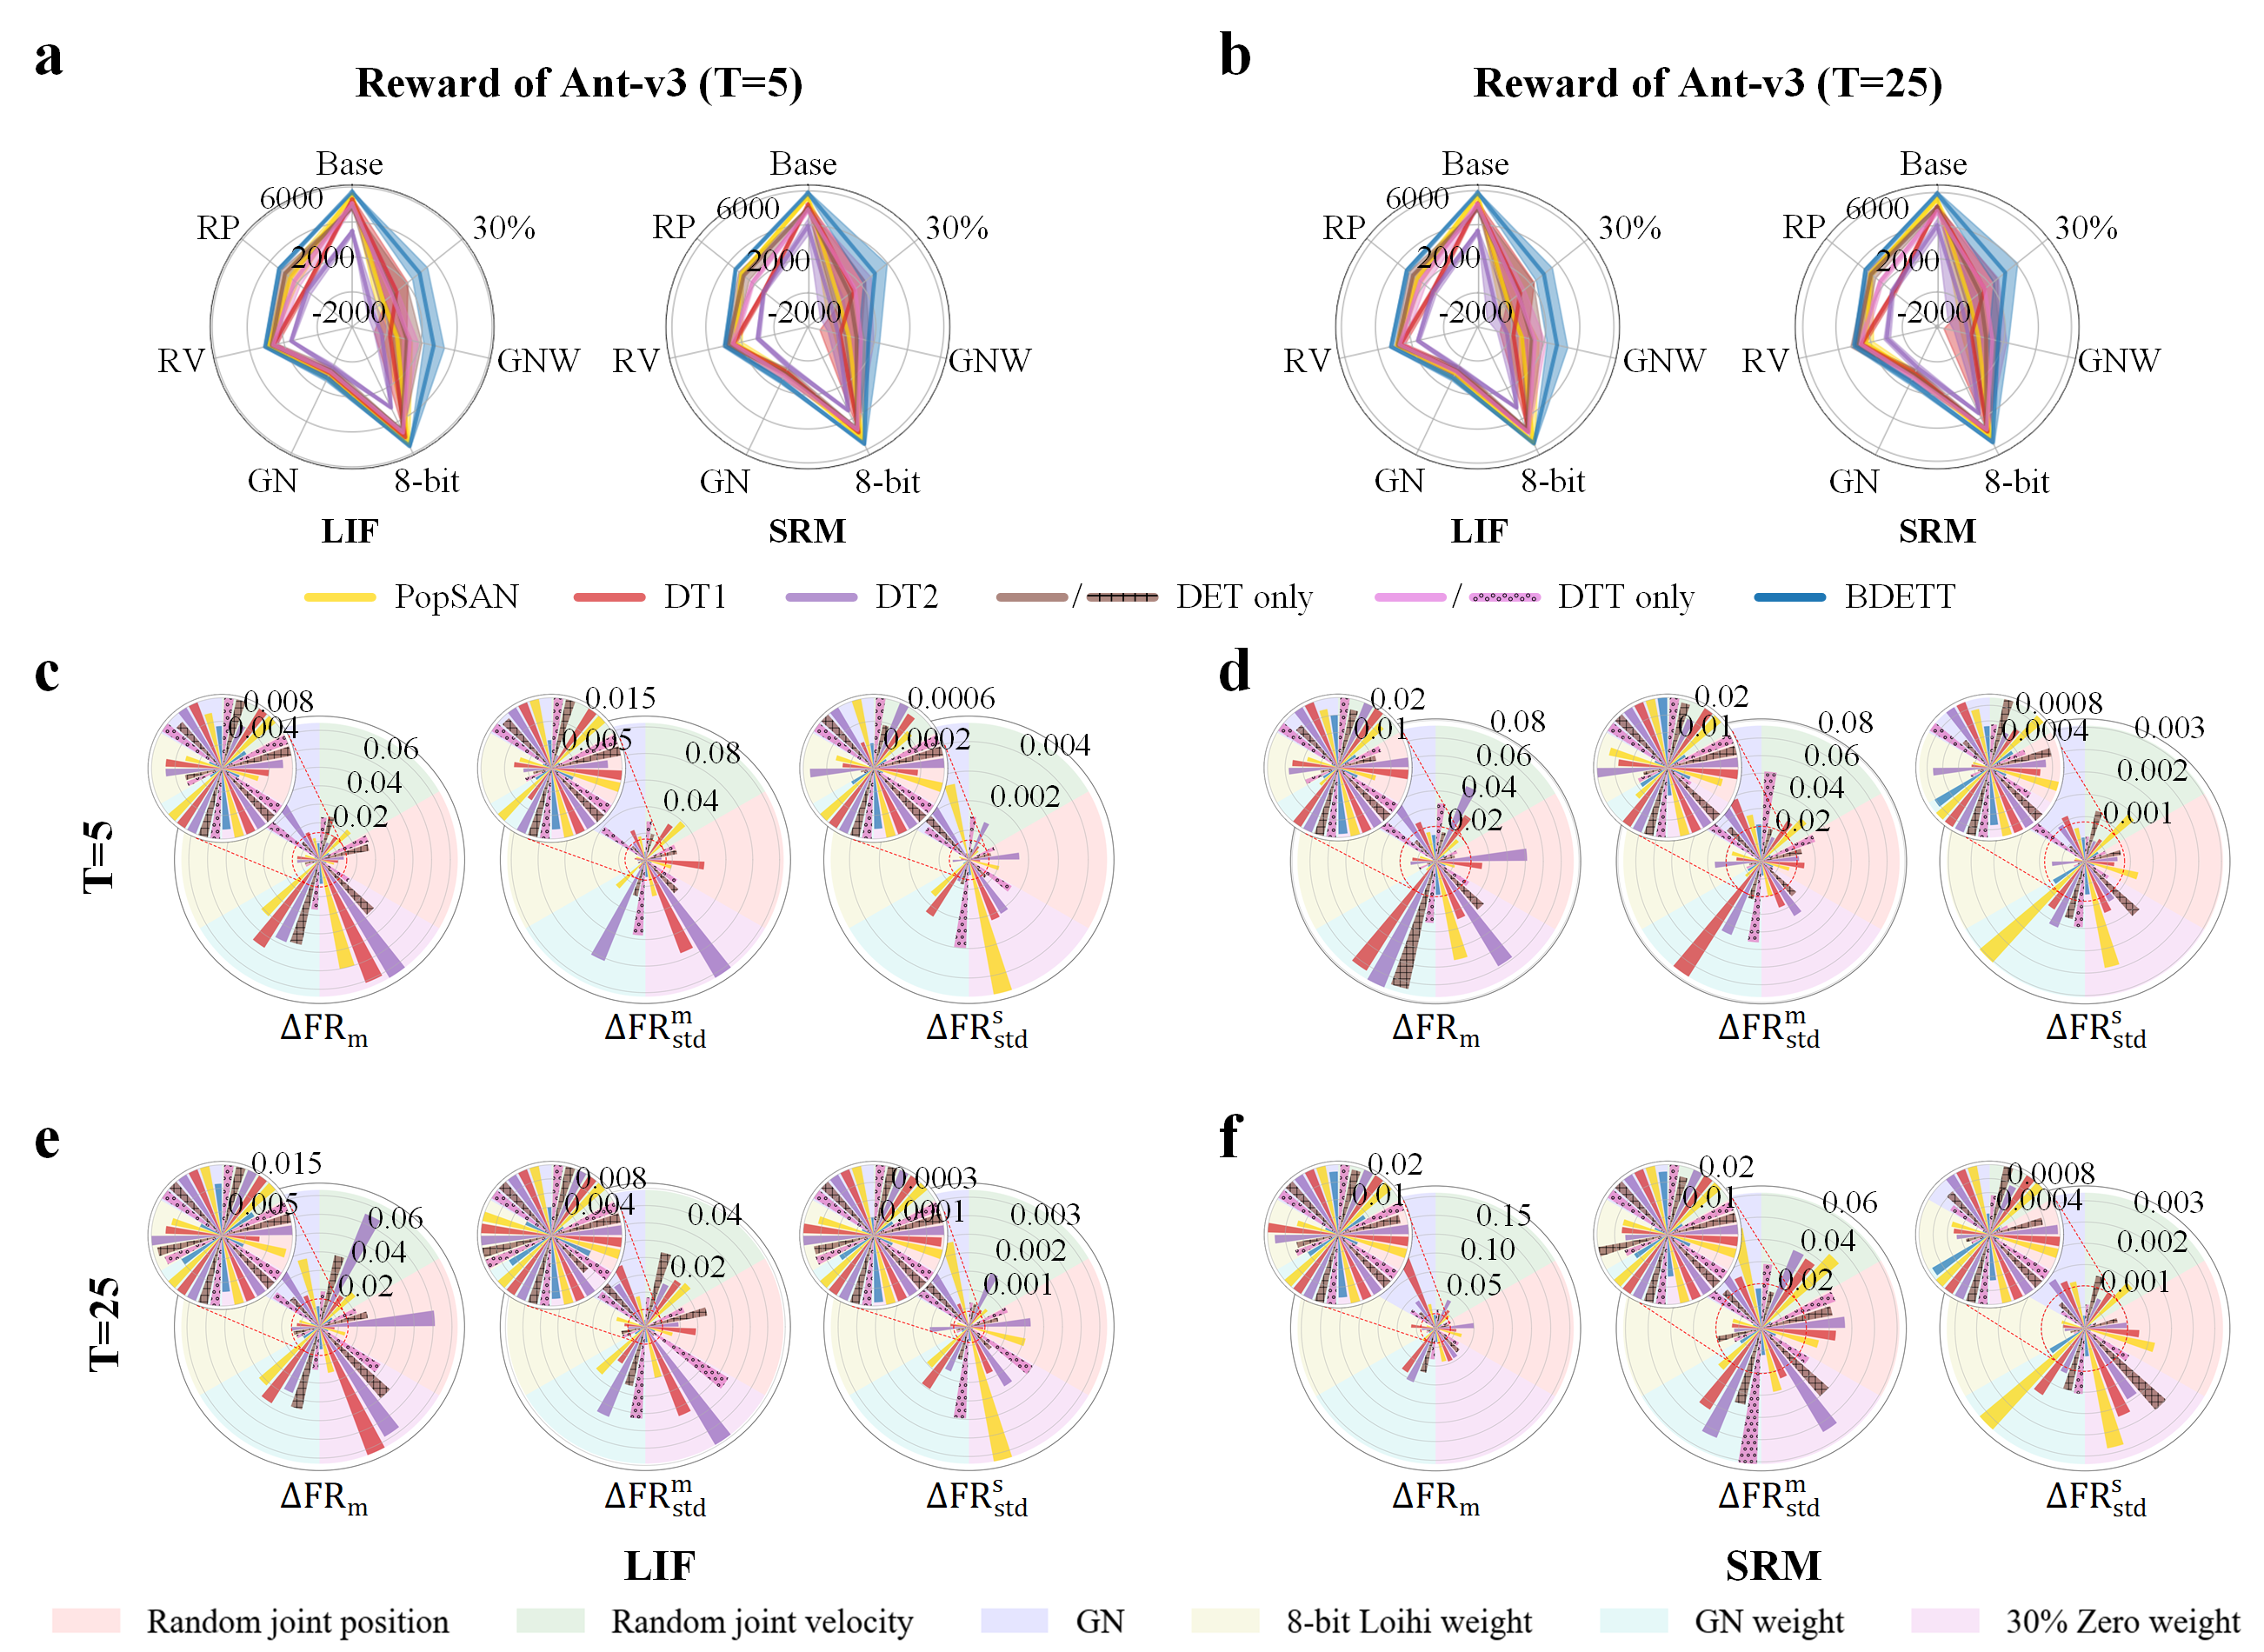}
	\vspace{-0.2cm}
	\caption{
	     The experimental results obtained in the Ant-v3 tasks. a \& b. The rewards obtained under normal and different degraded conditions under the $T=5$ and $T=25$ settings, respectively. `Base' denotes the base condition; `RP' and `RV' represent random joint position and random joint velocity, respectively; `8-bit', `GNW', and `$30\%$' denote the 8-bit Loihi weights, GN weights, and $30\%$ zero weights, respectively. c \& d. Homeostasis measurements obtained under the $T=5$ setting for the LIF- and SRM-based host SNNs, respectively. e \& f. Homeostasis results obtained with the $T=25$ setup for the LIF- and SRM-based host SNNs, respectively.
	}
	\label{fig:SN_Ant_results}
	%\vspace{-0.2cm}
\end{figure}

\subsection*{Assessment---Reward} 
As in the HalfCheetah-v3 tasks, we present the rewards of all competing host SNNs under the original normal conditions with the $T=5$ and $T=25$ settings; see Table~\ref{tab:Degraded environment mujoco Ant}. Compared to HalfCheetah-v3's $17$-dimensional state, the state of an Ant-v3 task has $111$ dimensions. Thus, the rewards obtained from the Ant-v3 experiments are much lower than those obtained in the HalfCheetah-v3 tasks. Nevertheless, the proposed \DTname\ offers the highest rewards in the Ant-v3 tasks, and it improves upon the rewards of the LIF- and SRM-based baseline models by at least $173$ and $236$, respectively. 

\noindent
Relative to the HalfCheetah-v3 tasks, DT1 offers much better rewards in the Ant-v3 tasks under normal conditions. However, the rewards provided by DT1 and DT2 are still lower than those of the baseline PopSAN model. This observation is consistent with those obtained in the obstacle avoidance and HalfCheetah-v3 experiments.

\noindent
We show the quantitative performance of all competing methods under degraded input and weight uncertainty conditions in Tables~\ref{tab:Degraded inputs mujoco Ant} and~\ref{tab:Weight pollution mujoco Ant}, respectively. In Figures~\ref{fig:SN_Ant_results}a and b, we also intuitively present the results. The proposed \DTname\ is still the best performer under all experimental conditions based on the obtained results. A more detailed analysis for each degraded condition is provided in the following.

\noindent
\tb{Degraded Inputs} 
Compared to that of a HalfCheetah-v3 agent, the observation (state) of an Ant-v3 agent $s$ represents a $111$-dimensional data consisting of $13$-dimensional joint position information, $14$-dimensional joint velocity information, and $84$-dimensional contact force data. We disturb Ant-v3's observation in the same three ways introduced in the HalfCheetah-v3 tasks: 
% An action is a $6$-dimensional joint torque, three of them are the torques of the front thigh, shin, and foot, and the rest three are the torques of the back ones. 
``Random joint position", ``Random joint velocity", and ``GN". The average rewards obtained in the ten evaluations conducted under these three different conditions are shown in Table~\ref{tab:Degraded inputs mujoco Ant}. Under all experimental settings, the proposed \DTname\ offers the host SNNs the highest rewards, significantly improving upon the reward of the baseline PopSAN model by at least $213$. 
% More importantly, besides the robustness, the proposed \DTname\ provides the most stable performance, which is highlighted by the smallest STDs under all the DI settings.  

\noindent
\tb{Weight Uncertainty} We leverage the same weight uncertainty conditions as those used in the robot obstacle avoidance and HalfCheetah-v3 experiments. The experimental results are shown in Table~\ref{tab:Weight pollution mujoco Ant}. The proposed \DTname\ remains the best performer under all weight uncertainty conditions. As in the HalfCheetah-v3 experiments, even with low-precision 8-bit weights, the proposed \DTname\ helps both the LIF- and SRM-based host SNNs achieve higher rewards than those offered by the baseline counterparts with high-precision floating-point weights under $T=5$ (\ie 5570 vs. 5526 and 5648 vs. 5643, respectively). With the $T=25$ setup, the SRM-based host SNN exhibits the same pattern.

%%%%%%%%%%%%%%%%%%%%%%%%%%%%%%%%%%% Ant-v3 %%%%%%%%%%%%%%%%%%%%%%%%%%%%%%%

\begin{table}
\vspace{-0.5cm}
\centering
  \caption{Quantitative performance of Mujoco Ant-v3 tasks under standard testing condition.}

  \vspace{0.2cm}
  \label{tab:Degraded environment mujoco Ant}

  \centering
  \small
  \setlength\tabcolsep{2pt}
  \begin{tabular}{lllll}
    \toprule
     
     & \multicolumn{1}{c}{\textbf{LIF} ($T=5$)}     & \multicolumn{1}{c}{\textbf{SRM} ($T=5$)}   & \multicolumn{1}{c}{\textbf{LIF} ($T=25$)}     & \multicolumn{1}{c}{\textbf{SRM} ($T=25$)}             \\
    \cmidrule(r){2-2}
    \cmidrule(r){3-3}
    \cmidrule(r){4-4}
    \cmidrule(r){5-5}
     \textbf{Name}  & \makecell[c]{Reward$\uparrow$}      &  \makecell[c]{Reward$\uparrow$}  & \makecell[c]{Reward$\uparrow$}      &  \makecell[c]{Reward$\uparrow$}    \\
    \hline
    PopSAN  & \makecell[c]{5526 ($\sigma\mbox{-}81$)}      & \makecell[c]{5643 ($\sigma\mbox{-}84$)} & \makecell[c]{5711 ($\sigma\mbox{-}105$)}      & \makecell[c]{5612 ($\sigma\mbox{-}105$)}  \\

    DT1~\cite{hao2020biologically}   & \makecell[c]{5272 ($\sigma\mbox{-}142$)}     &   \makecell[c]{5179 ($\sigma\mbox{-}157$)}  & \makecell[c]{5218 ($\sigma\mbox{-}164$)}     &   \makecell[c]{5121 ($\sigma\mbox{-}117$)} \\
    DT2~\cite{kim2021spiking}  &  \makecell[c]{3454 ($\sigma\mbox{-}183$)}    &  \makecell[c]{3925 ($\sigma\mbox{-}483$)}   &  \makecell[c]{3628 ($\sigma\mbox{-}180$)}    &  \makecell[c]{4016 ($\sigma\mbox{-}445$)}    \\
    % DT3~\cite{sengupta2019going}   & 49.93    & 19.27   & 63.5\%  & 51.35 & 19.23 & 52.5\%  \\
    \hline
    DET only  & \makecell[c]{4836 ($\sigma\mbox{-}82$)}    &  \makecell[c]{4971 ($\sigma\mbox{-}128$)} & \makecell[c]{4957 ($\sigma\mbox{-}113$)}    &  \makecell[c]{5125 ($\sigma\mbox{-}144$)}\\
    DTT only  & \makecell[c]{5041 ($\sigma\mbox{-}294$)}      &   \makecell[c]{4883 ($\sigma\mbox{-}154$)} & \makecell[c]{5192 ($\sigma\mbox{-}267$)}      &   \makecell[c]{4864 ($\sigma\mbox{-}187$)} \\
    \hline
    \DTname\   & \makecell[c]{\textbf{5726 ($\sigma\mbox{-}61$)}}         & \makecell[c]{\textbf{5879 ($\sigma\mbox{-}117$)}} & \makecell[c]{\textbf{5884}} ($\sigma\mbox{-}97$)      & \makecell[c]{\textbf{5942}} ($\sigma\mbox{-}136$)  \\
    \bottomrule
  \end{tabular}
  \vspace{-0.3cm}
\end{table}

\begin{table}
\vspace{-0.3cm}
    \caption{Quantitative performance of Mujoco Ant-v3 tasks under degraded input conditions.}
  \label{tab:Degraded inputs mujoco Ant}
  \centering
    % \scriptsize
  %\fontsize{7pt}{\baselineskip}\selectfont
  \small
  \setlength\tabcolsep{2pt}
  \begin{tabular}{llllll}
    \toprule
     
     & & \multicolumn{1}{c}{\textbf{LIF} ($T=5$)}     & \multicolumn{1}{c}{\textbf{SRM} ($T=5$)} & \multicolumn{1}{c}{\textbf{LIF} ($T=25$)}     & \multicolumn{1}{c}{\textbf{SRM} ($T=25$)} \\
    \cmidrule(r){3-3}
\cmidrule(r){4-4}
\cmidrule(r){5-5}
\cmidrule(r){6-6}
 
      \textbf{Type} & \textbf{Name}  & \makecell[c]{Reward$\uparrow$}        &  \makecell[c]{Reward$\uparrow$}  & \makecell[c]{Reward$\uparrow$}        &  \makecell[c]{Reward$\uparrow$}    \\
    \hline
    \makecell[c]{\multirow{7}{*}{\makecell[c]{Random \\ joint \\ position}}}
    & PopSAN   & \makecell[c]{2503 ($\sigma\mbox{-}503$)}    & \makecell[c]{3004 ($\sigma\mbox{-}131$)}  & \makecell[c]{2544 ($\sigma\mbox{-}337$)}    & \makecell[c]{3036 ($\sigma\mbox{-}152$)}
 \\
    & DT1~\cite{hao2020biologically}   & \makecell[c]{1435 ($\sigma\mbox{-}130$)}     &  \makecell[c]{1333 ($\sigma\mbox{-}122$)}  & \makecell[c]{1380 ($\sigma\mbox{-}158$)}     &  \makecell[c]{1258 ($\sigma\mbox{-}150$)}   \\
    & DT2~\cite{kim2021spiking}  & \makecell[c]{1280 ($\sigma\mbox{-}234$)}   & \makecell[c]{1330 ($\sigma\mbox{-}99$)}   & \makecell[c]{1335 ($\sigma\mbox{-}206$)}   & \makecell[c]{1364 ($\sigma\mbox{-}152$)}
 \\
    \cline{2-6}

    & DET only   & \makecell[c]{2907 ($\sigma\mbox{-}320$)}    & \makecell[c]{2836 ($\sigma\mbox{-}392$)}   & \makecell[c]{2862 ($\sigma\mbox{-}342$)}    & \makecell[c]{2994 ($\sigma\mbox{-}332$)}    \\
    & DTT only & \makecell[c]{2213 ($\sigma\mbox{-}389$)}      & \makecell[c]{2190 ($\sigma\mbox{-}119$)}    & \makecell[c]{2305 ($\sigma\mbox{-}373$)}      & \makecell[c]{2273 ($\sigma\mbox{-}162$)}  \\
    \cline{2-6}

    & \DTname\   & \makecell[c]{\textbf{3339 ($\sigma\mbox{-}111$)}}     & \makecell[c]{\textbf{3450 ($\sigma\mbox{-}75$)}} & \makecell[c]{\textbf{3320 ($\sigma\mbox{-}126$)}}     & \makecell[c]{\textbf{3427}} ($\sigma\mbox{-}115$)
\\

\hline
 \makecell[c]{\multirow{6}{*}{\makecell[c]{Random \\ joint \\ velocity}}}   & PopSAN  & \makecell[c]{2890 ($\sigma\mbox{-}115$)}   & \makecell[c]{2372 ($\sigma\mbox{-}390$)}
& \makecell[c]{2858 ($\sigma\mbox{-}149$)}   & \makecell[c]{2287 ($\sigma\mbox{-}427$)}  \\
&  DT1~\cite{hao2020biologically}         & \makecell[c]{2628 ($\sigma\mbox{-}232$)}       & \makecell[c]{2508 ($\sigma\mbox{-}166$)}      & \makecell[c]{2643 ($\sigma\mbox{-}259$)}       & \makecell[c]{2574 ($\sigma\mbox{-}232$)}  \\

&  DT2~\cite{kim2021spiking}  & \makecell[c]{1579 ($\sigma\mbox{-}89$)}       &  \makecell[c]{1025 ($\sigma\mbox{-}139$)}   & \makecell[c]{1595 ($\sigma\mbox{-}131$)}       &  \makecell[c]{1009 ($\sigma\mbox{-}208$)}  \\
    \cline{2-6}
& DET only  & \makecell[c]{2720 ($\sigma\mbox{-}365$)}      & \makecell[c]{2809 ($\sigma\mbox{-}296$)}   & \makecell[c]{2802 ($\sigma\mbox{-}197$)}      & \makecell[c]{2896 ($\sigma\mbox{-}372$)}   \\

& DTT only  & \makecell[c]{2635 ($\sigma\mbox{-}234$)}       & \makecell[c]{2515 ($\sigma\mbox{-}201$)}  & \makecell[c]{2699 ($\sigma\mbox{-}255$)}       & \makecell[c]{2618 ($\sigma\mbox{-}260$)}    \\
    \cline{2-6}
& \DTname\   & \makecell[c]{\textbf{3103 ($\sigma\mbox{-}95$)}}      & \makecell[c]{\textbf{2984 ($\sigma\mbox{-}176$)}}   & \makecell[c]{\textbf{3217 ($\sigma\mbox{-}119$)}}      & \makecell[c]{\textbf{2996}} ($\sigma\mbox{-}195$)
    \\
\hline
  \makecell[c]{\multirow{6}{*}{GN}} &
    PopSAN & \makecell[c]{977 ($\sigma\mbox{-}320$)}   & \makecell[c]{1031 ($\sigma\mbox{-}212$)}   & \makecell[c]{1022 ($\sigma\mbox{-}358$)}   & \makecell[c]{1059 ($\sigma\mbox{-}217$)}  \\

& DT1~\cite{hao2020biologically}    & \makecell[c]{922 ($\sigma\mbox{-}234$)}      &  \makecell[c]{958 ($\sigma\mbox{-}156$)}   & \makecell[c]{875 ($\sigma\mbox{-}270$)}      &  \makecell[c]{1012 ($\sigma\mbox{-}178$)}  \\

 & DT2~\cite{kim2021spiking}  &   \makecell[c]{560 ($\sigma\mbox{-}179$)}    &   \makecell[c]{583 ($\sigma\mbox{-}158$)}  &   \makecell[c]{664 ($\sigma\mbox{-}163$)}    &   \makecell[c]{623 ($\sigma\mbox{-}235$) }  \\
    \cline{2-6}
& DET only  & \makecell[c]{782 ($\sigma\mbox{-}246$)}     & \makecell[c]{1048 ($\sigma\mbox{-}345$)}    & \makecell[c]{844 ($\sigma\mbox{-}304$)}     & \makecell[c]{1105 ($\sigma\mbox{-}364$)} \\

& DTT only   & \makecell[c]{849 ($\sigma\mbox{-}177$)}      & \makecell[c]{1172 ($\sigma\mbox{-}209$)}  & \makecell[c]{906 ($\sigma\mbox{-}170$)}      & \makecell[c]{1255 ($\sigma\mbox{-}218$)}   \\
    \cline{2-6}
& \DTname\   & \makecell[c]{\textbf{1269 ($\sigma\mbox{-}166$)}}       & \makecell[c]{\textbf{1559 ($\sigma\mbox{-}138$)}}  & \makecell[c]{\textbf{1339 ($\sigma\mbox{-}156$)}}       & \makecell[c]{\textbf{1576}} ($\sigma\mbox{-}161$) \\ 

    \bottomrule
  \end{tabular}
\vspace{-0.3cm}
\end{table}

\begin{table}
\vspace{-0.3cm}
    \caption{Quantitative performance of Mujoco Ant-v3 tasks with weight uncertainty conditions.}
  \label{tab:Weight pollution mujoco Ant}
  \centering
    % \scriptsize
  %\fontsize{7pt}{\baselineskip}\selectfont
  \small
  \setlength\tabcolsep{2pt}
  \begin{tabular}{llllll}
    \toprule
     
     & & \multicolumn{1}{c}{\textbf{LIF} ($T=5$)}     & \multicolumn{1}{c}{\textbf{SRM} ($T=5$)} & \multicolumn{1}{c}{\textbf{LIF} ($T=25$)}     & \multicolumn{1}{c}{\textbf{SRM} ($T=25$)} \\
    \cmidrule(r){3-3}
\cmidrule(r){4-4}
\cmidrule(r){5-5}
\cmidrule(r){6-6}
 
      \textbf{Type} & \textbf{Name}  & \makecell[c]{Reward$\uparrow$}        &  \makecell[c]{Reward$\uparrow$}  & \makecell[c]{Reward$\uparrow$}        &  \makecell[c]{Reward$\uparrow$}    \\
    \hline
    \multirow{6}{*}{\makecell[c]{8-bit \\ Loihi \\ weight}}
    & PopSAN  & \makecell[c]{5347 ($\sigma\mbox{-}175$)}         & \makecell[c]{5285 ($\sigma\mbox{-}158$)}   & \makecell[c]{5504 ($\sigma\mbox{-}210$)}         & \makecell[c]{5228 ($\sigma\mbox{-}139$)}
 \\
    & DT1~\cite{hao2020biologically}   & \makecell[c]{5004 ($\sigma\mbox{-}88$)}     &  \makecell[c]{4889 ($\sigma\mbox{-}163$)}  & \makecell[c]{4826 ($\sigma\mbox{-}102$)}     &  \makecell[c]{4902 ($\sigma\mbox{-}182$)}  \\
    & DT2~\cite{kim2021spiking} & \makecell[c]{3122 ($\sigma\mbox{-}77$)}   & \makecell[c]{3463 ($\sigma\mbox{-}99$)}    & \makecell[c]{3266 ($\sigma\mbox{-}93$)}   & \makecell[c]{3676 ($\sigma\mbox{-}86$)}
 \\
    \cline{2-6}

    & DET only  & \makecell[c]{4561 ($\sigma\mbox{-}135$)}    & \makecell[c]{4634 ($\sigma\mbox{-}111$)}    & \makecell[c]{4663 ($\sigma\mbox{-}156$)}    & \makecell[c]{4727 ($\sigma\mbox{-}153$)}     \\
    & DTT only  & \makecell[c]{4703 ($\sigma\mbox{-}56$)}      & \makecell[c]{4722 ($\sigma\mbox{-}87$)}  & \makecell[c]{4903 ($\sigma\mbox{-}63$)}      & \makecell[c]{4779 ($\sigma\mbox{-}126$)}  \\
    \cline{2-6}

    & \DTname\    &  \makecell[c]{\textbf{5570 ($\sigma\mbox{-}59$)}}      & \makecell[c]{\textbf{5648 ($\sigma\mbox{-}73$)}}  &  \makecell[c]{\textbf{5606 ($\sigma\mbox{-}52$)}}      & \makecell[c]{\textbf{5620}} ($\sigma\mbox{-}143$)
\\

\hline
 \multirow{6}{*}{\makecell[c]{GN \\ weight}}   & PopSAN  & \makecell[c]{637 ($\sigma\mbox{-}860$)}  &  \makecell[c]{467 ($\sigma\mbox{-}951$)}    & \makecell[c]{667 ($\sigma\mbox{-}1002$)}  &  \makecell[c]{444 ($\sigma\mbox{-}1105$)}  
 \\
&  DT1~\cite{hao2020biologically}       & \makecell[c]{221 ($\sigma\mbox{-}949$)}       & \makecell[c]{-57 ($\sigma\mbox{-}1245$)}        & \makecell[c]{155 ($\sigma\mbox{-}839$)}       & \makecell[c]{6 ($\sigma\mbox{-}1722$)}        \\

&  DT2~\cite{kim2021spiking}   & \makecell[c]{-265 ($\sigma\mbox{-}488$)}       &  \makecell[c]{-173 ($\sigma\mbox{-}640$)} & \makecell[c]{-226 ($\sigma\mbox{-}628$)}       &  \makecell[c]{-198 ($\sigma\mbox{-}883$)}
 \\
    \cline{2-6}
& DET only  & \makecell[c]{1208 ($\sigma\mbox{-}855$)}      & \makecell[c]{940 ($\sigma\mbox{-}750$)}   & \makecell[c]{1258 ($\sigma\mbox{-}638$)}      & \makecell[c]{923 ($\sigma\mbox{-}883$)}    \\

& DTT only  & \makecell[c]{1392 ($\sigma\mbox{-}467$)}       & \makecell[c]{1204 ($\sigma\mbox{-}746$)}   & \makecell[c]{1448 ($\sigma\mbox{-}644$)}       & \makecell[c]{1310 ($\sigma\mbox{-}867$)}    \\
    \cline{2-6}
& \DTname\   & \makecell[c]{\textbf{2782 ($\sigma\mbox{-}599$)}}      & \makecell[c]{\textbf{1658 ($\sigma\mbox{-}640$)}}    & \makecell[c]{\textbf{2780 ($\sigma\mbox{-}621$)}}      & \makecell[c]{\textbf{1669}} ($\sigma\mbox{-}612$)  \\
\hline
  \multirow{6}{*}{\makecell[c]{$30\%$ \\ Zero \\ weight }} &
    PopSAN & \makecell[c]{287 ($\sigma\mbox{-}524$)}        & \makecell[c]{372 ($\sigma\mbox{-}994$)}   & \makecell[c]{273 ($\sigma\mbox{-}633$)}        & \makecell[c]{407 ($\sigma\mbox{-}959$)}   \\

& DT1~\cite{hao2020biologically}    & \makecell[c]{1247 ($\sigma\mbox{-}801$)}      &  \makecell[c]{1450 ($\sigma\mbox{-}863$)}   & \makecell[c]{1200 ($\sigma\mbox{-}1020$)}      &  \makecell[c]{1552 ($\sigma\mbox{-}996$)}  \\

 & DT2~\cite{kim2021spiking}   &   \makecell[c]{-548 ($\sigma\mbox{-}354$)}    &   \makecell[c]{-203 ($\sigma\mbox{-}901$)}  &   \makecell[c]{-563 ($\sigma\mbox{-}743$)}    &   \makecell[c]{-183 ($\sigma\mbox{-}1125$)}   \\
    \cline{2-6}
& DET only  & \makecell[c]{1007 ($\sigma\mbox{-}960$)}     & \makecell[c]{1136 ($\sigma\mbox{-}1179$)}   & \makecell[c]{1084 ($\sigma\mbox{-}1092$)}     & \makecell[c]{1186 ($\sigma\mbox{-}1084$)}   \\

& DTT only    & \makecell[c]{908 ($\sigma\mbox{-}428$)}      & \makecell[c]{1559 ($\sigma\mbox{-}1167$)}  & \makecell[c]{1038 ($\sigma\mbox{-}487$)}      & \makecell[c]{1563 ($\sigma\mbox{-}1049$)}  \\
    \cline{2-6}
& \DTname\   &  \makecell[c]{\textbf{2931 ($\sigma\mbox{-}544$)}}       & \makecell[c]{\textbf{3046 ($\sigma\mbox{-}886$)}}  &  \makecell[c]{\textbf{2978 ($\sigma\mbox{-}605$)}}       & \makecell[c]{\textbf{3152}} ($\sigma\mbox{-}924$) \\ 

    \bottomrule
  \end{tabular}
\vspace{-0.3cm}
\end{table}

%%%%%%%%%%%%%%%%%%%%%%% homeostasis %%%%%%%%%%%%%%%%%%%
\begin{table}
  \caption{The raw homeostasis measurements and the corresponding changes with respect to the baseline condition in Mujoco Ant-v3 tasks with the $T=5$ setting.}
%   \caption{Firing rate evaluation test of different methods on different SNN models in successful trials (T=5)}
  \label{SMtab:Ant HOME T5}
  \centering
  \scriptsize
  \setlength\tabcolsep{4pt}
  \begin{tabular}{llllllll}
    \toprule
     
     & & \multicolumn{3}{c}{\textbf{LIF} ($T=5$)}     & \multicolumn{3}{c}{\textbf{SRM} ($T=5$)}                \\
    \cmidrule(r){3-5}
    \cmidrule(r){6-8}
     \textbf{Type} & \textbf{Name}  & \makecell[c]{$\text{FR}_m (\Delta)$}        & \makecell[c]{$\text{FR}_{std}^m (\Delta)$}     & \makecell[c]{$\text{FR}_{std}^s (\Delta)$}         & \makecell[c]{$\text{FR}_m (\Delta)$}        & \makecell[c]{$\text{FR}_{std}^m (\Delta)$}     & \makecell[c]{$\text{FR}_{std}^s (\Delta)$}     \\ 
    \hline
    \multirow{7}{*}{\makecell[c]{baseline \\ condition}}
    & PopSAN  & 0.548 & 0.262 & 0.002169  & 0.197 & 0.150 & 0.001823\\
    & DT1~\cite{hao2020biologically}   & 0.531 & 0.253 & 0.002483 & 0.446 & 0.251 & 0.002172\\
    & DT2~\cite{kim2021spiking}     & 0.770 & 0.223 & 0.004427 & 0.580 & 0.167 & 0.003238\\

    & DET only   & 0.289 & 0.246  & 0.001820 & 0.328 & 0.187 & 0.002027 \\
    & DTT only &  0.547 & 0.280 & 0.001554  & 0.443 & 0.276 & 0.002942  \\
    & \DTname\  &  0.271 & 0.204 & 0.001325  & 0.213  & 0.199 & 0.001535 \\
    \hline
    \multirow{7}{*}{\makecell[c]{Random \\ joint \\ position}}
    & PopSAN  &  0.556 (0.008) &  0.242 (0.020) & 0.003210 (0.001041) & 0.208 (0.011) & 0.134 (0.016) & 0.003022 (0.001199) \\
    & DT1~\cite{hao2020biologically}    &  0.521 (0.010) & 0.209 (0.044) & 0.002859 (0.000376) & 0.420 (0.026) & 0.275 (0.024) & 0.002819 (0.000647) \\
    & DT2~\cite{kim2021spiking}    &  0.757 (0.013) &  0.211 (0.012) & 0.002735 (0.001692) & 0.529 (0.051) & 0.188 (0.021) & 0.002521 (0.000717) \\

    & DET only   &  0.262 (0.027) & 0.270 (0.024) & 0.002575 (0.000755) & 0.339 (0.011) & 0.210 (0.023) & 0.002831 (0.000804) \\
    & DTT only &  0.519 (0.028) & 0.256 (0.024) & 0.002481 (0.000927) & 0.430 (0.013) & 0.244 (0.032) & 0.002454 (0.000488) \\
    & \DTname\  &  0.275 \textbf{(0.004)} & 0.209  \textbf{(0.005)} & 0.001240 \textbf{(0.000085)} & 0.207 \textbf{(0.006)} & 0.192 \textbf{(0.007)} & 0.001308 \textbf{(0.000227)} \\
    \hline
    \multirow{7}{*}{\makecell[c]{Random \\ joint \\ velocity}}
    & PopSAN  &  0.526 (0.022) & 0.223 (0.039) & 0.001743 (0.000426) &  0.180 (0.017) & 0.117 (0.033) & 0.003239 (0.001416) \\
    & DT1~\cite{hao2020biologically}    &  0.516 (0.015) & 0.221 (0.032) & 0.003031 (0.000548) & 0.415 (0.031) & 0.278 (0.027) & 0.002766 (0.000594) \\
    & DT2~\cite{kim2021spiking}    &  0.760 (0.010) & 0.220 (0.003) & 0.003049 (0.001378) & 0.534 (0.046) & 0.182 (0.015) & 0.002749 (0.000489) \\

    & DET only   &  0.265 (0.024) & 0.266 (0.020) & 0.001443 (0.000377) & 0.345 (0.017) & 0.206 (0.019) & 0.003182 (0.001155) \\
    & DTT only &  0.524 (0.023) &  0.251 (0.029) & 0.003020 (0.001466) & 0.410 (0.033) & 0.225 (0.051) & 0.002385 (0.000557) \\
    & \DTname\  &  0.265 \textbf{(0.006)} & 0.206 \textbf{(0.002)} & 0.001452 \textbf{(0.000127)} & 0.207 \textbf{(0.006)} & 0.193 \textbf{(0.006)} & 0.001882 \textbf{(0.000347)} \\
    \hline
    \multirow{7}{*}{\makecell[c]{GN}}
    & PopSAN  &  0.560 (0.012) & 0.244 (0.018) & 0.004782 (0.002613) &  0.180 (0.017) &  0.123 (0.027) &  0.002589 (0.000766) \\
    & DT1~\cite{hao2020biologically}    &  0.515 (0.016) & 0.229 (0.024) & 0.002723 (0.000240) & 0.470 (0.024) & 0.289 (0.038) & 0.003259 (0.001087) \\
    & DT2~\cite{kim2021spiking}    &  0.727 (0.043) & 0.238 (0.015) & 0.002130 (0.002297) & 0.527 (0.053) & 0.204 (0.037) & 0.004192 (0.000954) \\

    & DET only   &  0.302 (0.013) & 0.260 (0.014) & 0.003762 (0.001942) & 0.312 (0.016) & 0.161 (0.026) & 0.002495 \textbf{(0.000468)} \\
    & DTT only &  0.506 (0.041) & 0.241 (0.039) & 0.003306 (0.001752) & 0.390 (0.053) & 0.320 (0.044) & 0.004334 (0.001392) \\
    & \DTname\  &  0.262 \textbf{(0.009)} & 0.198 \textbf{(0.006)} & 0.001539 \textbf{(0.000214)} & 0.198 \textbf{(0.015)} & 0.178 \textbf{(0.021)} &  0.002068 (0.000533) \\
    \hline
    \multirow{7}{*}{\makecell[c]{8-bit \\ Loihi \\ weight}}
    & PopSAN  &  0.540 (0.008) &  0.269 (0.007) &  0.001838 (0.000331) & 0.206 (0.009) & 0.167 (0.017) & 0.001602 (0.000221) \\
    & DT1~\cite{hao2020biologically}    &  0.519 (0.012) & 0.261 (0.008) & 0.002217 (0.000266) & 0.459 (0.013) & 0.237 (0.014) & 0.002406 (0.000234) \\
    & DT2~\cite{kim2021spiking}    &  0.758 (0.012) & 0.217 (0.006) & 0.003884 (0.000543) & 0.566 (0.014) & 0.193 (0.026) & 0.002513 (0.000725) \\

    & DET only   &  0.281 (0.008) & 0.250 (0.004) & 0.001933 (0.000113) & 0.323 (0.005) & 0.194 (0.007) & 0.001869 (0.000158) \\
    & DTT only &  0.539 (0.008) & 0.286 (0.006) & 0.001463 (0.000091) & 0.433 (0.010) & 0.285 (0.009) & 0.003206 (0.000264) \\
    & \DTname\  &  0.274 \textbf{(0.003)} & 0.206 \textbf{(0.002)} &  0.001280 \textbf{(0.000045)} & 0.215 \textbf{(0.002)} & 0.203 \textbf{(0.004)} & 0.001602 \textbf{(0.000067)} \\
    \hline
    \multirow{7}{*}{\makecell[c]{GN \\ weight}}
    & PopSAN  &  0.507 (0.041) &  0.291 (0.029) & 0.003844 (0.001675) & 0.190 (0.007) & 0.138 (0.012) & 0.004859 (0.003036) \\
    & DT1~\cite{hao2020biologically}    &  0.475 (0.056) & 0.261 (0.008) & 0.004749 (0.002266) & 0.519 (0.073) & 0.328 (0.077) & 0.003441 (0.001269) \\
    & DT2~\cite{kim2021spiking}    &  0.722 (0.048) & 0.305 (0.082) & 0.003632 (0.000795) & 0.503 (0.077) & 0.212 (0.045) & 0.004833 (0.001595) \\

    & DET only   & 0.242  (0.047) & 0.218 (0.028) & 0.000966 (0.000854) & 0.402 (0.074) & 0.209 (0.022) & 0.003346 (0.001319) \\
    & DTT only &  0.520 (0.027) & 0.223 (0.057) & 0.004540 (0.002986) & 0.408 (0.035) & 0.322 (0.046) & 0.004416 (0.001474) \\
    & \DTname\  &  0.268 \textbf{(0.003)} & 0.208 \textbf{(0.004)} & 0.001548 \textbf{(0.000223)} & 0.208 \textbf{(0.005)} & 0.190 \textbf{(0.009)} & 0.002351 \textbf{(0.000816)} \\
    \hline
    \multirow{7}{*}{\makecell[c]{30\% \\ Zero \\ weight}}
    & PopSAN  &  0.488 (0.060) & 0.290 (0.028) & 0.006801 (0.004632) & 0.140 (0.057) & 0.130 (0.020) & 0.004246 (0.002423) \\
    & DT1~\cite{hao2020biologically}    &  0.460 (0.071) & 0.328 (0.075) & 0.004668 (0.002185) & 0.411 (0.035) & 0.223 (0.028) & 0.003402 (0.001230) \\
    & DT2~\cite{kim2021spiking}    &  0.696 (0.074) & 0.326 (0.103) & 0.002308 (0.002119) & 0.511 (0.069) & 0.203 (0.036) & 0.004283 (0.001045) \\

    & DET only   &  0.250 (0.039) & 0.279 (0.033) & 0.001023 (0.000797) & 0.364 (0.036) & 0.213 (0.026) & 0.003631 (0.001604) \\
    & DTT only &  0.566 (0.019) & 0.308 (0.028) & 0.003243 (0.001689) & 0.465 (0.022) & 0.268 \textbf{(0.008)} & 0.003563 \textbf{(0.000621)} \\
    & \DTname\  &  0.258 \textbf{(0.013)} & 0.217 \textbf{(0.013)} & 0.001840 \textbf{(0.000515)} & 0.194 \textbf{(0.019)} & 0.191 \textbf{(0.008)} & 0.002276 (0.000741) \\
    
    \bottomrule
  \end{tabular}
\end{table}

\begin{table}
  \caption{The raw homeostasis measurements and the corresponding changes with respect to the baseline condition in Mujoco Ant-v3 tasks with the $T=25$ setup.}
%   \caption{Firing rate evaluation test of different methods on different SNN models in successful trials (T=5)}
  \label{SMtab:Ant HOME T25}
  \centering
  \scriptsize
  \setlength\tabcolsep{4pt}
  \begin{tabular}{llllllll}
    \toprule
     
     & & \multicolumn{3}{c}{\textbf{LIF} $(T=25)$}     & \multicolumn{3}{c}{\textbf{SRM} ($T=25$)}           \\
    \cmidrule(r){3-5}
    \cmidrule(r){6-8}
     \textbf{Type} & \textbf{Name}  & \makecell[c]{$\text{FR}_m (\Delta)$}        & \makecell[c]{$\text{FR}_{std}^m (\Delta)$}     & \makecell[c]{$\text{FR}_{std}^s (\Delta)$}         & \makecell[c]{$\text{FR}_m (\Delta)$}        & \makecell[c]{$\text{FR}_{std}^m (\Delta)$}     & \makecell[c]{$\text{FR}_{std}^s (\Delta)$}     \\ 
    \hline
    \multirow{7}{*}{\makecell[c]{baseline \\ condition}}
    & PopSAN  & 0.535   & 0.258   & 0.002247   & 0.213  & 0.166   & 0.002027  \\
    & DT1~\cite{hao2020biologically}   & 0.530 & 0.252 & 0.002688  & 0.453 & 0.244 & 0.001694 \\
    & DT2~\cite{kim2021spiking}     & 0.753 & 0.230 & 0.004728  & 0.563 & 0.182 & 0.003493\\

    & DET only   & 0.302  & 0.250   & 0.001947  & 0.334  &  0.192  & 0.001872\\
    & DTT only &  0.541  & 0.276   &  0.001526  & 0.451 & 0.281 & 0.002485\\
    & \DTname\  & 0.275  & 0.204    &  0.001503 & 0.222 & 0.195 & 0.001829 \\
    \hline
    \multirow{7}{*}{\makecell[c]{Random \\ joint \\ position}}
    & PopSAN  &   0.549 (0.014) &  0.242 (0.016) &  0.003794 (0.001547) &  0.248 (0.035) &  0.140 (0.026) &  0.003682 (0.001655) \\
    & DT1~\cite{hao2020biologically}    &   0.522 (0.008) &  0.223 (0.029) &  0.003074 (0.000386) &  0.426 (0.027) &  0.277 (0.033) &  0.002951 (0.001257) \\
    & DT2~\cite{kim2021spiking}     &   0.692 (0.061) &  0.211 (0.019) &  0.003076 (0.001652) &  0.513 (0.050) &  0.219 (0.037) &  0.002523 (0.000970) \\

    & DET only   &   0.276 (0.026) &  0.286 (0.036) &  0.002744 (0.000797) &  0.352 (0.018) &  0.224 (0.032) &  0.002642 (0.000770) \\
    & DTT only   &   0.520 (0.021) &  0.252 (0.024) &  0.002636 (0.001110) &  0.430 (0.021) &  0.246 (0.035) &  0.002206 (0.000279) \\
    & \DTname\  &   0.280 \textbf{(0.005)} &  0.210 \textbf{(0.006)} &  0.001386 \textbf{(0.000117)} &  0.216 \textbf{(0.006)} &  0.188 \textbf{(0.007)} &  0.001682 \textbf{(0.000147)} \\
    \hline
    \multirow{7}{*}{\makecell[c]{Random \\ joint \\ velocity}}
    & PopSAN  &   0.510 (0.025) &  0.224 (0.034) &  0.001589 (0.000658) &  0.189 (0.024) &  0.121 (0.045) &  0.003472 (0.001445) \\
    & DT1~\cite{hao2020biologically}    &   0.510 (0.020) &  0.220 (0.032) &  0.003236 (0.000548) &  0.424 (0.029) &  0.281 (0.037) &  0.002692 (0.000998) \\
    & DT2~\cite{kim2021spiking}     &   0.688 (0.065) &  0.203 (0.027) &  0.003163 (0.001565) &  0.522 (0.041) &  0.220 (0.038) &  0.002732 (0.000761) \\

    & DET only   &   0.263 (0.039) &  0.294 (0.044) &  0.002583 (0.000636) &  0.353 (0.019) &  0.209 (0.017) &  0.003135 (0.001263) \\
    & DTT only   &   0.522 (0.019) &  0.259 (0.017) &  0.002184 (0.000658) &  0.426 (0.025) &  0.252 (0.029) &  0.001921 (0.000564) \\
    & \DTname\  &   0.267 \textbf{(0.008)} &  0.206 \textbf{(0.002)} &  0.001632 \textbf{(0.000129)} &  0.213 \textbf{(0.009)} &  0.190 \textbf{(0.005)} &  0.002005 \textbf{(0.000176)} \\
    \hline
    \multirow{7}{*}{\makecell[c]{GN}}
    & PopSAN  &   0.572 (0.037) &  0.240 (0.018) &  0.004581 (0.002334) &  0.180 (0.033) &  0.120 (0.046) &  0.003148 (0.001121) \\
    & DT1~\cite{hao2020biologically}    &   0.512 (0.018) &  0.214 (0.038) &  0.002012 (0.000676) &  0.633 \textbf{(0.018)} &  0.269 (0.025) &  0.002885 (0.001191) \\
    & DT2~\cite{kim2021spiking}     &   0.718 (0.035) &  0.259 (0.029) &  0.002833 (0.001895) &  0.520 (0.043) &  0.232 (0.050) &  0.002148 (0.001345) \\

    & DET only   &   0.323 (0.021) &  0.299 (0.049) &  0.003665 (0.001718) &  0.305 (0.029) &  0.169 (0.023) &  0.002684 (0.000812) \\
    & DTT only   &   0.512 (0.029) &  0.244 (0.032) &  0.003522 (0.001996) &  0.412 (0.039) &  0.328 (0.047) &  0.003144 (0.000659) \\
    & \DTname\  &   0.264 \textbf{(0.011)} &  0.200 \textbf{(0.004)} &  0.001400 \textbf{(0.000103)} &  0.204 \textbf{(0.018)} &  0.177 \textbf{(0.018)} &  0.002129 \textbf{(0.000300)} \\
    \hline
    \multirow{7}{*}{\makecell[c]{8-bit \\ Loihi \\ weight}}
    & PopSAN  &   0.546 (0.011) &  0.275 (0.017) &  0.002569 (0.000322) &  0.225 (0.012) &  0.179 (0.013) &  0.002581 (0.000554) \\
    & DT1~\cite{hao2020biologically}    &   0.542 (0.012) &  0.264 (0.012) &  0.003189 (0.000501) &  0.421 (0.032) &  0.257 (0.013) &  0.001184 (0.000510) \\
    & DT2~\cite{kim2021spiking}     &   0.738 (0.015) &  0.220 (0.010) &  0.003680 (0.001048) &  0.545 (0.018) &  0.194 (0.012) &  0.003026 (0.000467) \\

    & DET only   &   0.316 (0.014) &  0.236 (0.014) &  0.002292 (0.000345) &  0.346 (0.012) &  0.212 (0.020) &  0.002214 (0.000342) \\
    & DTT only   &   0.554 (0.013) &  0.290 (0.014) &  0.001174 (0.000352) &  0.438 (0.013) &  0.294 (0.013) &  0.002763 (0.000278) \\
    & \DTname\  &   0.270 \textbf{(0.005)} &  0.200 \textbf{(0.004)} &  0.001576 \textbf{(0.000073)} &  0.218 \textbf{(0.004)} &  0.199 \textbf{(0.004)} &  0.001722 \textbf{(0.000107)} \\
    \hline
    \multirow{7}{*}{\makecell[c]{GN \\ weight}}
    & PopSAN  &   0.493 (0.042) &  0.295 (0.037) &  0.003726 (0.001479) &  0.190 (0.023) &  0.141 (0.025) &  0.005216 (0.003189) \\
    & DT1~\cite{hao2020biologically}    &  0.482 (0.048) &  0.277 (0.025) &  0.004663 (0.001975) &  0.522 (0.069) &  0.287 (0.043) &  0.003540 (0.001846) \\
    & DT2~\cite{kim2021spiking}     &   0.715 (0.038) &  0.286 (0.056) &  0.003431 (0.001297) &  0.486 (0.077) &  0.235 (0.053) &  0.004632 (0.001139) \\

    & DET only   &   0.257 (0.045) &  0.215 (0.035) &  0.001036 (0.000911) &  0.394 (0.060) &  0.227 (0.035) &  0.003373 (0.001501) \\
    & DTT only   &   0.518 (0.023) &  0.223 (0.053) &  0.003998 (0.002472) &  0.410 (0.041) &  0.342 (0.061) &  0.004025 (0.001540) \\
    & \DTname\  &   0.265 \textbf{(0.010)} &  0.211 \textbf{(0.007)} &  0.001729 \textbf{(0.000226)} &  0.212 \textbf{(0.010)} &  0.206 \textbf{(0.011)} &  0.002773 \textbf{(0.000944)} \\
    \hline
    \multirow{7}{*}{\makecell[c]{30\% \\ Zero \\ weight}}
    & PopSAN  &   0.510 (0.025) &  0.288 (0.030) &  0.005942 (0.003695) &  0.168 (0.045) &  0.137 (0.029) &  0.004893 (0.002866) \\
    & DT1~\cite{hao2020biologically}    &   0.457 (0.073) &  0.307 (0.055) &  0.004043 (0.001355) &  0.406 (0.047) &  0.220 (0.024) &  0.003909 (0.002215) \\
    & DT2~\cite{kim2021spiking}     &   0.685 (0.068) &  0.309 (0.079) &  0.002863 (0.001865) &  0.517 (0.046) &  0.236 (0.054) &  0.005426 (0.001933) \\

    & DET only   &   0.252 (0.050) &  0.243 \textbf{(0.007)} &  0.001132 (0.000815) &  0.376 (0.042) &  0.232 (0.040) &  0.004387 (0.002515) \\
    & DTT only   &   0.579 (0.038) &  0.332 (0.056) &  0.003538 (0.002012) &  0.487 (0.036) &  0.256 (0.025) &  0.003692 (0.001207) \\
    & \DTname\  &   0.263 \textbf{(0.012)} &  0.213 (0.009) &  0.001883 \textbf{(0.000380)} &  0.204 \textbf{(0.018)} &  0.183 \textbf{(0.012)} &  0.002485 \textbf{(0.000656)} \\
    
    \bottomrule
  \end{tabular}
\end{table}

% \begin{figure}[ht!]
% 	\centering
% 	\includegraphics [scale=0.15]{figures/Ant_homeostasis.png}
% 	\vspace{-0.3cm}
% 	\caption{
% 		\bd{The changes of quantified homeostasis with respect to the base condition in Mujoco Ant-v3.}
% % 		Firing rate evaluation test of different methods on different SNN models in success trails.
% 	}
% 	\label{fig:ant_h_changes}
% 	\vspace{-0.5cm}
% \end{figure}

\subsection*{Assessment---Homeostatic} The raw homeostasis measurements obtained with both T=5 and T=25 are provided in Tables~\ref{SMtab:Ant HOME T5} and~\ref{SMtab:Ant HOME T25}, respectively. The corresponding homeostasis plots are shown in Figures~\ref{fig:SN_Ant_results}c-f.

\noindent
The homeostasis results obtained in the Ant-v3 tasks demonstrate the effectiveness of the proposed \DTname\ in terms of regulating the neuronal firing rates of the host SNNs, inducing minimal changes in all three metrics when transferring from the base conditions to all other experimental settings. We witness that the strongest homeostasis again provides the highest rewards.

\subsection*{Assessment---Ablation Studies}
The experimental results obtained in the Ant-v3 task ablation studies under different conditions are reported in the rows named `DET only' and `DTT only' in Tables~\ref{tab:Degraded environment mujoco Ant}, ~\ref{tab:Degraded inputs mujoco Ant}, and ~\ref{tab:Weight pollution mujoco Ant}. All listed evaluations validate that the \DTname\ scheme performs better than any single component. As shown in Table~\ref{tab:Weight pollution mujoco Ant}, under the ``GN weight" condition, both `DET only' and `DTT only' offer both the LIF- and SRM-based host SNNs higher rewards than the other competing dynamic threshold schemes. As in the other tasks, the dynamic threshold scheme with only one component cannot effectively regulate the firing rate statuses of the host SNNs, prohibiting meaningful homeostasis. When combining the DTT and DET components, we witness much more stable homeostasis for all host SNNs.
