# Supplementary material for: Biologically Inspired Dynamic Thresholds for Spiking Neural Networks
Source: arXiv:2206.04426 source file (2023-06-19)
Supplement: Supplementary file 2 [file CC_HC_experiment_results.tex]

\subsection*{Training} 
The adopted population-coded SAN (PopSAN) and its modified variants are trained by using the twin-delayed deep deterministic policy gradient (TD3) off-policy algorithm~\cite{fujimoto2018addressing} and the following hyperparameter settings: $D=0.75$ for the LIF; $\eta=0.01$ and $\psi=6.0$ for the DET; $C=3.0$ for the DTT; and $\tau_s=\tau_r=1.0$ for the SRM. Compared to the settings of the obstacle avoidance tasks, the only different setting is the value of $\psi$ for the DET. Following the training protocol of the PopSAN, we set the batch size to $100$ and the learning rates to $0.0001$ for both the actor and critic networks. The reward discount factor is set to $0.99$, and the maximum length of the replay buffer is set to $1$ million. We use PyTorch~\cite{paszke2019pytorch} to train all competing SNNs with an i7-7700 CPU and an NVIDIA GTX 1080Ti GPU.

\begin{figure}[ht!]
	\centering
	\includegraphics [scale=0.25]{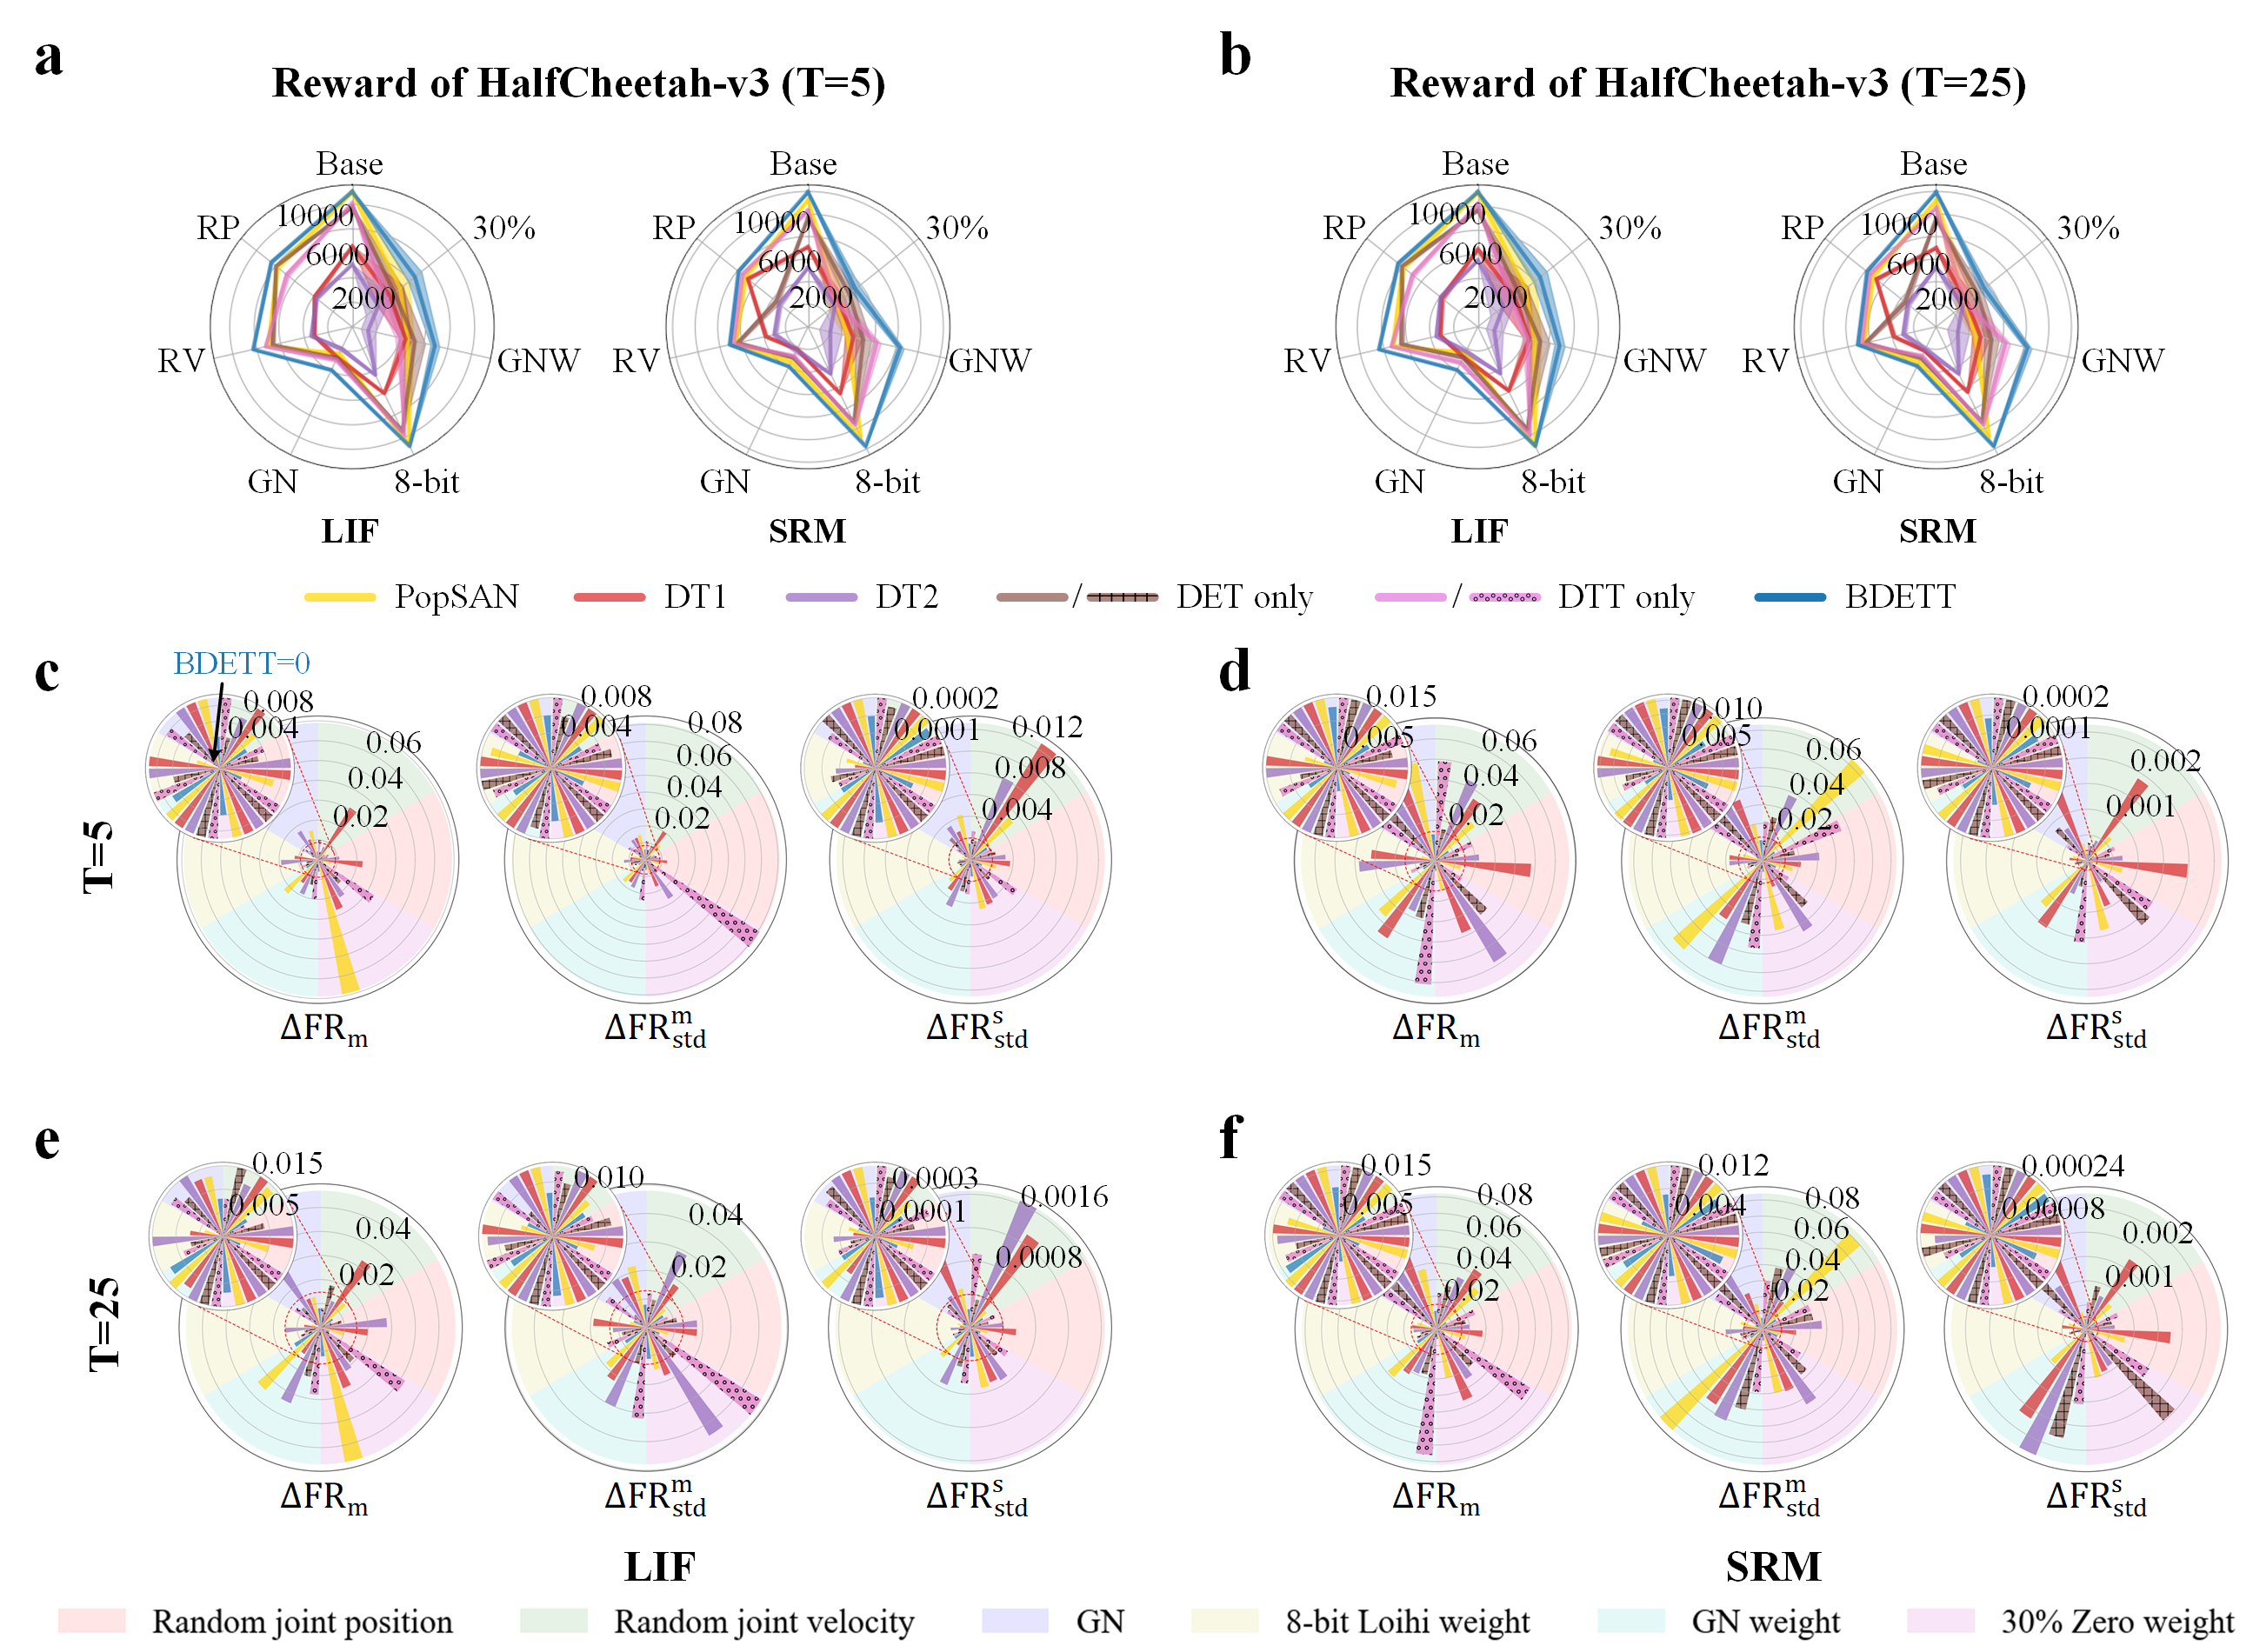}
	\vspace{-0.2cm}
	\caption{
	    The experimental results obtained in the HalfCheetah-v3 tasks. a \& b. The rewards obtained under normal and different degraded conditions with $T=5$ and $T=25$ settings, respectively. `Base' indicates the base condition; `RP' indicates random joint position; `RV' denotes random joint velocity; `8-bit', `GNW', and `$30\%$' denote the 8-bit Loihi weights, GN weights, and $30\%$ zero weights, respectively. c \& d. Homeostasis measurements obtained with the $T=5$ setting for the LIF- and SRM-based host SNNs, respectively. e \& f. Homeostasis results obtained with the $T=25$ setup for the LIF- and SRM-based host SNNs, respectively.
	}
	\label{fig:SN_HC_results}
	%\vspace{-0.2cm}
\end{figure}

\subsection*{Assessment---Reward}
After determining the evaluation settings of the PopSAN~\cite{tang2020deep}, we train ten models corresponding to ten random seeds, and the best-performing model is used for our assessments under different degraded conditions. In particular, the best-performing model is evaluated ten times under each experimental condition, and the mean reward of the ten evaluations represents the model's performance. Each evaluation consists of ten episodes, and each episode lasts for a maximum of $1000$ execution steps. Table~\ref{tab:Degraded environment mujoco HC} shows the ten evaluations' average rewards and the corresponding standard deviations of all competing SNNs under a normal testing condition. Here, we also present the quantitative performance achieved under the $T=5$ and $T=25$ settings. With both the LIF and SRM models, the proposed \DTname\ offers the host SNNs the best rewards in all experimental settings under normal testing conditions (\ie the base conditions). 

\noindent
Unlike in the obstacle avoidance tasks, even with grid searches, the rewards offered by DT1 and DT2 are significantly lower than those provided by the baseline PopSAN model. This indicates that dynamic threshold schemes may perform worse than a simple static threshold, especially for heuristic-based schemes. More importantly, we observe similar patterns in the obstacle avoidance tasks; the SRs offered by DT1 and DT2 are lower than those of the baseline SAN-NR model in most experimental conditions. 

\noindent
Tables~\ref{tab:Degraded inputs mujoco HC} and~\ref{tab:Weight pollution mujoco HC} show the quantitative performance of all competing approaches under degraded input and weight uncertainty conditions, respectively. The results are also illustrated in Figures~\ref{fig:SN_HC_results}a and b for the $T=5$ and $T=25$ settings, respectively. We provide a more detailed analysis for each degraded condition in the following.

% \begin{figure}[h]
% 	\centering

% 	\includegraphics [scale=0.6]{figures/CC_DC}
% 	\vspace{-0.2cm}
% 	\caption{
% 	    \tb{Illustrations of continuous control task and the specially designed degraded conditions.}
% 		(a) The control loop of the agents (\ie halfcheetah and ant). For each step, the current state is converted to spike trains by an encoder as input to the host SNN, and output spike trains are converted to control signals by a decoder. (b) The three specially designed degraded inputs, where the red color symbols indicate the disturbed ones. Note that we only demonstrate one random leg's random selection from each agent, respectively. (c) The three specially designed weight uncertainty conditions.
% 	}
% 	\label{fig:OA_degraded}
% 	%\vspace{-0.2cm}
% \end{figure}

\noindent
\tb{Degraded Inputs} 
In the HalfCheetah-v3 continuous control task, an observation (state) $s$ represents $17$-dimensional data consisting of $8$-dimensional joint position information and $9$-dimensional joint velocity information. 
% An action is a $6$-dimensional joint torque, three of them are the torques of the front thigh, shin, and foot, and the rest three are the torques of the back ones. 
Similar to the degraded input experiments conducted in the robot obstacle avoidance tasks, we disturb a HalfCheetah-v3's observations in three different ways. a) ``Random joint position": for each episode, one of the eight joint positions is randomly selected, and its original position is replaced by a random number sampled from a Gaussian distribution $\mathcal N(0,0.1)$. b) ``Random joint velocity": we randomly select one of the nine joint velocities in each episode and change its observed velocity to a random number sampled from a Gaussian distribution $\mathcal N(0,10.0)$. c) ``GN": For each episode, we add Gaussian noise (\ie $s_{input} + \mathcal N(0,1.0)$, as suggested in a study regarding LSTM-LMC~\cite{choi2019deep}) to each of the $17$ joint states. The average rewards obtained from the ten evaluations conducted under these three different conditions are shown in Table~\ref{tab:Degraded inputs mujoco HC}. 

\noindent
Under all experimental settings, the proposed \DTname\ offers the host SNNs the highest rewards, significantly improving upon the rewards of the baseline PopSAN model by at least $438$ with $T=5$, and $358$ with $T=25$. Compared to the other two degraded input conditions, the ``GN" condition disturbs all dimensions of the HalfCheetah-v3 state. Therefore, we observe that the lowest rewards obtained by all host SNNs occur with the ``GN" setting. Even though the DT1 method hosted by an LIF-based SNN reduces the rewards of the baseline PopSAN model by almost half, it outperforms the baseline model with both $T$ settings under the ``GN" condition. Furthermore, the proposed \DTname\ provides the most stable performance, highlighted by it obtaining the smallest standard deviations under all the degraded input settings.  

\noindent
\tb{Weight Uncertainty} We leverage the same weight uncertainty conditions as those introduced in robot obstacle avoidance experiments to demonstrate the effectiveness of all competing dynamic threshold schemes, and the corresponding results are shown in Table~\ref{tab:Weight pollution mujoco HC}. The proposed \DTname\ remains the best performer under the weight uncertainty conditions. Note that the SRM-based \DTname\ outperforms other methods by significant margins under the ``GN weight" settings, highlighting that the proposed dynamic threshold scheme can effectively deal with weight uncertainty errors. We also notice that the DT2 scheme produces the lowest rewards under all experimental weight uncertainty settings, indicating that predefining a target firing rate does not work well with weight uncertainty conditions. Surprisingly, even with low-precision 8-bit weights, the proposed \DTname\ helps the SRM-based host SNN achieve higher rewards than those obtained with high-precision weights under the $T=5$ and $T=25$ settings ($11767$ vs. $11268$ with $T=5$ and $11760$ vs. $11247$ with $T=25$).

\begin{table}
\vspace{-0.5cm}
\centering
  \caption{Quantitative Performance of Mujoco HalfCheetah-v3 Tasks under standard testing condition.}

  \vspace{0.2cm}
  \label{tab:Degraded environment mujoco HC}

  \centering
  \small
  \setlength\tabcolsep{2pt}
  \begin{tabular}{lllll}
    \toprule
     
     & \multicolumn{1}{c}{\textbf{LIF} ($T=5$)}     & \multicolumn{1}{c}{\textbf{SRM} ($T=5$)}    & \multicolumn{1}{c}{\textbf{LIF} ($T=25$)}     & \multicolumn{1}{c}{\textbf{SRM} ($T=25$)}             \\
    \cmidrule(r){2-3}
    \cmidrule(r){4-5}
     \textbf{Name}  & \makecell[c]{Reward$\uparrow$}      &  \makecell[c]{Reward$\uparrow$}    & \makecell[c]{Reward$\uparrow$}      &  \makecell[c]{Reward$\uparrow$}   \\
    \hline
    PopSAN  & \makecell[c]{10989 ($\sigma\mbox{-}49$)}      & \makecell[c]{11268 ($\sigma\mbox{-}149$)}                           & \makecell[c]{11137 ($\sigma\mbox{-}70$)}  & \makecell[c]{11247 ($\sigma\mbox{-}132$)}                  \\
    DT1~\cite{hao2020biologically}   & \makecell[c]{6572 ($\sigma\mbox{-}85$)}     &   \makecell[c]{7085 ($\sigma\mbox{-}69$)}    & \makecell[c]{6438 ($\sigma\mbox{-}102$)}  & \makecell[c]{7001 ($\sigma\mbox{-}82$)}                    \\
    DT2~\cite{kim2021spiking}  &  \makecell[c]{5110 ($\sigma\mbox{-}30$)}    &  \makecell[c]{5262 ($\sigma\mbox{-}77$)}           & \makecell[c]{5523 ($\sigma\mbox{-}67$)}   & \makecell[c]{5311 ($\sigma\mbox{-}113$)}                   \\
    % DT3~\cite{sengupta2019going}   & 49.93    & 19.27   & 63.5\%  & 51.35 & 19.23 & 52.5\%                                      & 49.93    & 19.27   & 63.5\%  & 51.35 & 19.23 & 52.5\%                                                  \\
    \hline                                                                                                                         
    DET only  & \makecell[c]{9794 ($\sigma\mbox{-}107$)}    &  \makecell[c]{9694 ($\sigma\mbox{-}112$)}                           & \makecell[c]{9704 ($\sigma\mbox{-}125$)}  & \makecell[c]{9619 ($\sigma\mbox{-}105$)}                   \\
    DTT only  & \makecell[c]{10104 ($\sigma\mbox{-}44$)}      &   \makecell[c]{10332 ($\sigma\mbox{-}106$)}                       & \makecell[c]{10221 ($\sigma\mbox{-}57$)}  & \makecell[c]{10563 ($\sigma\mbox{-}83$)}                   \\
    \hline                                                                                                                         
    \DTname\   & \makecell[c]{\textbf{11064 ($\sigma\mbox{-}28$)}}         & \makecell[c]{\textbf{11960 ($\sigma\mbox{-}86$)}}    & \makecell[c]{\textbf{11209 ($\sigma\mbox{-}56$)}} & \makecell[c]{\textbf{11956 ($\sigma\mbox{-}95$)}}  \\
    \bottomrule
  \end{tabular}
  \vspace{-0.3cm}
\end{table}

\begin{table}
\vspace{-0.3cm}
    \caption{Quantitative performance of Mujoco HalfCheetah-v3 tasks under degraded input conditions.}
  \label{tab:Degraded inputs mujoco HC}
  \centering
    % \scriptsize
%   \fontsize{7pt}{\baselineskip}\selectfont
  \small
  \setlength\tabcolsep{2pt}
  \begin{tabular}{llllll}
    \toprule
     
     & & \multicolumn{1}{c}{\textbf{LIF} ($T=5$)}     & \multicolumn{1}{c}{\textbf{SRM} ($T=5$)} & \multicolumn{1}{c}{\textbf{LIF} ($T=25$)}     & \multicolumn{1}{c}{\textbf{SRM} ($T=25$)} \\
    \cmidrule(r){3-3}
\cmidrule(r){4-4}
\cmidrule(r){5-5}
\cmidrule(r){6-6}
 
      \textbf{Type} & \textbf{Name}  & \makecell[c]{Reward$\uparrow$}        &  \makecell[c]{Reward$\uparrow$}  & \makecell[c]{Reward$\uparrow$}        &  \makecell[c]{Reward$\uparrow$}    \\
    \hline
    \makecell[c]{\multirow{7}{*}{\makecell[c]{Random \\ joint \\ position}}}
    & PopSAN  & \makecell[c]{7832 ($\sigma\mbox{-}222$)}    & \makecell[c]{7120 ($\sigma\mbox{-}214$)}   & \makecell[c]{7947 ($\sigma\mbox{-}253$)}    & \makecell[c]{7167 ($\sigma\mbox{-}197$)}
 \\
    & DT1~\cite{hao2020biologically}   & \makecell[c]{3923 ($\sigma\mbox{-}204$)}     &  \makecell[c]{6830 ($\sigma\mbox{-}140$)}    & \makecell[c]{3835 ($\sigma\mbox{-}248$)}     &  \makecell[c]{6792 ($\sigma\mbox{-}157$)}  \\
    & DT2~\cite{kim2021spiking} & \makecell[c]{3750 ($\sigma\mbox{-}171$)}   & \makecell[c]{3230 ($\sigma\mbox{-}239$)}   & \makecell[c]{3950 ($\sigma\mbox{-}192$)}   & \makecell[c]{3213 ($\sigma\mbox{-}230$)}
 \\
    \cline{2-6}

    & DET only  & \makecell[c]{7954 ($\sigma\mbox{-}103$)}    & \makecell[c]{3582 ($\sigma\mbox{-}284$)}   & \makecell[c]{8051 ($\sigma\mbox{-}148$)}    & \makecell[c]{3502 ($\sigma\mbox{-}323$)}     \\
    & DTT only  & \makecell[c]{6817 ($\sigma\mbox{-}221$)}      & \makecell[c]{7428 ($\sigma\mbox{-}234$)}  & \makecell[c]{6922 ($\sigma\mbox{-}202$)}      & \makecell[c]{7493 ($\sigma\mbox{-}182$)}  \\
    \cline{2-6}

    & \DTname\   & \makecell[c]{\textbf{8465 ($\sigma\mbox{-}121$)}}     & \makecell[c]{\textbf{7883 ($\sigma\mbox{-}78$)}}   & \makecell[c]{\textbf{8463 ($\sigma\mbox{-}130$)}}     & \makecell[c]{\textbf{7846 ($\sigma\mbox{-}70$)}}
\\

\hline
 \makecell[c]{\multirow{6}{*}{\makecell[c]{Random \\ joint \\ velocity}}}   & PopSAN  & \makecell[c]{7020 ($\sigma\mbox{-}146$)}   & \makecell[c]{6576 ($\sigma\mbox{-}147$)} 
& \makecell[c]{7223 ($\sigma\mbox{-}165$)}   & \makecell[c]{6583 ($\sigma\mbox{-}168$)}
 \\
&  DT1~\cite{hao2020biologically}     & \makecell[c]{3187 ($\sigma\mbox{-}142$)}       & \makecell[c]{3836 ($\sigma\mbox{-}181$)}   & \makecell[c]{3203 ($\sigma\mbox{-}148$)}       & \makecell[c]{3855 ($\sigma\mbox{-}202$)}      \\

&  DT2~\cite{kim2021spiking}  & \makecell[c]{3395 ($\sigma\mbox{-}209$)}       &  \makecell[c]{3031 ($\sigma\mbox{-}239$)}  & \makecell[c]{3506 ($\sigma\mbox{-}208$)}       &  \makecell[c]{2965 ($\sigma\mbox{-}241$)} 
\\
    \cline{2-6}
& DET only  & \makecell[c]{6664 ($\sigma\mbox{-}179$)}      & \makecell[c]{6392 ($\sigma\mbox{-}206$)}   & \makecell[c]{6498 ($\sigma\mbox{-}219$)}      & \makecell[c]{6435 ($\sigma\mbox{-}213$)}    \\

& DTT only  & \makecell[c]{7249 ($\sigma\mbox{-}137$)}       & \makecell[c]{6772 ($\sigma\mbox{-}299$)}   & \makecell[c]{7363 ($\sigma\mbox{-}150$)}       & \makecell[c]{6762 ($\sigma\mbox{-}247$)}   \\
    \cline{2-6}
& \DTname\   & \makecell[c]{\textbf{8302 ($\sigma\mbox{-}84$)}}      & \makecell[c]{\textbf{7116 ($\sigma\mbox{-}146$)}}  & \makecell[c]{\textbf{8422 ($\sigma\mbox{-}94$)}}      & \makecell[c]{\textbf{7127 ($\sigma\mbox{-}131$)}} 
 \\
\hline
   \makecell[c]{\multirow{6}{*}{GN}} &
    PopSAN & \makecell[c]{2440 ($\sigma\mbox{-}199$)}   & \makecell[c]{3457 ($\sigma\mbox{-}187$)}  & \makecell[c]{2393 ($\sigma\mbox{-}214$)}   & \makecell[c]{3494 ($\sigma\mbox{-}187$)}   \\

& DT1~\cite{hao2020biologically}    & \makecell[c]{2790 ($\sigma\mbox{-}187$)}      &  \makecell[c]{2210 ($\sigma\mbox{-}124$)}  & \makecell[c]{2773 ($\sigma\mbox{-}198$)}      &  \makecell[c]{2355 ($\sigma\mbox{-}120$)} \\

 & DT2~\cite{kim2021spiking}  &   \makecell[c]{1994 ($\sigma\mbox{-}175$)}    &   \makecell[c]{2307 ($\sigma\mbox{-}272$)}    &   \makecell[c]{2281 ($\sigma\mbox{-}223$)}    &   \makecell[c]{2210 ($\sigma\mbox{-}251$)}  \\
    \cline{2-6}
& DET only  & \makecell[c]{2831 ($\sigma\mbox{-}157$)}     & \makecell[c]{3013 ($\sigma\mbox{-}130$)}  & \makecell[c]{2807 ($\sigma\mbox{-}163$)}     & \makecell[c]{3061 ($\sigma\mbox{-}155$)} \\

& DTT only   & \makecell[c]{2974 ($\sigma\mbox{-}194$)}      & \makecell[c]{2851 ($\sigma\mbox{-}81$)}  & \makecell[c]{3281 ($\sigma\mbox{-}173$)}      & \makecell[c]{2855 ($\sigma\mbox{-}115$)}  \\
    \cline{2-6}
& \DTname\   & \makecell[c]{\textbf{3909 ($\sigma\mbox{-}101$)}}       & \makecell[c]{\textbf{3895 ($\sigma\mbox{-}81$)}} & \makecell[c]{\textbf{3965 ($\sigma\mbox{-}83$)}}       & \makecell[c]{\textbf{3852 ($\sigma\mbox{-}69$)}} \\ 

    \bottomrule
  \end{tabular}
\vspace{-0.3cm}
\end{table}

\begin{table}
\vspace{-0.3cm}
    \caption{Quantitative performance of Mujoco HalfCheetah-v3 tasks under weight uncertainty conditions.}
  \label{tab:Weight pollution mujoco HC}
  \centering
    % \scriptsize
  %\fontsize{7pt}{\baselineskip}\selectfont
 \small
  \setlength\tabcolsep{2pt}
  \begin{tabular}{llllll}
    \toprule
     
     & & \multicolumn{1}{c}{\textbf{LIF} ($T=5$)}     & \multicolumn{1}{c}{\textbf{SRM} ($T=5$)} & \multicolumn{1}{c}{\textbf{LIF} ($T=25$)}     & \multicolumn{1}{c}{\textbf{SRM} ($T=25$)} \\
    \cmidrule(r){3-3}
\cmidrule(r){4-4}
\cmidrule(r){5-5}
\cmidrule(r){6-6}
 
      \textbf{Type} & \textbf{Name}  & \makecell[c]{Reward$\uparrow$}        &  \makecell[c]{Reward$\uparrow$}  & \makecell[c]{Reward$\uparrow$}        &  \makecell[c]{Reward$\uparrow$}    \\    \hline
    \makecell[c]{\multirow{6}{*}{\makecell[c]{8-bit \\ Loihi \\ weight}}}
    & PopSAN  & \makecell[c]{10728 ($\sigma\mbox{-}47$)}         & \makecell[c]{10802 ($\sigma\mbox{-}32$)}   & \makecell[c]{10926 ($\sigma\mbox{-}59$)}         & \makecell[c]{10850 ($\sigma\mbox{-}44$)}
 \\
    & DT1~\cite{hao2020biologically}   & \makecell[c]{6026 ($\sigma\mbox{-}63$)}     &  \makecell[c]{6569 ($\sigma\mbox{-}46$)}    & \makecell[c]{5883 ($\sigma\mbox{-}102$)}     &  \makecell[c]{6420 ($\sigma\mbox{-}97$)}  \\
    & DT2~\cite{kim2021spiking} & \makecell[c]{4372 ($\sigma\mbox{-}54$)}   & \makecell[c]{4629 ($\sigma\mbox{-}50$)}  & \makecell[c]{4301 ($\sigma\mbox{-}87$)}   & \makecell[c]{4636 ($\sigma\mbox{-}74$)}   \\
    \cline{2-6}

    & DET only & \makecell[c]{9455 ($\sigma\mbox{-}125$)}    & \makecell[c]{9398 ($\sigma\mbox{-}60$)}    & \makecell[c]{9474 ($\sigma\mbox{-}137$)}    & \makecell[c]{9376 ($\sigma\mbox{-}82$)}         \\
    & DTT only  & \makecell[c]{9803 ($\sigma\mbox{-}44$)}      & \makecell[c]{9636 ($\sigma\mbox{-}84$)}  & \makecell[c]{9968 ($\sigma\mbox{-}69$)}      & \makecell[c]{9645 ($\sigma\mbox{-}113$)}   \\
    \cline{2-6}

    & \DTname\  &  \makecell[c]{\textbf{10823 ($\sigma\mbox{-}37$)}}      & \makecell[c]{\textbf{11767 ($\sigma\mbox{-}45$)}} &  \makecell[c]{\textbf{10990 ($\sigma\mbox{-}61$)}}      & \makecell[c]{\textbf{11760 ($\sigma\mbox{-}68$)}}
\\

\hline
 \makecell[c]{\multirow{6}{*}{\makecell[c]{GN \\ weight}}}   & PopSAN  & \makecell[c]{4640 ($\sigma\mbox{-}510$)}  &  \makecell[c]{3583 ($\sigma\mbox{-}347$)}  & \makecell[c]{4816 ($\sigma\mbox{-}583$)}  &  \makecell[c]{3597 ($\sigma\mbox{-}426$)}              \\
&  DT1~\cite{hao2020biologically}         & \makecell[c]{4483 ($\sigma\mbox{-}491$)}       & \makecell[c]{4128 ($\sigma\mbox{-}754$)}        & \makecell[c]{4365 ($\sigma\mbox{-}466$)}       & \makecell[c]{4051 ($\sigma\mbox{-}760$)}       \\

&  DT2~\cite{kim2021spiking}   & \makecell[c]{1334 ($\sigma\mbox{-}616$)}       &  \makecell[c]{2028 ($\sigma\mbox{-}1026$)}   & \makecell[c]{1402 ($\sigma\mbox{-}721$)}       &  \makecell[c]{1982 ($\sigma\mbox{-}993$)} 
\\
    \cline{2-6}
& DET only  & \makecell[c]{5251 ($\sigma\mbox{-}859$)}      & \makecell[c]{5032 ($\sigma\mbox{-}705$)}    & \makecell[c]{5313 ($\sigma\mbox{-}801$)}      & \makecell[c]{5035 ($\sigma\mbox{-}652$)}  \\

& DTT only   & \makecell[c]{4013 ($\sigma\mbox{-}423$)}       & \makecell[c]{6250 ($\sigma\mbox{-}368$)}   & \makecell[c]{4238 ($\sigma\mbox{-}468$)}       & \makecell[c]{6327 ($\sigma\mbox{-}403$)}  \\
    \cline{2-6}
& \DTname\   & \makecell[c]{\textbf{6928 ($\sigma\mbox{-}373$)}}      & \makecell[c]{\textbf{8381 ($\sigma\mbox{-}320$)}}  & \makecell[c]{\textbf{6957 ($\sigma\mbox{-}429$)}}      & \makecell[c]{\textbf{8321 ($\sigma\mbox{-}352$)}}  \\
\hline
  \multirow{6}{*}{\makecell[c]{ $30\%$ \\ Zero \\ weight}} &
    PopSAN & \makecell[c]{5020 ($\sigma\mbox{-}923$)}        & \makecell[c]{3233 ($\sigma\mbox{-}879$)}   & \makecell[c]{5078 ($\sigma\mbox{-}1031$)}        & \makecell[c]{3304 ($\sigma\mbox{-}950$)}  \\

& DT1~\cite{hao2020biologically}     & \makecell[c]{3995 ($\sigma\mbox{-}1319$)}      &  \makecell[c]{3503 ($\sigma\mbox{-}571$)}  & \makecell[c]{3927 ($\sigma\mbox{-}1406$)}      &  \makecell[c]{3484 ($\sigma\mbox{-}772$)}    \\

 & DT2~\cite{kim2021spiking}  &   \makecell[c]{2721 ($\sigma\mbox{-}1281$)}    &   \makecell[c]{3056 ($\sigma\mbox{-}555$)}    &   \makecell[c]{2713 ($\sigma\mbox{-}1352$)}    &   \makecell[c]{3002 ($\sigma\mbox{-}582$)}  \\
    \cline{2-6}
& DET only & \makecell[c]{4436 ($\sigma\mbox{-}801$)}     & \makecell[c]{4682 ($\sigma\mbox{-}540$)}  & \makecell[c]{4406 ($\sigma\mbox{-}822$)}     & \makecell[c]{4692 ($\sigma\mbox{-}515$)}  \\

& DTT only    & \makecell[c]{3583 ($\sigma\mbox{-}692$)}      & \makecell[c]{3268 ($\sigma\mbox{-}641$)}  & \makecell[c]{3604 ($\sigma\mbox{-}662$)}      & \makecell[c]{3359 ($\sigma\mbox{-}705$)}  \\
    \cline{2-6}
& \DTname\   &  \makecell[c]{\textbf{6551 ($\sigma\mbox{-}679$)}}       & \makecell[c]{\textbf{5386 ($\sigma\mbox{-}443$)}}  &  \makecell[c]{\textbf{6619 ($\sigma\mbox{-}712$)}}       & \makecell[c]{\textbf{5474 ($\sigma\mbox{-}388$)}}  \\ 

    \bottomrule
  \end{tabular}
\vspace{-0.3cm}
\end{table}

\subsection*{Assessment---Homeostatic} 
% We use the same three metrics (\ie FR$_m$, FR$_{std}^m$, and FR$_{std}^m$) as the ones used in the robot obstacle avoidance tasks to measure the homeostasis of an SNN in HalfCheetah-v3 studies. In the context of the HalfCheetah-v3 tasks, a trial means an episode. Hence, based on our evaluation settings, the three metrics of an SNN are calculated based on 100 episodes (\ie 10 episodes x 10 evaluations). In Figure~\ref{fig:half_h_changes}, we show the changes in these three metrics when transferring from the baseline condition to all other experimental settings. 

In the main manuscript, the changes in the quantified homeostasis values with respect to the base condition (\ie the normal Mujoco testing condition) under $T=5$ are illustrated. The raw homeostasis measurements and the corresponding changes used for plotting the polar chart in the main manuscript are reported in Table~\ref{SMtab:HC HOME T5}. In addition, we also provide the experimental homeostasis results obtained under $T=25$ in Table~\ref{SMtab:HC HOME T25}. The corresponding polar plots obtained under the $T=5$ and $T=25$ setups are shown in Figures~\ref{fig:SN_HC_results}c-f.

\noindent
The results are consistent with those obtained in the obstacle avoidance tasks. The proposed \DTname\ scheme offers the strongest homeostasis, indicating the effectiveness of the proposed dynamic threshold scheme. The essential goal of homeostasis is to enhance the host SNN's performance. Therefore, we expect the SNNs with stronger homeostasis (\ie smaller $\Delta\text{FR}_m$, $\Delta\text{FR}_{std}^m$, and $\Delta\text{FR}_{std}^s$ values) to outperform those with weaker homeostasis. Our experimental results confirm this expectation.

% The proposed \DTname\ offers the strongest homeostasis to the host SNNs among all competing approaches. Correspondingly, the SNNs with \DTname\ scheme perform the best in all conditions. The opposite also holds. For example, in the `Random joint velocity' section of Figure~\ref{fig:half_h_changes}(a), (b), and (c), DT1 shows the maximum changes in all three metrics. Correspondingly, DT1 hosted by a LIF-based SNN shows the worst performance under `Random joint velocity' experiments (see Table~\ref{tab:Weight pollution mujoco HC}). However, the opposite relationships are not as consistent as the positive relationships, meaning we should focus on the smallest changes more than the largest changes. 
 
\subsection*{Assessment---Ablation Studies}
The ablation study results are reported in the rows named ``DET only'' and ``DTT only'' in Tables~\ref{tab:Degraded environment mujoco HC}, ~\ref{tab:Degraded inputs mujoco HC}, and ~\ref{tab:Weight pollution mujoco HC}. In addition, the results are illustrated in Figure~\ref{fig:SN_HC_results}. The results reflect the same facts that we observed in the obstacle avoidance tasks. The dynamic threshold schemes with only the DET or DTT components cannot effectively regulate the firing rate statuses of the host SNNs, prohibiting meaningful homeostasis. For the LIF-based host SNNs, one extreme example is illustrated in the ``30\% Zero weight" sections of Figures~\ref{fig:SN_HC_results}c and e, where `DTT only' reports the largest change among all competing approaches under all experimental conditions in terms of $\Delta\text{FR}_{std}^m$. With the $T=25$ setup, as shown in Figures~\ref{fig:SN_HC_results}d and f, the $\Delta\text{FR}_m$ values of `DTT only' in the ``GN weight" sections are the largest across all experimental settings.   

\begin{table}
  \caption{The raw homeostasis measurements and the corresponding changes with respect to the baseline condition in Mujoco HalfCheetah-v3 tasks with $T=5$.}
%   \caption{Firing rate evaluation test of different methods on different SNN models in successful trials ($T=5$)}
  \label{SMtab:HC HOME T5}
  \centering
  \scriptsize
  \setlength\tabcolsep{4pt}
  \begin{tabular}{llllllll}
    \toprule
     
     & & \multicolumn{3}{c}{\textbf{LIF} ($T=5$)}     & \multicolumn{3}{c}{\textbf{SRM} ($T=5$)}                \\
    \cmidrule(r){3-5}
    \cmidrule(r){6-8}
     \textbf{Type} & \textbf{Name}  & \makecell[c]{$\text{FR}_m (\Delta)$}        & \makecell[c]{$\text{FR}_{std}^m (\Delta)$}     & \makecell[c]{$\text{FR}_{std}^s (\Delta)$}         & \makecell[c]{$\text{FR}_m (\Delta)$}        & \makecell[c]{$\text{FR}_{std}^m (\Delta)$}     & \makecell[c]{$\text{FR}_{std}^s (\Delta)$}     \\ 
    \hline
    \multirow{7}{*}{\makecell[c]{baseline \\ condition}}
    & PopSAN  &0.433   & 0.228  & 0.000978  & 0.427 & 0.241 &  0.002146\\
    & DT1~\cite{hao2020biologically}   & 0.412  & 0.239  & 0.001342  & 0.474  & 0.248 & 0.002166 \\
    & DT2~\cite{kim2021spiking}     & 0.697  &  0.298  &   0.000911  & 0.530  & 0.302 & 0.001472\\

    & DET only   & 0.284 & 0.220 &  0.001084 & 0.335 & 0.243 & 0.001558\\
    & DTT only &  0.646  & 0.257  & 0.002291 & 0.501 & 0.334 & 0.002541\\
    & \DTname\  & 0.249  &  0.190 & 0.001152 & 0.212 & 0.160 & 0.000952 \\
    \hline
    \multirow{7}{*}{\makecell[c]{Random \\ joint \\ position}}
    & PopSAN  &  0.426 (0.007) & 0.237 (0.009) & 0.001230 (0.000252) & 0.440 (0.013) & 0.258 (0.017) & 0.002852 (0.000706) \\
    & DT1~\cite{hao2020biologically}    &  0.435 (0.023) & 0.252 (0.013) & 0.001713 (0.000371) & 0.426 (0.048) & 0.269 (0.021) & 0.004145 (0.001979) \\
    & DT2~\cite{kim2021spiking}     & 0.686 (0.011)  & 0.289 (0.009)  & 0.001239 (0.000328) & 0.508 (0.022) & 0.333 (0.031) & 0.002164 (0.000692) \\

    & DET only   & 0.289 (0.005)  & 0.227 (0.007) &  0.001323 (0.000239) & 0.347 (0.012) & 0.261 (0.018) & 0.002006 (0.000448) \\
    & DTT only & 0.640 (0.006) &   0.263 (0.006)  &  0.002077 (0.000214) & 0.521 (0.020) & 0.380 (0.046) & 0.003124 (0.000583) \\
    & \DTname\  & 0.246 \textbf{(0.003)} & 0.186 \textbf{(0.004)} & 0.001268 \textbf{(0.000116)} & 0.209 \textbf{(0.003)} & 0.152 \textbf{(0.008)} & 0.001071 \textbf{(0.000119)} \\
    \hline
    \multirow{7}{*}{\makecell[c]{Random \\ joint \\ velocity}}
    & PopSAN  & 0.439 (0.006) & 0.240 (0.012) & 0.001502 (0.000524) & 0.453 (0.026) & 0.314 (0.073) & 0.001513 (0.000633)\\
   
    & DT1~\cite{hao2020biologically}    &  0.381 (0.031) & 0.259 (0.020) & 0.002602 (0.001260) & 0.510 (0.036) & 0.261 (0.013) & 0.004051 (0.001885)\\
    & DT2~\cite{kim2021spiking}     & 0.690 (0.007) & 0.289 (0.009) & 0.001725 (0.000814) & 0.487 (0.043) & 0.340 (0.038) & 0.001896 (0.000424)\\

    & DET only   & 0.280 \textbf{(0.004)} & 0.214 (0.006) & 0.000905 \textbf{(0.000179)} & 0.351 (0.016) & 0.219 (0.024) & 0.001846 (0.000288)\\
    & DTT only & 0.656 (0.010) & 0.246 (0.011) & 0.002027 (0.000264) & 0.550 (0.049) & 0.355 (0.021) & 0.002891 (0.000350)\\
    & \DTname\  & 0.245 \textbf{(0.004)}    & 0.186 \textbf{(0.004)} & 0.001336 (0.000184) & 0.204 \textbf{(0.008)} & 0.168 \textbf{(0.008)} & 0.001104 \textbf{(0.000152)} \\
    \hline
    \multirow{7}{*}{\makecell[c]{GN}}
    & PopSAN  &  0.418 (0.015) & 0.243 (0.015) & 0.001400 (0.000422) & 0.476 (0.049) & 0.221 (0.020) & 0.002481 (0.000335)\\
    
    & DT1~\cite{hao2020biologically}    & 0.423 (0.011) & 0.225 (0.014) & 0.001623 (0.000281) & 0.535 (0.061) & 0.283 (0.035) & 0.004810 (0.002644)\\
    & DT2~\cite{kim2021spiking}     &0.680 (0.017) &  0.312 (0.014) &  0.001273 (0.000362) & 0.481 (0.049) & 0.362 (0.060) & 0.002215 (0.000743)   \\

    & DET only   &  0.278 (0.006) & 0.212 (0.008) & 0.001353 (0.000269) & 0.302 (0.033) & 0.277 (0.034) & 0.002411 (0.000853) \\
    & DTT only & 0.638 (0.008) & 0.269 (0.012) &  0.002448 (0.000157) & 0.434 (0.067) & 0.301 (0.033) & 0.002062 (0.000479)\\
    & \DTname\  &0.245 \textbf{(0.004)}  &  0.184 \textbf{(0.006)}  & 0.001300 \textbf{(0.000148)}  & 0.225 \textbf{(0.013)} & 0.171 \textbf{(0.011)} & 0.001093 \textbf{(0.000141)}\\
    \hline
    \multirow{7}{*}{\makecell[c]{8-bit \\ Loihi \\ weight}}
    & PopSAN  & 0.430 (0.003) & 0.221 (0.007) & 0.001061 (0.000083) & 0.420 (0.007) & 0.252 (0.011) & 0.001847 (0.000299)\\
    
    & DT1~\cite{hao2020biologically}    &  0.424 (0.012) & 0.248 (0.009) & 0.001285 (0.000057) & 0.442 (0.032) & 0.230 (0.018) & 0.002520 (0.000354)\\
    & DT2~\cite{kim2021spiking}      &  0.678 (0.019) & 0.285 (0.013) & 0.001022 (0.000111) & 0.492 (0.038) & 0.320 (0.018) & 0.001701 (0.000229) \\

    & DET only   &  0.290 (0.006) & 0.229 (0.009) & 0.001211 (0.000127) & 0.327 (0.008) & 0.235 (0.008) & 0.001303 (0.000255)\\
    & DTT only &  0.655 (0.009) & 0.264 (0.007) & 0.002402 (0.000111) & 0.488 (0.013) & 0.343 (0.009) & 0.002707 (0.000166)\\
    & \DTname\  &  0.249 \textbf{(0.000)}  &  0.186 \textbf{(0.004)} & 0.001114 \textbf{(0.000038)} & 0.215 \textbf{(0.003)} & 0.163 \textbf{(0.003)} & 0.000907 \textbf{(0.000045)}\\
    \hline
    \multirow{7}{*}{\makecell[c]{GN \\ weight}}
    & PopSAN  &  0.456 (0.023) & 0.210 (0.018) & 0.001249 (0.000271) & 0.464 (0.037) & 0.305 (0.064) & 0.003358 (0.001212)\\
    
    & DT1~\cite{hao2020biologically}    &  0.426 (0.014) & 0.223 (0.016) & 0.001004 (0.000338) & 0.429 (0.045) & 0.285 (0.037) & 0.003702 (0.001536)\\
    & DT2~\cite{kim2021spiking}     & 0.678 (0.019) &  0.316 (0.018) &  0.001381 (0.000470) & 0.503 (0.027) & 0.362 (0.060) & 0.002172 (0.000700)\\

    & DET only   &  0.271 (0.013) & 0.227 (0.007) & 0.001385 (0.000301) & 0.364 (0.029) & 0.208 (0.035) & 0.001042 (0.000516)\\
    & DTT only & 0.626 (0.020) & 0.281 (0.024) & 0.001972 (0.000319) & 0.562 (0.061) & 0.287 (0.047) & 0.004133 (0.001592)\\
    & \DTname\  & 0.256 \textbf{(0.007)} &  0.185 \textbf{(0.005)} & 0.001264 \textbf{(0.000112)} & 0.219 \textbf{(0.007)} & 0.165 \textbf{(0.005)} & 0.001049 \textbf{(0.000097)}\\
    \hline
    \multirow{7}{*}{\makecell[c]{30\% \\ Zero \\ weight}}
    & PopSAN  & 0.502 (0.069) & 0.220 (0.008) & 0.001441 (0.000463) & 0.412 (0.015) & 0.279 (0.038) & 0.003522 (0.001376)\\

    & DT1~\cite{hao2020biologically}    & 0.439 (0.027) & 0.256 (0.017) & 0.001784 (0.000442) & 0.436 (0.038) & 0.263 (0.015) & 0.001216 (0.000950) \\
    & DT2~\cite{kim2021spiking}     & 0.675 (0.022) &  0.325 (0.027) &  0.001327 (0.000416) & 0.472 (0.058) & 0.258 (0.044) & 0.000994 (0.000478)\\

    & DET only   & 0.268 (0.016) & 0.210 (0.010) & 0.001329 (0.000245) & 0.370 (0.035) & 0.210 (0.033)  &0.003205 (0.001647)\\
    & DTT only & 0.680 (0.034) &  0.338 (0.081)  & 0.002804 (0.000513) & 0.485 (0.016) & 0.317 (0.017) & 0.001024 (0.001517) \\
    & \DTname\  & 0.243 \textbf{(0.006)} &  0.184 \textbf{(0.006)}  &  0.001306 \textbf{(0.000154)} & 0.217 \textbf{(0.005)} & 0.154 \textbf{(0.006)} & 0.001058 \textbf{(0.000106)}\\
    
    \bottomrule
  \end{tabular}
\end{table}

% \begin{figure}[ht!]
% 	\centering
% 	\includegraphics [scale=0.15]{figures/half_homeostasis.png}
% 	\vspace{-0.3cm}
% 	\caption{
% 		\bd{The changes of quantified homeostasis with respect to the base condition in Mujoco HalfCheetah-v3.}
% % 		Firing rate evaluation test of different methods on different SNN models in success trials.
% 	}
% 	\label{fig:half_h_changes}
% 	\vspace{-0.5cm}
% \end{figure}

\begin{table}
  \caption{The raw homeostasis measurements and the corresponding changes with respect to the baseline condition in Mujoco HalfCheetah-v3 tasks with the $T=25$ setup.}
%   \caption{Firing rate evaluation test of different methods on different SNN models in successful trials ($T=5$)}
  \label{SMtab:HC HOME T25}
  \centering
  \scriptsize
  \setlength\tabcolsep{4pt}
  \begin{tabular}{llllllll}
    \toprule
     
     & & \multicolumn{3}{c}{\textbf{LIF} ($T=25$)}     & \multicolumn{3}{c}{\textbf{SRM} ($T=25$)}                \\
    \cmidrule(r){3-5}
    \cmidrule(r){6-8}
     \textbf{Type} & \textbf{Name}  & \makecell[c]{$\text{FR}_m (\Delta)$}        & \makecell[c]{$\text{FR}_{std}^m (\Delta)$}     & \makecell[c]{$\text{FR}_{std}^s (\Delta)$}         & \makecell[c]{$\text{FR}_m (\Delta)$}        & \makecell[c]{$\text{FR}_{std}^m (\Delta)$}     & \makecell[c]{$\text{FR}_{std}^s (\Delta)$}     \\ 
    \hline
    \multirow{7}{*}{\makecell[c]{baseline \\ condition}}
    & PopSAN  & 0.436    & 0.230   & 0.001156    & 0.440  & 0.252   & 0.002217  \\
    & DT1~\cite{hao2020biologically}   & 0.420 & 0.240 & 0.001158 & 0.470 & 0.247 & 0.001869 \\
    & DT2~\cite{kim2021spiking}     & 0.676  & 0.290 & 0.000939 & 0.521 & 0.305 & 0.001785\\

    & DET only   & 0.292 & 0.225 & 0.001237  & 0.341  & 0.253 & 0.001631\\
    & DTT only & 0.635 & 0.257 & 0.002433  & 0.493 & 0.340 & 0.002722 \\
    & \DTname\  & 0.251 & 0.192 & 0.001292 & 0.215 & 0.173 & 0.001074 \\
    \hline
    \multirow{7}{*}{\makecell[c]{Random \\ joint \\ position}}
    & PopSAN  &   0.426 (0.010) &  0.238 (0.008) &  0.001381 (0.000225) &  0.458 (0.018) &  0.264 (0.012) &  0.003048 (0.000831) \\
    & DT1~\cite{hao2020biologically}    &   0.440 (0.020) &   0.258 (0.018) &   0.001721 (0.000563) &  0.442 (0.028) &  0.268 (0.021) &  0.003632 (0.001763) \\
    & DT2~\cite{kim2021spiking}     &   0.648 (0.028) &  0.272 (0.018) &  0.001348 (0.000409) &  0.501 (0.020) &  0.342 (0.037) &  0.002384 (0.000599) \\

    & DET only   &   0.301 (0.009) &  0.236 (0.011) &  0.001464 (0.000227) &  0.359 (0.018) &  0.285 (0.032) &  0.002179 (0.000548) \\
    & DTT only   &   0.630 (0.005) &  0.265 (0.008) &  0.002104 (0.000329) &  0.518 (0.025) &  0.372 (0.032) &  0.003438 (0.000716) \\
    & \DTname\  &   0.247 \textbf{(0.004)} &  0.187 \textbf{(0.005)} &  0.001431 \textbf{(0.000139)} &  0.210 \textbf{(0.005)} &  0.163 \textbf{(0.010)} &  0.001242 \textbf{(0.000168)} \\
    \hline
    \multirow{7}{*}{\makecell[c]{Random \\ joint \\ velocity}}
    & PopSAN  &   0.450 (0.014) &  0.239 (0.009) &  0.001425 (0.000269) &  0.474 (0.034) &  0.332 (0.080) &  0.002922 (0.000705) \\
    & DT1~\cite{hao2020biologically}    &   0.387 (0.033) &  0.258 (0.018) &  0.002474 (0.001316) &  0.427 (0.043) &  0.268 (0.021) &  0.003572 (0.001703) \\
    & DT2~\cite{kim2021spiking}     &   0.664 (0.012) &  0.261 (0.029) &  0.002582 (0.001643) &  0.487 (0.034) &  0.347 (0.042) &  0.002529 (0.000744) \\

    & DET only   &   0.310 (0.018) &  0.235 (0.010) &  0.001582 (0.000345) &  0.368 (0.027) &  0.292 (0.039) &  0.002544 (0.000913) \\
    & DTT only   &   0.627 (0.008) &  0.269 (0.012) &  0.001548 (0.000885) &  0.515 (0.022) &  0.370 (0.030) &  0.003282 (0.000560) \\
    & \DTname\  &   0.245 \textbf{(0.006)} &  0.185 \textbf{(0.007)} &  0.001478 \textbf{(0.000186)} &  0.208 \textbf{(0.007)} &  0.183 \textbf{(0.010)} &  0.001305 \textbf{(0.000231)} \\
    \hline
    \multirow{7}{*}{\makecell[c]{GN}}
    & PopSAN  &   0.423 (0.013) &  0.252 (0.022) &  0.001633 (0.000477) &  0.403 (0.037) &  0.236 (0.016) &  0.002574 (0.000357) \\
    & DT1~\cite{hao2020biologically}    &   0.433 (0.013) &  0.221 (0.019) &  0.002061 (0.000903) &  0.552 (0.082) &  0.271 (0.024) &  0.003784 (0.001915) \\
    & DT2~\cite{kim2021spiking}     &   0.642 (0.034) &  0.310 (0.020) &  0.001385 (0.000446) &  0.480 (0.041) &  0.373 (0.068) &  0.002833 (0.001048) \\

    & DET only   &   0.281 (0.011) &  0.219 \textbf{(0.006)} &  0.001610 (0.000373) &  0.304 (0.037) &  0.290 (0.037) &  0.003082 (0.001451) \\
    & DTT only   &   0.622 (0.013) &  0.274 (0.017) &  0.002762 (0.000329) &  0.453 (0.040) &  0.305 (0.035) &  0.002048 (0.000674) \\
    & \DTname\  &   0.243 \textbf{(0.008)} &  0.184 (0.008) &  0.001512 \textbf{(0.000220)} &  0.226 \textbf{(0.011)} &  0.180 \textbf{(0.007)} &  0.001283 \textbf{(0.000209)} \\
    \hline
    \multirow{7}{*}{\makecell[c]{8-bit \\ Loihi \\ weight}}
    & PopSAN  &   0.432 (0.004) &  0.224 (0.006) &  0.001310 (0.000154) &  0.452 (0.012) &  0.238 (0.014) &  0.001849 (0.000368) \\
    & DT1~\cite{hao2020biologically}    &   0.427 (0.007) &  0.221 (0.019) &  0.001035 (0.000123) &  0.485 (0.015) &  0.259 (0.012) &  0.002363 (0.000494) \\
    & DT2~\cite{kim2021spiking}     &   0.661 (0.015) &  0.278 (0.012) &  0.001174 (0.000235) &  0.535 (0.014) &  0.328 (0.023) &  0.001976 (0.000191) \\

    & DET only   &   0.299 (0.007) &  0.234 (0.009) &  0.001379 (0.000142) &  0.351 (0.010) &  0.267 (0.014)  &  0.001275 (0.000356) \\
    & DTT only   &   0.644 (0.009) &  0.242 (0.015) &  0.002210 (0.000223) &  0.506 (0.013) &  0.354 (0.014)  &  0.002894 (0.000172) \\
    & \DTname\  &   0.250 \textbf{(0.001)} &  0.197 \textbf{(0.005)} &  0.001393 \textbf{(0.000101)} &  0.211 \textbf{(0.004)} &  0.178 \textbf{(0.005)} &  0.001169 \textbf{(0.000094)} \\
    \hline
    \multirow{7}{*}{\makecell[c]{GN \\ weight}}
    & PopSAN  &   0.471 (0.035) &  0.211 (0.019) &  0.001637 (0.000481) &  0.479 (0.039) &  0.336 (0.084) &  0.003181 (0.000964) \\
    & DT1~\cite{hao2020biologically}    &   0.433 \textbf{(0.013)} &   0.218 (0.022) &  0.000904 (0.000254) &  0.438 (0.032) &  0.302 (0.055) &  0.004041 (0.002172) \\
    & DT2~\cite{kim2021spiking}     &   0.642 (0.034) &  0.320 (0.030) &  0.001683 (0.000744) &  0.492 (0.029) &  0.366 (0.061) &  0.004585 (0.002800) \\

    & DET only   &   0.271 (0.021) &  0.238 (0.013) &  0.001720 (0.000483) &  0.369 (0.028) &  0.202 (0.051) &  0.003927 (0.002296) \\
    & DTT only   &   0.607 (0.028) &  0.289 (0.032) &  0.003104 (0.000671) &  0.569 (0.076) &  0.301 (0.039) &  0.004273 (0.001551) \\
    & \DTname\  &   0.264 \textbf{(0.013)} &  0.183 \textbf{(0.009)} &  0.001512 \textbf{(0.000220)} &  0.229 \textbf{(0.014)} &  0.182 \textbf{(0.009)} &  0.001199 \textbf{(0.000125)} \\
    \hline
    \multirow{7}{*}{\makecell[c]{30\% \\ Zero \\ weight}}
    & PopSAN  &   0.493 (0.057) &  0.215 (0.015) &  0.001892 (0.000736) &  0.410 (0.030) &  0.292 (0.040) &  0.003237 (0.001020) \\
    & DT1~\cite{hao2020biologically}    &   0.447 (0.027) &  0.258 (0.018) &  0.001859 (0.000701) &  0.424 (0.046) &  0.288 (0.041) &  0.000926 (0.000943) \\
    & DT2~\cite{kim2021spiking}     &   0.655 (0.021) &  0.334 (0.044) &  0.001674 (0.000735) &  0.486 (0.035) &  0.251 (0.054) &  0.000896 (0.000889) \\

    & DET only   &   0.273 (0.019) &  0.239 (0.014) &  0.001692 (0.000455) &  0.371 (0.030) &  0.216 (0.037) &  0.004106 (0.002475) \\
    & DTT only   &   0.677 (0.042) &  0.305 (0.048) &  0.002976 (0.000543) &  0.426 (0.067) &  0.312 (0.028) &  0.001176 (0.001546) \\
    & \DTname\  &   0.239 \textbf{(0.012)} &  0.181 \textbf{(0.011)} &  0.001642 \textbf{(0.000350)} &  0.221 \textbf{(0.006)} &  0.180 \textbf{(0.007)} &  0.001183 \textbf{(0.000109)} \\
    
    \bottomrule
  \end{tabular}
\end{table}

% \begin{figure}[ht!]
% 	\centering
% 	\includegraphics [scale=0.15]{figures/T25_half_homeostasis.png}
% 	\vspace{-0.3cm}
% 	\caption{
% 		\bd{The changes of quantified homeostasis with respect to the base condition in Mujoco HalfCheetah-v3.(T=25)}
% % 		Firing rate evaluation test of different methods on different SNN models in success trails.
% 	}
% 	\label{fig:T25_half_h_changes}
% 	\vspace{-0.5cm}
% \end{figure}
