# Supplementary material for: Biologically Inspired Dynamic Thresholds for Spiking Neural Networks
Source: arXiv:2206.04426 source file (2023-06-19)
Supplement: Supplementary file 3 [file CC_HC_experimental_details.tex]

\noindent
In this section, we provide additional experimental details related to SNNs’ inputs and training process in continuous control tasks.

\noindent
\djc{
\tb{SNNs Input}
In HalfCheetah-v3, the state consists of 17-D data, where the first 8-D is joint position information, the last 9-D is joint velocity information, and the action space is 6-D joint torque. Specifically, $s = \{J_p, J_v\}$, where $J_p$ and $J_v$ are the relative $8$-D joint position and $9$-D joint velocity information, respectively. $a = \{b_t, b_s, b_f, f_t, f_s, f_f\}$, where $b_t$, $b_s$ and $b_f$ are the torques of the behind thigh, shin and foot respectively, and $f_t$, $f_s$ and $f_f$ are the torques of the front thigh, shin and foot respectively. The reward consists of the difference between the value of the forward velocity and the energy consumption of the joint. 
} 

\noindent
\djc{
In Ant-v3, the state consists of 111-D data, where the first 13-D is joint position information, the middle 14-D is joint velocity information, the last 84-D is contact force, and the action space is 8-D joint torque. Specifically, $s = \{J_p, J_v, J_f\}$, where $J_p$, $J_v$ and $J_f$ are the relative $13$-D joint position, $14$-D joint velocity and $84$-D joint contact force information, respectively. $a = \{h_1, h_2, h_3, h_4, a_1, a_2, a_3, a_4\}$, where $h_1$, $h_2$, $h_3$ and $h_4$ are the torques of the 4 hip joints, and $a_1$, $a_2$, $a_3$ and $a_4$ are the torques of the 4 ankle joints. The reward consists of the difference between the positive reward and the negative reward, where the positive reward includes forward velocity reward and health reward, and the negative reward includes joint energy consumption and contact force consumption.
} 

\noindent
\djc{
Our evaluation baseline model is the population-coded spiking actor network (PopSAN)~\cite{tang2020deep}. PopSAN is an improved version of SAN~\cite{tang2020reinforcement} to accommodate high-dimensional control tasks. It consists of population encode, SAN and population decode. In HalfCheetah-v3, population encode encodes 17-D state information into 170-D spike trains through a layer of fully connected networks. Then processed through the SAN, which is a fully connected three-layer SNN (\ie two 256-neuron hidden layers and one 60-neuron output layer). Finally, the 60-D spike signal is mapped to the 6-D action by population decoding through a layer of 1-D convolution with kernel size of 10.
}

\noindent
\djc{
\tb{Training Process}
We adopt PopSAN's training environments and training hyperparameter settings to train all competing SNNs. PopSAN is based on Twin Delayed Deep Deterministic Policy Gradient(TD3)~\cite{fujimoto2018addressing}. During the training, we set batch size as $100$ and learning rates as $0.0001$ for both actor and critic networks. We set reward discount factor as $0.99$ and maximum length of replay buffer as $1000000$. We use PyTorch~\cite{paszke2019pytorch} to train all competing SNNs with an i7-7700 CPU and NVIDIA GTX 1080Ti GPU.
}

% \djc{
%  We evaluated our method on the OpenAI gym~\cite{brockman2016openai} tasks with rich and unstable dynamics that are commonly used for benchmarking continuous control algorithms. To limit the effect of initialization, we trained 10 models for each algorithm corresponding to 10 random seeds. Each model was trained for 1 million steps and then the trained models are tested in a degraded environment. To compensate for the effect of randomness in the tasks, we computed the average reward for 10 evaluations with 10 episodes each, where each episode lasted for a maximum of 1000 execution steps.
% }

\noindent
\djc{
 We evaluated our method on the OpenAI gym~\cite{brockman2016openai} tasks with rich and unstable dynamics that are commonly used for benchmarking continuous control algorithms. To limit the effect of initialization, we trained 10 models for each algorithm corresponding to 10 random seeds. Each model was trained for 1 million steps and then the trained models are tested in a degraded environment. We choose the best-performing model for testing. To compensate for the effect of randomness in the tasks, we computed the average reward for 10 evaluations with 10 episodes each, where each episode lasted for a maximum of 1000 execution steps.
}
