# Supplementary material for: Biologically Inspired Dynamic Thresholds for Spiking Neural Networks
Source: arXiv:2206.04426 source file (2023-06-19)
Supplement: Supplementary file 4 [file Math_def.tex]

\noindent
In this section, we provide mathematical definitions for DT1, DT2, and Loihi weight transferring. In addition, we formally define the proposed homeostasis metrics. 

\noindent
\tb{DT1} 
Hao~\etal\cite{hao2020biologically} noted that neurons do not (or barely) fire when their thresholds are too large, which can negatively affect model performance. Therefore, they proposed DT1 to slow threshold growth. For the $i$-th neuron in the $l$-th layer, DT1 at timestamp $t$ is mathematically defined as: 

\begin{align}
    \Theta_{DT1,i}^{l}(t) &= \Theta_{const}+ (-\Theta_{DT1,i}^{l}(t-1)+\frac{\Theta_{initial}}{|2\Theta_{DT1,i}^{l}(t-1)-\Theta_{initial}|}\sum_{i=1}^{n^l}s_i^{l}(t)), \label{SMeq:DT1}
    % \Theta_{DT3,i}^{t,l} &= max(\Theta_{DT3,i}^{t-1,l}, max(w_{ij}*s_j^l(t))) \text{for } j= 1,2, ..., N^l, \label{eq:DT3}
\end{align}
where $\Theta_{const}$ and $\Theta_{initial}$ are two hyperparameters; the dynamic threshold is mainly controlled by a dynamic scaling factor $\frac{\Theta_{initial}}{|2\Theta_{DT1,i}^{l}(t-1)-\Theta_{initial}|}$; $n^l$ is the total number of neurons in the $l$-th layer. For fair comparisons with other competing approaches, we apply grid search to find the optimal values of $\Theta_{initial}$ and $\Theta_{const}$ and ensure that the host SNNs of DT1 offer similar success rates (SRs) in the static obstacle avoidance task to those of other approaches. Based on the grid search, $\Theta_{initial}$ is set to 10.0; 0.5 and 0.2 are the optimal values of $\Theta_{const}$ for the LIF-based and SRM-based host SNNs, respectively. 

\noindent
\tb{DT2} Inspired by the observed homeostasis in biology, Kim \etal\cite{kim2021spiking} proposed DT2 to maintain neurons' firing rates at a predefined constant target frequency. Mathematically, for the $i$-th neuron in the $l$-th layer, DT2 at timestamp $t$ is defined as:

\begin{align}
\Theta_{DT2,i}^{l}(t) &= \Theta_{DT2,i}^{l}(t-1)+(\sum_{i=1}^{n^l}s_i^{l}(t))-f_{target}^l)\times\Theta_{DT2,i}^{l}(t-1)\times\gamma, \label{SMeq:DT2}
\end{align}
where $f_{target}^l$ is the predefined constant target frequency; $\gamma$ is a homeostasis factor that determines the threshold changing rate. Based on our grid search, we set $f_{target}^l$ to 85 (\ie 1/3 of 256) for the three $256$-neuron layers and $\gamma$ to $0.004$ to achieve the same static obstacle avoidance performance as that of other competing SNNs.

% \tb{DT2} Kim \etal\cite{kim2021spiking} borrowed from the $k$-winner-take-all(kWAT) method to design dynamic thresholds that directly control the firing rate of neurons and maintain the firing rate always around an artificially set constant value through threshold adjustment (see Eq.~\ref{SMeq:DT2}). Kim \etal~\cite{kim2021spiking} believes DT2 can keep the firing frequency similar as homeostasis in biolog then the network can keep the firing rate almost constantly and all parameters balance well although the weights, one of the network components change at every training cycle according to the learning algorithm.
% %However, it would make the model lack the ability to discriminate between rapid changes. 
% In this paper, we set $\gamma=0.004$ based on the optimal results shown in~\cite{kim2021spiking} and $f_{target}^l$ as 85 (\ie 1/3 of 256). These settings ensure that the SR of DT1 and DT2 in the designed static testing environment is relatively the same (\ie within ±2\%, See Table~\ref{SMtab:Sta_test}) to the baseline.

% \begin{align}
% \Theta_{DT2,i}^{l}(t) &= \Theta_{DT2,i}^{l}(t-1)+(\sum_{i=1}^{N^l}s_i^{l}(t))-f_{target}^l)\times\Theta_{DT2,i}^{l}(t-1)\times\gamma, \label{SMeq:DT2}
% \end{align}

\noindent
\tb{8-Bit Loihi Weights}
In our weight uncertainty (WU) experiments, we scale and round up the learned floating-point synaptic weights to low-precision 8-bit weights. The weight scaling process is defined as:

\begin{align}
      r^{l} & = \frac{w_{\text{max}}^{\text{Loihi}}}{w_{\text{max}}^{l}},    \\
      w^{(l)(\text{Loihi})}_{ij} & = \text{round}(r^{l} w^{l}_{ij}), \\
      \Theta^{(l)(\text{Loihi})}_i(t) & = \text{round}(r^{l}\Theta^{l}_i(t)), \\
      v^{l}_i(t) & = v^{(l)(\text{Loihi})}_i(t) / r^{l},  \label{seq:loihi_v}
\end{align}
where $r^{l}$ is the rescaling ratio of layer $l$; $w_{max}^{\text{Loihi}}$ is the
maximum weight that Loihi supports; $w_{max}^{l}$ is the maximum weight of the $l$-th layer of the host SNN; $w_{ij}^{l}$ is the synaptic weight between the $i$-th neuron in the $l$-th layer and the $j$-th neuron in the $(l-1)$-th layer, and $w^{(l)(\text{Loihi})}_{ij}$ is the corresponding rescaled weight on Loihi; $\Theta^{l}_i(t)$ and $\Theta^{(l)(\text{Loihi})}_i(t)$ are the original membrane threshold and the corresponding threshold for Loihi of the $i$-th neuron in the $l$-th layer at timestamp $t$, respectively; $\text{round}(x)$ is a rounding function that returns the rounded version of $x$. Notably, to estimate $\Theta^{l}_i(t)$, we need to know the original membrane potentials. However, all the membrane potentials on Loihi are rescaled. Therefore, to obtain the original membrane potentials, we need to reverse the process defined in Eq~\ref{seq:loihi_v}.

\noindent
\tb{Homeostasis Metrics} We leverage three statistical metrics to quantify the homeostasis of an SNN. Mathematically, they are defined as follows:

\begin{align}
\text{FR}_m &= \mu(\text{FR}_m^p)\quad \text{for}\quad p=1,2,..., P,\\
\text{FR}_{std}^m &= \mu(\text{FR}_{std}^p)\quad \text{for}\quad p=1,2,...,P,\\
\text{FR}_{std}^s &= \sigma(\text{FR}_{std}^p)\quad \text{for}\quad p=1,2,...,P,\\
%\text{FR}_{cv} &= \text{FR}_{std} / \text{FR}_m; \\
\text{FR}_m^p &= \mu(f_i^{l,p}) \quad \text{for } i= 1,2, ..., N^l\quad l= 1,2, ..., L, \\
\text{FR}_{std}^p &= \sigma(f_i^{l,p}) \quad \text{for } i= 1,2, ..., N^l\quad l= 1,2, ..., L, \\
f^{l,p}_i &= \frac{\sum_{t^p=1}^{T^p}s_i^l(t^p)}{T^p}, 
\end{align}
where, $T^p$ is the time taken for the $p$-th trial and $f_i^{l,p}$ is the firing rate of the $i$-th neuron in the $l$-th layer during the $p$-th trial. $\text{FR}_m^p$ denotes the mean firing rate of all neurons of an SNN during the $p$-th trial, and $\text{FR}_{std}^p$ is the standard deviation of all neuron firing rates for an SNN during the $p$-th trial. The definitions of $\text{FR}_m$, $\text{FR}_{std}^m$, and $\text{FR}_{std}^s$ are defined in the main paper.
