# Supplementary material for: Biologically Inspired Dynamic Thresholds for Spiking Neural Networks
Source: arXiv:2206.04426 source file (2023-06-19)
Supplement: Supplementary file 5 [file OA_additional_with_CRP.tex]

\subsection*{Additional Quantitative Performance}
\label{SMsec:performance}
In this section, we provide additional experimental results related to obstacle avoidance performance. Specifically, we show the quantitative performance of all competing SNNs in static obstacle avoidance tasks. Besides the reported success rate (SR), we report the following two additional results, namely: Common routes percentage (CRP), the percentage of the successful routes that had the common start and goal positions across all competing SNNs to all successful trials of a specific SNN; b) Overtime percentage (OTP), the percentage of overtime trials to total trials (\ie 200 trials), where overtime is defined as the trial that the robot cannot reach the goal within 1000 steps but without touching any obstacle. 

% \tb{T=5} Table~\ref{SMtab:Sta_test}, Table~\ref{SMtab:Degraded environment}, Table~\ref{SMtab:Degraded inputs}, Table~\ref{SMtab:Weight pollution}

% We show the performance of all models under a normal condition (\ie the original SAN's static testing environment as shown in Figure~\ref{SMfig:env}(b)) in Table~\ref{SMtab:Sta_test}. For fairness, we apply grid search on all tunable hyperparameters to ensure the SRs of all competing approaches are relatively the same (\ie, within ±2\%) when testing in the designed static testing environment.

\noindent
The quantitative performance of all competing SNNs in static obstacle avoidance tasks are shown in Table~\ref{SMtab:Sta_test}. The corresponding testing environment is shown in Figure~\ref{SMfig:env}(b), where we adopt the same 200 start-goal pairs as the ones used for testing SAN. The SRs of all competing SNNs are relatively the same which is ensured by grid search on all tunable hyperparameters. There is no overtime trial among all experiments. Since the lowest SRs are pretty high (\ie 96\% for LIF and 95\% for SRM), the CRPs are also pretty high. 

\noindent
Table~\ref{SMtab:Degraded environment}, ~\ref{SMtab:Degraded inputs}, and ~\ref{SMtab:Weight pollution} show the quantitative performance of all competing approaches in dynamic obstacle, degraded inputs, and weight uncertain experiments, respectively. Since the lowest SRs lower than those obtained in static obstacle avoidance experiments, the CRPs reduce significantly. In terms of OTP, we witness high overtime trials in the `0.2' section of degraded inputs and the `GN weight' section of weight uncertain. 
As discussed in the main paper, with the `0.2' setup, the three disturbed lasers generate more spikes than it is supposed to, making the robot more cautious. Thus, it slows down the speed of the robot, introducing more over time trials. As expected, adding GN noise to learned weights reduces the effectiveness avoidance policy. However, our approach gets the most negligible impact, offering the best SRs.

\begin{table}

\caption{Quantitative performance of obstacle avoidance with static obstacles.}

  \label{SMtab:Sta_test}
  \centering
  
  \setlength\tabcolsep{5pt}
  
  \begin{tabular}{lllllll}
    \toprule
     
     & \multicolumn{3}{c}{\textbf{LIF ($T=5$)}}     & \multicolumn{3}{c}{\textbf{SRM ($T=5$)}}                \\
    \cmidrule(r){2-4}
    \cmidrule(r){5-7}
    \textbf{Name}  & \makecell[c]{SR$\uparrow$}    &  \makecell[c]{CRP}       & \makecell[c]{OTP}        & \makecell[c]{SR$\uparrow$}    &  \makecell[c]{CRP}       & \makecell[c]{OTP} \\
    \hline
    SAN  & \makecell[c]{98\%}   & 89.8\% & 0.0\%  & \textbf{96.5\%}  & 89.1\% & 0.0\%  \\
    SAN-NR  & \makecell[c]{98\%}  & 89.8\% & 0.0\% & 95.5\% &90.1\%  &0.0\%  \\
    DT1~\cite{hao2020biologically}     &  96.5\%   & 91.2\% & 0.0\% & \makecell[c]{95\%} &90.5\%  &  0.0\% \\
    DT2~\cite{kim2021spiking}     & \makecell[c]{97\%}  & 90.7\% & 0.0\%  & \makecell[c]{95\%}  &90.5\% & 0.0\%\\
    % DT3~\cite{sengupta2019going}   & 49.93    & 19.27   & 63.5\%  & 51.35 & 19.23 & 52.5\%  \\
    \hline
    DET only   & \makecell[c]{96\%} & 91.7\% & 0.0\%  & 95.5\% & 90.1\% & 0.0\% \\
    DTT only   & \makecell[c]{97\%}& 90.7\% & 0.0\%  & 95.5\%  & 90.1\% &0.0\% \\
    \hline
    \DTname\   & \textbf{98.5\%} & 89.3\% & 0.0\% & \textbf{96.5\%} & 89.1\% &  0.0\% \\
    \bottomrule
  \end{tabular}

  \end{table}

\begin{table}
% \begin{minipage}{1.0\linewidth}
\caption{Quantitative performance of obstacle avoidance with dynamic obstacles (DO).}
  \vspace{0.2cm}
  \label{SMtab:Degraded environment}
  \centering

  \setlength\tabcolsep{5pt}
  \begin{tabular}{lllllll}
    \toprule
     
     & \multicolumn{3}{c}{\textbf{LIF ($T=5$)}}     & \multicolumn{3}{c}{\textbf{SRM ($T=5$)}}                \\
    \cmidrule(r){2-4}
    \cmidrule(r){5-7}
     \textbf{Name}  & \makecell[c]{SR$\uparrow$}    &  \makecell[c]{CRP}       & \makecell[c]{OTP}        & \makecell[c]{SR$\uparrow$}    &  \makecell[c]{CRP}       & \makecell[c]{OTP} \\
    \hline
    SAN  & 81.5\%     & 43.6\%   & 0.0\% & 78.5\% & 31.8\% & 0.0\%   \\
    SAN-NR  & 83.5\%    & 42.5\%   & 0.0\% & 77.5\% &32.3\% & 0.5\%  \\

    DT1~\cite{hao2020biologically}   & 74.5\%    & 47.7\%   & 0.0\%   & 68.5\%   &  36.5\% & 0.0\% \\
    DT2~\cite{kim2021spiking}  &  \makecell[c]{80\%}  & 44.4\% & 0.0\%  &  71.5\%  & 35.0\% & 0.5\% \\
    % DT3~\cite{sengupta2019going}   & 49.93    & 19.27   & 63.5\%  & 51.35 & 19.23 & 52.5\%  \\
    \hline
    DET only  & \makecell[c]{81\%}    &43.8\%    & 0.0\% & 78.5\%  & 31.8\% & 0.5\%\\
    DTT only  & \makecell[c]{88\%}    & 40.3\%   & 0.0\% & 83.5\% & 29.9\% &  0.0\%\\
    \hline
    \DTname\   & \textbf{92.5\%}    & 38.4\%   &  0.0\%   & \textbf{90.5\%} & 27.6\% &  0.0\%  \\
    \bottomrule
  \end{tabular}
  \vspace{0.3cm}
\end{table}

\begin{table}

%   \caption{Degraded environment of different methods on different SNN models}
%   \vspace{-0.2cm}
%   \label{tab:Degraded environment}
%   \centering
%   \scriptsize
%   \setlength\tabcolsep{2pt}
%   \begin{tabular}{lllllll}
%     \toprule
     
%      & \multicolumn{3}{c}{\textbf{LIF}}     & \multicolumn{3}{c}{\textbf{SRM}}                \\
%     \cmidrule(r){2-4}
%     \cmidrule(r){5-7}
%      \textbf{Name}  & \makecell[c]{SR$\uparrow$}    &  \makecell[c]{AD(m)$\downarrow$}       & \makecell[c]{AS(m/s)$\uparrow$}        & \makecell[c]{SR$\uparrow$}    &  \makecell[c]{AD(m)$\downarrow$}       & \makecell[c]{AS(m/s)$\uparrow$} \\
%     \hline
%     SAN  & 81.5\%     & 18.01   & 0.436 & 78.5\% & 18.62& 0.429   \\
%     SAN-NR  & 83.5\%    & 18.21   & 0.427 & 77.5\% &18.21 & 0.398  \\

%     DT1~\cite{hao2020biologically}   & 74.5\%    & 18.27   & 0.420   & 68.5\%   &   18.41 & 0.422 \\
%     DT2~\cite{kim2021spiking}  &  \makecell[c]{80\%}  & 18.62 & 0.438  &  71.5\%  & 18.50 & 0.412 \\
%     % DT3~\cite{sengupta2019going}   & 49.93    & 19.27   & 63.5\%  & 51.35 & 19.23 & 52.5\%  \\
%     \hline
%     DET only  & \makecell[c]{81\%}    &18.71    & 0.412  & 78.5\%  & 18.54 & 0.409\\
%     DTT only  & \makecell[c]{88\%}    & 17.53   & 0.433 & 83.5\% & 18.81 &  0.418\\
%     \hline
%     \DTname\   & \textbf{92.5\%}    & 17.55   &  0.420    & \textbf{90.5\%} & 18.26 &  0.409  \\
%     \bottomrule
%   \end{tabular}
%   \vspace{0.1cm}
    \caption{Quantitative performance of obstacle avoidance with degraded inputs (DI).}
  \label{SMtab:Degraded inputs}
  \centering
%   \scriptsize
  \setlength\tabcolsep{5pt}
  \begin{tabular}{llllllll}
    \toprule
     
     & & \multicolumn{3}{c}{\textbf{LIF ($T=5$)}}     & \multicolumn{3}{c}{\textbf{SRM ($T=5$)}}                \\
    \cmidrule(r){3-5}
    \cmidrule(r){6-8}
     \textbf{\tiny{Noise}} & \textbf{Name}  & \makecell[c]{SR$\uparrow$}    &  \makecell[c]{CRP}       & \makecell[c]{OTP}        & \makecell[c]{SR$\uparrow$}    &  \makecell[c]{CRP}       & \makecell[c]{OTP}\\
    \hline
    \multirow{7}{*}{\makecell[c]{0.2}}
    & SAN  & 78.5\%    & 42.0\%   & 1.5\% & \makecell[c]{68\%} & 30.1\% & 1.0\%   \\
    & SAN-NR  & \makecell[c]{80\%} & 41.3\% & 2.5\%  & \makecell[c]{59\%} & 34.7\% & 3.0\%  \\
    % & DT1~\cite{hao2020biologically}     & 71.5\%    & 18.74   & 0.312 & \makecell[c]{35\%} & 25.58 &  0.378  \\
   
    & DT1~\cite{hao2020biologically}   & 65.5\%    & 50.4\%   & 4.0\%  &  \makecell[c]{64\%}   &   32.0\%  & 3.5\%\\
    & DT2~\cite{kim2021spiking} & \makecell[c]{78\%}  & 42.3\%  & 3.0\% & 53.5\%   & 38.3\% &  3.5\% \\
    % & DT3~\cite{sengupta2019going}   & 66.33    & 19.57   & 64.5\% & 71.89 & 20.12 & 44.5\% \\
    \cline{2-8}
    & DET only  & \makecell[c]{83\%}   & 39.8\%   & 2.0\% & 71.5\% & 28.7\% & 3.0\%\\
    & DTT only  & 78.5\%    & 42.0\%   & 3.5\% & 64.5\% & 31.8\% & 1.0\% \\
    \cline{2-8}
    & \DTname\   & \textbf{\makecell[c]{90\%}}   &  36.7\%  & 2.5\% & \textbf{79.5\%} & 25.8\% & 3.5\%  \\
    \hline
    \multirow{7}{*}{\makecell[c]{6.0}}
    & SAN  & \makecell[c]{71\%}   & 43.7\%   & 0.0\% & \makecell[c]{70\%} & 32.9\% &  0.0\%   \\
    & SAN-NR  & \makecell[c]{70\%} & 44.3\% & 0.0\%  &  61.5\% &37.4\% & 0.0\% \\
    % & DT1~\cite{hao2020biologically}     & 73.5\%    & 17.82   & 0.421 & 59.5\% & 18.89 &  0.421  \\
   
    & DT1~\cite{hao2020biologically}     & \makecell[c]{62\%}    & 50.0\%   & 0.0\% & \makecell[c]{67\%}  &  34.3\%  & 0.0\% \\
    & DT2~\cite{kim2021spiking}  & 61.5\%    & 50.4\%   & 0.0\%   &  \makecell[c]{55\%}   & 41.8\% & 0.5\%\\
    % & DT3~\cite{sengupta2019going}   & 43.57    & 18.03   & \makecell[c]{51\%} & 44.42 & 19.32 & 49.5\% \\
    \cline{2-8}
    & DET only  & \makecell[c]{80\%}    & 38.8\%   & 0.0\% & \makecell[c]{79\%} & 29.1\% & 0.0\% \\
    & DTT only  & \makecell[c]{80\%}   & 38.8\%    & 0.0\% & 75.5\% & 30.5\% & 0.0\% \\
    \cline{2-8}
    & \DTname\   & \textbf{\makecell[c]{84.5\%}}   &  36.7\%  & 0.0\%  & \textbf{\makecell[c]{83\%}} & 27.7\% &  0.0\% \\
    
    \hline
    \multirow{7}{*}{\makecell[c]{GN}}
    
    & SAN & 71.5\%  & 38.5\%  & 0.0\% & \makecell[c]{57\%}  & 30.7\% & 0.0\%   \\
    & SAN-NR  & \makecell[c]{72\%} & 38.2\% & 0.0\%  &  65.5\% &26.7\% & 1.0\%\\
    % & DT1~\cite{hao2020biologically}     & 68.5\%    & 18.87   & 0.387 & \makecell[c]{70\%} & \textbf{18.03} &  0.392  \\
    
    & DT1~\cite{hao2020biologically}    & 60.5\%    & 45.5\%   & 0.5\% &  \makecell[c]{58\%}  &   30.2\% &  0.0\%   \\
    & DT2~\cite{kim2021spiking}  &   71.5\%  & 38.5\%  &  1.5\% &   61.5\%  & 28.5\%  &  0.0\% \\
    % & DT3~\cite{sengupta2019going}   & 48.93    & 19.84   & 53.5\% & 47.98 & 18.81 & \makecell[c]{47\%} \\
    \cline{2-8}
    & DET only  & 78.5\%    & 35.0\%   & 1.0\% & 75.5\% & 23.2\% & 0.5\% \\
    & DTT only   & 75.5\%   & 36.4\%  & 0.0\% & \makecell[c]{69\%} & 25.4\% & 0.0\%\\
    \cline{2-8}
    & \DTname\   & \textbf{\makecell[c]{84.5\%}}    & 32.5\%   & 0.0\%  & \textbf{82.5\%} & 21.2\% & 0.0\%  \\

    \bottomrule
    
  \end{tabular}
  \end{table}
  
  \begin{table}
%   \vspace{0.3cm}
      \caption{Quantitative performance of obstacle avoidance with weight uncertainty (WU)}
    %   \vspace{-0.2cm}
  \label{SMtab:Weight pollution}
  \centering
%   \scriptsize
  \setlength\tabcolsep{5pt}
  \begin{tabular}{llllllll}
    \toprule
     
     & & \multicolumn{3}{c}{\textbf{LIF ($T=5$)}}     & \multicolumn{3}{c}{\textbf{SRM ($T=5$)}}                \\
    \cmidrule(r){3-5}
    \cmidrule(r){6-8}
     \textbf{Type} & \textbf{Name}  & \makecell[c]{SR$\uparrow$}    &  \makecell[c]{CRP}       & \makecell[c]{OTP}        & \makecell[c]{SR$\uparrow$}    &  \makecell[c]{CRP}       & \makecell[c]{OTP}\\

     \hline
    \multirow{7}{*}{\makecell[c]{8-bit \\ Loihi \\ weight}}
    & SAN  & \makecell[c]{78.5\%}    & 43.3\%  & 0.0\%  & \makecell[c]{77\%} &30.5\% & 0.0\%   \\
    & SAN-NR  & 79.5\%    &  42.8\%  & 0.0\%  & 76.5\%   & 30.7\%   &  0.5\%  \\
    % & DT1~\cite{hao2020biologically}     & 34.5\%    & 20.33   & 0.401 & 30.2\% & 19.93 &  0.422  \\
    % & DT2~\cite{kim2021spiking}     & 55.6\%    & 18.91   & 0.431 & 45.2\% & 20.09 & 0.430 \\
    & DT1~\cite{hao2020biologically}  & \makecell[c]{70\%}  &  48.6\%  & 0.0\%  & \makecell[c]{67\%}  & 35.1\%  & 0.0\% \\
    & DT2~\cite{kim2021spiking}  & \makecell[c]{78.5\%}   & 43.3\%   & 0.0\%  & 67.5\%    & 34.8\%   & 1.0\% \\
    % & DT3~\cite{sengupta2019going}   & 63.12    & 20.10   & 21.5\% & 50.75 & 21.31 & 24.1\% \\
    \cline{2-8}
    & DET only  & 77.5\%   &  43.9\%  & 0.0\% & \makecell[c]{75\%}  & 31.3\%    & 0.0\% \\
    & DTT only  &  86\%    & 39.5\%   & 0.0\% & 80.5\% & 29.2\%  & 0.0\% \\
    \cline{2-8}
    & \DTname\   & \makecell[c]{\textbf{90\%}}   &  37.8\%  & 0.0\% & \textbf{88.5\%} & 26.6\% & 0.0\%  \\
    
    \hline
    
    \multirow{7}{*}{\makecell[c]{GN \\ weight \\ (5 rounds)}}
    & SAN  & \makecell[c]{51.3\%} & 28.7\% & 1.2\% &  \makecell[c]{0\%} & \makecell[c]{-} & \makecell[c]{20.3\%}   \\
    & SAN-NR  & \makecell[c]{52.5\%}    & 28.0\%   & 1.6\%  & 37.2\% & 30.6\% & 2.4\%   \\
    & DT1~\cite{hao2020biologically}     & 54.6\%     & 26.9\%   & 2.3\% & \makecell[c]{44.9\%} & 25.4\% &  3.0\%  \\
    & DT2~\cite{kim2021spiking}     & 73.2\%    & 20.1\%  & 2.1\% & 43.6\% & 26.1\% & 2.4\% \\
    % & DT3~\cite{sengupta2019going}   & 47.89    & 19.04   & 33.0\% & 53.67 & 22.44 & 28.2\% \\
    \cline{2-8}
    & DET only  & 61.8\%    & 23.8\%  & 1.8\% & 43.3\% & 26.3\% & 2.5\% \\
    & DTT only  & 77.1\%   & 19.1\%   & 1.5\% & \makecell[c]{46.4\%} & 24.6\% & 1.6\%\\
    \cline{2-8}
    & \DTname\   & \textbf{\makecell[c]{87.7\%}}   &  16.8\%  &  0.8\% & \textbf{61.8\%} & 18.4\% &  1.3\% \\
    
    \hline
    \multirow{7}{*}{\makecell[c]{ $30\%$ \\ Zero \\ weight  \\ (5 rounds)}}
    & SAN  & \makecell[c]{59.3\%}    & 32.4\%  & 0.0\% & \makecell[c]{0\%} &\makecell[c]{-} & 17.7\%   \\
    & SAN-NR  & 61.6\%    & 31.2\%   &0.0\% & 46.5\%    & 21.1\%   & 0.0\%    \\
    % & DT1~\cite{hao2020biologically}     & 34.5\%    & 20.33   & 0.401 & 30.2\% & 19.93 &  0.422  \\
    % & DT2~\cite{kim2021spiking}     & 55.6\%    & 18.91   & 0.431 & 45.2\% & 20.09 & 0.430 \\
    & DT1~\cite{hao2020biologically}  & \makecell[c]{41.2\%}    & 46.6\%   & 0.7\%  & 44.3\%  &  22.1\% & 0.0\% \\
    & DT2~\cite{kim2021spiking}  & 55.6\%    & 34.5\%   & 0.3\% &   49.1\%  & 20.0\%  &  0.8\%\\
    % & DT3~\cite{sengupta2019going}   & 63.12    & 20.10   & 21.5\% & 50.75 & 21.31 & 24.1\% \\
    \cline{2-8}
    & DET only  & 46.2\%    & 41.6\%   & 0.0\% & 39.8\% & 24.6\% & 1.4\%\\
    & DTT only  &  60.6\%    & 31.7\%   & 0.0\% & 45.4\% & 21.6\% & 0.5\%\\
    \cline{2-8}
    & \DTname\   & \textbf{77.2\%}   &  24.9\%  & 0.0\% &\textbf{65.2\%} & 15.1\% & 0.3\%  \\

    \bottomrule

  \end{tabular}

% \end{minipage}
\end{table}

\newpage

\noindent
\bd{
As discussed in the main paper, each robot state is encoded into 24 Poisson spike trains, and each spike train has $T$ timesteps. Due to the limited space, we only report the experimental results based on $T=5$ in the main paper. Here, we show the quantitative performance with $T=25$. Our approach still offers the best SRs across all experimental settings. Specifically, in the dynamic obstacle experiments (Table~\ref{SMtab:Degraded environment T=25}), our approach outperforms the runner-ups by a significant marge, 9.5\% with LIF and 12.5\% with SRM; As shown in Table~\ref{SMtab:Degraded inputs T=25}, the proposed \DTname\ improves the SRs of both LIF-based and SRM-based baseline model (i.e., SAN-NR) by at least 11.5\% and 18\%, respectively; Under the three weight uncertainty conditions (see Table~\ref{SMtab:Weight pollution T=25}), the proposed \DTname\ increases the SRs of the baseline model SAN-NR by at least 9.5\%, 14.2\%, and 14.8\%, respectively.
}

% \djc{As shown in Table~\ref{SMtab:Degraded environment T=25}, our approach delivers the best SRs with both LIF and SRM neuron models in T=25 test. Notably, it outperforms the runner-ups by a significant marge, 9.5\% with LIF and 12.5\% with SRM. The results evidence that the proposed bio-plausible DT scheme provides substantial environment adaptiveness to the host SNNs.}

% \djc{ The results of T=25 degraded inputs tests are shown in Table~\ref{SMtab:Degraded inputs T=25}. In all experiments, the SRs obtained from our \DTname\ scheme still maintain the highest and outperform the runner-ups by at least 11.5\%. It reflects the proposed DT scheme provides the host SNNs with strong adaptiveness to all designed degraded inputs, which is highly desired and appreciated in mobile robot applications. 
% Remarkably, under all degraded inputs experiments, the proposed \DTname\ improves the SRs of both LIF-based and SRM-based baseline model (i.e., SAN-NR) by at least 11.5\% and 18\%, respectively.
% }

% \djc{Again, under the three weight uncertainty conditions (see Table~\ref{SMtab:Weight pollution T=25}), the proposed \DTname\ increases the SRs of the baseline model SAN-NR by at least 9.5\%, 14.2\%, and 14.8\%, respectively.}

\noindent
\bd{
Based on Table~\ref{SMtab:Sta_test} and Table~\ref{SMtab:Sta_test T=25}, compared to the SRs obtained with $T=5$ settings, $T=25$ settings only change the SRs slightly (\ie $\pm 0.5\%$), indicating that all competing SNNs are not sensitive to the $T$ value in static obstacle avoidance tasks. The observations also hold in the dynamic obstacle experiments with the two different $T$ value (Table~\ref{SMtab:Degraded environment} vs Table~\ref{SMtab:Degraded environment T=25}). However, We observe the SRs increases with larger $T$ value in the most degraded inputs and weight uncertainty experiments, especially in `GN weight' and `30\% zero weight' settings. 
}

% \tb{T=25} Table~\ref{SMtab:Sta_test T=25}, Table~\ref{SMtab:Degraded environment T=25} T=25 Interference experiments.

\begin{table}
\caption{Quantitative performance of obstacle avoidance with static obstacles ($T=25$).}

  \label{SMtab:Sta_test T=25}
  \centering
  
  \setlength\tabcolsep{5pt}
  
  \begin{tabular}{lllllll}
    \toprule
     
     & \multicolumn{3}{c}{\textbf{LIF ($T=25$)}}     & \multicolumn{3}{c}{\textbf{SRM ($T=25$)}}                \\
    \cmidrule(r){2-4}
    \cmidrule(r){5-7}
    \textbf{Name}  & \makecell[c]{SR$\uparrow$}    &  \makecell[c]{CRP}       & \makecell[c]{OTP}        & \makecell[c]{SR$\uparrow$}    &  \makecell[c]{CRP}       & \makecell[c]{OTP} \\
    \hline
    SAN  & \makecell[c]{98\%} & 91.3\%  &   0.0\%  & 96\%  &  88.5\% &    0.0\%  \\
    SAN-NR  & \textbf{98.5\%} & 90.9\%  &   0.0\%   & 95.5\% &  89.0\% &  0.0\%   \\
    DT1~\cite{hao2020biologically}     & \makecell[c]{96\%} & 93.2\%  &   0.0\%   & 94.5\%  & 89.9\%  &    0.5\%  \\
    DT2~\cite{kim2021spiking}     & \makecell[c]{97\%} & 92.3\% &  0.0\% &  94\% &  90.4\% &  0.0\%   \\
    % DT3~\cite{sengupta2019going}   & 49.93    & 19.27   & 63.5\%  & 51.35 & 19.23 & 52.5\%  \\
    \hline
    DET only  & 95.5\%& 93.7\%  &   0.0\%   & 95\% & 89.5\%  &  0.0\%   \\
    DTT only   & 97\% &  92.3\% &   0.0\%   &95\% & 89.5\%  &   0.0\%  \\
    \hline
    \DTname\   & 98\% & 91.3\%  &   0.0\%   & \textbf{97\%}&  87.6\% &   0.0\%  \\
    \bottomrule
  \end{tabular}
\end{table}

\begin{table}
% \begin{minipage}{1.0\linewidth}
\caption{Quantitative performance of obstacle avoidance with dynamic obstacles ($T=25$).}
  \vspace{0.2cm}
  \label{SMtab:Degraded environment T=25}
  \centering
%   \small
  \setlength\tabcolsep{5pt}
  \begin{tabular}{lllllll}
    \toprule
     
     & \multicolumn{3}{c}{\textbf{LIF ($T=25$)}}     & \multicolumn{3}{c}{\textbf{SRM ($T=25$)}}                \\
    \cmidrule(r){2-4}
    \cmidrule(r){5-7}
     \textbf{Name}  & \makecell[c]{SR$\uparrow$}    &  \makecell[c]{CRP}       & \makecell[c]{OTP}        & \makecell[c]{SR$\uparrow$}    &  \makecell[c]{CRP}       & \makecell[c]{OTP} \\
    \hline
    SAN  & 81\% & 42.0\% & 0.0\% & 77.5\% & 33.5\% & 0.0\%  \\
    SAN-NR  & 83.5\%& 40.7\%  & 0.0\%  & 77\% & 33.8\% & 1.0\% \\

    DT1~\cite{hao2020biologically}   &74\% & 45.9\% & 0.5\% & 68.5\%& 38.0\% & 0.5\% \\
    DT2~\cite{kim2021spiking}  &  80\%   & 42.5\% & 0.0\%  &  71.5\%& 36.4\% &0.0\% \\
    % DT3~\cite{sengupta2019going}   & 49.93    & 19.27   & 63.5\%  & 51.35 & 19.23 & 52.5\%  \\
    \hline
    DET only  & 80.5\%  & 42.2\%  &0.0\%   &   78.5\%& 33.1\% & 1.0\% \\
    DTT only  & 86.5\%  & 39.3\%  & 0.0\%  &   82\%& 31.7\% & 0.0\% \\
    \hline 
    \DTname\   &  \textbf{93\%}  & 36.6\%  & 0.0\%  &  \textbf{89.5\%} & 29.1\% &  0.5\% \\
    \bottomrule
  \end{tabular}
  \end{table}

\begin{table}

    \caption{Quantitative performance of obstacle avoidance with degraded inputs ($T=25$)}
  \label{SMtab:Degraded inputs T=25}
  \centering
%   \scriptsize
  \setlength\tabcolsep{5pt}
  \begin{tabular}{llllllll}
    \toprule
     
     & & \multicolumn{3}{c}{\textbf{LIF ($T=25$)}}     & \multicolumn{3}{c}{\textbf{SRM ($T=25$)}}                \\
    \cmidrule(r){3-5}
    \cmidrule(r){6-8}
     \textbf{\tiny{Noise}} & \textbf{Name}  & \makecell[c]{SR$\uparrow$}    &  \makecell[c]{CRP}       & \makecell[c]{OTP}        & \makecell[c]{SR$\uparrow$}    &  \makecell[c]{CRP}       & \makecell[c]{OTP}\\
    \hline
    \multirow{7}{*}{\makecell[c]{0.2}}
    & SAN  &  74\%  &41.9\%  &2.5\% &  60.5\%  & 24.8\% & 1.0\% \\
    & SAN-NR  &76\%  &40.8\%  &3.0\%  & 39.5\% & 38.0\% & 4.5\% \\
    % & DT1~\cite{hao2020biologically}     & 71.5\%    & 18.74   & 0.312 & \makecell[c]{35\%} & 25.58 &  0.378  \\
   
    & DT1~\cite{hao2020biologically}  & 60.5\% &51.2\% &3.5\% & 58.5\% &25.6\%   &  5.0\% \\
    & DT2~\cite{kim2021spiking} & 72.5\% &42.8\% &4.0\% & 49\%  &30.6\%  & 3.5\% \\
    % & DT3~\cite{sengupta2019going}   & 66.33    & 19.57   & 64.5\% & 71.89 & 20.12 & 44.5\% \\
    \cline{2-8}
    & DET only & 77.5\% &40.0\% &3.5\% & 67.5\%  &  22.2\% &   3.0\%\\
    & DTT only & 72.5\% & 42.8\% &3.5\% &  62\% & 24.2\%  &  2.5\%   \\
    \cline{2-8}
    & \DTname\   & \textbf{87.5\%}   &35.4\%  &3.5\%  &\textbf{76\%}  & 19.7\%  &  4.5\%  \\
    \hline
    \multirow{7}{*}{\makecell[c]{6.0}}
    & SAN  &  73\% & 43.2\% & 0.0\% &  72\%  &34.7\% & 0.0\%\\
    & SAN-NR  &71\%  &44.4\%  & 0.0\% & 65.5\%  & 38.2\% & 0.0\%  \\
    % & DT1~\cite{hao2020biologically}     & 73.5\%    & 17.82   & 0.421 & 59.5\% & 18.89 &  0.421  \\
   
    & DT1~\cite{hao2020biologically} & 64\% & 49.2\% &0.0\%  & 66.5\%  & 37.6\% &  0.0\%    \\
    & DT2~\cite{kim2021spiking} & 61.5\%  & 51.2\%  &0.0\%  & 57.5\%  & 43.5\% &  0.0\% \\
    % & DT3~\cite{sengupta2019going}   & 43.57    & 18.03   & \makecell[c]{51\%} & 44.42 & 19.32 & 49.5\% \\
    \cline{2-8}
    & DET only &79.5\%   & 39.6\% &0.0\%  & 79.5\%  & 31.4\% & 0.0\% \\
    & DTT only  &81\%  & 38.9\% & 0.0\% & 76\%  & 32.9\% &  0.0\% \\
    \cline{2-8}
    & \DTname\   & \textbf{86\%} &  36.6\% & 0.0\% & \textbf{83.5\%}  & 29.9\% &  0.0\%\\
    
    \hline
    \multirow{7}{*}{\makecell[c]{GN}}
    
    & SAN  & 63\% & 37.3\%   &  0.0\%  & 51.5\%  & 32.0\%  &  0.5\% \\
    & SAN-NR & 67\% &35.1\%  & 0.5\% & 54.5\% & 30.3\%  &  2.0\%\\
    % & DT1~\cite{hao2020biologically}     & 68.5\%    & 18.87   & 0.387 & \makecell[c]{70\%} & \textbf{18.03} &  0.392  \\
    
    & DT1~\cite{hao2020biologically} & 56.5\%  &41.6\%   & 0.5\%  & 55.5\%  & 29.7\% &    0.0\% \\
    & DT2~\cite{kim2021spiking}  & 68\%  & 34.6\%   &  1.0\% & 57\%  & 28.9\% & 1.5\% \\
    % & DT3~\cite{sengupta2019going}   & 48.93    & 19.84   & 53.5\% & 47.98 & 18.81 & \makecell[c]{47\%} \\
    \cline{2-8}
    & DET only & 76\%  & 30.9\%   & 2.0\%  & 71\%  & 23.2\% & 0.5\% \\
    & DTT only  & 70.5\%   & 33.3\%   & 0.0\%  &  66.5\% & 24.8\% & 0.5\% \\
    \cline{2-8}
    & \DTname\  & \textbf{81.5\%} & 28.8\%   & 0.0\%   & \textbf{79\%}  & 20.9\%  & 0.5\% \\

    \bottomrule
  \end{tabular}
  
    \end{table}
    
\begin{table}

      \caption{Quantitative  performance  of  obstacleavoidance with weight uncertainty ($T=25$)}
  \label{SMtab:Weight pollution T=25}
  \centering
%   \scriptsize
  \setlength\tabcolsep{5pt}
  \begin{tabular}{llllllll}
    \toprule
     
     & & \multicolumn{3}{c}{\textbf{LIF ($T=25$)}}     & \multicolumn{3}{c}{\textbf{SRM ($T=25$)}}                \\
    \cmidrule(r){3-5}
    \cmidrule(r){6-8}
     \textbf{Type} & \textbf{Name}  & \makecell[c]{SR$\uparrow$}    &  \makecell[c]{CRP}       & \makecell[c]{OTP}        & \makecell[c]{SR$\uparrow$}    &  \makecell[c]{CRP}       & \makecell[c]{OTP}\\
    \hline
    \multirow{7}{*}{\makecell[c]{8-bit \\ Loihi \\ weight}}
    & SAN  & 77.5\%   & 39.4\% & 0.0\%  & 74.5\% & 29.5\%  & 0.0\% \\
    & SAN-NR  & 79\% & 38.6\% & 0.0\%  & 75.5\%  & 29.1\%  & 0.0\% \\
    % & DT1~\cite{hao2020biologically}     & 71.5\%    & 18.74   & 0.312 & \makecell[c]{35\%} & 25.58 &  0.378  \\
   
    & DT1~\cite{hao2020biologically} & 67.5\% &45.2\% & 0.5\%  & 65.5\%  &33.6\%  &  0.0\%\\
    & DT2~\cite{kim2021spiking} & 77\% &39.6\% & 0.0\% & 67\% & 32.8\% &0.5\%  \\
    % & DT3~\cite{sengupta2019going}   & 66.33    & 19.57   & 64.5\% & 71.89 & 20.12 & 44.5\% \\
    \cline{2-8}
    & DET only & 74.5\% & 40.9\% & 0.5\%  & 75\%  & 29.3\% &  0.0\%  \\
    & DTT only & 81.5\% & 37.4\%  &  0.0\%  & 80\%  &  27.5\% &  0.0\%  \\
    \cline{2-8}
    & \DTname\   & \textbf{88.5\%} &34.5\% & 0.0\%   & \textbf{87.5\%} & 25.1\% & 0.0\%   \\
    \hline
    \multirow{7}{*}{\makecell[c]{GN \\ weight \\ (5 rounds)}}
    & SAN  & 36.2\% & 28.5\% & 3.6\%   & 0\%  & -  & 18.4\%  \\
    & SAN-NR  & 39.0\% & 26.4\% & 3.1\%  & 38.4\%  & 21.9\% & 2.1\%  \\
    % & DT1~\cite{hao2020biologically}     & 73.5\%    & 17.82   & 0.421 & 59.5\% & 18.89 &  0.421  \\
   
    & DT1~\cite{hao2020biologically}  & 35.7\% & 28.9\%  & 3.3\%  & 32.4\% & 25.9\%  & 4.7\%  \\
    & DT2~\cite{kim2021spiking}  & 56.2\% &  18.3\% &  2.0\%  & 30.3\% & 27.7\%  &  2.9\%  \\
    % & DT3~\cite{sengupta2019going}   & 43.57    & 18.03   & \makecell[c]{51\%} & 44.42 & 19.32 & 49.5\% \\
    \cline{2-8}
    & DET only   & 47.0\% & 21.9\%  & 2.3\%  & 34.1\% &  24.6\% &2.6\%\\
    & DTT only   & 64.7\% & 15.9\%  & 1.8\%  & 36.8\% &  22.8\% & 1.4\% \\
    \cline{2-8}
    & \DTname\   &  \textbf{70.1\%}   & 14.7\%  &  0.4\%   & \textbf{52.6\%}  & 16.0\%  & 2.5\%   \\
    
    \hline
    \multirow{7}{*}{\makecell[c]{$30\%$ \\ Zero \\ weight \\ (5 rounds)}}
    
    & SAN  & 51.2\% & 29.7\%  & 0.0\%  & 0\% & -  &  19.4\%   \\
    & SAN-NR & 53.6\% & 28.4\% & 0.0\% & 36.5\% & 21.6\% & 0.2\%  \\
    % & DT1~\cite{hao2020biologically}     & 68.5\%    & 18.87   & 0.387 & \makecell[c]{70\%} & \textbf{18.03} &  0.392  \\
    
    & DT1~\cite{hao2020biologically}    & 32.2\% & 47.2\% & 1.3\% & 31.7\% &24.9\%  & 0.6\%   \\
    & DT2~\cite{kim2021spiking}  & 48.0\% & 31.7\% & 0.0\%  & 37.8\% & 20.9\% & 1.1\%  \\
    % & DT3~\cite{sengupta2019going}   & 48.93    & 19.84   & 53.5\% & 47.98 & 18.81 & \makecell[c]{47\%} \\
    \cline{2-8}
    & DET only  &33.6\%  & 45.2\% & 0.8\% & 29.3\%  & 27.0\% & 2.5\% \\
    & DTT only   & 50.3\% & 30.2\% & 0.4\% & 38.8\% & 20.4\% & 1.3\% \\
    \cline{2-8}
    & \DTname\  &\textbf{68.4\%}  & 22.2\% & 0.0\% & \textbf{56.5\%} & 14.0\% & 0.7\%  \\

    \bottomrule
  \end{tabular}

\end{table}

% \tb{$\eta$ test} Table~\ref{SMtab:eta}
% \begin{table}
% \caption{Quantitative performance in dynamic obstacles scenes with different $\eta$.}
%   \vspace{0.2cm}
%   \label{SMtab:eta}
%   \centering
%   \small
%   \setlength\tabcolsep{2pt}
%   \begin{tabular}{lllllll}
%     \toprule
     
%      & \multicolumn{3}{c}{\textbf{LIF}}     & \multicolumn{3}{c}{\textbf{SRM}}                \\
%     \cmidrule(r){2-4}
%     \cmidrule(r){5-7}
%      \textbf{$\eta$}  & \makecell[c]{SR$\uparrow$}    &  \makecell[c]{AD(m)$\downarrow$}       & \makecell[c]{AS(m/s)$\uparrow$}        & \makecell[c]{SR$\uparrow$}    &  \makecell[c]{AD(m)$\downarrow$}       & \makecell[c]{AS(m/s)$\uparrow$} \\
%     \hline
%      0.01 & 92.5\% & & & 90.5\%   \\
%      0.05 & 89.5\%  & & & 86.5\% \\

%      0.50  & 87.5\% & & & 79\%\\
%      -0.01 & 91\% &  & &89\% \\
%      -0.50 & 0\%  &  & & 0\% \\
%     \bottomrule
%   \end{tabular}
% \end{table}
