# Supplementary material for: Biologically Inspired Dynamic Thresholds for Spiking Neural Networks
Source: arXiv:2206.04426 source file (2023-06-19)
Supplement: Supplementary file 6 [file OA_experiment_results.tex]

\subsection*{Experimental Setup}
In the obstacle avoidance experiments, our evaluation baseline model and test environment are modified variants of the spiking actor network (SAN)~\cite{tang2020reinforcement} and its original simulated test environment, respectively. The SAN is a part of the spiking deep deterministic policy gradient (SDDPG) framework~\cite{tang2020reinforcement}, which is a fully connected four-layer SNN (\ie three 256-neuron hidden layers and one two-neuron output layer). This network maps a state $s$ of a robot to a control action $a$.
Specifically, a state $s = \{G_{dis}, G_{dir}, \nu, \omega, L\}$ is encoded into $24$ Poisson spike trains as inputs of the SAN, and each spike train has $T$ timesteps. $G_{dis}$ and $G_{dir}$ are the relative $1$-D distances from the robot to the goal and a $2$-D direction (\ie right and left directions), respectively; $\nu$ and $\omega$ are the robot's $1$-D linear and $2$-D angular velocities (\ie rightward and leftward angular velocities); $L$ denotes the distance measurements obtained from a Robo Peak light detection and ranging (RPLIDAR) laser range scanner (range: {0.2-40 m}), which has a field of view of $180$ degrees with $18$ range measurements, each with a $10$-degree resolution. The two output spike trains are decoded to control the robot via an action $a = \{\nu_L, \nu_R\}$, where $\nu_L$ and $\nu_R$ are the left and right wheel speeds of the differential-drive mobile robot, respectively~\cite{tang2020reinforcement}. 

\begin{figure}[h]
	\centering

	\includegraphics [scale=0.5]{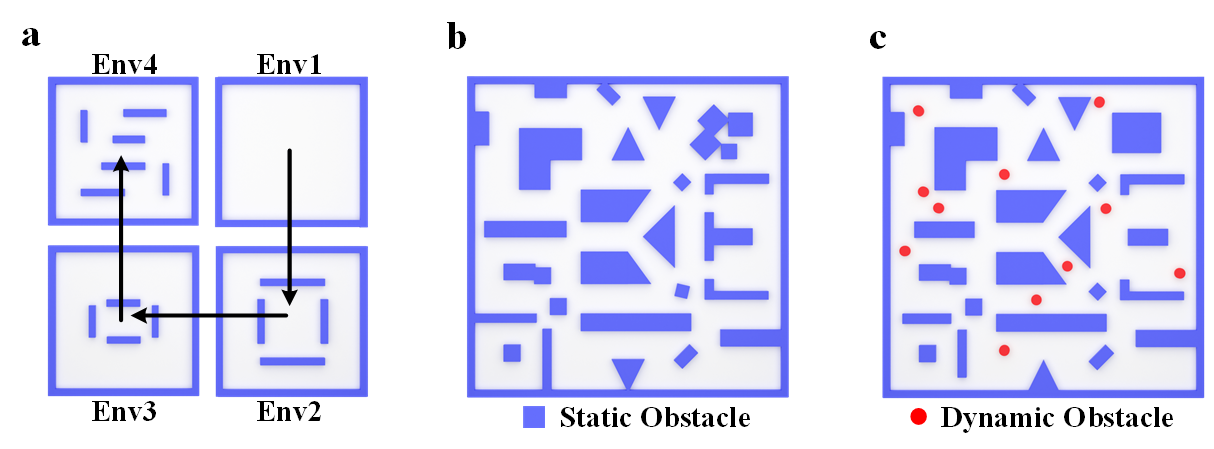}
	\vspace{-0.2cm}
% 	\begin{flushleft}
% 	    \textbf{Fig. S2. Illustrations of the training, static testing and dynamic testing environments.} a. The training environments of the obstacle avoidance tasks. The training processes of all competing SNNs start from Env1 and end with Env4. b. Static testing environment. c. Dynamic testing environment. In addition to static obstacles, $11$ dynamic obstacles are inserted. 
% 	\end{flushleft}
	\caption{
	    Illustrations of the training, static testing and dynamic testing environments.
		a. The training environments of the obstacle avoidance tasks. The training processes of all competing SNNs start from Env1 and end with Env4. b. Static testing environment. c. Dynamic testing environment. In addition to static obstacles, $11$ dynamic obstacles are inserted. 
	}
	\label{SMfig:env}
	%\vspace{-0.2cm}
\end{figure}

\subsection*{Training} The SAN and its modified versions are trained with the original SDDPG framework. 
The training environments consist of four different maps, as shown in Figure~\ref{SMfig:env}a. In particular, during the training process, we set $100$, $200$, $300$, and $400$ start-goal pairs in the Env1, Env2, Env3, and Env4, respectively. The training starts from Env1 and ends with Env4. Following the training protocol described by Tang \etal\cite{tang2020reinforcement}, the hyperparameters related to training are set as follows: $D=0.75$ for the LIF; $\eta=0.01$ and $\psi=4.0$ for the dynamic energy threshold (DET); $C=3.0$ for the dynamic temporal threshold (DTT); $\tau_s=\tau_r=1.0$ for the SRM; $\text{collision reward}=-20$; $\text{goal reward}=30$; $\text{step reward}=15$; goal $l_2$ distance $\text{threshold}=0.5$ m; obstacle $l_2$ distance $\text{threshold}=0.35$ m; $\epsilon$ ranges for Env1 to Env4 of $(0.9, 0.1)$, $(0.6, 0.1)$, $(0.6, 0.1)$, and $(0.6, 0.1)$, respectively; and corresponding $\epsilon$-decays of $0.999$ for the four environments. During the training procedure, we set the batch size to $256$ and the learning rates to $0.00001$ for both the actor and critic networks. We use PyTorch~\cite{paszke2019pytorch} to train and test all competing SNNs with an i7-7700 CPU and an NVIDIA GTX 1080Ti GPU. We direct the readers to the SAN algorithm~\cite{tang2020reinforcement} for details.

% \begin{figure}
% % \vspace{-0.3cm}
% \centering
% \includegraphics [scale=0.1]{figures/test_env_.png}
% 	\vspace{-0.3cm}
% 	\caption{\tb{Obstacle avoidance testing environment.}}
% 	\label{fig:test_env}
% % 	\vspace{-0.3cm}
% \end{figure}

% \begin{figure}[h]
% 	\centering

% 	\includegraphics [scale=0.4]{figures/OA_degraded}
% 	\vspace{-0.2cm}
% 	\caption{
% 	    \tb{Illustrations of obstacle avoidance task and the specially designed degraded conditions.}
%         (a) The obstacle avoidance task environment and dynamic obstacles. (b) The control loop of the robot. The current state is converted to spike trains as input to the host SNN, and output spike trains are converted to control signals for each step. (c) The three specially designed degraded inputs, where the blue lasers are the disturbed ones. `0.2' and `6.0' mean the detection range of the three disturbed lasers are fixed to 0.2m and 6.0m, respectively; Under the `GN' setting, we add a Gaussian noise $\mathcal{N}(0, 1.0)$ to all initially detected ranges.   (d) The three specially designed weight uncertainty conditions. The `32 bit $\rightarrow$ 8 bit' means we lower all learned weights' precision from $32$ bit to $8$ bit; The `GN weight' means we add a sampled Gaussian noise $\mathcal{N}(0, 0.05)$ to all learned synaptic weights; Under the `$30\%$ zero weight' setting, $30\%$ of randomly selected synaptic weights are set to $0$.
% 	}
% 	\label{fig:OA_degraded}
% 	%\vspace{-0.2cm}
% \end{figure}

\subsection*{Assessment---Success Rate}
\label{sec:performance}
We evaluate the obstacle avoidance capabilities of the proposed method by using SR as a metric. The SR is the percentage of successful passes out of $200$ trials. A successful pass is a trial in which the robot can reach its destination without touching any static or dynamic obstacle within $1000$ steps. 
In addition to the SR, we also report the overtime percentage (OTP), the percentage of overtime trials out of the total trials (\ie $200$ trials), where overtime is defined as a trial in which the robot cannot reach the goal within $1000$ steps but does not touch any obstacle. 

\noindent
We use the Gazebo simulator to construct a $20\times20\ m^2$ static test environment (see Figure~\ref{SMfig:env}b) and adopt the randomly sampled $200$ start-goal location pairs used for testing the SAN~\cite{tang2020reinforcement}. For fairness, we apply grid searches on all tunable hyperparameters to ensure that the SRs of all competing approaches are relatively the same (\ie within $\pm 2 \%$) when testing in the static testing environment. The quantitative experimental results obtained by all competing dynamic threshold methods in the static obstacle avoidance tasks are shown in Table~\ref{SMtab:Sta_test}. Due to space limits, we only report the experimental results based on $T=5$ in the main manuscript. Here, we offer the quantitative performance with both $T=5$ and $T=25$. 

\noindent
Based on Table~\ref{SMtab:Sta_test}, compared to the SRs obtained with $T=5$, the SRs obtained under $T=25$ only change slightly (\ie $\pm 0.5\%$), indicating that all competing SNNs are not sensitive to the $T$ value in static obstacle avoidance tasks. The observations related to the $T$ value also hold in the dynamic obstacle experiments (see Table~\ref{SMtab:Degraded environment}). However, we observe that the SRs decrease as the $T$ value increases for most degraded input and weight uncertainty experiments. 

\noindent
Tables~\ref{SMtab:Degraded environment}, ~\ref{SMtab:Degraded inputs}, and ~\ref{SMtab:Weight pollution} show the quantitative performance of all competing approaches in dynamic obstacle, degraded inputs, and weight uncertainty experiments, respectively. The SRs are also shown in Figures~\ref{fig:SN_OA_results}a and b. In terms of the OTPs, we witness high levels of overtime trials in the ``0.2" section of the degraded inputs condition and the ``GN weight" section of the weight uncertainty condition.
As discussed in the main manuscript, with the ``0.2" setup, the three disturbed lasers generate more spikes than they are supposed to, making the robot more cautious. Thus, the robot's speed slows, leading to more overtime trials. As expected, adding Gaussian noise to the learned weights reduces the effectiveness of the avoidance policy. However, our approach faces the most negligible impact, offering the best SRs under all experimental results. In the following, we provide a more detailed analysis for each degraded condition.

\noindent
\tb{Dynamic Obstacles} As discussed, we introduce $11$ dynamically moving cylinders to the static testing environment; see Figure~\ref{SMfig:env}c. Table~\ref{SMtab:Degraded environment} shows the corresponding experimental results obtained under this condition. Our approach delivers the highest SRs with both the LIF and SRM neuron models. Notably, under both the $T=5$ and $T=25$ settings, the proposed approach outperforms the runners-up by significant margins (by at least $9\%$ over the LIF model and $12\%$ over the SRM). The results demonstrate that the proposed bioinspired dynamic threshold scheme provides substantial environmental adaptability to the host SNNs. Since all the synaptic weights and static thresholds of both the SAN and the SAN with no resting operation (SAN-NR) are learned from the environments with static obstacles only, we expect that they cannot adapt well to an environment with dynamic objects. Surprisingly, compared to the static threshold scheme, the two heuristic dynamic threshold schemes, DT1 and DT2, obtain lower SRs. The threshold dynamics provided by DT1 rely on two hyperparameters, the constant potential and initial potential. DT2 requires a target firing count to be set. These hyperparameters are justified during the training process but fixed during testing. We believe that these hyperparameters dramatically impact the adaptability of the tested heuristic dynamic threshold schemes. In contrast, the dynamics offered by the proposed bioinspired dynamic energy-temporal threshold (\DTname) scheme are dynamically based on layerwise statistical cues.

\noindent 
\tb{Degraded Inputs} In this experiment, as discussed in our main manuscript, in addition to the presence of dynamic obstacles, we disturb the obtained range measurements in three different ways: a) ``0.2": we set the 3rd, 9th, and 15th laser ranges to $0.2$ m. In this case, the three modified measurements always report obstacles in their perception fields even when none are present; b) ``6.0": the ranges of the same three lasers are set to $6.0$ m, which is the average visible range in the test environment. This means that the three lasers cannot perceive any object; c) ``GN": we add Gaussian noise (\ie $clip(s_{input} + \mathcal N(0,1.0), 0.2, 6.0)$, as suggested in a study regarding long short-term memory with a local map critic (LSTM-LMC)~\cite{choi2019deep}) to each of the $18$ range measurements. The experimental results obtained under these settings are shown in Table~\ref{SMtab:Degraded inputs}. 

\begin{figure}[th]
	\centering
	\includegraphics [scale=0.16]{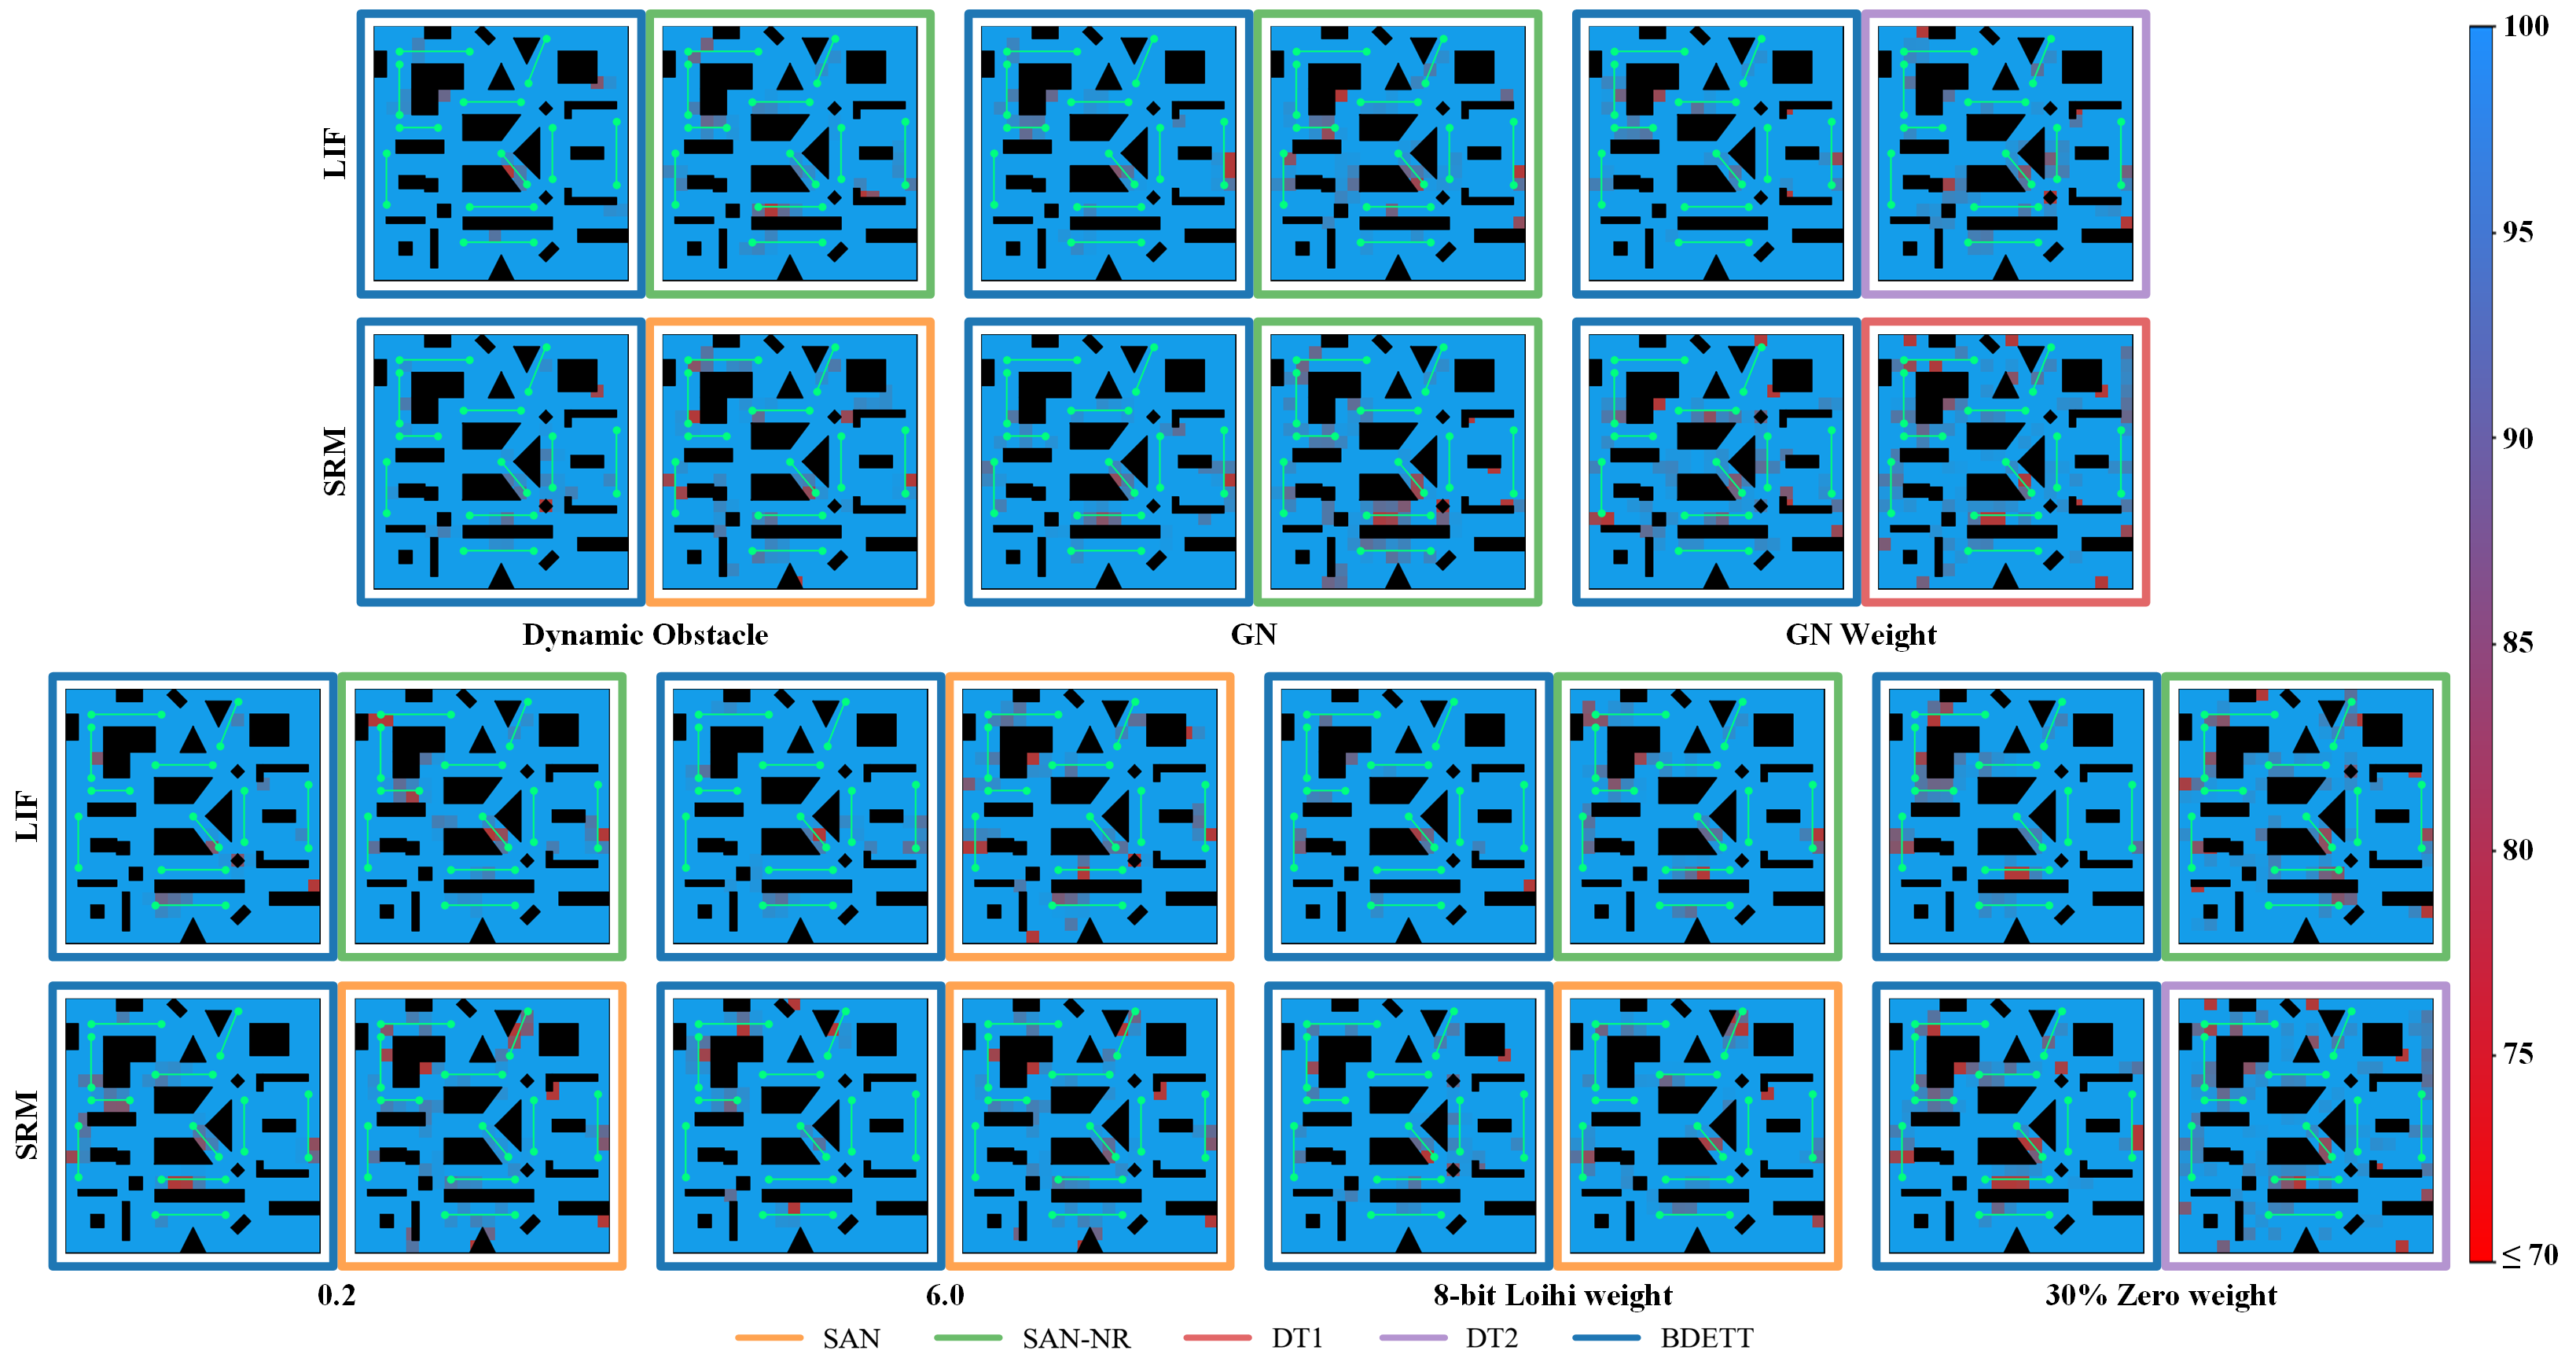}
	\vspace{-0.2cm}
	\caption{
	    The success rate heatmaps. The heatmaps yielded by the best and runner-up performers under four different conditions indicate the areas with lower success rates (\ie those shown in red).
	}
	\label{fig:SN_OA_heatmap}
	%\vspace{-0.2cm}
\end{figure}

\begin{figure}[t]
	\centering
	\includegraphics [scale=0.25]{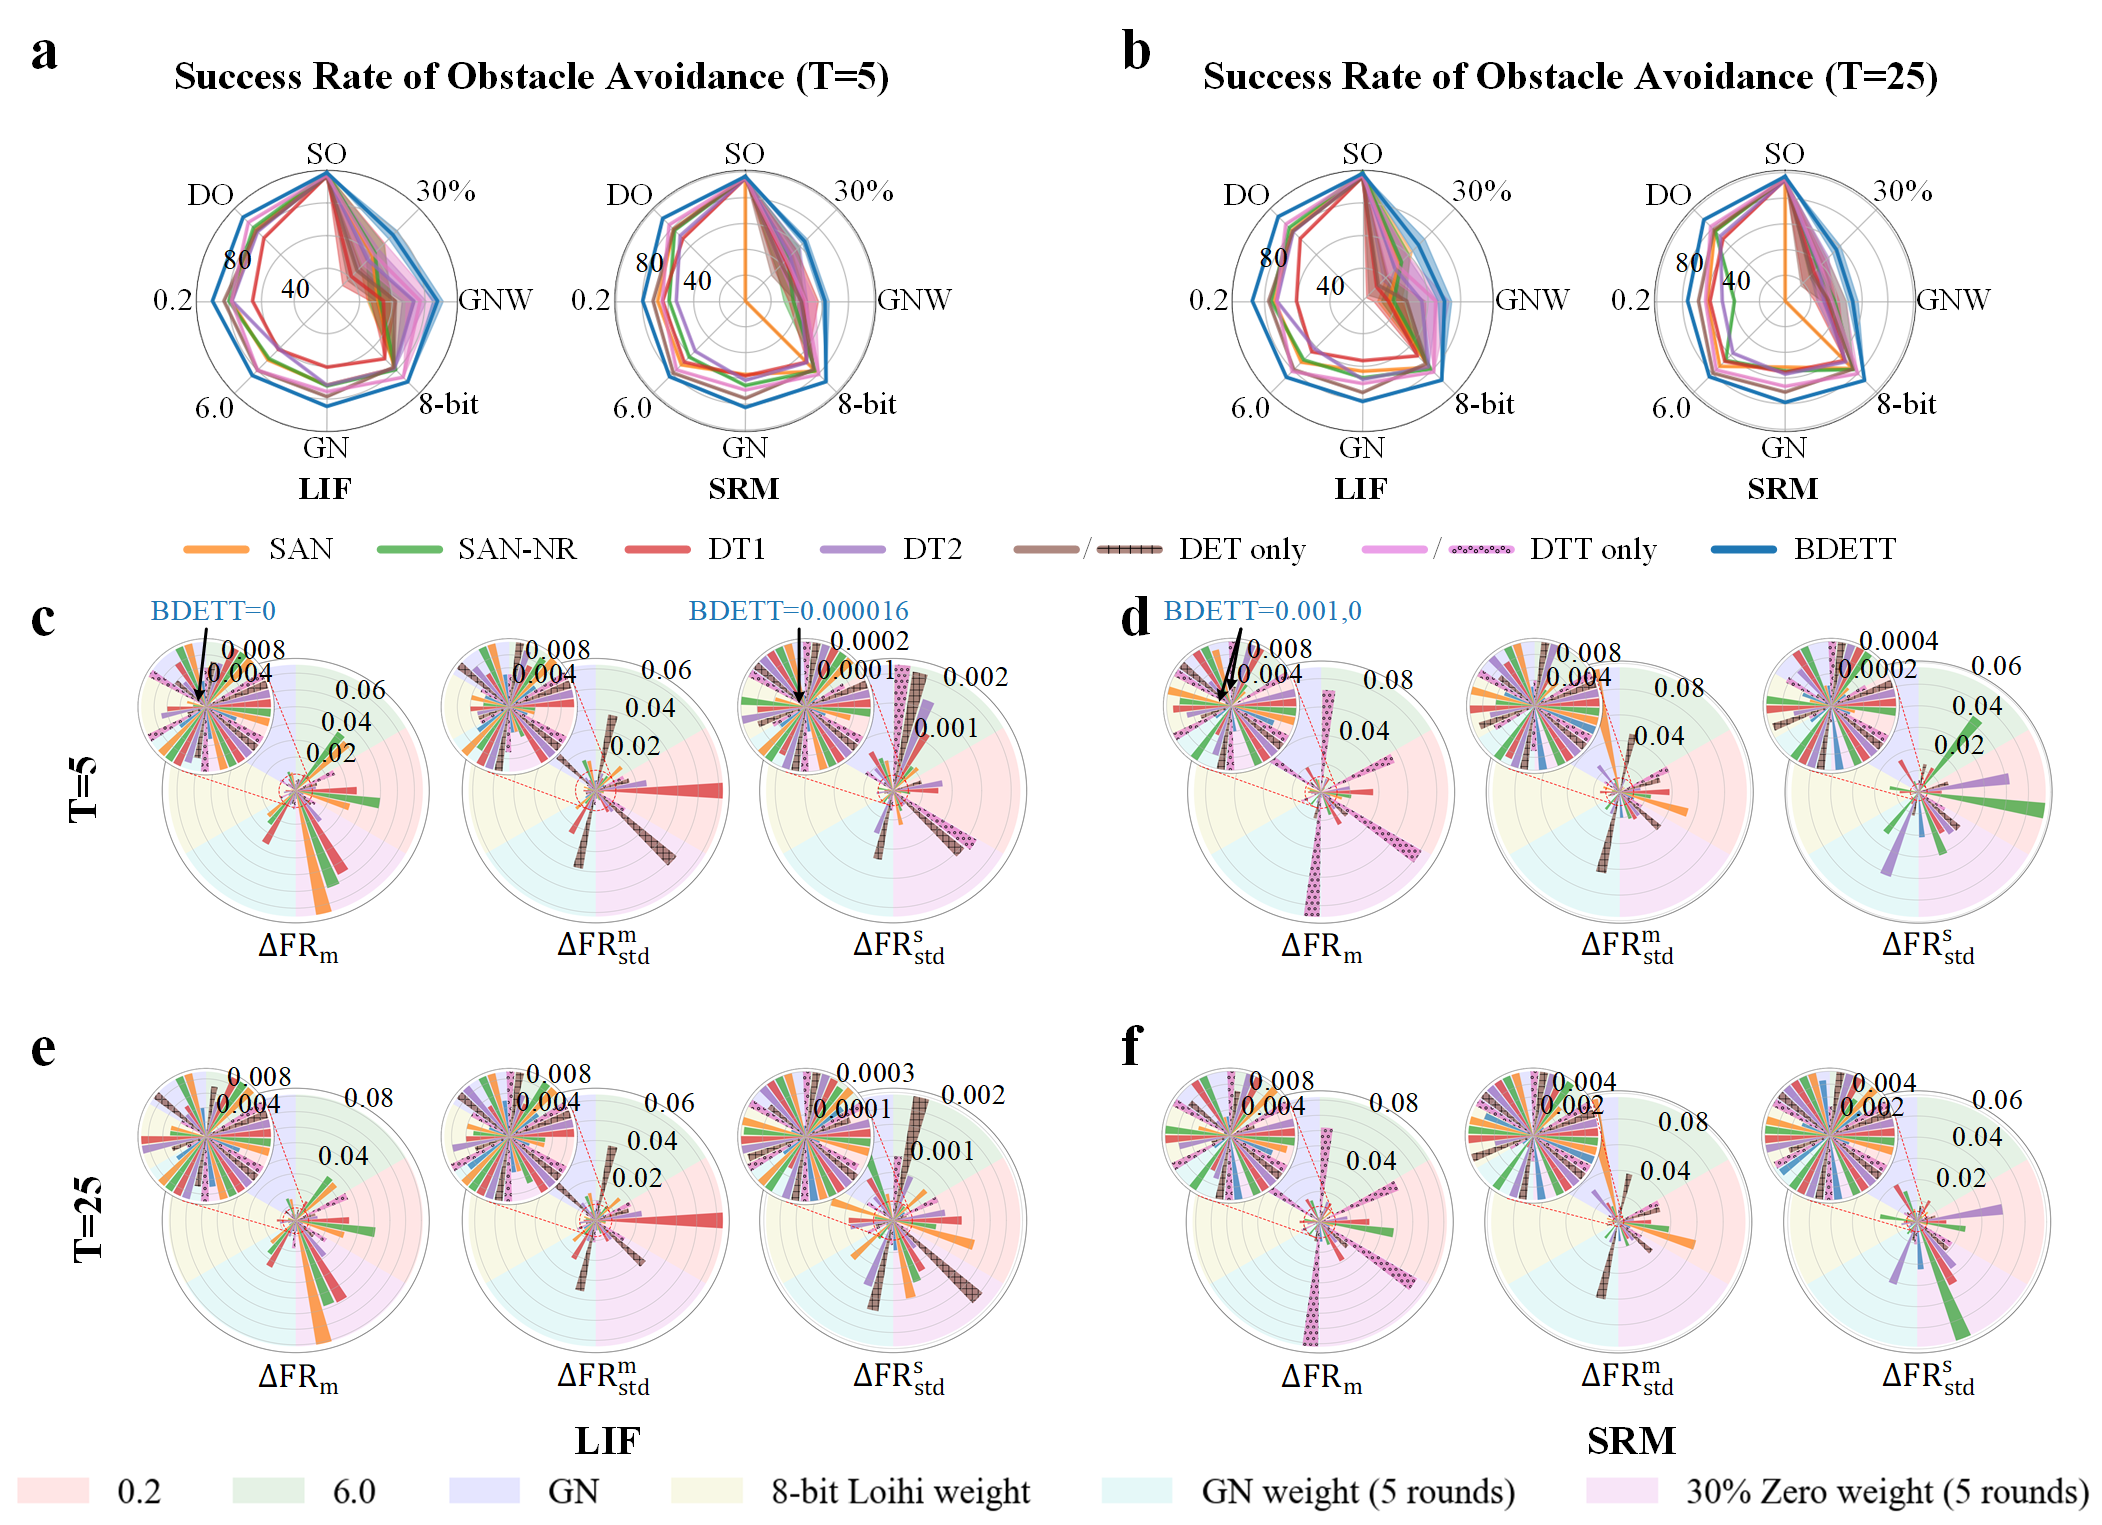}
	\vspace{-0.2cm}
	\caption{
	    The experimental results obtained for the robot obstacle avoidance tasks. a \& b. The SRs of obstacle avoidance under normal and different degraded conditions under the $T=5$ and $T=25$ settings, respectively. `SO' denotes the static obstacle condition; `DO' represents the dynamic obstacle condition; `0.2', `6.0', and `GN' are the three degraded input conditions; `8-bit', `GNW', and `$30\%$' denotes the 8-bit Loihi weights, GN weights, and $30\%$ zero weights, respectively. c \& d. Homeostasis measurements obtained with the $T=5$ setting by the LIF- and SRM-based host SNNs. e \& f. The homeostasis results obtained with the $T=25$ setup by the LIF- and SRM-based host SNNs, respectively. 
	}
	\label{fig:SN_OA_results}
	%\vspace{-0.2cm}
\end{figure}

\noindent
In all degraded input experiments, the SRs offered by our \DTname\ scheme still remain the highest and outperform the runners-up by at least $10\%$. This reflects that the proposed dynamic threshold scheme provides the host SNNs with strong adaptability to all designed degraded inputs, which is highly desired and appreciated in mobile robot applications. In the ``0.2" setup, the three disturbed lasers generate more spikes than they are supposed to, making the robot more cautious. All host SNNs obtain lower SRs than those obtained under the dynamic obstacle settings. However, the SRM-based host SNNs are significantly impacted. We believe the reason for this is that the spike response and refractory kernels of the SRM amplify the intense spikes triggered by the three modified measurements. In the ``6.0" experiments, the three modified measurements trigger fewer spikes, and the robot becomes more relaxed due to the `hyperopia' effect. Therefore, we expect more failed passes than in the ``0.2" setup. This is true for the LIF-based SNNs but not for the SRM-based SNNs. Since the three farsighted lasers reduce the signal amplification effects caused by the two kernels, the SRM-based SNNs perform better here than in the ``0.2'' experiments. Under the ``GN" condition, the SRs of all competing host SNNs decrease, but our approach is the least affected and induces the lowest SR drops. Remarkably, under all degraded input experiments, the proposed \DTname\ improves upon the SRs of both the LIF-based and SRM-based baseline models (\ie SAN-NR) by at least $10\%$ and $17\%$, respectively. The success rates of the best and runner-up performers under ``0.2'' and ``6.0'' conditions are also qualitatively illustrated in Figure~\ref{fig:SN_OA_heatmap}.

\noindent
\tb{Weight Uncertainty} Neuromorphic hardware (\eg Loihi) achieves computing efficiency by sacrificing the weight precision, and an $8$-bit integer normally yields the highest precision. Therefore, when deploying an SNN on neuromorphic hardware, one needs to scale and round up the learned floating-point synaptic weights to low-precision weights. We mimic this scenario by mapping the learned weights to Intel's Loihi $8$-bit integer weights. The mapping equations are provided in Supplementary Note 2. In addition, we design two extra weight pollution experiments. ``GN weight" involves adding Gaussian noise (\ie $w_{ij} + \mathcal N(0,0.05)$) to all synaptic weights; under ``30\% zero weight", we reandomly set $30\%$ of the synaptic weights between every two adjacent layers to $0$. To reduce the impact caused by the randomness introduced in the two additional experiments, we report the average SRs of 5-round tests. 

\noindent
As shown in Table~\ref{SMtab:Weight pollution}, the proposed \DTname\ can effectively reduce the impact caused by degraded synaptic weights and deliver the best SRs under all experimental settings. Low-precision weight convergence slightly reduces the SRs of all competing host SNNs slightly. We observe that the effectiveness of the SRM-based SNNs is dramatically impacted by the ``GN weight" and ``$30\%$ zero weight" pollution settings, especially the SAN. This means that SRM-based models are more sensitive to weight changes than LIF-based SNNs. Again, under the three degraded conditions, the proposed \DTname\ increases the SRs of the baseline model SAN-NR by at least $9.5\%$, $14.2\%$, and $14.8\%$. The success rates of the best and runner-up performers under ``8-bit Loihi weight'' and ``30\% zero weight'' conditions are also qualitatively illustrated in Figure~\ref{fig:SN_OA_heatmap}.

\begin{table}
% \begin{center}
%     Table S1. Quantitative performance of obstacle avoidance with static obstacles.
% \end{center}
\caption{Quantitative performance of obstacle avoidance with static obstacles.}
  \label{SMtab:Sta_test}
  \centering
  \setlength\tabcolsep{5pt}
  \begin{tabular}{lllllllll}
    \toprule
     
     & \multicolumn{2}{c}{\textbf{LIF} ($T=5$)}     & \multicolumn{2}{c}{\textbf{SRM} ($T=5$)}    & \multicolumn{2}{c}{\textbf{LIF} ($T=25$)}     & \multicolumn{2}{c}{\textbf{SRM} ($T=25$)}            \\
    \cmidrule(r){2-3}
    \cmidrule(r){4-5}
    \cmidrule(r){6-7}
    \cmidrule(r){8-9}
    \textbf{Name}  & \makecell[c]{SR$\uparrow$}    & \makecell[c]{OTP}   & \makecell[c]{SR$\uparrow$}    & \makecell[c]{OTP} & \makecell[c]{SR$\uparrow$}    & \makecell[c]{OTP}   & \makecell[c]{SR$\uparrow$}    & \makecell[c]{OTP} \\
    \hline
    SAN  & \makecell[c]{98\%}   & 0.0\%  & \textbf{96.5\%}  & 0.0\%  & \makecell[c]{98\%}   &   0.0\%  & \makecell[c]{96\%}   &    0.0\% \\
    SAN-NR  & \makecell[c]{98\%}  & 0.0\% & 95.5\%   &0.0\%  & \textbf{98.5\%}   &   0.0\%   & 95.5\%  &  0.0\% \\
    DT1~\cite{hao2020biologically}     &  96.5\%   & 0.0\% & \makecell[c]{95\%}  &  0.0\% & \makecell[c]{96\%}   &   0.0\%   & 94.5\%    &    0.5\% \\
    DT2~\cite{kim2021spiking}     & \makecell[c]{97\%}  & 0.0\%  & \makecell[c]{95\%}  & 0.0\% & \makecell[c]{97\%}  &  0.0\% & \makecell[c]{94\%}  &  0.0\% \\
    % DT3~\cite{sengupta2019going}   & 49.93    & 19.27   & 63.5\%  & 51.35 & 19.23 & 52.5\%  \\
    \hline
    DET only   & \makecell[c]{96\%}  & 0.0\%  & 95.5\%  & 0.0\% & 95.5\%  &   0.0\%   & \makecell[c]{95\%}  &  0.0\%\\
    DTT only   & \makecell[c]{97\%} & 0.0\%  & 95.5\%  &0.0\% & \makecell[c]{97\%}  &   0.0\%   &\makecell[c]{95\%}   &   0.0\%\\
    \hline
    \DTname\   & \textbf{98.5\%} & 0.0\% & \textbf{96.5\%} &  0.0\% & \makecell[c]{98\%}   &   0.0\%   & \makecell[c]{\textbf{97\%}} &   0.0\% \\
    \bottomrule
  \end{tabular}
\end{table}

% \begin{table}
% \caption{Quantitative performance of obstacle avoidance with static obstacles ($T=25$).}

%   \label{SMtab:Sta_test T=25}
%   \centering
  
%   \setlength\tabcolsep{5pt}
  
%   \begin{tabular}{lllll}
%     \toprule
     
%      & \multicolumn{2}{c}{\textbf{LIF ($T=25$)}}     & \multicolumn{2}{c}{\textbf{SRM ($T=25$)}}                \\
%     \cmidrule(r){2-3}
%     \cmidrule(r){4-5}
%     \textbf{Name}  & \makecell[c]{SR$\uparrow$}         & \makecell[c]{OTP}        & \makecell[c]{SR$\uparrow$}           & \makecell[c]{OTP} \\
%     \hline
%     SAN  & \makecell[c]{98\%}   &   0.0\%  & \makecell[c]{96\%}   &    0.0\%  \\
%     SAN-NR  & \textbf{98.5\%}   &   0.0\%   & 95.5\%  &  0.0\%   \\
%     DT1~\cite{hao2020biologically}     & \makecell[c]{96\%}   &   0.0\%   & 94.5\%    &    0.5\%  \\
%     DT2~\cite{kim2021spiking}     & \makecell[c]{97\%}  &  0.0\% & \makecell[c]{94\%}  &  0.0\%   \\
%     % DT3~\cite{sengupta2019going}   & 49.93    & 19.27   & 63.5\%  & 51.35 & 19.23 & 52.5\%  \\
%     \hline
%     DET only  & 95.5\%  &   0.0\%   & \makecell[c]{95\%}  &  0.0\%   \\
%     DTT only   & \makecell[c]{97\%}  &   0.0\%   &\makecell[c]{95\%}   &   0.0\%  \\
%     \hline
%     \DTname\   & \makecell[c]{98\%}   &   0.0\%   & \makecell[c]{\textbf{97\%}} &   0.0\%  \\
%     \bottomrule
%   \end{tabular}
% \end{table}

\begin{table}
% \begin{minipage}{1.0\linewidth}
\caption{Quantitative performance of obstacle avoidance with dynamic obstacles.}
  \vspace{0.2cm}
  \label{SMtab:Degraded environment}
  \centering

  \setlength\tabcolsep{5pt}
  \begin{tabular}{lllllllll}
    \toprule
     
     & \multicolumn{2}{c}{\textbf{LIF} ($T=5$)}     & \multicolumn{2}{c}{\textbf{SRM} ($T=5$)}   & \multicolumn{2}{c}{\textbf{LIF} ($T=25$)}     & \multicolumn{2}{c}{\textbf{SRM} ($T=25$)}              \\
    \cmidrule(r){2-3}
    \cmidrule(r){4-5}
    \cmidrule(r){6-7}
    \cmidrule(r){8-9}
     \textbf{Name}  & \makecell[c]{SR$\uparrow$}      & \makecell[c]{OTP}       & \makecell[c]{SR$\uparrow$}        & \makecell[c]{OTP} & \makecell[c]{SR$\uparrow$}          & \makecell[c]{OTP}        & \makecell[c]{SR$\uparrow$}           & \makecell[c]{OTP} \\
    \hline
    SAN  & 81.5\%      & 0.0\% & 78.5\%   & 0.0\%   & \makecell[c]{81\%}  & 0.0\% & 77.5\%  & 0.0\% \\
    SAN-NR  & 83.5\%   & 0.0\% & 77.5\%  & 0.5\%    & 83.5\%  & 0.0\%  & \makecell[c]{77\%}  & 1.0\%\\

    DT1~\cite{hao2020biologically}   & 74.5\%      & 0.0\%   & 68.5\%    & 0.0\%    &\makecell[c]{74\%}  & 0.5\% & 68.5\% & 0.5\%    \\
    DT2~\cite{kim2021spiking}  &  \makecell[c]{80\%}   & 0.0\%  &  71.5\%   & 0.5\% &\makecell[c]{80\%}    & 0.0\%  &  71.5\% &0.0\% \\
    % DT3~\cite{sengupta2019going}   & 49.93    & 19.27   & 63.5\%  & 51.35 & 19.23 & 52.5\%  \\
    \hline
    DET only  & \makecell[c]{81\%}      & 0.0\% & 78.5\%   & 0.5\%          & 80.5\%   &0.0\%   &   78.5\% & 1.0\%                                 \\
    DTT only  & \makecell[c]{88\%}      & 0.0\% & 83.5\%   &  0.0\%         & 86.5\%    & 0.0\%  &   \makecell[c]{82\%} & 0.0\%                    \\
    \hline                                                                   
    \DTname\   & \textbf{92.5\%}     &  0.0\%   & \textbf{90.5\%}  &  0.0\% &\makecell[c]{\textbf{93\%}}   & 0.0\%  &  \textbf{89.5\%} &  0.5\%    \\
    \bottomrule
  \end{tabular}
  \vspace{0.3cm}
\end{table}

\begin{table}
    \caption{Quantitative performance of obstacle avoidance under degraded input conditions.}
  \label{SMtab:Degraded inputs}
  \centering
%   \scriptsize
  \setlength\tabcolsep{5pt}
  \begin{tabular}{lllllllllllll}
    \toprule
    & & \multicolumn{2}{c}{\textbf{LIF} ($T=5$)}     & \multicolumn{2}{c}{\textbf{SRM} ($T=5$)}   & \multicolumn{2}{c}{\textbf{LIF} ($T=25$)}     & \multicolumn{2}{c}{\textbf{SRM} ($T=25$)}              \\
    \cmidrule(r){3-4}
    \cmidrule(r){5-6}
    \cmidrule(r){7-8}
    \cmidrule(r){9-10}
     \textbf{Type} & \textbf{Name}  & \makecell[c]{SR$\uparrow$}      & \makecell[c]{OTP}       & \makecell[c]{SR$\uparrow$}        & \makecell[c]{OTP} & \makecell[c]{SR$\uparrow$}          & \makecell[c]{OTP}        & \makecell[c]{SR$\uparrow$}           & \makecell[c]{OTP} \\
    \hline
    \multirow{7}{*}{\makecell[c]{0.2}}
    & SAN  & 78.5\%   & 1.5\% & \makecell[c]{68\%}  & 1.0\%                                   &74\%    &2.5\% &  60.5\%   & 1.0\%     \\
    & SAN-NR  & \makecell[c]{80\%} & 2.5\%  & \makecell[c]{59\%}  & 3.0\%                     &76\%    &3.0\%  & 39.5\%  & 4.5\%     \\
    & DT1~\cite{hao2020biologically}   & 65.5\%   & 4.0\%  &  \makecell[c]{64\%}  & 3.5\%     & 60.5\%  &3.5\% & 58.5\%    &  5.0\%  \\
    & DT2~\cite{kim2021spiking} & \makecell[c]{78\%}  & 3.0\% & 53.5\%  &  3.5\%              & 72.5\%  &4.0\% & 49\%    & 3.5\%     \\
    % & DT3~\cite{sengupta2019going}   & 66.33    & 19.57   & 64.5\% & 71.89 & 20.12 & 44.5\%  66.33    & 19.57   & 64.5\% & 71.89   \\
    \cline{2-10}                                                                                
    & DET only  & \makecell[c]{83\%}    & 2.0\% & 71.5\%  & 3.0\%                             & 77.5\%  &3.5\% & 67.5\%   &   3.0\%  \\
    & DTT only  & 78.5\%      & 3.5\% & 64.5\%  & 1.0\%                                       & 72.5\%  &3.5\% &  62\%   &  2.5\%    \\
    \cline{2-10}                                                                                
    & \DTname\   & \textbf{\makecell[c]{90\%}}    & 2.5\% & \textbf{79.5\%} & 3.5\%           & \textbf{87.5\%} &3.5\%  &\textbf{76\%}    &  4.5\%     \\
    \hline
    \multirow{7}{*}{\makecell[c]{6.0}}
    & SAN  & \makecell[c]{71\%}     & 0.0\% & \makecell[c]{70\%}  &  0.0\%                                &73\%  & 0.0\% &  72\%   & 0.0\%                     \\
    & SAN-NR  & \makecell[c]{70\%} & 0.0\%  &  61.5\%  & 0.0\%                                            &71\%   & 0.0\% & 65.5\%   & 0.0\%                   \\
    & DT1~\cite{hao2020biologically}     & \makecell[c]{62\%}   & 0.0\% & \makecell[c]{67\%}   & 0.0\%    &64\%  &0.0\%  & 66.5\%   &  0.0\%                   \\
    & DT2~\cite{kim2021spiking}  & 61.5\%    & 0.0\%   &  \makecell[c]{55\%}  & 0.5\%                   &61.5\%    &0.0\%  & 57.5\%   &  0.0\%             \\
    % & DT3~\cite{sengupta2019going}   & 43.57    & 18.03   & \makecell[c]{51\%} & 44.42 & 19.32 & 49.5\%  43.57    & 18.03   & \makecell[c]{51\%} & 44.42 &   \\
    \cline{2-10}                                                                                            
    & DET only  & \makecell[c]{80\%}    & 0.0\% & \makecell[c]{79\%}  & 0.0\%                             &79.5\%   &0.0\%  & 79.5\%  & 0.0\%                  \\
    & DTT only  & \makecell[c]{80\%}    & 0.0\% & 75.5\%  & 0.0\%                                         &81\%   & 0.0\% & 76\%   &  0.0\%                    \\
    \cline{2-10}                                                                                            
    & \DTname\   & \textbf{\makecell[c]{84.5\%}}   & 0.0\%  & \textbf{\makecell[c]{83\%}} &  0.0\%        &\textbf{86\%}  & 0.0\% & \textbf{83.5\%}  &  0.0\%  \\
    
    \hline
    \multirow{7}{*}{\makecell[c]{GN}}
    & SAN & 71.5\%   & 0.0\% & \makecell[c]{57\%}  & 0.0\%                                                   & 63\%    &  0.0\%  & 51.5\%    &  0.5\%                     \\
    & SAN-NR  & \makecell[c]{72\%}  & 0.0\%  &  65.5\%  & 1.0\%                                              & 67\%  & 0.5\% & 54.5\%  &  2.0\%                           \\
    & DT1~\cite{hao2020biologically}    & 60.5\%     & 0.5\% &  \makecell[c]{58\%}  &  0.0\%                 & 56.5\%     & 0.5\%  & 55.5\%   &    0.0\%                  \\
    & DT2~\cite{kim2021spiking}  &   71.5\%   &  1.5\% &   61.5\%   &  0.0\%                                 & 68\%   &  1.0\% & 57\%   & 1.5\%                           \\
    % & DT3~\cite{sengupta2019going}   & 48.93    & 19.84   & 53.5\% & 47.98 & 18.81 & \makecell[c]{47\%}    & 48.93    & 19.84   & 53.5\% & 47.98 & 18.81 & \makec       \\
    \cline{2-10}                                                                                              
    & DET only  & 78.5\%      & 1.0\% & 75.5\% & 0.5\%                                                       & 76\%  & 2.0\%  & 71\%  & 0.5\%                             \\
    & DTT only   & 75.5\%   & 0.0\% & \makecell[c]{69\%} & 0.0\%                                             & 70.5\% & 0.0\%  &  66.5\%  & 0.5\%                         \\
    \cline{2-10}                                                                                              
    & \DTname\   & \textbf{\makecell[c]{84.5\%}}       & 0.0\%  & \textbf{82.5\%}  & 0.0\%                   & \textbf{81.5\%} & 0.0\%   & \textbf{79\%}    & 0.5\%       \\
    
    \bottomrule
  \end{tabular}
\end{table}

\begin{table}
%   \vspace{0.3cm}
      \caption{Quantitative performance of obstacle avoidance under weight uncertainty conditions.}
    %   \vspace{-0.2cm}
  \label{SMtab:Weight pollution}
  \centering
  \scriptsize
  \setlength\tabcolsep{5pt}
  \begin{tabular}{lllllllllllll}
    \toprule
    & & \multicolumn{2}{c}{\textbf{LIF} ($T=5$)}     & \multicolumn{2}{c}{\textbf{SRM} ($T=5$)}   & \multicolumn{2}{c}{\textbf{LIF} ($T=25$)}     & \multicolumn{2}{c}{\textbf{SRM} ($T=25$)}              \\
    \cmidrule(r){3-4}
    \cmidrule(r){5-6}
    \cmidrule(r){7-8}
    \cmidrule(r){9-10}
     \textbf{Type} & \textbf{Name}  & \makecell[c]{SR$\uparrow$}      & \makecell[c]{OTP}       & \makecell[c]{SR$\uparrow$}        & \makecell[c]{OTP} & \makecell[c]{SR$\uparrow$}          & \makecell[c]{OTP}        & \makecell[c]{SR$\uparrow$}           & \makecell[c]{OTP} \\
     \hline
    \multirow{7}{*}{\makecell[c]{8-bit \\ Loihi \\ weight}}
    & SAN  & \makecell[c]{78.5\%}     & 0.0\%  & \makecell[c]{77\%}  & 0.0\%                               & \makecell[c]{77.5\%} & 0.0\%  & \makecell[c]{74.5\%}   & 0.0\%                  \\
    & SAN-NR  & \makecell[c]{79.5\%}     & 0.0\%  & \makecell[c]{76.5\%}      &  0.5\%                     & \makecell[c]{79\%}   & 0.0\%  & \makecell[c]{75.5\%}   & 0.0\%                    \\
    & DT1~\cite{hao2020biologically}  & \makecell[c]{70\%}   & 0.0\%  & \makecell[c]{67\%}    & 0.0\%      & \makecell[c]{67.5\%} & 0.5\%  & \makecell[c]{65.5\%}   & 0.0\%                 \\
    & DT2~\cite{kim2021spiking}  & \makecell[c]{78.5\%}    & 0.0\%  & \makecell[c]{67.5\%}       & 1.0\%   & \makecell[c]{77\%}   & 0.0\%  & \makecell[c]{67\%}     & 0.5\%                          \\
    % & DT3~\cite{sengupta2019going}   & 63.12    & 20.10   & 21.5\% & 50.75 & 21.31 & 24.1\%              & \makecell[c]{66.33  & 19.57   & \makecell[c]{64.5\% & 71.89 & 20.12 & 44.5\%  \\
    \cline{2-10}                                                                                                                              
    & DET only  & \makecell[c]{77.5\%}   & 0.0\% & \makecell[c]{75\%}    & 0.0\%                           & \makecell[c]{74.5\%} & 0.5\%  & \makecell[c]{75\%}     & 0.0\%                    \\
    & DTT only  &  \makecell[c]{86\%}     & 0.0\% & \makecell[c]{80.5\%}  & 0.0\%                          & \makecell[c]{81.5\%} & 0.0\%  & \makecell[c]{80\%}     & 0.0\%                  \\
    \cline{2-10}                                                                                                                              
    & \DTname\   & \makecell[c]{\textbf{90\%}}    & 0.0\% & \makecell[c]{\textbf{88.5\%}}  & 0.0\%         & \makecell[c]{\textbf{88.5\%}} & \makecell[c]{0.0\%}    & \makecell[c]{\textbf{87.5\%}}  & 0.0\% \\
    \hline
    
    \multirow{7}{*}{\makecell[c]{GN \\ weight \\ (5 rounds)}}
    & SAN  & \makecell[c]{51.3\% ($\sigma\mbox{-}6.8$)}  & 1.2\% &  \makecell[c]{0\% ($\sigma\mbox{-}0$)}  & \makecell[c]{20.3\%}                        & 36.2\% ($\sigma\mbox{-}7.3$) & 3.6\%   & 0\%  ($\sigma\mbox{-}0$)  & 18.4\%                              \\
    & SAN-NR  & \makecell[c]{52.5\% ($\sigma\mbox{-}7.1$)}     & 1.6\%  & \makecell[c]{37.2\% ($\sigma\mbox{-}7.6$)}  & 2.4\%                            & 39.0\%  ($\sigma\mbox{-}7.8$)  & 3.1\%  & 38.4\%  ($\sigma\mbox{-}8.9$)  & 2.1\%                         \\
    & DT1~\cite{hao2020biologically}     & \makecell[c]{54.6\% ($\sigma\mbox{-}7.9$)} & 2.3\% & \makecell[c]{44.9\% ($\sigma\mbox{-}11.4$)} &  3.0\%     & 35.7\% ($\sigma\mbox{-}9.2$)  & 3.3\%  & 32.4\%  ($\sigma\mbox{-}9.6$)   & 4.7\%                         \\
    & DT2~\cite{kim2021spiking}     & \makecell[c]{73.2\% ($\sigma\mbox{-}7.4$)}  & 2.1\% & \makecell[c]{43.6\% ($\sigma\mbox{-}4.4$)} & 2.4\%           & 56.2\%  ($\sigma\mbox{-}9.3$)  &  2.0\%  & 30.3\%  ($\sigma\mbox{-}5.7$)  &  2.9\%                       \\
    % & DT3~\cite{sengupta2019going}   & 47.89    & 19.04   & 33.0\% & 53.67 & 22.44 & 28.2\%                                                            & 43.57    & 18.03   & \makecell[c]{51\%} & 44.42 & 19.32 & 49.5\%                                         \\
    \cline{2-10}                                                                                                                                          
    & DET only  & \makecell[c]{61.8\% ($\sigma\mbox{-}12.0$)}  & 1.8\% & \makecell[c]{43.3\% ($\sigma\mbox{-}4.6$)} & 2.5\%                              & 47.0\% ($\sigma\mbox{-}11.3$)   & 2.3\%  & 34.1\% ($\sigma\mbox{-}5.4$) &2.6\%                           \\
    & DTT only  & \makecell[c]{77.1\% ($\sigma\mbox{-}8.8$)}  & 1.5\% & \makecell[c]{46.4\% ($\sigma\mbox{-}8.0$)}  & 1.6\%                              & 64.7\% ($\sigma\mbox{-}8.0$)  & 1.8\%  & 36.8\% ($\sigma\mbox{-}10.2$) & 1.4\%                           \\
    \cline{2-10}                                                                                                                                          
    & \DTname\   & \textbf{\makecell[c]{87.7\% ($\sigma\mbox{-}3.3$)}}   &  0.8\% & \makecell[c]{\textbf{61.8\% ($\sigma\mbox{-}2.9$)}} &  1.3\%         & \textbf{70.1\%} ($\sigma\mbox{-}4.2$)    &  0.4\%   & \textbf{52.6\%} ($\sigma\mbox{-}4.0$)    & 2.5\%   \\
    
    \hline
    \multirow{7}{*}{\makecell[c]{ $30\%$ \\ Zero \\ weight  \\ (5 rounds)}}
    & SAN  & \makecell[c]{59.3\% ($\sigma\mbox{-}10.5$)}    & 0.0\% & \makecell[c]{0\% ($\sigma\mbox{-}0$)}  & 17.7\%                                    & 51.2\% ($\sigma\mbox{-}11.3$)   & 0.0\%  & 0\% ($\sigma\mbox{-}0$)   &  19.4\%                            \\
    & SAN-NR  & \makecell[c]{61.6\% ($\sigma\mbox{-}7.5$)}     &0.0\% & \makecell[c]{46.5\% ($\sigma\mbox{-}12.4$)}    & 0.0\%                           & 53.6\% ($\sigma\mbox{-}6.7$)  & 0.0\% & 36.5\% ($\sigma\mbox{-}9.9$)  & 0.2\%                             \\
    & DT1~\cite{hao2020biologically}  & \makecell[c]{41.2\% ($\sigma\mbox{-}7.7$)}    & 0.7\%  & \makecell[c]{44.3\% ($\sigma\mbox{-}11.7$)} & 0.0\%     & 32.2\% ($\sigma\mbox{-}9.1$)  & 1.3\% & 31.7\% ($\sigma\mbox{-}12.6$)   & 0.6\%                           \\
    & DT2~\cite{kim2021spiking}  & \makecell[c]{55.6\% ($\sigma\mbox{-}9.3$)}    & 0.3\% & \makecell[c]{49.1\% ($\sigma\mbox{-}10.8$)}  &  0.8\%         & 48.0\% ($\sigma\mbox{-}10.5$) & 0.0\%  & 37.8\% ($\sigma\mbox{-}10.2$)  & 1.1\%                           \\
    % & DT3~\cite{sengupta2019going}   & 63.12    & 20.10   & 21.5\% & 50.75 & 21.31 & 24.1\%                                                            & 48.93    & 19.84   & 53.5\% & 47.98 & 18.81 & \makecell[c]{47\%}                                          \\
    \cline{2-10}                                                                                                                                          
    & DET only  & \makecell[c]{46.2\% ($\sigma\mbox{-}8.5$)}   & 0.0\% & \makecell[c]{39.8\% ($\sigma\mbox{-}11.5$)} & 1.4\%                             &33.6\% ($\sigma\mbox{-}8.5$)  & 0.8\% & 29.3\% ($\sigma\mbox{-}12.3$)  & 2.5\%                             \\
    & DTT only  & \makecell[c]{60.6\% ($\sigma\mbox{-}9.5$)}     & 0.0\% & \makecell[c]{45.4\% ($\sigma\mbox{-}7.4$)} & 0.5\%                            & 50.3\% ($\sigma\mbox{-}8.7$)  & 0.4\% & 38.8\% ($\sigma\mbox{-}8.0$)  & 1.3\%                             \\
    \cline{2-10}                                                                                                                                          
    & \DTname\   & \makecell[c]{\textbf{77.2\% ($\sigma\mbox{-}3.6$)}}   & 0.0\% & \makecell[c]{\textbf{65.2\% ($\sigma\mbox{-}2.7$)}} & 0.3\%           &\textbf{68.4\%} ($\sigma\mbox{-}5.2$)  & 0.0\% & \textbf{56.5\%} ($\sigma\mbox{-}4.3$)  & 0.7\%            \\
    
    \bottomrule
  \end{tabular}

% \end{minipage}
\end{table}

\clearpage
\subsection*{Assessment---Homeostatic}
\label{sec:homeostatic}

In the main manuscript, we show the quantified homeostasis changes induced during all successful trials with respect to the base condition (\ie the homeostasis obtained in the dynamic obstacle experiments) under the $T=5$ setting. Table~\ref{SMtab:hom_success_5} provides the raw homeostasis measurements and the corresponding changes used for plotting the polar chart in the main manuscript. 

\noindent
We also offer the measured homeostasis and corresponding changes obtained under the $T=25$ setting in Table~\ref{SMtab:hom_success_25}. The corresponding polar plots are shown in Figures~\ref{fig:SN_OA_results}e and f. Similar to the observations obtained in the experiments with $T=5$, the association between homeostasis and the obstacle avoidance SR still holds for $T=25$; stronger homeostasis offers better performance. Notably, our approach induces the smallest changes in the three metrics across all experimental settings, except for the $\Delta\text{FR}_{std}^m$ obtained in the SRM-based 8-bit Loihi weight experiment. Furthermore, the proposed \DTname\ delivers the best obstacle avoidance SRs in all designed experimental conditions with $T=25$; see Tables~\ref{SMtab:Degraded environment}, ~\ref{SMtab:Degraded inputs}, and~\ref{SMtab:Weight pollution} and Figures~\ref{fig:SN_OA_results}e and f.

% The proposed \DTname\ offers the strongest homeostasis to the host SNNs among all competing approaches. Correspondingly, the SNNs with \DTname\ scheme perform the best in all conditions. The opposite also holds. For example, in `0.2' section of Figure~\ref{fig:h_changes}(b), DT1 gives the maximum change. Besides, it gives the second largest values in `0.2' section of Figure~\ref{fig:h_changes} (a) and (c). Correspondingly, DT1 hosted by a LIF-based SNN shows the worst performance (see Table~\ref{tab:Degraded inputs}). These experimental results validate that strong homeostasis provided by our \DTname\ can effectively enhance an SNNs' adaptiveness to different degraded conditions. We argue that this is a highly desired capability not only for the field of mobile robotics but also for broader machine learning.

\begin{table}
  \caption{\bd{The raw homeostasis measurements of successful trials and the corresponding changes with respect to the baseline condition in obstacle avoidance tasks with the $T=5$ setting.}}
%   \caption{Firing rate evaluation test of different methods on different SNN models in successful trials ($T=5$)}
  \label{SMtab:hom_success_5}
  \centering
  \scriptsize
  \setlength\tabcolsep{4pt}
  \begin{tabular}{llllllll}
    \toprule
     
     & & \multicolumn{3}{c}{\textbf{LIF} ($T=5$)}     & \multicolumn{3}{c}{\textbf{SRM} ($T=5$)}                \\
    \cmidrule(r){3-5}
    \cmidrule(r){6-8}
     \textbf{Type} & \textbf{Name}  & \makecell[c]{$\text{FR}_m (\Delta)$}        & \makecell[c]{$\text{FR}_{std}^m (\Delta)$}     & \makecell[c]{$\text{FR}_{std}^s (\Delta)$}         & \makecell[c]{$\text{FR}_m (\Delta)$}        & \makecell[c]{$\text{FR}_{std}^m (\Delta)$}     & \makecell[c]{$\text{FR}_{std}^s (\Delta)$}     \\ 
    \hline
    \multirow{7}{*}{\makecell[c]{Dynamic \\ obstacle \\ (baseline \\ condition)}}
    & SAN  &0.523 &0.325  &0.000891  &0.278 &0.301  &0.000596   \\
    & SAN-NR  &0.515  &0.330  &0.001029   &0.487  & 0.309 &0.006853  \\
    & DT1~\cite{hao2020biologically}   &0.443   &0.325    &0.001738 &0.482   &0.310    &0.002942      \\
    & DT2~\cite{kim2021spiking}     &0.400   &0.345  &0.002136  &0.418  &0.309    &0.005873      \\

    & DET only   &0.508  &0.336    &0.001024  &0.380  &0.276    &0.002564 \\
    & DTT only & 0.456  & 0.320        &0.000902   &0.475   &0.294   &0.002284  \\
    & \DTname\  & 0.439   &  0.312    & 0.000916  &0.501   &0.298      &0.001759   \\
    \hline
    \multirow{7}{*}{\makecell[c]{0.2}}
    & SAN  &0.556 (0.033) &0.329 (0.004)  &0.000750 (0.000141)  &0.293 (0.015) &0.247 (0.054)  &0.000746 (0.000150)   \\
    & SAN-NR  &0.565 (0.050)  &0.326 (0.004)  &0.000738 (0.000291)   & 0.508 (0.021)  &0.333 (0.024)  &0.001069 (0.005784)    \\
    & DT1~\cite{hao2020biologically}    &0.479 (0.036)   &0.387 (0.062)    &0.000973 (0.000765)    &0.518 (0.036)   &0.348 (0.038)    &0.003993 (0.001051)   \\
    & DT2~\cite{kim2021spiking}     &0.412 (0.012)  &0.370 (0.025)    &0.001293 (0.000843)    &0.438 (0.020)  &0.325 (0.016)    &0.001709 (0.004164)    \\

    & DET only   &0.495 (0.013)  &0.353 (0.017)    &0.001523 (0.000499)  &0.380 (0.000)  &0.244 (0.032)    &0.003969 (0.001405)    \\
    & DTT only & 0.481 (0.025)  & 0.335 (0.015)        & 0.000768 (0.000134)  &0.420 (0.055)   &0.335 (0.041)         &0.002040 (0.000244)    \\
    & \DTname\  &0.444\textbf{ (0.005)}   &0.315\textbf{ (0.003)}      &0.000851\textbf{ (0.000065)}    &0.494\textbf{ (0.007)}   &0.310\textbf{ (0.012)}      &0.001884\textbf{ (0.000125)}  \\
    \hline
    \multirow{7}{*}{\makecell[c]{6.0}}
    & SAN  &0.564 (0.041) &0.342 (0.017)  &0.001454 (0.000563)  &0.275 (0.003) &0.306 (0.005)  &0.000747 (0.000151)   \\
    & SAN-NR  &0.558 (0.043)  &0.339 (0.009)  &0.001548 (0.000519)   &0.483 (0.004)  &0.306 (0.003)  &0.002533 (0.004320) \\
    & DT1~\cite{hao2020biologically}    &0.432 (0.011)   &0.318 (0.007)    &0.002862 (0.001124)   &0.471 (0.011)  & 0.315 (0.005)   &0.004224 (0.001282)   \\
    & DT2~\cite{kim2021spiking}     &0.407 (0.007)  &0.354 (0.009)    &0.003785 (0.001649)    &0.408 (0.010)  &0.320 (0.011)   &0.005417 (0.000456)  \\

    & DET only   &0.515 (0.007)  &0.374 (0.038)    &0.003088 (0.002064)  &0.377 (0.003)  &0.230 (0.046)    &0.003889 (0.001325)    \\
    & DTT only &0.450 (0.006)   & 0.325 (0.005)        &0.003057 (0.002155)   &0.403 (0.072)   &0.290 (0.004)     &0.002855 (0.000571)   \\
    & \DTname\  & 0.440\textbf{ (0.001)}  &0.317\textbf{ (0.005)}      &0.000960\textbf{ (0.000044)}   &0.501\textbf{ (0.000)}   &0.300\textbf{ (0.002)}     &0.001870\textbf{ (0.000111)}   \\
    \hline
    \multirow{7}{*}{\makecell[c]{GN}}
    & SAN  &0.534 (0.011) &0.310 (0.015)  &0.001416 (0.000525)  &0.287 (0.009) & 0.204 (0.097) &0.000727 (0.000131)  \\
    & SAN-NR  &0.527 (0.012)  &0.314 (0.016)  & 0.001622 (0.000593)  & 0.497 (0.010) &0.298 (0.011) & 0.007395 (0.000542)   \\
    & DT1~\cite{hao2020biologically}    & 0.451 (0.008)  &0.319 (0.006)    &0.000982 (0.000756)  & 0.502 (0.020)  &0.302 (0.008)    &0.004634 (0.001692) \\
    & DT2~\cite{kim2021spiking}     &0.405 (0.005)  &0.337 (0.008)    &0.001654 (0.000482)    &0.423 (0.005)  &0.283 (0.026)    &0.005578 (0.000295)   \\

    & DET only   & 0.502 (0.006) &0.361 (0.025)    &0.001228 (0.000204)  &0.390 (0.010)  &0.283 (0.007)    &0.002454 (0.000110)   \\
    & DTT only &0.445 (0.011)   &0.315 (0.005)         & 0.001453 (0.000551)  &0.390 (0.085)   & 0.308 (0.014)        &0.001968 (0.000316)  \\
    & \DTname\  & 0.443\textbf{ (0.004)}  & 0.307\textbf{ (0.005)}     &0.000880\textbf{ (0.000036)}   &0.500\textbf{ (0.001)}   &0.301\textbf{ (0.003)}    &0.001886\textbf{ (0.000127)}   \\
    \hline
    \multirow{7}{*}{\makecell[c]{8-bit \\ Loihi \\ weight}}
    & SAN  &0.520 (0.003) &0.319 (0.006)  &0.000988 (0.000097)  &0.288 (0.010) &0.314 (0.013)  &0.000731\textbf{ (0.000135)}   \\
    & SAN-NR  &0.513 (0.002)   & 0.334\textbf{ (0.004)}  & 0.001286 (0.000257)    & 0.479 (0.008) &0.315 (0.006) &0.005527 (0.001326)  \\
    & DT1~\cite{hao2020biologically}    &  0.437 (0.006)  & 0.319 (0.006)    & 0.001589 (0.000149)  &0.473 (0.009)  &0.325 (0.015)  &0.002084 (0.000858)     \\
    & DT2~\cite{kim2021spiking}      &0.407 (0.007)   &0.340 (0.005)     &0.001853 (0.000283)    & 0.425 (0.007) &0.316 (0.007)  &0.005638 (0.000235)    \\

    & DET only   & 0.505 (0.003)  & 0.341 (0.005)    &0.000868 (0.000156)   & 0.385 (0.005) &0.285 (0.009)    &0.002185 (0.000379)    \\
    & DTT only & 0.446 (0.010)  & 0.325 (0.005)        & 0.000787 (0.000115)  & 0.460 (0.015)  &0.301 (0.007)   &0.002436 (0.000152)   \\
    & \DTname\  & 0.439\textbf{ (0.000)}  & 0.308\textbf{ (0.004)}     & 0.000932\textbf{ (0.000016)}  &0.500\textbf{ (0.001)}    &0.293\textbf{ (0.005)}      &0.001570 (0.000189) \\
    \hline
    \multirow{7}{*}{\makecell[c]{GN \\ weight \\  (5 rounds)}}
    & SAN  &0.501 (0.022) &0.338 (0.013)  &0.001192 (0.000301)  & - & - & -  \\
    & SAN-NR  &0.490 (0.025)  &0.338 (0.008)  &0.001281 (0.000252)   &0.498 (0.011)  &0.326 (0.017)  &0.004461 (0.002392)    \\
    & DT1~\cite{hao2020biologically}    & 0.407 (0.036)  &0.349 (0.024)    &0.001902 (0.000164)  &0.487 (0.005)   &0.319 (0.009)    &0.003573 (0.000631)     \\
    & DT2~\cite{kim2021spiking}     &0.391 (0.009)  &0.335 (0.010)    & 0.001356 (0.000780)   &0.410 (0.008)  &0.291 (0.018)    & 0.010002 (0.004129)   \\

    & DET only   &0.516 (0.008)  &0.375 (0.039)    &0.002225 (0.001201)  &0.399 (0.019)  &0.212 (0.064)    &0.003675 (0.001111)    \\
    & DTT only &0.467 (0.011)   & 0.327 (0.007)        &0.001244 (0.000342)   &0.387 (0.088)   &  0.301 (0.007)  & 0.002387 (0.000103)  \\
    & \DTname\  &0.444\textbf{ (0.005)}   & 0.318\textbf{ (0.006)}     &0.001013\textbf{ (0.000097)} &0.498\textbf{ (0.003)}   &0.299\textbf{ (0.001)}      &0.001602\textbf{ (0.000157)} \\
    \hline
    \multirow{7}{*}{\makecell[c]{30\% \\ Zero \\ weight\\ (5 rounds)}}
    & SAN  &0.448 (0.075) &0.321\textbf{ (0.004)}  &0.001490 (0.000599)  &- & - & -   \\
    & SAN-NR  &0.454 (0.061)  &0.335 (0.005)  &0.001399 (0.000370)   &0.470 (0.017)  &0.331 (0.022)  &0.009941 (0.003088)  \\
    & DT1~\cite{hao2020biologically}    & 0.387 (0.056)  &0.313 (0.012)    &0.002045 (0.000307)  & 0.456 (0.026)  &0.334 (0.024)    &0.005103 (0.002161)    \\
    & DT2~\cite{kim2021spiking}     &0.377 (0.023)  &0.358 (0.013)    &0.001834 (0.000302)    &0.403 (0.015)  &0.332 (0.023)    &0.003469 (0.002404)   \\

    & DET only   &0.520 (0.012)  &0.387 (0.051)    &0.002582 (0.001558)  &0.356 (0.024)  &0.235 (0.041)    &0.005036 (0.002472)   \\
    & DTT only & 0.470 (0.014)  & 0.337 (0.017)        & 0.002551 (0.001649)  &0.394 (0.081)   &0.274 (0.020)         &0.003706 (0.001422) \\
    & \DTname\  &0.444\textbf{ (0.005) }  & 0.316\textbf{ (0.004)}     &0.000993\textbf{ (0.000077)}   &0.497\textbf{ (0.004)}   &0.318\textbf{ (0.020)}      &0.003855\textbf{ (0.002096)}    \\
    
    \bottomrule
  \end{tabular}
\end{table}

\begin{table}
  \caption{The raw homeostasis measurements of successful trials and the corresponding changes with respect to the baseline condition in obstacle avoidance tasks with the $T=25$ setting.}
  \label{SMtab:hom_success_25}
  \centering
  \scriptsize
  \setlength\tabcolsep{4pt}
  \begin{tabular}{llllllll}
    \toprule
     
     & & \multicolumn{3}{c}{\textbf{LIF} ($T=25$)}     & \multicolumn{3}{c}{\textbf{SRM} ($T=25$)}                \\
    \cmidrule(r){3-5}
    \cmidrule(r){6-8}
     \textbf{Type} & \textbf{Name}  & \makecell[c]{$\text{FR}_m (\Delta)$}        & \makecell[c]{$\text{FR}_{std}^m (\Delta)$}     & \makecell[c]{$\text{FR}_{std}^s (\Delta)$}         & \makecell[c]{$\text{FR}_m (\Delta)$}        & \makecell[c]{$\text{FR}_{std}^m (\Delta)$}     & \makecell[c]{$\text{FR}_{std}^s (\Delta)$}     \\ 
    \hline
    \multirow{7}{*}{\makecell[c]{Dynamic \\ obstacle \\(baseline \\condition)}}
    & SAN  &  0.524  & 0.325  &  0.002098  & 0.285  & 0.306  & 0.001504    \\
    & SAN-NR  & 0.515   & 0.331  & 0.001440  & 0.488   & 0.312  &  0.003486 \\
    & DT1~\cite{hao2020biologically}    & 0.447  & 0.324  &0.002155  & 0.485   & 0.319  & 0.002473 \\
    & DT2~\cite{kim2021spiking}     & 0.401  & 0.347  & 0.002470 & 0.420  &  0.314 & 0.005771\\

    & DET only   & 0.509  & 0.336  & 0.001206  & 0.384  & 0.279  & 0.002483\\
    & DTT only &  0.449  & 0.317   & 0.001736  & 0.475  & 0.301  & 0.002515    \\
    & \DTname\ & 0.439   & 0.311  & 0.001035  & 0.501  & 0.301  & 0.002394\\
    \hline
    \multirow{7}{*}{\makecell[c]{0.2}}
    & SAN  & 0.556 (0.032) & 0.330 (0.005)  & 0.000798 (0.001300)  & 0.294 (0.009) &  0.245 (0.061) & 0.001004 (0.000500)  \\
    & SAN-NR  &  0.566 (0.051)  & 0.326 (0.005)  & 0.000768 (0.000670)  & 0.536 (0.048)  &  0.351 (0.039) & 0.001224 (0.002260) \\
    & DT1~\cite{hao2020biologically}    & 0.481 (0.034) & 0.387 (0.063)  & 0.001097 (0.001060)   & 0.517 (0.032)  & 0.344 (0.025) & 0.003823 (0.001350) \\
    & DT2~\cite{kim2021spiking}     & 0.415 (0.014)  & 0.370 (0.023)   & 0.001662 (0.000810)  & 0.438 (0.018)  & 0.326 (0.012)  & 0.001781 (0.003990) \\

    & DET only   &0.496 (0.013)  &  0.353 (0.017) & 0.001424 (0.000218)  &  0.380 (0.004) & 0.246 (0.033)  &  0.003362 (0.000879) \\
    & DTT only &  0.485 (0.036)  & 0.336 (0.019)  & 0.000972 (0.000760)  & 0.420 (0.055)  & 0.335 (0.034)  &  0.003116 (0.000601) \\
    & \DTname\  & 0.444\textbf{ (0.005)} & 0.314\textbf{ (0.003)}   & 0.001104\textbf{ (0.000069)}  & 0.494\textbf{ (0.007)}  &  0.310\textbf{ (0.010)} &  0.002238\textbf{ (0.000160)}\\
    \hline
    \multirow{7}{*}{\makecell[c]{6.0}}
    & SAN  & 0.558 (0.034) & 0.341 (0.016)  & 0.001415 (0.000683)  & 0.275 (0.010)  & 0.303 (0.003)  & 0.000839 (0.000665) \\
    & SAN-NR  &0.550 (0.035)  & 0.340 (0.009)  & 0.001165 (0.000275)  & 0.484 (0.004)  & 0.306 (0.006)  &  0.003828 (0.000342)  \\
    & DT1~\cite{hao2020biologically}    &0.433 (0.014) & 0.319\textbf{ (0.005)}  & 0.002449 (0.000294)  & 0.471 (0.014)  &  0.315 (0.004) & 0.003621 (0.001148)\\
    & DT2~\cite{kim2021spiking}    & 0.406 (0.005)  & 0.353 (0.006)  & 0.003206 (0.000736)  & 0.406 (0.014)  &  0.320 (0.006) & 0.005094 (0.000667) \\

    & DET only   &0.516 (0.007)  &0.374 (0.038)   & 0.003172 (0.001966)  & 0.377 (0.007)  & 0.241 (0.038)  & 0.003248 (0.000765) \\
    & DTT only & 0.450 (0.001)  &  0.327 (0.010) & 0.002744 (0.001008)  & 0.413 (0.062)  & 0.289 (0.012)  &  0.002742 (0.000227)\\
    & \DTname\  &0.440\textbf{ (0.001)}  & 0.316\textbf{ (0.005)}  &  0.001247\textbf{ (0.000212)} & 0.501\textbf{ (0.000)}  & 0.300\textbf{ (0.001)}  &0.002092\textbf{ (0.000302)} \\
    \hline
    \multirow{7}{*}{\makecell[c]{GN}}
    & SAN  & 0.538 (0.014)  & 0.311 (0.014)  & 0.002522 (0.000424)  & 0.288\textbf{ (0.003)}  & 0.209 (0.097)  & 0.000883 (0.000621) \\
    & SAN-NR  & 0.530 (0.015)   & 0.318 (0.013)  &  0.003055 (0.001615) &0.503 (0.015)   & 0.299 (0.013)  & 0.005029 (0.001543)\\
    & DT1~\cite{hao2020biologically}    &0.452 (0.005)  & 0.319\textbf{ (0.005)}  &  0.001408 (0.000747) & 0.502 (0.017)  &0.302 (0.017)   &  0.004470 (0.001997)\\
    & DT2~\cite{kim2021spiking}     & 0.405\textbf{ (0.004)}  & 0.336 (0.011)  & 0.002005 (0.000465)  & 0.423\textbf{ (0.003)}  &0.283 (0.031)  &0.005235 (0.000536) \\

    & DET only   & 0.500 (0.009) & 0.367 (0.031)  & 0.001424 (0.000218)  & 0.392 (0.008)   & 0.286 (0.007)  & 0.003130 (0.000647) \\
    & DTT only & 0.445 (0.004)   &  0.311 (0.006) & 0.001260 (0.000476)  & 0.401 (0.074)  & 0.310 (0.009)  & 0.001795 (0.000720) \\
    & \DTname\  & 0.443\textbf{ (0.004)} &  0.306\textbf{ (0.005)}  & 0.001085\textbf{ (0.000050)}  & 0.498\textbf{ (0.003)}  &  0.301\textbf{ (0.000)}  &  0.001962\textbf{ (0.000432)} \\
    \hline
    \multirow{7}{*}{\makecell[c]{8-bit \\ Loihi \\ weight}}
    & SAN  & 0.519 (0.005)   &  0.319 (0.006) & 0.001106 (0.000992)  & 0.290 (0.005)  & 0.315 (0.009)  & 0.000961 (0.000543) \\
    & SAN-NR  & 0.510 (0.005)   & 0.336 (0.005)  & 0.001153 (0.000287)  & 0.478 (0.010)  &  0.317 (0.005) &  0.005220 (0.001734) \\
    & DT1~\cite{hao2020biologically}    & 0.435 (0.012) & 0.318 (0.006)  & 0.001467 (0.000688)  & 0.472 (0.013)  & 0.327 (0.008)  & 0.001854 (0.000619)\\
    & DT2~\cite{kim2021spiking}     & 0.411 (0.010)  & 0.339 (0.008)  &  0.001802 (0.000668) & 0.428 (0.008)  &  0.317\textbf{ (0.003)} &0.005032 (0.000739) \\

    & DET only   & 0.504 (0.005) & 0.341 (0.005)  & 0.000924 (0.000282)  & 0.387 (0.003)  & 0.288 (0.009)  & 0.002816 (0.000333) \\
    & DTT only & 0.446 (0.003)   & 0.327 (0.010)  & 0.001302 (0.000434)  & 0.462 (0.013)   &  0.303 (0.002)  & 0.002038 (0.000477) \\
    & \DTname\  & 0.439\textbf{ (0.000)} & 0.308\textbf{ (0.003)}  & 0.001107\textbf{ (0.000072)} &  0.502\textbf{ (0.001)}  & 0.297 (0.004) & 0.002164\textbf{ (0.000230)} \\
    \hline
    \multirow{7}{*}{\makecell[c]{GN \\ weight \\  (5 rounds)}}
    & SAN  & 0.503 (0.021)  & 0.340 (0.015)  & 0.001241 (0.000857)  &  - &  - &  -\\
    & SAN-NR  & 0.488 (0.027)   & 0.340 (0.009)  & 0.001796 (0.000356)  & 0.499 (0.011)   & 0.328 (0.016)  & 0.004204 (0.000718) \\
    & DT1~\cite{hao2020biologically}    & 0.413 (0.034)  &0.346 (0.022)   & 0.002318 (0.000163)  & 0.491 (0.006)  & 0.320\textbf{ (0.001)}   &  0.003065 (0.000592)\\
    & DT2~\cite{kim2021spiking}     & 0.390 (0.011) & 0.336 (0.011)  &  0.001382 (0.001088) & 0.411 (0.007)  & 0.292 (0.017)  &0.008895 (0.003124)  \\

    & DET only   & 0.516 (0.007)  & 0.372 (0.036)  & 0.002643 (0.001437)  & 0.397 (0.013)  & 0.218 (0.061)  & 0.003384 (0.000901) \\
    & DTT only & 0.467 (0.018)  & 0.328 (0.011)  & 0.001352 (0.000384)  & 0.393 (0.082)  &  0.303 (0.002)  & 0.003581 (0.001066) \\
    & \DTname\  & 0.444\textbf{ (0.005)} & 0.318\textbf{ (0.007)}  & 0.001163\textbf{ (0.000128)}  & 0.498\textbf{ (0.003)}  & 0.300\textbf{ (0.001)}  & 0.001923\textbf{ (0.000471)}\\
    \hline
    \multirow{7}{*}{\makecell[c]{30\% \\ Zero \\ weight\\ (5 rounds)}}
    & SAN  & 0.443 (0.081) & 0.320\textbf{ (0.005)}  & 0.000862 (0.001236)  & -  &-   & -\\
    & SAN-NR  &0.457 (0.058)    & 0.338 (0.007)   & 0.002461 (0.001021)  & 0.472 (0.016)  &  0.332 (0.020)  &  0.009380 (0.005894)\\
    & DT1~\cite{hao2020biologically}    & 0.388 (0.059) & 0.312 (0.012)  & 0.001257 (0.000898)  & 0.456 (0.029)  & 0.334\textbf{ (0.015)} & 0.005820 (0.003347) \\
    & DT2~\cite{kim2021spiking}     &0.372 (0.029)  &  0.359 (0.012) & 0.001930 (0.000540)  &  0.403 (0.017) & 0.332 (0.018)  & 0.003060 (0.002711) \\

    & DET only   &0.524 (0.015)  & 0.368 (0.032)  &  0.002974 (0.001786) & 0.360 (0.024)  & 0.245 (0.034)  & 0.004378 (0.001895) \\
    & DTT only & 0.472 (0.023)  & 0.334 (0.017)  &  0.002013 (0.000277) & 0.402 (0.073)  & 0.280 (0.021) &0.004420 (0.001905) \\
    & \DTname\  & 0.446\textbf{ (0.007)} & 0.316\textbf{ (0.005)}  &  0.001502\textbf{ (0.000467)} & 0.488\textbf{ (0.013)}  &  0.316\textbf{ (0.015)} &0.004638\textbf{ (0.002244)} \\

    \bottomrule
  \end{tabular}
\end{table}

\subsection*{Assessment---Ablation Studies}
We conduct ablation studies to validate the effectiveness of the DET and DTT components of the proposed \DTname. The results obtained under different degraded conditions are reported in the rows named ``DET only'' and ``DTT only'' in Tables~\ref{SMtab:Sta_test}, ~\ref{SMtab:Degraded environment}, ~\ref{SMtab:Degraded inputs}, and ~\ref{SMtab:Weight pollution}. The ablation study results are also illustrated in Figure~\ref{fig:SN_OA_results}. All listed evaluations validate that the \DTname\ scheme performs better than any single component. The dynamic threshold scheme with only one component cannot effectively regulate the firing rate statuses of the host SNNs, prohibiting meaningful homeostasis. One extreme example is illustrated in Figure~\ref{fig:SN_OA_results}f. The $\Delta\text{FR}_{m}$ changes induced under the `DTT only' setting are the largest among all competing approaches under all experimental conditions. Notably, when combined with the other component, the proposed \DTname\ provides the strongest homeostasis for the host SNNs. This validates the biologically observed positive correlation encoded by the DET and the negative correlation enforced by the DTT, which are equally essential for effectively maintaining the homeostasis of an SNN.
