# Supplementary material for: Biologically Inspired Dynamic Thresholds for Spiking Neural Networks
Source: arXiv:2206.04426 source file (2023-06-19)
Supplement: Supplementary file 7 [file approach.tex]

\noindent
A typical biological neuron has four morphological regions: a cell body, dendrites, an axon, and synaptic terminals. Inside the cell body (\ie the soma), a nuclear envelope contains the cell's genes. The short tree-like dendrites branch out from the cell body, and they are the main apparatus for receiving incoming signals from other neurons. The long tubular axon covered by the myelin sheath extends some distance from the cell body and carries action potential to other neurons through synaptic terminals. A typical nerve neuron is illustrated in Figure~\ref{fig:pipeline}a. 

\noindent
In a nerve cell that is at rest, the extracellular surface of the cell membrane has an excess positive charge, while the cytoplasmic side has an excess negative charge. The cell membrane maintains the separation of charge as a barrier against the diffusion of ions; see Figure~\ref{fig:pipeline}b. The electrical potential difference across the membrane is defined as the membrane potential, which has three different statuses: resting, depolarization, and hyperpolarization. At rest, no net charge movement across the membrane occurs, and the resting membrane potential is maintained. By convention, the potential outside the cell is defined as zero, and hence, the resting potential is a negative value. A net flow of cations or anions into or out of a cell disturbs the resting membrane, causing depolarization or hyperpolarization, respectively. Depolarization indicates less negative membrane potential, while hyperpolarization signifies more negative potential; see Figure~\ref{fig:pipeline}c.

\begin{figure}[t]
	\centering
	\includegraphics [scale=0.237]{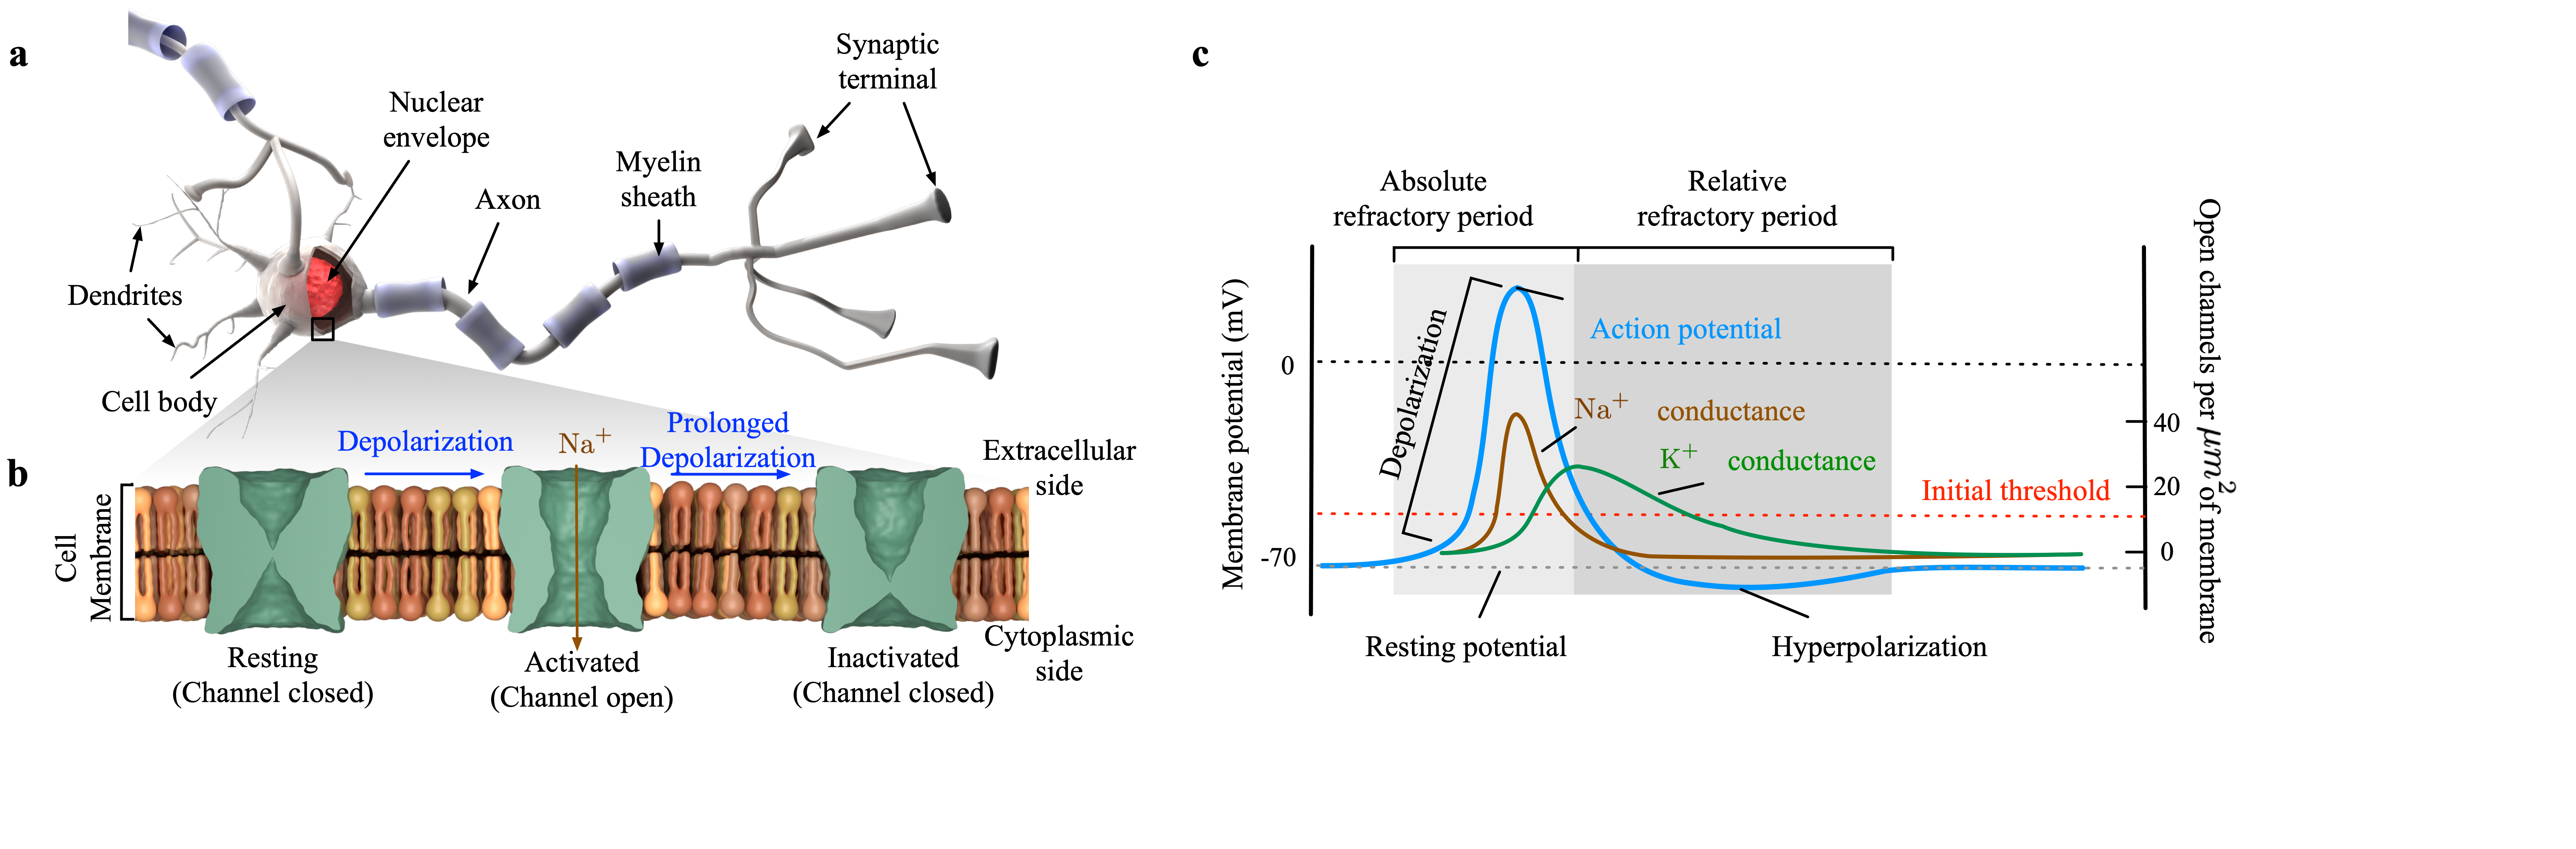}
% 	\vspace{-0.4cm}
	\caption{
		a. The structure of a neuron. b. We demonstrate a sodium ($\text{Na}^+$) voltage-gated channel under resting, activated, and inactivated (refractory) states. The $\text{Na}^+$ channel enters an inactivated state after depolarization and returns to a resting state only after the membrane potential is restored to its resting potential. c. The process of action potential generation, which is based on the Hodgkin-Huxley model~\cite{Hodgkin1952}, involves the sequential opening of voltage-gated Na$^+$ and K$^+$ channels. The Na$^+$ and K$^+$ conductance curves are adapted from the Hodgkin-Kuxley model~\cite{Hodgkin1952}.
	}
	\label{fig:pipeline}
% 	\vspace{-0.4cm}
\end{figure}

\subsection*{Dynamic Thresholds in Biological Neurons}
The Hodgkin-Huxley model~\cite{Hodgkin1952} 
\bd{has served as an archetype for compartmental models of the electrophysiology of biological membranes (see Figure~\ref{fig:pipeline}a). Many numerical methods leverage the Hodgkin-Huxley model as their testbeds, which can be applied to more complex models~\cite{azouz2000dynamic, TanAndrew:2014:nature, HHstillstanding2007:nature}. We use the Hodgkin-Huxley model to introduce the concept of threshold in biological neurons. }
Based on the Hodgkin-Huxley model, an action potential is produced when the membrane potential is higher than a particular threshold; this involves the following sequence of processes. First, when the membrane potential is higher than a threshold, the associated depolarization opens sodium ($\text{Na}^+$) channels, resulting in an inward $\text{Na}^+$ current. By discharging the membrane capacitance, the inward current causes further depolarization and the opening of more $\text{Na}^+$ channels, resulting in a further increase in the inward current. Second, under prolonged depolarization, the voltage-gated $\text{Na}^+$ channels become inactive. Furthermore, after some delay, the voltage-gated potassium ($\text{K}^+$) channels begin to open, causing an outward $\text{K}^+$ current that tends to repolarize the membrane (see Figure~\ref{fig:pipeline}b). The second process underlies the absolute refractory period~\cite{tackmann1974refractory}, a period during which no action potential can be elicited. After that, with some $\text{K}^+$ channels being closed and some $\text{Na}^+$ channels recovering from inactivation, the membrane enters a relative refractory period~\cite{tackmann1974refractory} (see Figure~\ref{fig:pipeline}c). During this period, it is possible to trigger an action potential, but this requires a higher threshold. 
%See Supplementary Note 3 for related concepts.

\noindent
Note that a small subthreshold depolarization cannot trigger an action potential, as it not only increases the inward $\text{Na}^+$ current but also increases the outward $\text{K}^+$ current~\cite{Hodgkin1952}. Only at a specific membrane potential value does the net ionic current become inward, depositing a net positive charge on the inside of the membrane capacitance. This specific value is the potential (or spike) threshold~\cite{kandel:neural}.

\noindent
\bd{The threshold changes dynamically, widely observed in the different nervous systems~\cite{zhang2003the,cooper2012the,fontaine2014spike,azouz2000dynamic,yeung2004synaptic,sun2009experience,pozo2010unraveling,pena2002postsynaptic,azouz2003adaptive}. A thread of studies leverage the Hodgkin-Huxley model to verify the observed threshold dynamics~\cite{platkiewicz2010threshold, azouz2000dynamic}. However, not all spike initiation dynamics of biological neurons can be accurately described by the Hodgkin-Huxley model~\cite{Naundorf:2006:nature}.}
