# Supplementary material for: Biologically Inspired Dynamic Thresholds for Spiking Neural Networks
Source: arXiv:2206.04426 source file (2023-06-19)
Supplement: Supplementary file 8 [file impact_0.2.tex]

\noindent
In the proposed DET component, a constant `0.2' is used for balancing the contributions of the specifically designed bias items, \ie $0.2(\max(v_i^{l}(t)) - \min(v_i^{l}(t)))$ and $0.2(\max(\Theta_i^{l}(t)) - \min(\Theta_i^{l}(t)))$.

\noindent
Based on our experimental results, the effectiveness of the proposed \DTname\ is not sensitive to this value. In the obstacle avoidance tasks (see Tables~\ref{tab:0.2 OA DO}, ~\ref{tab:0.2 OA DI}, and ~\ref{tab:0.2 OA WU}), when the constant value is within the range of $[0.1, 0.5]$, the standard deviations of the SRs for the LIF- and SRM-based host SNNs are $0.005$ and $0.007$, respectively. More importantly, even with an extreme value of $1.0$, the corresponding SRs are higher than those offered by all other competing dynamic threshold approaches.

\noindent
In the HalfCheetah-v3 tasks (see Tables~\ref{tab:0.2 HC normal}, ~\ref{tab:0.2 HC DI}, and ~\ref{tab:0.2 HC WU}) and the Ant-v3 tasks (see Table~\ref{tab:0.2 Ant normal}, ~\ref{tab:0.2 Ant DI}, and ~\ref{tab:0.2 Ant WU}), the proposed \DTname\ method is more sensitive to the coefficient value than in the obstacle avoidance tasks. When the constant value is within the range of $[0.1, 0.5]$, the standard deviations of the rewards are $94$ and $107$ for the LIF- and SRM-based host SNNs in the HalfCheetah-v3 tasks, respectively. In the Ant-v3 experiments, the LIF- and SRM-based SNNs provide rewards of $114$ and $111$, respectively. With the extreme value of 1.0, under some experimental conditions, the rewards offered by our approach are still higher than those provided by other methods (e.g., the ``30\% zero weight" condition of HalfCheetah-v3 and the ``GN weight" condition of Ant-v3). However, with the extreme value of $1.0$, the effectiveness of the proposed \DTname\ scheme is reduced. This means that the sensitivity to the constant value increases as the complexity of the given task increases. 

\noindent
Note that the value of `0.2' offers the most effective and robust performance across all three tasks under all experimental conditions. Therefore, we set the coefficient to `0.2' in our proposed dynamic threshold scheme.

%%%%%%%%%%%%%%%%%%%%%%%%%%%% 0.2 begin OA %%%%%%%%%%%%%%%%%%%%%%%%%%%%%%
\begin{table}
\vspace{-0.5cm}
\centering
 \caption{Quantitative performance of obstacle avoidance tasks with different constant coefficient settings under static obstacle condition.}

  \vspace{0.2cm}
  \label{tab:0.2 OA SO}

  \centering
  \small
  \setlength\tabcolsep{2pt}
  \begin{tabular}{lll}
    \toprule
     
     & \multicolumn{1}{c}{\textbf{LIF} ($T=5$)}     & \multicolumn{1}{c}{\textbf{SRM} ($T=5$)}                \\
    \cmidrule(r){2-2}
    \cmidrule(r){3-3}
     \textbf{Constant}  & \makecell[c]{SR$\uparrow$}      &  \makecell[c]{SR$\uparrow$}      \\
    \hline
    0.1  & \makecell[c]{97.5\%}      & \makecell[c]{\textbf{96.5\%}}  \\

    0.2(original)  & \makecell[c]{\textbf{98.5\%}}         & \makecell[c]{\textbf{96.5\%}} \\
    0.3  &  \makecell[c]{\textbf{98.5\%}}    &  \makecell[c]{\textbf{96.5\%}}    \\
    % DT3~\cite{sengupta2019going}   & 49.93    & 19.27   & 63.5\%  & 51.35 & 19.23 & 52.5\%  \\
    % \hline
    0.4  & \makecell[c]{97.5\%}    &  \makecell[c]{95.5\%} \\
    0.5  & \makecell[c]{98\%}      &   \makecell[c]{95\%}  \\
    % \hline
    1.0   &  \makecell[c]{93.5\%}  &  \makecell[c]{91.5\%}\\
    \bottomrule
  \end{tabular}
%   \vspace{-0.3cm}
\end{table}

\begin{table}
\vspace{-0.2cm}
\centering
 \caption{Quantitative performance of obstacle avoidance tasks with different constant coefficient settings under dynamic obstacle condition.}

  \vspace{0.2cm}
  \label{tab:0.2 OA DO}

  \centering
  \small
  \setlength\tabcolsep{2pt}
  \begin{tabular}{lll}
    \toprule
     
     & \multicolumn{1}{c}{\textbf{LIF} ($T=5$)}     & \multicolumn{1}{c}{\textbf{SRM} ($T=5$)}                \\
    \cmidrule(r){2-2}
    \cmidrule(r){3-3}
     \textbf{Constant}  & \makecell[c]{SR$\uparrow$}      &  \makecell[c]{SR$\uparrow$}      \\
    \hline
    0.1  & \makecell[c]{91.5\%}      & \makecell[c]{\textbf{90.5\%}}   \\

    0.2(original)  & \makecell[c]{\textbf{92.5\%}}         & \makecell[c]{\textbf{90.5\%}} \\
    0.3  &  \makecell[c]{92\%}    &  \makecell[c]{90\%}    \\
    % DT3~\cite{sengupta2019going}   & 49.93    & 19.27   & 63.5\%  & 51.35 & 19.23 & 52.5\%  \\
    % \hline
    0.4  & \makecell[c]{92\%}    &  \makecell[c]{89\%} \\
    0.5  & \makecell[c]{91\%}      &   \makecell[c]{89\%}  \\
    % \hline
    1.0   &  \makecell[c]{86\%}  &  \makecell[c]{80.5\%}\\
    \bottomrule
  \end{tabular}
  \vspace{-0.3cm}
\end{table}

\begin{table}
\vspace{-0.3cm}
    \caption{Quantitative performance of obstacle avoidance tasks with different constant coefficient settings under degraded input conditions.}
  \label{tab:0.2 OA DI}
  \centering
  \scriptsize
  \setlength\tabcolsep{1pt}
  \begin{tabular}{llllllllllll}
    \toprule
     
     & & \multicolumn{1}{c}{\textbf{LIF} ($T=5$)}     & \multicolumn{1}{c}{\textbf{SRM} ($T=5$)}  & & & \multicolumn{1}{c}{\textbf{LIF} ($T=5$)}     & \multicolumn{1}{c}{\textbf{SRM} ($T=5$)}  & & & \multicolumn{1}{c}{\textbf{LIF} ($T=5$)}     & \multicolumn{1}{c}{\textbf{SRM} ($T=5$)}            \\
    \cmidrule(r){3-3}
    \cmidrule(r){4-4}
    \cmidrule(r){7-7}
    \cmidrule(r){8-8}
    \cmidrule(r){11-11}
    \cmidrule(r){12-12}
      \textbf{Type} & \textbf{Constant}  & \makecell[c]{SR$\uparrow$}        &  \makecell[c]{SR$\uparrow$}    &\textbf{ Type} & \textbf{Constant}  & \makecell[c]{SR$\uparrow$}        &  \makecell[c]{SR$\uparrow$}    &\textbf{ Type} & \textbf{Constant}  & \makecell[c]{SR$\uparrow$}  &  \makecell[c]{SR$\uparrow$} 
      \\
    \hline
    \makecell[c]{\multirow{7}{*}{\makecell[c]{0.2}}}
    & 0.1  & \makecell[c]{89\%}    & \makecell[c]{78\%}   & \makecell[c]{\multirow{6}{*}{\makecell[c]{0.6}}}   & 0.1  & \makecell[c]{83.5\%}   & \makecell[c]{82\%} &
  \makecell[c]{\multirow{6}{*}{GN}} & 
    0.1 & \makecell[c]{83.5\%}   & \makecell[c]{82\%}   \\
    & 0.2(original)   & \textbf{\makecell[c]{90\%}}      & \makecell[c]{\textbf{79.5\%}}   & & 0.2(original)    & \textbf{\makecell[c]{84.5\%}}      & \textbf{\makecell[c]{83\%}} 
    & & 0.2(original)    & \textbf{\makecell[c]{84.5\%}}       & \makecell[c]{\textbf{82.5\%}}\\
    & 0.3 & \makecell[c]{89\%}   & \makecell[c]{77.5\%}  & &  0.3  & \makecell[c]{83\%}       &  \makecell[c]{81.5\%} 
    & & 0.3  &   \makecell[c]{84\%}    &   \makecell[c]{82\%}   \\

    & 0.4  & \makecell[c]{87\%}    & \makecell[c]{75\%}    & & 0.4  & \makecell[c]{82\%}      & \makecell[c]{79\%}    & & 0.4  & \makecell[c]{84\%}     & \makecell[c]{81.5\%}   \\
    & 0.5  & \makecell[c]{87.5\%}      & \makecell[c]{75\%}  & & 0.5  & \makecell[c]{81.5\%}       & \makecell[c]{80.5\%}    &  & 0.5   & \makecell[c]{83\%}      & \makecell[c]{81\%} \\

    & 1.0   & \makecell[c]{83.5\%}    & \makecell[c]{70.5\%}   & & 1.0   & \makecell[c]{76\%}      & \makecell[c]{76.5\%}
    & & 1.0   & \makecell[c]{77\%}     & \makecell[c]{70.5\%}\\
    \bottomrule
  \end{tabular}
\vspace{-0.3cm}
\end{table}

\begin{table}
\vspace{-0.3cm}
    \caption{Quantitative performance of obstacle avoidance tasks with different constant coefficient settings under weight uncertainty conditions.}
  \label{tab:0.2 OA WU}
  \centering
  \scriptsize
  \setlength\tabcolsep{0.2pt}
  \begin{tabular}{llllllllllll}
    \toprule
     
     & & \multicolumn{1}{c}{\textbf{LIF} ($T=5$)}     & \multicolumn{1}{c}{\textbf{SRM} ($T=5$)}  & & & \multicolumn{1}{c}{\textbf{LIF} ($T=5$)}     & \multicolumn{1}{c}{\textbf{SRM} ($T=5$)}  & & & \multicolumn{1}{c}{\textbf{LIF} ($T=5$)}     & \multicolumn{1}{c}{\textbf{SRM} ($T=5$)}            \\
    \cmidrule(r){3-3}
    \cmidrule(r){4-4}
    \cmidrule(r){7-7}
    \cmidrule(r){8-8}
    \cmidrule(r){11-11}
    \cmidrule(r){12-12}
      \textbf{Type} & \textbf{Constant}  & \makecell[c]{SR$\uparrow$}        &  \makecell[c]{SR$\uparrow$}    &\textbf{ Type} & \textbf{Constant}  & \makecell[c]{SR$\uparrow$}        &  \makecell[c]{SR$\uparrow$}    &\textbf{ Type} & \textbf{Constant}  & \makecell[c]{SR$\uparrow$}  &  \makecell[c]{SR$\uparrow$} 
      \\
    \hline
    \multirow{6}{*}{\makecell[c]{8-bit \\ Loihi \\ weight}}
    & 0.1  & \makecell[c]{89.5\%}         & \makecell[c]{87.5\%}   & \multirow{6}{*}{\makecell[c]{GN \\ weight \\ (5 rounds)}}
    & 0.1  & \makecell[c]{87.2\%}  &  \makecell[c]{60.5\%}   &
    \multirow{6}{*}{\makecell[c]{ $30\%$ \\ Zero \\ weight \\ (5 rounds)}}
    & 0.1  & \makecell[c]{\textbf{77.2\%}}        & \makecell[c]{64.0\%}    \\
    & 0.2(original)   & \textbf{\makecell[c]{90\%}}      & \makecell[c]{\textbf{88.5\%}}     & & 0.2(original)     & \textbf{\makecell[c]{87.7\%}}      & \textbf{\makecell[c]{61.8\%}}      & & 0.2(original)    & \textbf{\makecell[c]{77.2\%}}       & \makecell[c]{\textbf{65.2\%}}  \\
    & 0.3 & \makecell[c]{\textbf{90\%}}   & \makecell[c]{88\%}  & &  0.3  & \makecell[c]{86.3\%}       &  \makecell[c]{60.0\%} 
    & & 0.3  &   \makecell[c]{75.8\%}    &   \makecell[c]{64.2\%}   \\

    & 0.4 & \makecell[c]{88.5\%}    & \makecell[c]{88\%}    & & 0.4  & \makecell[c]{85.7\%}      & \makecell[c]{58.6\%}    & & 0.4  & \makecell[c]{74.3\%}     & \makecell[c]{63.5\%}   \\
    & 0.5  & \makecell[c]{87.5\%}      & \makecell[c]{87\%}  & & 0.5   & \makecell[c]{84.1\%}       & \makecell[c]{57.4\%}    &  & 0.5    & \makecell[c]{72.8\%}      & \makecell[c]{83.6\%} \\ 
    & 1.0   & \makecell[c]{83\%}       & \makecell[c]{79.5\%}           & & 1.0  & \makecell[c]{80.3\%}       & \makecell[c]{52.3\%}   & & 1.0 & \makecell[c]{67.1\%}       & \makecell[c]{52.9\%  }  \\
    \bottomrule
  \end{tabular}
% \vspace{-0.3cm}
\end{table}

%%%%%%%%%%%%%%%%%%%%%%%%%%%% 0.2 end %%%%%%%%%%%%%%%%%%%%%%%%%%%%%%

%%%%%%%%%%%%%%%%%%%%%% HalfCheetah-v3 0.2 %%%%%%%%%%%%%%%%%%%%%%%%%%%%%%%%%%%

\begin{table}
\vspace{-0.3cm}
\centering
 \caption{Quantitative performance of HalfCheetah-v3 tasks with different constant coefficient settings under standard testing conditions.}

  \vspace{0.2cm}
  \label{tab:0.2 HC normal}

  \centering
  \small
  \setlength\tabcolsep{2pt}
  \begin{tabular}{lll}
    \toprule
     
     & \multicolumn{1}{c}{\textbf{LIF} ($T=5$)}     & \multicolumn{1}{c}{\textbf{SRM} ($T=5$)}                \\
    \cmidrule(r){2-2}
    \cmidrule(r){3-3}
     \textbf{Constant}  & \makecell[c]{Reward$\uparrow$}      &  \makecell[c]{Reward$\uparrow$}      \\
    \hline
    0.1  & \makecell[c]{11029}      & \makecell[c]{11903}   \\

    0.2(original)  & \makecell[c]{\textbf{11064}}         & \makecell[c]{\textbf{11960}} \\
    0.3  &  \makecell[c]{10987}    &  \makecell[c]{11875}    \\
    % DT3~\cite{sengupta2019going}   & 49.93    & 19.27   & 63.5\%  & 51.35 & 19.23 & 52.5\%  \\
    % \hline
    0.4  & \makecell[c]{10976}    &  \makecell[c]{11682} \\
    0.5  & \makecell[c]{10793}      &   \makecell[c]{11724}  \\
    % \hline
    1.0   &  \makecell[c]{10028}  &  \makecell[c]{11123}\\
    \bottomrule
  \end{tabular}
%   \vspace{-0.3cm}
\end{table}

\begin{table}
\vspace{-0.3cm}
    \caption{Quantitative performance of HalfCheetah-v3 tasks with different constant coefficient settings under degraded input conditions.}
  \label{tab:0.2 HC DI}
  \centering
  \scriptsize
  \setlength\tabcolsep{1pt}
  \begin{tabular}{llllllllllll}
    \toprule
     
     & & \multicolumn{1}{c}{\textbf{LIF} ($T=5$)}     & \multicolumn{1}{c}{\textbf{SRM} ($T=5$)}  & & & \multicolumn{1}{c}{\textbf{LIF} ($T=5$)}     & \multicolumn{1}{c}{\textbf{SRM} ($T=5$)}  & & & \multicolumn{1}{c}{\textbf{LIF} ($T=5$)}     & \multicolumn{1}{c}{\textbf{SRM} ($T=5$)}            \\
    \cmidrule(r){3-3}
    \cmidrule(r){4-4}
    \cmidrule(r){7-7}
    \cmidrule(r){8-8}
    \cmidrule(r){11-11}
    \cmidrule(r){12-12}
      \textbf{Type} & \textbf{Constant}  & \makecell[c]{Reward$\uparrow$}        &  \makecell[c]{Reward$\uparrow$}    &\textbf{ Type} & \textbf{Constant}  & \makecell[c]{Reward$\uparrow$}        &  \makecell[c]{Reward$\uparrow$}    &\textbf{ Type} & \textbf{Constant}  & \makecell[c]{Reward$\uparrow$}  &  \makecell[c]{Reward$\uparrow$} 
      \\
    \hline
    \makecell[c]{\multirow{7}{*}{\makecell[c]{Random \\ joint \\ position}}}
    & 0.1  & \makecell[c]{8379}    & \makecell[c]{7767}   & \makecell[c]{\multirow{6}{*}{\makecell[c]{Random \\ joint \\ velocity}}}   & 0.1  & \makecell[c]{8241}   & \makecell[c]{7023} &
  \makecell[c]{\multirow{6}{*}{GN}} &
    0.1 & \makecell[c]{3832}   & \makecell[c]{3825}   \\
    & 0.2(original)   & \textbf{\makecell[c]{8465}}      & \makecell[c]{\textbf{7883}}   & & 0.2(original)    & \textbf{\makecell[c]{8302}}      & \textbf{\makecell[c]{7116}} 
    & & 0.2(original)    & \textbf{\makecell[c]{3909}}       & \makecell[c]{\textbf{3895}}\\
    & 0.3 & \makecell[c]{8302}   & \makecell[c]{7748}  & &  0.3  & \makecell[c]{8159}       &  \makecell[c]{6968} 
    & & 0.3  &   \makecell[c]{3790}    &   \makecell[c]{3810}   \\

    & 0.4  & \makecell[c]{8351}    & \makecell[c]{7703}    & & 0.4  & \makecell[c]{8113}      & \makecell[c]{6743}    & & 0.4  & \makecell[c]{3673}     & \makecell[c]{3724}   \\
    & 0.5  & \makecell[c]{8188}      & \makecell[c]{7615}  & & 0.5  & \makecell[c]{8044}       & \makecell[c]{6702}    &  & 0.5   & \makecell[c]{3711}      & \makecell[c]{3641} \\

    & 1.0   & \makecell[c]{7580}    & \makecell[c]{7180}   & & 1.0   & \makecell[c]{7702}      & \makecell[c]{6231}
    & & 1.0   & \makecell[c]{3420}     & \makecell[c]{3172}\\
    \bottomrule
  \end{tabular}
% \vspace{-0.3cm}
\end{table}

\begin{table}
\vspace{-0.3cm}
    \caption{Quantitative performance of HalfCheetah-v3 tasks with different constant coefficient settings under weight uncertainty conditions.}
  \label{tab:0.2 HC WU}
  \centering
  \scriptsize
  \setlength\tabcolsep{1pt}
  \begin{tabular}{llllllllllll}
    \toprule
     
     & & \multicolumn{1}{c}{\textbf{LIF} ($T=5$)}     & \multicolumn{1}{c}{\textbf{SRM} ($T=5$)}  & & & \multicolumn{1}{c}{\textbf{LIF} ($T=5$)}     & \multicolumn{1}{c}{\textbf{SRM} ($T=5$)}  & & & \multicolumn{1}{c}{\textbf{LIF} ($T=5$)}     & \multicolumn{1}{c}{\textbf{SRM} ($T=5$)}            \\
    \cmidrule(r){3-3}
    \cmidrule(r){4-4}
    \cmidrule(r){7-7}
    \cmidrule(r){8-8}
    \cmidrule(r){11-11}
    \cmidrule(r){12-12}
      \textbf{Type} & \textbf{Constant}  & \makecell[c]{Reward$\uparrow$}        &  \makecell[c]{Reward$\uparrow$}    &\textbf{ Type} & \textbf{Constant}  & \makecell[c]{Reward$\uparrow$}        &  \makecell[c]{Reward$\uparrow$}    &\textbf{ Type} & \textbf{Constant}  & \makecell[c]{Reward$\uparrow$}  &  \makecell[c]{Reward$\uparrow$} 
      \\
    \hline
    \multirow{7}{*}{\makecell[c]{8-bit \\ Loihi \\ weight}}
    & 0.1  & \makecell[c]{10780}         & \makecell[c]{11624}   & \multirow{7}{*}{\makecell[c]{GN \\ weight}}
    & 0.1  & \makecell[c]{6798}  &  \makecell[c]{8142}   &
    \multirow{7}{*}{\makecell[c]{ $30\%$ \\ Zero \\ weight}}
    & 0.1  & \makecell[c]{6428}        & \makecell[c]{5250}    \\
    & 0.2(original)   & \textbf{\makecell[c]{10823}}      & \makecell[c]{\textbf{11767}}     & & 0.2(original)     & \textbf{\makecell[c]{6928}}      & \textbf{\makecell[c]{8381}}      & & 0.2(original)    & \textbf{\makecell[c]{6551}}       & \makecell[c]{\textbf{5386}}  \\
    & 0.3 & \makecell[c]{10672}   & \makecell[c]{11584}  & &  0.3  & \makecell[c]{6920}       &  \makecell[c]{8077} 
    & & 0.3  &   \makecell[c]{6531}    &   \makecell[c]{5188}   \\

    & 0.4 & \makecell[c]{10658}    & \makecell[c]{11467}    & & 0.4  & \makecell[c]{6818}      & \makecell[c]{7936}    & & 0.4  & \makecell[c]{6286}     & \makecell[c]{5102}   \\
    & 0.5  & \makecell[c]{10583}      & \makecell[c]{11385}  & & 0.5   & \makecell[c]{6674}       & \makecell[c]{7769}    &  & 0.5    & \makecell[c]{6290}      & \makecell[c]{4975} \\ 
    & 1.0   & \makecell[c]{9757}       & \makecell[c]{10648}           & & 1.0  & \makecell[c]{6113}       & \makecell[c]{7019}   & & 1.0 & \makecell[c]{5680}       & \makecell[c]{4562}  \\
    \bottomrule
  \end{tabular}
% \vspace{-0.3cm}
\end{table}

%%%%%%%%%%%%%%%%%%%%%% HalfCheetah-v3 0.2 end %%%%%%%%%%%%%%%%%%%%%%%%%%%%%%%%%%%

%%%%%%%%%%%%%%%%%%%%%% Ant-v3 0.2 %%%%%%%%%%%%%%%%%%%%%%%%%%%%%%%%%%%

\begin{table}
\vspace{-0.3cm}
\centering
 \caption{Quantitative performance of Ant-v3 tasks with different constant coefficient settings under standard testing conditions.}

  \vspace{0.2cm}
  \label{tab:0.2 Ant normal}

  \centering
  \small
  \setlength\tabcolsep{2pt}
  \begin{tabular}{lll}
    \toprule
     
     & \multicolumn{1}{c}{\textbf{LIF} ($T=5$)}     & \multicolumn{1}{c}{\textbf{SRM} ($T=5$)}                \\
    \cmidrule(r){2-2}
    \cmidrule(r){3-3}
     \textbf{Constant}  & \makecell[c]{Reward$\uparrow$}      &  \makecell[c]{Reward$\uparrow$}      \\
    \hline
    0.1  & \makecell[c]{5662}      & \makecell[c]{5803}   \\

    0.2(original)  & \makecell[c]{\textbf{5726}}         & \makecell[c]{\textbf{5879}} \\
    0.3  &  \makecell[c]{5648}    &  \makecell[c]{5747}    \\
    % DT3~\cite{sengupta2019going}   & 49.93    & 19.27   & 63.5\%  & 51.35 & 19.23 & 52.5\%  \\
    % \hline
    0.4  & \makecell[c]{5570}    &  \makecell[c]{5589} \\
    0.5  & \makecell[c]{5394}      &   \makecell[c]{5610}  \\
    % \hline
    1.0   &  \makecell[c]{5104}  &  \makecell[c]{5226}\\
    \bottomrule
  \end{tabular}
%   \vspace{-0.3cm}
\end{table}

\begin{table}
% \vspace{-0.3cm}
    \caption{Quantitative performance of Ant-v3 tasks with different constant coefficient settings under degraded inputs conditions.}
  \label{tab:0.2 Ant DI}
  \centering
  \scriptsize
  \setlength\tabcolsep{1pt}
  \begin{tabular}{llllllllllll}
    \toprule
     
     & & \multicolumn{1}{c}{\textbf{LIF} ($T=5$)}     & \multicolumn{1}{c}{\textbf{SRM} ($T=5$)}  & & & \multicolumn{1}{c}{\textbf{LIF} ($T=5$)}     & \multicolumn{1}{c}{\textbf{SRM} ($T=5$)}  & & & \multicolumn{1}{c}{\textbf{LIF} ($T=5$)}     & \multicolumn{1}{c}{\textbf{SRM} ($T=5$)}            \\
    \cmidrule(r){3-3}
    \cmidrule(r){4-4}
    \cmidrule(r){7-7}
    \cmidrule(r){8-8}
    \cmidrule(r){11-11}
    \cmidrule(r){12-12}
      \textbf{Type} & \textbf{Constant}  & \makecell[c]{Reward$\uparrow$}        &  \makecell[c]{Reward$\uparrow$}    &\textbf{ Type} & \textbf{Constant}  & \makecell[c]{Reward$\uparrow$}        &  \makecell[c]{Reward$\uparrow$}    &\textbf{ Type} & \textbf{Constant}  & \makecell[c]{Reward$\uparrow$}  &  \makecell[c]{Reward$\uparrow$} 
      \\
    \hline
    \makecell[c]{\multirow{7}{*}{\makecell[c]{Random \\ joint \\ position}}}
    & 0.1  & \makecell[c]{3241}    & \makecell[c]{3368}   & \makecell[c]{\multirow{6}{*}{\makecell[c]{Random \\ joint \\ velocity}}}   & 0.1  & \makecell[c]{2983}   & \makecell[c]{2772} &
  \makecell[c]{\multirow{6}{*}{GN}} &
    0.1 & \makecell[c]{1214}   & \makecell[c]{1478}   \\
    & 0.2(original)   & \textbf{\makecell[c]{3339}}      & \makecell[c]{\textbf{3450}}   & & 0.2(original)    & \textbf{\makecell[c]{3103}}      & \textbf{\makecell[c]{2984}} 
    & & 0.2(original)    & \textbf{\makecell[c]{1269}}       & \makecell[c]{\textbf{1559}}\\
    & 0.3 & \makecell[c]{3188}   & \makecell[c]{3380}  & &  0.3  & \makecell[c]{3032}       &  \makecell[c]{2704} 
    & & 0.3  &   \makecell[c]{1148}    &   \makecell[c]{1409}   \\

    & 0.4  & \makecell[c]{3213}    & \makecell[c]{3217}    & & 0.4  & \makecell[c]{2844}      & \makecell[c]{2655}    & & 0.4  & \makecell[c]{1003}     & \makecell[c]{1255}   \\
    & 0.5  & \makecell[c]{3062}      & \makecell[c]{3048}  & & 0.5  & \makecell[c]{2697}       & \makecell[c]{2517}    &  & 0.5   & \makecell[c]{980}      & \makecell[c]{1261} \\

    & 1.0   & \makecell[c]{2676}    & \makecell[c]{2572}   & & 1.0   & \makecell[c]{2230}      & \makecell[c]{2280}
    & & 1.0   & \makecell[c]{772}     & \makecell[c]{1083}\\
    \bottomrule
  \end{tabular}
\vspace{-0.5cm}
\end{table}

\begin{table}
\vspace{-0.5cm}
    \caption{Quantitative performance of Ant-v3 tasks with different constant coefficient settings under weight uncertainty conditions.}
  \label{tab:0.2 Ant WU}
  \centering
  \scriptsize
  \setlength\tabcolsep{1pt}
  \begin{tabular}{llllllllllll}
    \toprule
     
     & & \multicolumn{1}{c}{\textbf{LIF} ($T=5$)}     & \multicolumn{1}{c}{\textbf{SRM} ($T=5$)}  & & & \multicolumn{1}{c}{\textbf{LIF} ($T=5$)}     & \multicolumn{1}{c}{\textbf{SRM} ($T=5$)}  & & & \multicolumn{1}{c}{\textbf{LIF} ($T=5$)}     & \multicolumn{1}{c}{\textbf{SRM} ($T=5$)}            \\
    \cmidrule(r){3-3}
    \cmidrule(r){4-4}
    \cmidrule(r){7-7}
    \cmidrule(r){8-8}
    \cmidrule(r){11-11}
    \cmidrule(r){12-12}
      \textbf{Type} & \textbf{Constant}  & \makecell[c]{Reward$\uparrow$}        &  \makecell[c]{Reward$\uparrow$}    &\textbf{ Type} & \textbf{Constant}  & \makecell[c]{Reward$\uparrow$}        &  \makecell[c]{Reward$\uparrow$}    &\textbf{ Type} & \textbf{Constant}  & \makecell[c]{Reward$\uparrow$}  &  \makecell[c]{Reward$\uparrow$} 
      \\
    \hline
    \multirow{7}{*}{\makecell[c]{8-bit \\ Loihi \\ weight}}
    & 0.1  & \makecell[c]{5413}         & \makecell[c]{5600}   & \multirow{7}{*}{\makecell[c]{GN \\ weight}}
    & 0.1  & \makecell[c]{2703}  &  \makecell[c]{1596}   &
    \multirow{7}{*}{\makecell[c]{ $30\%$ \\ Zero \\ weight}}
    & 0.1  & \makecell[c]{2883}        & \makecell[c]{2925}    \\
    & 0.2(original)   & \textbf{\makecell[c]{5570}}      & \makecell[c]{\textbf{5648}}     & & 0.2(original)     & \textbf{\makecell[c]{2782}}      & \textbf{\makecell[c]{1658}}      & & 0.2(original)    & \textbf{\makecell[c]{2931}}       & \makecell[c]{\textbf{3046}}  \\
    & 0.3 & \makecell[c]{5373}   & \makecell[c]{5583}  & &  0.3  & \makecell[c]{2636}       &  \makecell[c]{1554} 
    & & 0.3  &   \makecell[c]{2945}    &   \makecell[c]{2990}   \\

    & 0.4 & \makecell[c]{5230}    & \makecell[c]{5349}    & & 0.4  & \makecell[c]{2488}      & \makecell[c]{1433}    & & 0.4  & \makecell[c]{2802}     & \makecell[c]{2731}   \\
    & 0.5  & \makecell[c]{5022}      & \makecell[c]{5224}  & & 0.5   & \makecell[c]{2523}       & \makecell[c]{1382}    &  & 0.5    & \makecell[c]{2652}      & \makecell[c]{2583} \\ 
    & 1.0   & \makecell[c]{4448}       & \makecell[c]{4783}           & & 1.0  & \makecell[c]{2205}       & \makecell[c]{1071}   & & 1.0 & \makecell[c]{2217}       & \makecell[c]{1992}  \\
    \bottomrule
  \end{tabular}
% \vspace{-0.3cm}
\end{table}

%%%%%%%%%%%%%%%%%%%%%% Ant-v3 0.2 %%%%%%%%%%%%%%%%%%%%%%%%%%%%%%%%%%%
