# Supplementary material for: Biologically Inspired Dynamic Thresholds for Spiking Neural Networks
Source: arXiv:2206.04426 source file (2023-06-19)
Supplement: Supplementary file 9 [file impact_random_seeds.tex]

\noindent
In this section, we study the impact of the random seeds during the training process on the proposed \DTname. For the obstacle avoidance tasks, we train five models for each LIF- and SRM-based host SNN, corresponding to five different random seeds. The SRs and the corresponding error bars of the trained host SNNs are reported in Figure~\ref{fig:RS_performance}a and Tables~\ref{tab:RS OA SO}, ~\ref{tab:RS OA DO}, ~\ref{tab: RS OA DI}, and ~\ref{tab: RS OA WU}.

\noindent
For the continuous control tasks, the rewards obtained in the HalfCheetah-v3 tasks under all experimental conditions are shown in Figure~\ref{fig:RS_performance}b. The corresponding experimental results are reported in Tables~\ref{tab:RS HC NC}, ~\ref{tab: RS HC DI}, and ~\ref{tab: RS HC WU}. In Tables~\ref{tab:RS Ant NC}, ~\ref{tab:RS Ant DI}, and ~\ref{tab:RS Ant WU}, we report the experimental results of the Ant-v3 tasks under all experimental settings. The results are also illustrated in Figure~\ref{fig:RS_performance}c. 

\noindent
Since the mean success rates and rewards obtained in the three tasks differ significantly, we calculate coefficients of variation to produce fair comparisons. We observe that the random seeds have the lowest impact on the obstacle avoidance tasks and the most substantial influence on the Ant-v3 tasks.

%%%%%%%%%%%%%%%%%%%%%%%%%%%% OA random seed begin %%%%%%%%%%%%%%%%%%%%%%%%%%%%%%

\begin{table}
\vspace{-0.5cm}
\centering
 \caption{Quantitative performance of obstacle avoidance tasks under the standard static obstacle conditions with respect to random seeds.}

  \vspace{0.2cm}
  \label{tab:RS OA SO}

  \centering
  \small
  \setlength\tabcolsep{3pt}
  \begin{tabular}{lll}
    \toprule
     
     & \multicolumn{1}{c}{\textbf{LIF} ($T=5$)}     & \multicolumn{1}{c}{\textbf{SRM} ($T=5$)}                \\
    \cmidrule(r){2-2}
    \cmidrule(r){3-3}
     \textbf{Random Seed}  & \makecell[c]{SR$\uparrow$}      &  \makecell[c]{SR$\uparrow$}      \\
    \hline
    \makecell[c]{1}  & \makecell[c]{\textbf{98.5\%}}      & \makecell[c]{96\%}   \\

    \makecell[c]{2}  & \makecell[c]{\textbf{98.5\%}}         & \makecell[c]{\textbf{96.5\%\%}} \\
    \makecell[c]{3}  &  \makecell[c]{97\%}    &  \makecell[c]{95\%}    \\
    % DT3~\cite{sengupta2019going}   & 49.93    & 19.27   & 63.5\%  & 51.35 & 19.23 & 52.5\%  \\
    % \hline
    \makecell[c]{4}  & \makecell[c]{96.5\%}    &  \makecell[c]{95.5\%} \\
    \makecell[c]{5}  & \makecell[c]{98\%}      &   \makecell[c]{96\%}  \\
    \hline
    \makecell[c]{Mean}   & \makecell[c]{97.7\%} &        \makecell[c]{95.8\%}   \\  
    \makecell[c]{Standard Deviation}    & \makecell[c]{0.008} &   \makecell[c]{0.005}    \\
    \hline
    \makecell[c]{Coefficient \\ of Variation}   & \makecell[c]{0.008} &        \makecell[c]{0.005}   \\ 
    \bottomrule
  \end{tabular}
%   \vspace{-0.3cm}
\end{table}

\begin{table}
\vspace{-0.3cm}
\centering
 \caption{Quantitative performance of obstacle avoidance tasks under dynamic obstacle conditions with respect to random seeds.}

  \vspace{0.2cm}
  \label{tab:RS OA DO}

  \centering
  \small
  \setlength\tabcolsep{3pt}
  \begin{tabular}{lll}
    \toprule
     
     & \multicolumn{1}{c}{\textbf{LIF} ($T=5$)}     & \multicolumn{1}{c}{\textbf{SRM} ($T=5$)}                \\
    \cmidrule(r){2-2}
    \cmidrule(r){3-3}
     \textbf{Random Seed}  & \makecell[c]{SR$\uparrow$}      &  \makecell[c]{SR$\uparrow$}      \\
    \hline
    \makecell[c]{1}  & \makecell[c]{92\%}      & \makecell[c]{89.5\%}   \\

    \makecell[c]{2}  & \makecell[c]{\textbf{92.5\%}}         & \makecell[c]{\textbf{90.5\%}} \\
    \makecell[c]{3}  &  \makecell[c]{91\%}    &  \makecell[c]{90.5\%}    \\
    % DT3~\cite{sengupta2019going}   & 49.93    & 19.27   & 63.5\%  & 51.35 & 19.23 & 52.5\%  \\
    % \hline
    \makecell[c]{4}  & \makecell[c]{92\%}    &  \makecell[c]{90\%} \\
    \makecell[c]{5}  & \makecell[c]{92.5\%}      &   \makecell[c]{89.5\%}  \\
    \hline
    \makecell[c]{Mean}   & \makecell[c]{92\%} &        \makecell[c]{90\%}   \\  
    \makecell[c]{Standard Deviation}    & \makecell[c]{0.005} &   \makecell[c]{0.004}    \\
    \hline
    \makecell[c]{Coefficient \\ of Variation}   & \makecell[c]{0.006} &        \makecell[c]{0.005}   \\ 
    \bottomrule
  \end{tabular}
  \vspace{-0.3cm}
\end{table}

\begin{table}
\vspace{-0.3cm}
    \caption{Quantitative performance of obstacle avoidance tasks under degraded input conditions with respect to random seeds.}
  \label{tab: RS OA DI}
  \centering
  \scriptsize
    \fontsize{6pt}{\baselineskip}\selectfont
  \setlength\tabcolsep{3pt}
  \begin{tabular}{llllllllllll}
    \toprule
     
     & & \multicolumn{1}{c}{\makecell[c]{\textbf{LIF} \\ ($T=5$)}}     & \multicolumn{1}{c}{\makecell[c]{\textbf{SRM} \\ ($T=5$)}}  & & & \multicolumn{1}{c}{\makecell[c]{\textbf{LIF}\\ ($T=5$)}}     & \multicolumn{1}{c}{\makecell[c]{\textbf{SRM}\\ ($T=5$)}}  & & & \multicolumn{1}{c}{\makecell[c]{\textbf{LIF} \\($T=5$)}}     & \multicolumn{1}{c}{\makecell[c]{\textbf{SRM} \\($T=5$)}}            \\
    \cmidrule(r){3-3}
    \cmidrule(r){4-4}
    \cmidrule(r){7-7}
    \cmidrule(r){8-8}
    \cmidrule(r){11-11}
    \cmidrule(r){12-12}
      \textbf{Type} & \textbf{Random Seed}  & \makecell[c]{SR$\uparrow$}        &  \makecell[c]{SR$\uparrow$}    &\textbf{ Type} & \textbf{Random Seed}  & \makecell[c]{SR$\uparrow$}        &  \makecell[c]{SR$\uparrow$}    &\textbf{ Type} & \textbf{Random Seed}  & \makecell[c]{SR$\uparrow$}  &  \makecell[c]{SR$\uparrow$} 
      \\
    \hline
    \makecell[c]{\multirow{7}{*}{\makecell[c]{0.2}}}
    & \makecell[c]{1}  & \makecell[c]{89\%}    & \makecell[c]{79\%}   & \makecell[c]{\multirow{7}{*}{\makecell[c]{0.6}}}   & \makecell[c]{1}  & \makecell[c]{83.5\%}   & \makecell[c]{82\%} &
  \makecell[c]{\multirow{7}{*}{GN}} & 
    \makecell[c]{1} & \makecell[c]{82.5\%}   & \makecell[c]{81.5\%}   \\
    & \makecell[c]{2}   & \textbf{\makecell[c]{90\%}}      & \makecell[c]{\textbf{79.5\%}}   & & \makecell[c]{2}    & \textbf{\makecell[c]{84.5\%}}      & \textbf{\makecell[c]{83\%}} 
    & & \makecell[c]{2}    & \textbf{\makecell[c]{84.5\%}}       & \makecell[c]{\textbf{82.5\%}}\\
    & \makecell[c]{3} & \makecell[c]{89.5\%}   & \makecell[c]{79\%}  & &  \makecell[c]{3}  & \makecell[c]{85\%}       &  \makecell[c]{82.5\%} 
    & & \makecell[c]{3}  &   \makecell[c]{83\%}    &   \makecell[c]{81.5\%}   \\

    & \makecell[c]{4}  & \makecell[c]{88\%}    & \makecell[c]{78.5\%}    & & \makecell[c]{4}  & \makecell[c]{84\%}      & \makecell[c]{81.5\%}    & & \makecell[c]{4}  & \makecell[c]{83.5\%}     & \makecell[c]{81\%}   \\
    & \makecell[c]{5}  & \makecell[c]{89\%}      & \makecell[c]{78\%}  & & \makecell[c]{5}  & \makecell[c]{83\%}       & \makecell[c]{82\%}    &  & \makecell[c]{5}   & \makecell[c]{82\%}      & \makecell[c]{82\%} \\
    
    \cline{2-4}
    \cline{6-8}
    \cline{10-12}
    & \makecell[c]{Mean}   & \makecell[c]{89.1\%} &        \makecell[c]{78.8\%} & &  \makecell[c]{Mean}   & \makecell[c]{84\%} &        \makecell[c]{82.2\%} & &  \makecell[c]{Mean}   & \makecell[c]{83.1\%} &        \makecell[c]{81.7\%} \\  
    & \makecell[c]{Standard Deviation}    & \makecell[c]{0.007} &   \makecell[c]{0.005}   & & \makecell[c]{Standard Deviation}    & \makecell[c]{0.007} &   \makecell[c]{0.005} & & \makecell[c]{Standard Deviation}    & \makecell[c]{0.009} &   \makecell[c]{0.005} \\
    \cline{2-4}
    \cline{6-8}
    \cline{10-12}
    & \makecell[c]{Coefficient \\ of Variation}   & \makecell[c]{0.007} &        \makecell[c]{0.006} & &  \makecell[c]{Coefficient \\ of Variation}   & \makecell[c]{0.008} &        \makecell[c]{0.006} & &  \makecell[c]{Coefficient \\ of Variation}   & \makecell[c]{0.010} &        \makecell[c]{0.006} \\
    \bottomrule
  \end{tabular}
\vspace{-0.3cm}
\end{table}

\begin{table}
\vspace{-0.3cm}
    \caption{Quantitative performance of obstacle avoidance tasks under weight uncertainty conditions with respect to random seeds.}
  \label{tab: RS OA WU}
  \centering
  \scriptsize
  \fontsize{6pt}{\baselineskip}\selectfont
  \setlength\tabcolsep{3pt}
  \begin{tabular}{llllllllllll}
    \toprule
     
     & & \multicolumn{1}{c}{\makecell[c]{\textbf{LIF} \\ ($T=5$)}}     & \multicolumn{1}{c}{\makecell[c]{\textbf{SRM} \\ ($T=5$)}}  & & & \multicolumn{1}{c}{\makecell[c]{\textbf{LIF}\\ ($T=5$)}}     & \multicolumn{1}{c}{\makecell[c]{\textbf{SRM}\\ ($T=5$)}}  & & & \multicolumn{1}{c}{\makecell[c]{\textbf{LIF} \\($T=5$)}}     & \multicolumn{1}{c}{\makecell[c]{\textbf{SRM} \\($T=5$)}}            \\
    \cmidrule(r){3-3}
    \cmidrule(r){4-4}
    \cmidrule(r){7-7}
    \cmidrule(r){8-8}
    \cmidrule(r){11-11}
    \cmidrule(r){12-12}
      \textbf{Type} & \textbf{Random Seed}  & \makecell[c]{SR$\uparrow$}        &  \makecell[c]{SR$\uparrow$}    &\textbf{ Type} & \textbf{Random Seed}  & \makecell[c]{SR$\uparrow$}        &  \makecell[c]{SR$\uparrow$}    &\textbf{ Type} & \textbf{Random Seed}  & \makecell[c]{SR$\uparrow$}  &  \makecell[c]{SR$\uparrow$} 
      \\
    \hline
    \makecell[c]{\multirow{7}{*}{\makecell[c]{8-bit \\ Loihi \\ weight}}}
    & \makecell[c]{1}  & \makecell[c]{\textbf{90\%}}    & \makecell[c]{87\%}   & \makecell[c]{\multirow{7}{*}{\makecell[c]{GN \\ weight \\ (5 rounds)}}}   & \makecell[c]{1}  & \makecell[c]{85.8\%}   & \makecell[c]{61\%} &
  \makecell[c]{\multirow{7}{*}{\makecell[c]{$30\%$ \\ Zero \\ weight \\ (5 rounds)}}} & 
    \makecell[c]{1} & \makecell[c]{76.8\%}   & \makecell[c]{64.5\%}   \\
    & \makecell[c]{2}   & \textbf{\makecell[c]{90\%}}      & \makecell[c]{\textbf{88.5\%}}     & & \makecell[c]{2}     & \textbf{\makecell[c]{87.7\%}}      & \textbf{\makecell[c]{61.8\%}}      & & \makecell[c]{2}    & \textbf{\makecell[c]{77.2\%}}       & \makecell[c]{\textbf{65.2\%}}  \\
    & \makecell[c]{3} & \makecell[c]{88.5\%}   & \makecell[c]{86\%}  & &  \makecell[c]{3}  & \makecell[c]{87.1\%}       &  \makecell[c]{61.3\%} 
    & & \makecell[c]{3}  &   \makecell[c]{75.9\%}    &   \makecell[c]{63.9\%}   \\

    & \makecell[c]{4}  & \makecell[c]{88.5\%}    & \makecell[c]{88.5\%}    & & \makecell[c]{4}  & \makecell[c]{86.6\%}      & \makecell[c]{60.2\%}    & & \makecell[c]{4}  & \makecell[c]{75.4\%}     & \makecell[c]{64.5\%}   \\
    & \makecell[c]{5}  & \makecell[c]{89\%}      & \makecell[c]{86.5\%}  & & \makecell[c]{5}  & \makecell[c]{87.5\%}       & \makecell[c]{60.8\%}    &  & \makecell[c]{5}   & \makecell[c]{76.9\%}      & \makecell[c]{65.0\%} \\

    \cline{2-4}
    \cline{6-8}
    \cline{10-12}
    & \makecell[c]{Mean}   & \makecell[c]{89.2\%} &        \makecell[c]{87.3\%} & &  \makecell[c]{Mean}   & \makecell[c]{86.9\%} &        \makecell[c]{61\%} & &  \makecell[c]{Mean}   & \makecell[c]{76.4\%} &        \makecell[c]{64.6\%} \\  
    & \makecell[c]{Standard Deviation}    & \makecell[c]{0.007} &   \makecell[c]{0.010}   & & \makecell[c]{Standard Deviation}    & \makecell[c]{0.007} &   \makecell[c]{0.005} & & \makecell[c]{Standard Deviation}    & \makecell[c]{0.007} &   \makecell[c]{0.005} \\
    \cline{2-4}
    \cline{6-8}
    \cline{10-12}
    & \makecell[c]{Coefficient \\ of Variation}   & \makecell[c]{0.008} &        \makecell[c]{0.012} & &  \makecell[c]{Coefficient \\ of Variation}   & \makecell[c]{0.008} &        \makecell[c]{0.009} & &  \makecell[c]{Coefficient \\ of Variation}   & \makecell[c]{0.009} &        \makecell[c]{0.007} \\
    \bottomrule
  \end{tabular}
% \vspace{-0.3cm}
\end{table}
%%%%%%%%%%%%%%%%%%%%%%%%%%%% OA random seed end %%%%%%%%%%%%%%%%%%%%%%%%%%%%%%

%%%%%%%%%%%%%%%%%%%%%%%%%%%% HC random seed begin %%%%%%%%%%%%%%%%%%%%%%%%%%%%%%
\begin{table}
% \vspace{-0.5cm}
\centering
 \caption{Quantitative performance of HalfCheetah-v3 tasks under standard testing condition with respect to random seeds.}

  \vspace{0.2cm}
  \label{tab:RS HC NC}

  \centering
  \small
  \setlength\tabcolsep{3pt}
  \begin{tabular}{lll}
    \toprule
     
     & \multicolumn{1}{c}{\textbf{LIF} ($T=5$)}     & \multicolumn{1}{c}{\textbf{SRM} ($T=5$)}                \\
    \cmidrule(r){2-2}
    \cmidrule(r){3-3}
     \textbf{Random Seed}  & \makecell[c]{Reward$\uparrow$}      &  \makecell[c]{Reward$\uparrow$}      \\
    \hline
    \makecell[c]{1}  & \makecell[c]{11064}      & \makecell[c]{11960}   \\

    \makecell[c]{2}  & \makecell[c]{10979}         & \makecell[c]{11873} \\
    \makecell[c]{3}  &  \makecell[c]{9848}    &  \makecell[c]{10474}    \\
    % DT3~\cite{sengupta2019going}   & 49.93    & 19.27   & 63.5\%  & 51.35 & 19.23 & 52.5\%  \\
    % \hline
    \makecell[c]{4}  & \makecell[c]{10881}    &  \makecell[c]{11061} \\
    \makecell[c]{5}  & \makecell[c]{8992}      &   \makecell[c]{11644}  \\
    \makecell[c]{6}  & \makecell[c]{10977}      &   \makecell[c]{10939}  \\
    \makecell[c]{7}  & \makecell[c]{10975}      &   \makecell[c]{11337}  \\
    \makecell[c]{8}  & \makecell[c]{10869}      &   \makecell[c]{11777}  \\
    \makecell[c]{9}  & \makecell[c]{10932}      &   \makecell[c]{10673}  \\
    \makecell[c]{10}  & \makecell[c]{10993}      &   \makecell[c]{11841}  \\
    
    \hline
    \makecell[c]{Mean}   & \makecell[c]{10651} &        \makecell[c]{11358}   \\  
    \makecell[c]{Standard Deviation}    & \makecell[c]{647} &   \makecell[c]{513}    \\
    \hline
    \makecell[c]{Coefficient \\ of Variation}   & \makecell[c]{0.061} &        \makecell[c]{0.045}   \\  
    % \hline
    \bottomrule
  \end{tabular}
  \vspace{-0.3cm}
\end{table}

\begin{table}
\vspace{-0.3cm}
    \caption{Quantitative performance of the HalfCheetah-v3 tasks under degraded input conditions with respect to random seeds.}
  \label{tab: RS HC DI}
  \centering
    % \fontsize{7pt}{\baselineskip}\selectfont
  \scriptsize
  \fontsize{6pt}{\baselineskip}\selectfont
  \setlength\tabcolsep{3pt}
  \begin{tabular}{llllllllllll}
    \toprule
     
     & & \multicolumn{1}{c}{\makecell[c]{\textbf{LIF} \\ ($T=5$)}}     & \multicolumn{1}{c}{\makecell[c]{\textbf{SRM} \\ ($T=5$)}}  & & & \multicolumn{1}{c}{\makecell[c]{\textbf{LIF}\\ ($T=5$)}}     & \multicolumn{1}{c}{\makecell[c]{\textbf{SRM}\\ ($T=5$)}}  & & & \multicolumn{1}{c}{\makecell[c]{\textbf{LIF} \\($T=5$)}}     & \multicolumn{1}{c}{\makecell[c]{\textbf{SRM} \\($T=5$)}}            \\
    \cmidrule(r){3-3}
    \cmidrule(r){4-4}
    \cmidrule(r){7-7}
    \cmidrule(r){8-8}
    \cmidrule(r){11-11}
    \cmidrule(r){12-12}
      \textbf{Type} & \textbf{Random Seed}  & \makecell[c]{Reward$\uparrow$}        &  \makecell[c]{Reward$\uparrow$}    &\textbf{ Type} & \textbf{Random Seed}  & \makecell[c]{Reward$\uparrow$}        &  \makecell[c]{Reward$\uparrow$}    &\textbf{ Type} & \textbf{Random Seed}  & \makecell[c]{Reward$\uparrow$}  &  \makecell[c]{Reward$\uparrow$} 
      \\
    \hline
    \makecell[c]{\multirow{12}{*}{\makecell[c]{Random \\ joint \\ position}}}
    & \makecell[c]{1}  & \makecell[c]{8465}    & \makecell[c]{7883}   & \makecell[c]{\multirow{12}{*}{\makecell[c]{Random \\ joint \\ position}}}   & \makecell[c]{1}  & \makecell[c]{8302}   & \makecell[c]{7116} &
  \makecell[c]{\multirow{12}{*}{GN}} & 
    \makecell[c]{1} & \makecell[c]{3909}   & \makecell[c]{3895}   \\
    & \makecell[c]{2}  & \makecell[c]{8452}     & \makecell[c]{7788}   & & \makecell[c]{2}    & \makecell[c]{8239}     & \makecell[c]{7101}  & & \makecell[c]{2}    & \makecell[c]{3820}       & \makecell[c]{3854}\\
    & \makecell[c]{3} & \makecell[c]{7617}   & \makecell[c]{6618}  & &  \makecell[c]{3}  & \makecell[c]{7575}       &  \makecell[c]{5684}     & & \makecell[c]{3}  &   \makecell[c]{3292}    &   \makecell[c]{2648}   \\
    & \makecell[c]{4}  & \makecell[c]{8399}    & \makecell[c]{7001}    & & \makecell[c]{4}  & \makecell[c]{8274}      & \makecell[c]{6208}    & & \makecell[c]{4}  & \makecell[c]{3797}     & \makecell[c]{2979}   \\
    & \makecell[c]{5}  & \makecell[c]{7003}      & \makecell[c]{7622}  & & \makecell[c]{5}  & \makecell[c]{7216}       & \makecell[c]{6869}    &  & \makecell[c]{5}   & \makecell[c]{2816}      & \makecell[c]{3561} \\
    & \makecell[c]{6} & \makecell[c]{8320}   & \makecell[c]{7280}  & &  \makecell[c]{6}  & \makecell[c]{8226}       &  \makecell[c]{6540}     & & \makecell[c]{6}  &   \makecell[c]{3675}    &   \makecell[c]{3197}   \\
    & \makecell[c]{7}  & \makecell[c]{8339}    & \makecell[c]{7557}    & & \makecell[c]{7}  & \makecell[c]{8288}      & \makecell[c]{6806}    & & \makecell[c]{7}  & \makecell[c]{3790}     & \makecell[c]{3636}   \\
    & \makecell[c]{8}  & \makecell[c]{8348}      & \makecell[c]{7832}  & & \makecell[c]{8}  & \makecell[c]{8129}       & \makecell[c]{6805}    &  & \makecell[c]{8}   & \makecell[c]{3743}      & \makecell[c]{3582} \\
    & \makecell[c]{9} & \makecell[c]{8329}   & \makecell[c]{6777}  & &  \makecell[c]{9}  & \makecell[c]{8118}       &  \makecell[c]{6044}     & & \makecell[c]{9}  &   \makecell[c]{3858}    &   \makecell[c]{2770}   \\
    & \makecell[c]{10}  & \makecell[c]{8423}    & \makecell[c]{7781}    & & \makecell[c]{10}  & \makecell[c]{8208}      & \makecell[c]{6964}    & & \makecell[c]{10}  & \makecell[c]{3806}     & \makecell[c]{3667}   \\
    
    \cline{2-4}
    \cline{6-8}
    \cline{10-12}
    & \makecell[c]{Mean}   & \makecell[c]{8169} &        \makecell[c]{7414} & &  \makecell[c]{Mean}   & \makecell[c]{8058} &        \makecell[c]{6614} & &  \makecell[c]{Mean}   & \makecell[c]{3651} &        \makecell[c]{3379} \\  
    & \makecell[c]{Standard Deviation}    & \makecell[c]{454} &   \makecell[c]{443}   & & \makecell[c]{Standard Deviation}    & \makecell[c]{345} &   \makecell[c]{459} & & \makecell[c]{Standard Deviation}    & \makecell[c]{322} &   \makecell[c]{426} \\
    \cline{2-4}
    \cline{6-8}
    \cline{10-12}
    & \makecell[c]{Coefficient \\ of Variation}   & \makecell[c]{0.056} &        \makecell[c]{0.06} & &  \makecell[c]{Coefficient \\ of Variation}   & \makecell[c]{0.043} &        \makecell[c]{0.069} & &  \makecell[c]{Coefficient \\ of Variation}   & \makecell[c]{0.088} &        \makecell[c]{0.126} \\  
    
    \bottomrule
  \end{tabular}
\vspace{-0.3cm}
\end{table}

\begin{table}
\vspace{-0.3cm}
    \caption{Quantitative performance of the HalfCheetah-v3 tasks under weight uncertainty conditions with respect to random seeds.}
  \label{tab: RS HC WU}
  \centering
    % \fontsize{7pt}{\baselineskip}\selectfont
  \scriptsize
  \fontsize{6pt}{\baselineskip}\selectfont
  \setlength\tabcolsep{3pt}
  \begin{tabular}{llllllllllll}
    \toprule
     
     & & \multicolumn{1}{c}{\makecell[c]{\textbf{LIF} \\ ($T=5$)}}     & \multicolumn{1}{c}{\makecell[c]{\textbf{SRM} \\ ($T=5$)}}  & & & \multicolumn{1}{c}{\makecell[c]{\textbf{LIF}\\ ($T=5$)}}     & \multicolumn{1}{c}{\makecell[c]{\textbf{SRM}\\ ($T=5$)}}  & & & \multicolumn{1}{c}{\makecell[c]{\textbf{LIF} \\($T=5$)}}     & \multicolumn{1}{c}{\makecell[c]{\textbf{SRM} \\($T=5$)}}            \\
    \cmidrule(r){3-3}
    \cmidrule(r){4-4}
    \cmidrule(r){7-7}
    \cmidrule(r){8-8}
    \cmidrule(r){11-11}
    \cmidrule(r){12-12}
      \textbf{Type} & \textbf{Random Seed}  & \makecell[c]{Reward$\uparrow$}        &  \makecell[c]{Reward$\uparrow$}    &\textbf{ Type} & \textbf{Random Seed}  & \makecell[c]{Reward$\uparrow$}        &  \makecell[c]{Reward$\uparrow$}    &\textbf{ Type} & \textbf{Random Seed}  & \makecell[c]{Reward$\uparrow$}  &  \makecell[c]{Reward$\uparrow$} 
      \\
    \hline
    \makecell[c]{\multirow{12}{*}{\makecell[c]{8-bit \\ Loihi \\ weight}}}
    & \makecell[c]{1}  & \makecell[c]{10823}    & \makecell[c]{11767}   & \makecell[c]{\multirow{12}{*}{\makecell[c]{GN \\ weight}}}   & \makecell[c]{1}  & \makecell[c]{6928}   & \makecell[c]{8381} &
  \makecell[c]{\multirow{12}{*}{\makecell[c]{$30\%$ \\ Zero \\ weight}}} & 
    \makecell[c]{1} & \makecell[c]{6551}   & \makecell[c]{5386}   \\
    & \makecell[c]{2}   & \makecell[c]{10767}   & \makecell[c]{11749}   & & \makecell[c]{2}   & \makecell[c]{6704}      & \makecell[c]{8307}      & & \makecell[c]{2}    & \makecell[c]{6486}       & \makecell[c]{5308}  \\
    & \makecell[c]{3} & \makecell[c]{10062}   & \makecell[c]{10406}  & &  \makecell[c]{3}  & \makecell[c]{6155}       &  \makecell[c]{7208}   & & \makecell[c]{3}  &   \makecell[c]{5671}    &   \makecell[c]{3970}   \\
    & \makecell[c]{4}  & \makecell[c]{10648}    & \makecell[c]{10780}    & & \makecell[c]{4}  & \makecell[c]{6858}      & \makecell[c]{7527}    & & \makecell[c]{4}  & \makecell[c]{6296}     & \makecell[c]{4254}   \\
    & \makecell[c]{5}  & \makecell[c]{9368}      & \makecell[c]{11452}  & & \makecell[c]{5}  & \makecell[c]{5857}       & \makecell[c]{8216}    &  & \makecell[c]{5}   & \makecell[c]{5217}      & \makecell[c]{5249} \\
    & \makecell[c]{6} & \makecell[c]{10532}   & \makecell[c]{11097}  & &  \makecell[c]{6}  & \makecell[c]{6656}       &  \makecell[c]{7537}   & & \makecell[c]{6}  &   \makecell[c]{6282}    &   \makecell[c]{5007}   \\
    & \makecell[c]{7}  & \makecell[c]{10284}    & \makecell[c]{11358}    & & \makecell[c]{7}  & \makecell[c]{6838}      & \makecell[c]{8046}    & & \makecell[c]{7}  & \makecell[c]{6341}     & \makecell[c]{5040}   \\
    & \makecell[c]{8}  & \makecell[c]{10617}      & \makecell[c]{11768}  & & \makecell[c]{8}  & \makecell[c]{6729}       & \makecell[c]{8306}    &  & \makecell[c]{8}   & \makecell[c]{6231}      & \makecell[c]{5337} \\
    & \makecell[c]{9} & \makecell[c]{10788}   & \makecell[c]{10733}  & &  \makecell[c]{9}  & \makecell[c]{6740}       &  \makecell[c]{7598}   & & \makecell[c]{9}  &   \makecell[c]{6537}    &   \makecell[c]{4227}   \\
    & \makecell[c]{10}  & \makecell[c]{10787}    & \makecell[c]{11496}    & & \makecell[c]{10}  & \makecell[c]{6765}      & \makecell[c]{8282}    & & \makecell[c]{10}  & \makecell[c]{6481}     & \makecell[c]{5081}   \\
    \cline{2-4}
    \cline{6-8}
    \cline{10-12}
    & \makecell[c]{Mean}   & \makecell[c]{10468} &        \makecell[c]{11261} & &  \makecell[c]{Mean}   & \makecell[c]{6623} &        \makecell[c]{7941} & &  \makecell[c]{Mean}   & \makecell[c]{6209} &        \makecell[c]{4886} \\  
    & \makecell[c]{Standard Deviation}    & \makecell[c]{435} &   \makecell[c]{460}   & & \makecell[c]{Standard Deviation}    & \makecell[c]{324} &   \makecell[c]{407} & & \makecell[c]{Standard Deviation}    & \makecell[c]{410} &   \makecell[c]{501} \\
    \cline{2-4}
    \cline{6-8}
    \cline{10-12}
    & \makecell[c]{Coefficient \\ of Variation}   & \makecell[c]{0.042} &        \makecell[c]{0.041} & &  \makecell[c]{Coefficient \\ of Variation}   & \makecell[c]{0.049} &        \makecell[c]{0.051} & &  \makecell[c]{Coefficient \\ of Variation}   & \makecell[c]{0.066} &        \makecell[c]{0.103} \\ 
    \bottomrule
  \end{tabular}
\vspace{-0.3cm}
\end{table}
%%%%%%%%%%%%%%%%%%%%%%%%%%%% HC random seed end%%%%%%%%%%%%%%%%%%%%%%%%%%%%%%

%%%%%%%%%%%%%%%%%%%%%%%%%%%% Ant random seed begin %%%%%%%%%%%%%%%%%%%%%%%%%%%%%%
\begin{table}
\vspace{-0.5cm}
\centering
 \caption{Quantitative performance of the Ant-v3 tasks under standard testing condition with respect to random seeds.}

  \vspace{0.2cm}
  \label{tab:RS Ant NC}

  \centering
  \small
  \setlength\tabcolsep{3pt}
  \begin{tabular}{lll}
    \toprule
     
     & \multicolumn{1}{c}{\textbf{LIF} ($T=5$)}     & \multicolumn{1}{c}{\textbf{SRM} ($T=5$)}                \\
    \cmidrule(r){2-2}
    \cmidrule(r){3-3}
     \textbf{Random Seed}  & \makecell[c]{Reward$\uparrow$}      &  \makecell[c]{Reward$\uparrow$}      \\
    \hline
    \makecell[c]{1}  & \makecell[c]{5726}      & \makecell[c]{5879}   \\

    \makecell[c]{2}  & \makecell[c]{5678}         & \makecell[c]{5758} \\
    \makecell[c]{3}  &  \makecell[c]{5306}    &  \makecell[c]{5798}    \\
    % DT3~\cite{sengupta2019going}   & 49.93    & 19.27   & 63.5\%  & 51.35 & 19.23 & 52.5\%  \\
    % \hline
    \makecell[c]{4}  & \makecell[c]{5553}    &  \makecell[c]{5480} \\
    \makecell[c]{5}  & \makecell[c]{3980}      &   \makecell[c]{5508}  \\
    \makecell[c]{6}  & \makecell[c]{4657}      &   \makecell[c]{5590}  \\
    \makecell[c]{7}  & \makecell[c]{5692}      &   \makecell[c]{4063}  \\
    \makecell[c]{8}  & \makecell[c]{5595}      &   \makecell[c]{5829}  \\
    \makecell[c]{9}  & \makecell[c]{5688}      &   \makecell[c]{5429}  \\
    \makecell[c]{10}  & \makecell[c]{5696}      &   \makecell[c]{5616}  \\
    
    \hline
    \makecell[c]{Mean}   & \makecell[c]{5357} &        \makecell[c]{4933}   \\  
    \makecell[c]{Standard Deviation}    & \makecell[c]{553} &   \makecell[c]{500}    \\
    \hline
    \makecell[c]{Coefficient \\ of Variation}   & \makecell[c]{0.103} &        \makecell[c]{0.101}   \\  
    % \hline
    \bottomrule
  \end{tabular}
  \vspace{-0.3cm}
\end{table}

\begin{table}
\vspace{-0.3cm}
    \caption{Quantitative performance of Ant-v3 tasks under degraded input conditions with respect to random seeds.}
  \label{tab:RS Ant DI}
  \centering
    % \fontsize{7pt}{\baselineskip}\selectfont
  \scriptsize
  \fontsize{6pt}{\baselineskip}\selectfont
  \setlength\tabcolsep{3pt}
  \begin{tabular}{llllllllllll}
    \toprule
     
     & & \multicolumn{1}{c}{\makecell[c]{\textbf{LIF} \\ ($T=5$)}}     & \multicolumn{1}{c}{\makecell[c]{\textbf{SRM} \\ ($T=5$)}}  & & & \multicolumn{1}{c}{\makecell[c]{\textbf{LIF}\\ ($T=5$)}}     & \multicolumn{1}{c}{\makecell[c]{\textbf{SRM}\\ ($T=5$)}}  & & & \multicolumn{1}{c}{\makecell[c]{\textbf{LIF} \\($T=5$)}}     & \multicolumn{1}{c}{\makecell[c]{\textbf{SRM} \\($T=5$)}}            \\
    \cmidrule(r){3-3}
    \cmidrule(r){4-4}
    \cmidrule(r){7-7}
    \cmidrule(r){8-8}
    \cmidrule(r){11-11}
    \cmidrule(r){12-12}
      \textbf{Type} & \textbf{Random Seed}  & \makecell[c]{Reward$\uparrow$}        &  \makecell[c]{Reward$\uparrow$}    &\textbf{ Type} & \textbf{Random Seed}  & \makecell[c]{Reward$\uparrow$}        &  \makecell[c]{Reward$\uparrow$}    &\textbf{ Type} & \textbf{Random Seed}  & \makecell[c]{Reward$\uparrow$}  &  \makecell[c]{Reward$\uparrow$} 
      \\
    \hline
    \makecell[c]{\multirow{12}{*}{\makecell[c]{Random \\ joint \\ position}}}
    & \makecell[c]{1}  & \makecell[c]{3339}    & \makecell[c]{3450}   & \makecell[c]{\multirow{12}{*}{\makecell[c]{Random \\ joint \\ position}}}   & \makecell[c]{1}  & \makecell[c]{3103}   & \makecell[c]{2984} &
  \makecell[c]{\multirow{12}{*}{GN}} & 
    \makecell[c]{1} & \makecell[c]{1269}   & \makecell[c]{1559}   \\
    & \makecell[c]{2}  & \makecell[c]{3323}     & \makecell[c]{3423}   & & \makecell[c]{2}    & \makecell[c]{2879}     & \makecell[c]{2869}  & & \makecell[c]{2}    & \makecell[c]{1166}       & \makecell[c]{1524}\\
    & \makecell[c]{3} & \makecell[c]{2973}   & \makecell[c]{3059}  & &  \makecell[c]{3}  & \makecell[c]{2651}       &  \makecell[c]{2930}     & & \makecell[c]{3}  &   \makecell[c]{1030}    &   \makecell[c]{1432}   \\
    & \makecell[c]{4}  & \makecell[c]{3161}    & \makecell[c]{3049}    & & \makecell[c]{4}  & \makecell[c]{2763}      & \makecell[c]{2731}    & & \makecell[c]{4}  & \makecell[c]{1093}     & \makecell[c]{1357}   \\
    & \makecell[c]{5}  & \makecell[c]{2053}      & \makecell[c]{3234}  & & \makecell[c]{5}  & \makecell[c]{2105}       & \makecell[c]{2870}    &  & \makecell[c]{5}   & \makecell[c]{796}      & \makecell[c]{1440} \\
    & \makecell[c]{6} & \makecell[c]{2424}   & \makecell[c]{3339}  & &  \makecell[c]{6}  & \makecell[c]{2547}       &  \makecell[c]{2863}     & & \makecell[c]{6}  &   \makecell[c]{881}    &   \makecell[c]{1396}   \\
    & \makecell[c]{7}  & \makecell[c]{2993}    & \makecell[c]{2252}    & & \makecell[c]{7}  & \makecell[c]{2822}      & \makecell[c]{2032}    & & \makecell[c]{7}  & \makecell[c]{1132}     & \makecell[c]{830}   \\
    & \makecell[c]{8}  & \makecell[c]{3216}      & \makecell[c]{3365}  & & \makecell[c]{8}  & \makecell[c]{2892}       & \makecell[c]{2829}    &  & \makecell[c]{8}   & \makecell[c]{1105}      & \makecell[c]{1501} \\
    & \makecell[c]{9} & \makecell[c]{3217}   & \makecell[c]{3300}  & &  \makecell[c]{9}  & \makecell[c]{3047}       &  \makecell[c]{2815}     & & \makecell[c]{9}  &   \makecell[c]{1268}    &   \makecell[c]{1464}   \\
    & \makecell[c]{10}  & \makecell[c]{3218}    & \makecell[c]{3237}    & & \makecell[c]{10}  & \makecell[c]{2860}      & \makecell[c]{2692}    & & \makecell[c]{10}  & \makecell[c]{1020}     & \makecell[c]{1385}   \\
    \cline{2-4}
    \cline{6-8}
    \cline{10-12}
    & \makecell[c]{Mean}   & \makecell[c]{2992} &        \makecell[c]{2847} & &  \makecell[c]{Mean}   & \makecell[c]{2767} &        \makecell[c]{2492} & &  \makecell[c]{Mean}   & \makecell[c]{1076} &        \makecell[c]{1250} \\  
    & \makecell[c]{Standard Deviation}    & \makecell[c]{402} &   \makecell[c]{332}   & & \makecell[c]{Standard Deviation}    & \makecell[c]{270} &   \makecell[c]{256} & & \makecell[c]{Standard Deviation}    & \makecell[c]{144} &   \makecell[c]{196} \\
    \cline{2-4}
    \cline{6-8}
    \cline{10-12}
    & \makecell[c]{Coefficient \\ of Variation}   & \makecell[c]{0.134} &        \makecell[c]{0.117} & &  \makecell[c]{Coefficient \\ of Variation}   & \makecell[c]{0.098} &        \makecell[c]{0.103} & &  \makecell[c]{Coefficient \\ of Variation}   & \makecell[c]{0.134} &        \makecell[c]{0.157} \\ 
    \bottomrule
  \end{tabular}
\vspace{-0.3cm}
\end{table}

\begin{table}
\vspace{-0.3cm}
    \caption{Quantitative performance of Ant-v3 tasks under weight uncertainty conditions with respect to random seeds.}
  \label{tab:RS Ant WU}
  \centering
    % \fontsize{7pt}{\baselineskip}\selectfont
  \scriptsize
  \fontsize{6pt}{\baselineskip}\selectfont
  \setlength\tabcolsep{3pt}
  \begin{tabular}{llllllllllll}
    \toprule
     
    & & \multicolumn{1}{c}{\makecell[c]{\textbf{LIF} \\ ($T=5$)}}     & \multicolumn{1}{c}{\makecell[c]{\textbf{SRM} \\ ($T=5$)}}  & & & \multicolumn{1}{c}{\makecell[c]{\textbf{LIF}\\ ($T=5$)}}     & \multicolumn{1}{c}{\makecell[c]{\textbf{SRM}\\ ($T=5$)}}  & & & \multicolumn{1}{c}{\makecell[c]{\textbf{LIF} \\($T=5$)}}     & \multicolumn{1}{c}{\makecell[c]{\textbf{SRM} \\($T=5$)}}            \\
    \cmidrule(r){3-3}
    \cmidrule(r){4-4}
    \cmidrule(r){7-7}
    \cmidrule(r){8-8}
    \cmidrule(r){11-11}
    \cmidrule(r){12-12}
      \textbf{Type} & \textbf{Random Seed}  & \makecell[c]{Reward$\uparrow$}        &  \makecell[c]{Reward$\uparrow$}    &\textbf{ Type} & \textbf{Random Seed}  & \makecell[c]{Reward$\uparrow$}        &  \makecell[c]{Reward$\uparrow$}    &\textbf{ Type} & \textbf{Random Seed}  & \makecell[c]{Reward$\uparrow$}  &  \makecell[c]{Reward$\uparrow$} 
      \\
    \hline
    \makecell[c]{\multirow{12}{*}{\makecell[c]{8-bit \\ Loihi \\ weight}}}
    & \makecell[c]{1}  & \makecell[c]{5570}    & \makecell[c]{5648}   & \makecell[c]{\multirow{12}{*}{\makecell[c]{GN \\ weight}}}   & \makecell[c]{1}  & \makecell[c]{2782}   & \makecell[c]{1658} &
  \makecell[c]{\multirow{12}{*}{\makecell[c]{$30\%$ \\ Zero \\ weight}}} & 
    \makecell[c]{1} & \makecell[c]{2931}   & \makecell[c]{3046}   \\
    & \makecell[c]{2}   & \makecell[c]{5398}   & \makecell[c]{5641}   & & \makecell[c]{2}   & \makecell[c]{2668}      & \makecell[c]{1503}      & & \makecell[c]{2}    & \makecell[c]{2849}       & \makecell[c]{2859}  \\
    & \makecell[c]{3} & \makecell[c]{5219}   & \makecell[c]{5611}  & &  \makecell[c]{3}  & \makecell[c]{2518}       &  \makecell[c]{1467}   & & \makecell[c]{3}  &   \makecell[c]{2729}    &   \makecell[c]{2674}   \\
    & \makecell[c]{4}  & \makecell[c]{5309}    & \makecell[c]{5291}    & & \makecell[c]{4}  & \makecell[c]{2580}      & \makecell[c]{1341}    & & \makecell[c]{4}  & \makecell[c]{2741}     & \makecell[c]{2929}   \\
    & \makecell[c]{5}  & \makecell[c]{4395}      & \makecell[c]{5201}  & & \makecell[c]{5}  & \makecell[c]{1816}       & \makecell[c]{1522}    &  & \makecell[c]{5}   & \makecell[c]{1840}      & \makecell[c]{2794} \\
    & \makecell[c]{6} & \makecell[c]{4853}   & \makecell[c]{5394}  & &  \makecell[c]{6}  & \makecell[c]{2303}       &  \makecell[c]{1466}   & & \makecell[c]{6}  &   \makecell[c]{2125}    &   \makecell[c]{2730}   \\
    & \makecell[c]{7}  & \makecell[c]{5166}    & \makecell[c]{3968}    & & \makecell[c]{7}  & \makecell[c]{2426}      & \makecell[c]{959}    & & \makecell[c]{7}  & \makecell[c]{2654}     & \makecell[c]{1895}   \\
    & \makecell[c]{8}  & \makecell[c]{5365}      & \makecell[c]{5610}  & & \makecell[c]{8}  & \makecell[c]{2646}       & \makecell[c]{1595}    &  & \makecell[c]{8}   & \makecell[c]{2826}      & \makecell[c]{2760} \\
    & \makecell[c]{9} & \makecell[c]{5544}   & \makecell[c]{5416}  & &  \makecell[c]{9}  & \makecell[c]{2601}       &  \makecell[c]{1427}   & & \makecell[c]{9}  &   \makecell[c]{2874}    &   \makecell[c]{2635}   \\
    & \makecell[c]{10}  & \makecell[c]{5254}    & \makecell[c]{5343}    & & \makecell[c]{10}  & \makecell[c]{2422}      & \makecell[c]{1497}    & & \makecell[c]{10}  & \makecell[c]{2802}     & \makecell[c]{2644}   \\
    \cline{2-4}
    \cline{6-8}
    \cline{10-12}
    & \makecell[c]{Mean}   & \makecell[c]{5207} &        \makecell[c]{4778} & &  \makecell[c]{Mean}   & \makecell[c]{2476} &        \makecell[c]{1294} & &  \makecell[c]{Mean}   & \makecell[c]{2637} &        \makecell[c]{2432} \\  
    & \makecell[c]{Standard Deviation}    & \makecell[c]{333} &   \makecell[c]{473}   & & \makecell[c]{Standard Deviation}    & \makecell[c]{257} &   \makecell[c]{181} & & \makecell[c]{Standard Deviation}    & \makecell[c]{342} &   \makecell[c]{294} \\
    \cline{2-4}
    \cline{6-8}
    \cline{10-12}
    & \makecell[c]{Coefficient \\ of Variation}   & \makecell[c]{0.064} &        \makecell[c]{0.099} & &  \makecell[c]{Coefficient \\ of Variation}   & \makecell[c]{0.104} &        \makecell[c]{0.140} & &  \makecell[c]{Coefficient \\ of Variation}   & \makecell[c]{0.130} &        \makecell[c]{0.121} \\ 
    \bottomrule
  \end{tabular}
\vspace{-0.3cm}
\end{table}

\begin{figure}[ht!]
	\centering
	\includegraphics [scale=0.19]{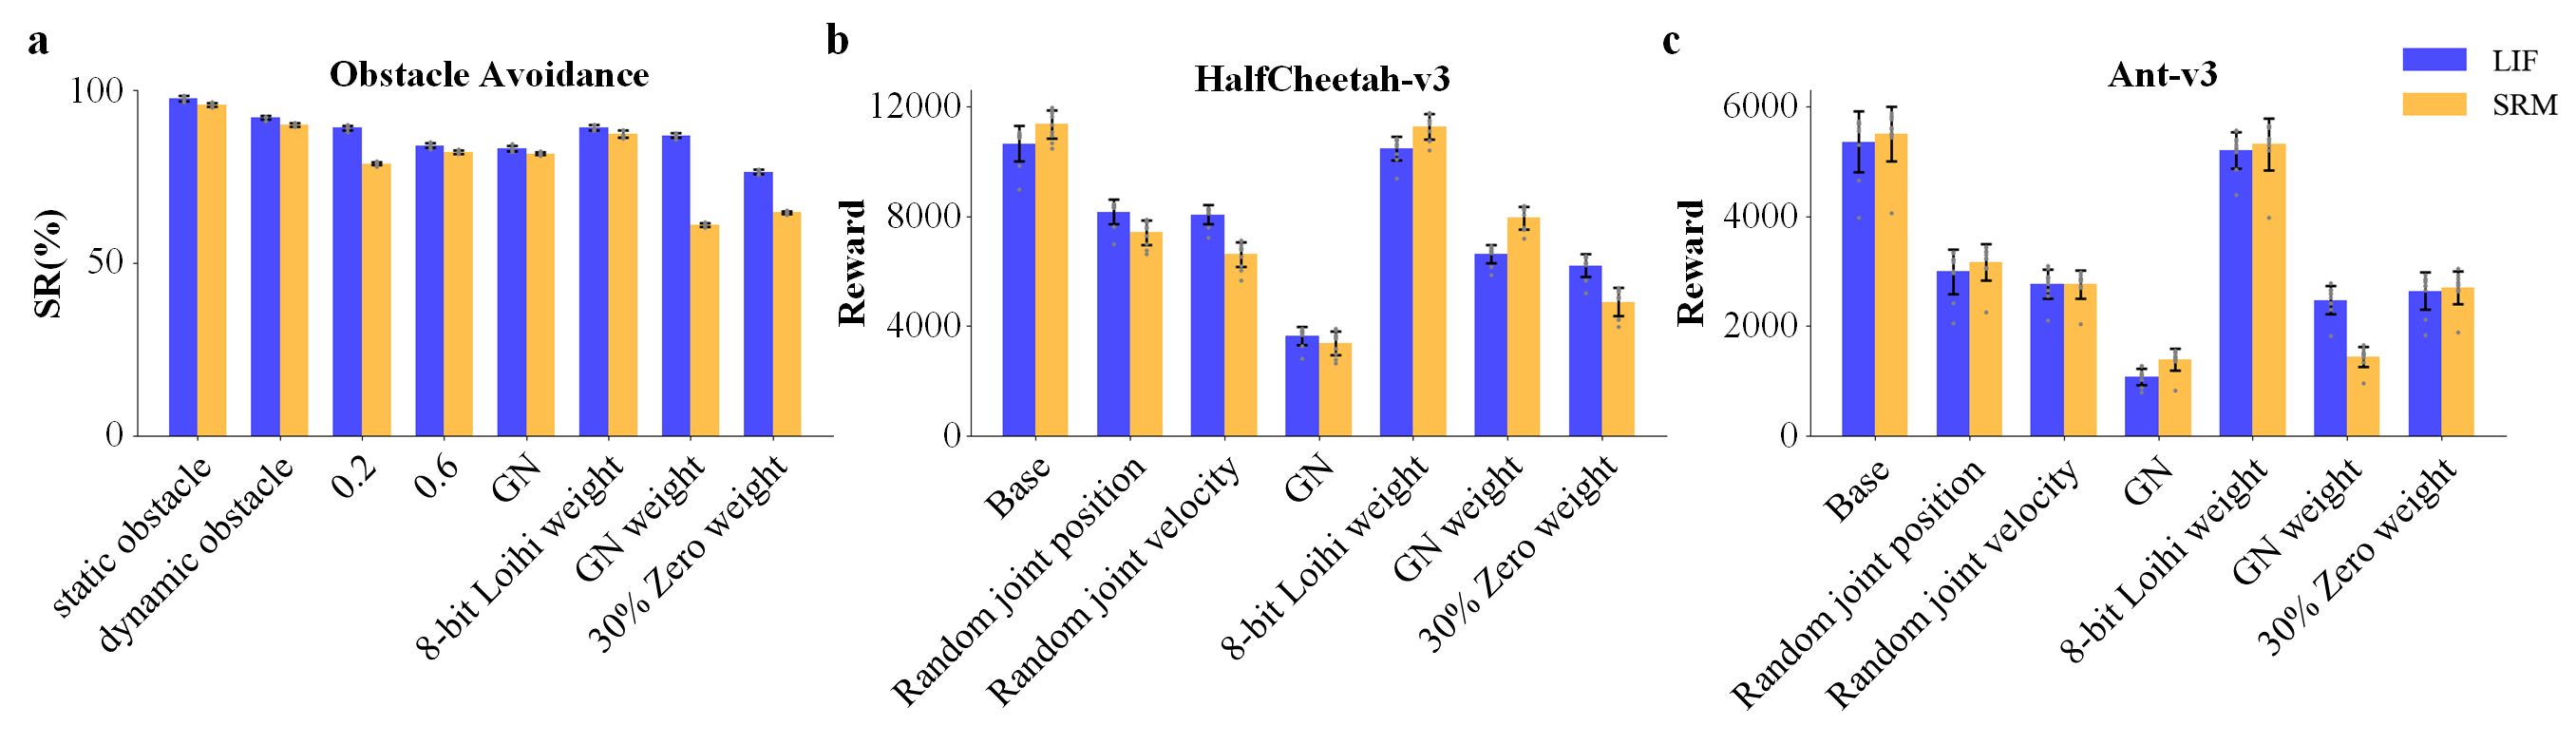}
	\vspace{-0.3cm}
	\caption{
		\bd{Quantitative performance of the LIF- and SRM-based \DTname\-host SNNs with respect to random seeds.}
	}
	\label{fig:RS_performance}
	\vspace{-0.5cm}
\end{figure}

%%%%%%%%%%%%%%%%%%%%%%%%%%%% Ant random seed end%%%%%%%%%%%%%%%%%%%%%%%%%%%%%%
