# Supplementary material for: Biologically Inspired Dynamic Thresholds for Spiking Neural Networks
Source: arXiv:2206.04426 source file (2023-06-19)
Supplement: Supplementary file 10 [file statistical_parameters_settings.tex]

We study the impact of the proposed layerwise statistical parameter settings, an extension of section 4.3 of our main paper. The experimental settings and the corresponding results are reported in Table~\ref{SMtab:SPS}. Without replacing the constants of the original biological model, the proposed method is is only slightly better than the ones without any training. Both LIF- and SRM-based experiments validate that the proposed statistical cues are essential to the proposed method.

\begin{table}[hb]
\caption{Quantitative performance of BDETT without statistical parameter settings (SPS) under the stardard testing conditions. OA means obstacle avoidance; HC-v3 indicates HalfCheetah-v3.}
  \label{SMtab:SPS}
  \centering
  \setlength\tabcolsep{5pt}
  \begin{tabular}{lllllllll}
    \toprule
     
     & & & \multicolumn{3}{c}{\textbf{LIF}}     & \multicolumn{3}{c}{\textbf{SRM}}        \\
    \cmidrule(r){4-6}
    \cmidrule(r){7-9}
    \textbf{Approach}  & SPS & Trained & \makecell[c]{OA \\ (SR$\uparrow$)}    & \makecell[c]{HC-v3 \\ (Reward$\uparrow$)}   & \makecell[c]{Ant-v3 \\ (Reward$\uparrow$)}    & \makecell[c]{OA \\ (SR$\uparrow$)}    & \makecell[c]{HC-v3 \\ (Reward$\uparrow$)}   & \makecell[c]{Ant-v3 \\ (Reward$\uparrow$)} \\
    \hline
    \DTname\ & \makecell[c]{\gb{Yes}} & \makecell[c]{\gb{Yes}} & \makecell[c]{92.5\%}   & \makecell[c]{11064}  & \makecell[c]{5726}  & \makecell[c]{90.5\%}  & \makecell[c]{11960}   &  \makecell[c]{5879}    \\
    \hline
    \DTname\ & \makecell[c]{\rb{No}} & \makecell[c]{\gb{Yes}}   & \makecell[c]{0\%}  & \makecell[c]{-35} & \makecell[c]{-9}   &\makecell[c]{0\%}  & \makecell[c]{-28}   &   \makecell[c]{-18}   \\
    \DTname\ & \makecell[c]{\gb{Yes}} & \makecell[c]{\rb{No}}  & \makecell[c]{0\%}  & \makecell[c]{-124} & \makecell[c]{-73}   &\makecell[c]{0\%}  & \makecell[c]{-59}   &   \makecell[c]{3}   \\  
    \bottomrule
  \end{tabular}
\end{table}
