# Supplementary material for: Biologically Inspired Dynamic Thresholds for Spiking Neural Networks
Source: arXiv:2206.04426 source file (2023-06-19)
Supplement: Supplementary file 11 [file CC_Ant_additional.tex]

%%%%%%%%%%%%%%%%%%%%%%%%%%%%%%%%%%% Ant-v3 T=25 %%%%%%%%%%%%%%%%%%%%%%%%%%%%%%%

% \begin{table}
% \vspace{-0.5cm}
% \centering
%   \caption{\tb{Quantitative performance of Mujoco Ant-v3. ($T=25$)}}

%   \vspace{0.2cm}
%   \label{tab:Degraded environment mujoco HC t25}

%   \centering
%   \small
%   \setlength\tabcolsep{2pt}
%   \begin{tabular}{lll}
%     \toprule
        
%      & \multicolumn{1}{c}{\textbf{LIF}}     & \multicolumn{1}{c}{\textbf{SRM}}                \\
%     \cmidrule(r){2-2}
%     \cmidrule(r){3-3}
%      \textbf{Name}  & \makecell[c]{Reward$\uparrow$}      &  \makecell[c]{Reward$\uparrow$}      \\
%     \hline
%     PopSAN  & \makecell[c]{5711 ($\sigma\mbox{-}105$)}      & \makecell[c]{5612 ($\sigma\mbox{-}105$)}   \\

%     DT1~\cite{hao2020biologically}   & \makecell[c]{5218 ($\sigma\mbox{-}164$)}     &   \makecell[c]{5121 ($\sigma\mbox{-}117$)} \\
%     DT2~\cite{kim2021spiking}  &  \makecell[c]{3628 ($\sigma\mbox{-}180$)}    &  \makecell[c]{4016 ($\sigma\mbox{-}445$)}    \\
%     % DT3~\cite{sengupta2019going}   & 49.93    & 19.27   & 63.5\%  & 51.35 & 19.23 & 52.5\%  \\
%     \hline
%     DET only  & \makecell[c]{4957 ($\sigma\mbox{-}113$)}    &  \makecell[c]{5125 ($\sigma\mbox{-}144$)} \\
%     DTT only  & \makecell[c]{5192 ($\sigma\mbox{-}267$)}      &   \makecell[c]{4864 ($\sigma\mbox{-}187$)}  \\
%     \hline
%     \DTname\   & \makecell[c]{\textbf{5884}} ($\sigma\mbox{-}97$)      & \makecell[c]{\textbf{5942}} ($\sigma\mbox{-}136$)  \\
%     \bottomrule
%   \end{tabular}
%   \vspace{-0.3cm}
% \end{table}
  
  

% \begin{table}
% \vspace{-0.3cm}
%     \caption{\tb{Quantitative performance of Mujoco Ant-v3 with degraded inputs. ($T=25$)}}
%   \label{tab:Degraded inputs mujoco HC t25}
%   \centering
%     % \scriptsize
%   \fontsize{7pt}{\baselineskip}\selectfont
%   \setlength\tabcolsep{4pt}
%   \begin{tabular}{llllllllllll}
%     \toprule
     
%      & & \multicolumn{1}{c}{\textbf{LIF}}     & \multicolumn{1}{c}{\textbf{SRM}}  & & & \multicolumn{1}{c}{\textbf{LIF}}     & \multicolumn{1}{c}{\textbf{SRM}}  & & & \multicolumn{1}{c}{\textbf{LIF}}     & \multicolumn{1}{c}{\textbf{SRM}}            \\
%     \cmidrule(r){3-3}
%     \cmidrule(r){4-4}
%     \cmidrule(r){7-7}
%     \cmidrule(r){8-8}
%     \cmidrule(r){11-11}
%     \cmidrule(r){12-12}
%       \textbf{Type} & \textbf{Name}  & \makecell[c]{Reward$\uparrow$}        &  \makecell[c]{Reward$\uparrow$}    &\textbf{ Type} & \textbf{Name}  & \makecell[c]{Reward$\uparrow$}        &  \makecell[c]{Reward$\uparrow$}    &\textbf{ Type} & \textbf{Name}  & \makecell[c]{Reward$\uparrow$}  &  \makecell[c]{Reward$\uparrow$} 
%       \\
%     \hline
%     \makecell[c]{\multirow{7}{*}{\makecell[c]{Random \\ joint \\ position}}}
%     & PopSAN  & \makecell[c]{2544 ($\sigma\mbox{-}337$)}    & \makecell[c]{3036 ($\sigma\mbox{-}152$)}   & \makecell[c]{\multirow{6}{*}{\makecell[c]{Random \\ joint \\ velocity}}}   & PopSAN  & \makecell[c]{2858 ($\sigma\mbox{-}149$)}   & \makecell[c]{2287 ($\sigma\mbox{-}427$)} &
%   \makecell[c]{\multirow{6}{*}{GN}} &
%     PopSAN & \makecell[c]{1022 ($\sigma\mbox{-}358$)}   & \makecell[c]{1059 ($\sigma\mbox{-}217$)}   \\
%     & DT1~\cite{hao2020biologically}   & \makecell[c]{1380 ($\sigma\mbox{-}158$)}     &  \makecell[c]{1258 ($\sigma\mbox{-}150$)}    & & DT1~\cite{hao2020biologically}     & \makecell[c]{2643 ($\sigma\mbox{-}259$)}       & \makecell[c]{2574 ($\sigma\mbox{-}232$)}     & & DT1~\cite{hao2020biologically}    & \makecell[c]{875 ($\sigma\mbox{-}270$)}      &  \makecell[c]{1012 ($\sigma\mbox{-}178$)}   \\
%     & DT2~\cite{kim2021spiking} & \makecell[c]{1335 ($\sigma\mbox{-}206$)}   & \makecell[c]{1364 ($\sigma\mbox{-}152$)}  & &  DT2~\cite{kim2021spiking}  & \makecell[c]{1595 ($\sigma\mbox{-}131$)}       &  \makecell[c]{1009 ($\sigma\mbox{-}208$)} 
%     & & DT2~\cite{kim2021spiking}  &   \makecell[c]{664 ($\sigma\mbox{-}163$)}    &   \makecell[c]{623 ($\sigma\mbox{-}235$) }   \\
%     \cline{2-4}
%     \cline{6-8}
%     \cline{10-12}
%     & DET only  & \makecell[c]{2862 ($\sigma\mbox{-}342$)}    & \makecell[c]{2994 ($\sigma\mbox{-}332$)}    & & DET only  & \makecell[c]{2802 ($\sigma\mbox{-}197$)}      & \makecell[c]{2896 ($\sigma\mbox{-}372$)}    & & DET only  & \makecell[c]{844 ($\sigma\mbox{-}304$)}     & \makecell[c]{1105 ($\sigma\mbox{-}364$)}   \\
%     & DTT only  & \makecell[c]{2305 ($\sigma\mbox{-}373$)}      & \makecell[c]{2273 ($\sigma\mbox{-}162$)}  & & DTT only  & \makecell[c]{2699 ($\sigma\mbox{-}255$)}       & \makecell[c]{2618 ($\sigma\mbox{-}260$)}    &  & DTT only   & \makecell[c]{906 ($\sigma\mbox{-}170$)}      & \makecell[c]{1255 ($\sigma\mbox{-}218$)} \\
%     \cline{2-4}
%     \cline{6-8}
%     \cline{10-12}
%     & \DTname\   & \makecell[c]{\textbf{3320 ($\sigma\mbox{-}126$)}}     & \makecell[c]{\textbf{3427}} ($\sigma\mbox{-}115$)   & & \DTname\   & \makecell[c]{\textbf{3217 ($\sigma\mbox{-}119$)}}      & \makecell[c]{\textbf{2996}} ($\sigma\mbox{-}195$)
%     & & \DTname\   & \makecell[c]{\textbf{1339 ($\sigma\mbox{-}156$)}}       & \makecell[c]{\textbf{1576}} ($\sigma\mbox{-}161$)\\
%     \bottomrule
%   \end{tabular}
% \vspace{-0.3cm}
% \end{table}



% \begin{table}
% \vspace{-0.3cm}
%     \caption{\tb{Quantitative performance of Mujoco Ant-v3 with weight uncertainly. ($T=25$)}}
%   \label{tab:Weight pollution mujoco HC t25}
%   \centering
% %   \scriptsize
%   \fontsize{7pt}{\baselineskip}\selectfont
%   \setlength\tabcolsep{4pt}
%   \begin{tabular}{llllllllllll}
%     \toprule
     
%      & & \multicolumn{1}{c}{\textbf{LIF}}     & \multicolumn{1}{c}{\textbf{SRM}}  & & & \multicolumn{1}{c}{\textbf{LIF}}     & \multicolumn{1}{c}{\textbf{SRM}}  & & & \multicolumn{1}{c}{\textbf{LIF}}     & \multicolumn{1}{c}{\textbf{SRM}}            \\
%     \cmidrule(r){3-3}
%     \cmidrule(r){4-4}
%     \cmidrule(r){7-7}
%     \cmidrule(r){8-8}
%     \cmidrule(r){11-11}
%     \cmidrule(r){12-12}
%       \textbf{Type} & \textbf{Name}  & \makecell[c]{Reward$\uparrow$}        &  \makecell[c]{Reward$\uparrow$}    &\textbf{ Type} & \textbf{Name}  & \makecell[c]{Reward$\uparrow$}        &  \makecell[c]{Reward$\uparrow$}    &\textbf{ Type} & \textbf{Name}  & \makecell[c]{Reward$\uparrow$}  &  \makecell[c]{Reward$\uparrow$} 
%       \\
%     \hline
%     \multirow{7}{*}{\makecell[c]{8-bit \\ Loihi \\ weight}}
%     & PopSAN  & \makecell[c]{5504 ($\sigma\mbox{-}210$)}         & \makecell[c]{5228 ($\sigma\mbox{-}139$)}   & \multirow{7}{*}{\makecell[c]{GN \\ weight}}
%     & PopSAN  & \makecell[c]{667 ($\sigma\mbox{-}1002$)}  &  \makecell[c]{444 ($\sigma\mbox{-}1105$)}   &
%     \multirow{7}{*}{\makecell[c]{ $30\%$ \\ Zero \\ weight}}
%     & PopSAN  & \makecell[c]{273 ($\sigma\mbox{-}633$)}        & \makecell[c]{407 ($\sigma\mbox{-}959$)}    \\
%     & DT1~\cite{hao2020biologically}   & \makecell[c]{4826 ($\sigma\mbox{-}102$)}     &  \makecell[c]{4902 ($\sigma\mbox{-}182$)}    & & DT1~\cite{hao2020biologically}     & \makecell[c]{155 ($\sigma\mbox{-}839$)}       & \makecell[c]{6 ($\sigma\mbox{-}1722$)}     & & DT1~\cite{hao2020biologically}    & \makecell[c]{1200 ($\sigma\mbox{-}1020$)}      &  \makecell[c]{1552 ($\sigma\mbox{-}996$)}   \\
%     & DT2~\cite{kim2021spiking} & \makecell[c]{3266 ($\sigma\mbox{-}93$)}   & \makecell[c]{3676 ($\sigma\mbox{-}86$)}  & &  DT2~\cite{kim2021spiking}  & \makecell[c]{-226 ($\sigma\mbox{-}628$)}       &  \makecell[c]{-198 ($\sigma\mbox{-}883$)} 
%     & & DT2~\cite{kim2021spiking}  &   \makecell[c]{-563 ($\sigma\mbox{-}743$)}    &   \makecell[c]{-183 ($\sigma\mbox{-}1125$)}   \\
%     \cline{2-4}
%     \cline{6-8}
%     \cline{10-12}
%     & DET only  & \makecell[c]{4663 ($\sigma\mbox{-}156$)}    & \makecell[c]{4727 ($\sigma\mbox{-}153$)}    & & DET only  & \makecell[c]{1258 ($\sigma\mbox{-}638$)}      & \makecell[c]{923 ($\sigma\mbox{-}883$)}    & & DET only  & \makecell[c]{1084 ($\sigma\mbox{-}1092$)}     & \makecell[c]{1186 ($\sigma\mbox{-}1084$)}   \\
%     & DTT only  & \makecell[c]{4903 ($\sigma\mbox{-}63$)}      & \makecell[c]{4779 ($\sigma\mbox{-}126$)}  & & DTT only  & \makecell[c]{1448 ($\sigma\mbox{-}644$)}       & \makecell[c]{1310 ($\sigma\mbox{-}867$)}    &  & DTT only   & \makecell[c]{1038 ($\sigma\mbox{-}487$)}      & \makecell[c]{1563 ($\sigma\mbox{-}1049$)} \\
%     \cline{2-4}
%     \cline{6-8}
%     \cline{10-12}
%     & \DTname\   &  \makecell[c]{\textbf{5606 ($\sigma\mbox{-}52$)}}      & \makecell[c]{\textbf{5620}} ($\sigma\mbox{-}143$)   & & \DTname\   & \makecell[c]{\textbf{2780 ($\sigma\mbox{-}621$)}}      & \makecell[c]{\textbf{1669}} ($\sigma\mbox{-}612$) 
%     & & \DTname\   &  \makecell[c]{\textbf{2978 ($\sigma\mbox{-}605$)}}       & \makecell[c]{\textbf{3152}} ($\sigma\mbox{-}924$)\\
%     \bottomrule
%   \end{tabular}
% \vspace{-0.3cm}
% \end{table}








%%%%%%%%%%%%%%%%%%%%%%% homeostasis %%%%%%%%%%%%%%%%%%%
% \begin{table}
%   \caption{The raw homeostasis measurements in the two statistical metrics and the corresponding changes with respect to the baseline condition in Mujoco Ant-v3. ($T=25$)}
% %   \caption{Firing rate evaluation test of different methods on different SNN models in successful trials (T=5)}
%   \label{SMtab:half-v3-t25}
%   \centering
%   \scriptsize
%   \setlength\tabcolsep{5pt}
%   \begin{tabular}{llllllll}
%     \toprule
     
%      & & \multicolumn{3}{c}{\textbf{LIF}}     & \multicolumn{3}{c}{\textbf{SRM}}                \\
%     \cmidrule(r){3-5}
%     \cmidrule(r){6-8}
%      \textbf{Type} & \textbf{Name}  & \makecell[c]{$\text{FR}_m (\Delta)$}        & \makecell[c]{$\text{FR}_{std}^m (\Delta)$}     & \makecell[c]{$\text{FR}_{std}^s (\Delta)$}         & \makecell[c]{$\text{FR}_m (\Delta)$}        & \makecell[c]{$\text{FR}_{std}^m (\Delta)$}     & \makecell[c]{$\text{FR}_{std}^s (\Delta)$}     \\ 
%     \hline
%     \multirow{7}{*}{\makecell[c]{baseline \\ condition}}
%     & PopSAN  & 0.535   & 0.258   & 0.002247   & 0.213  & 0.166   & 0.002027  \\
%     & DT1~\cite{hao2020biologically}   & 0.530 & 0.252 & 0.002688  & 0.453 & 0.244 & 0.001694 \\
%     & DT2~\cite{kim2021spiking}     & 0.753 & 0.230 & 0.004728  & 0.563 & 0.182 & 0.003493\\

%     & DET only   & 0.302  & 0.250   & 0.001947  & 0.334  &  0.192  & 0.001872\\
%     & DTT only &  0.541  & 0.276   &  0.001526  & 0.451 & 0.281 & 0.002485\\
%     & \DTname\  & 0.275  & 0.204    &  0.001503 & 0.222 & 0.195 & 0.001829 \\
%     \hline
%     \multirow{7}{*}{\makecell[c]{Random \\ joint \\ position}}
%     & PopSAN  &   0.549 (0.014) &  0.242 (0.016) &  0.003794 (0.001547) &  0.248 (0.035) &  0.140 (0.026) &  0.003682 (0.001655) \\
%     & DT1~\cite{hao2020biologically}    &   0.522 (0.008) &  0.223 (0.029) &  0.003074 (0.000386) &  0.426 (0.027) &  0.277 (0.033) &  0.002951 (0.001257) \\
%     & DT2~\cite{kim2021spiking}     &   0.692 (0.061) &  0.211 (0.019) &  0.003076 (0.001652) &  0.513 (0.050) &  0.219 (0.037) &  0.002523 (0.000970) \\

%     & DET only   &   0.276 (0.026) &  0.286 (0.036) &  0.002744 (0.000797) &  0.352 (0.018) &  0.224 (0.032) &  0.002642 (0.000770) \\
%     & DTT only   &   0.520 (0.021) &  0.252 (0.024) &  0.002636 (0.001110) &  0.430 (0.021) &  0.246 (0.035) &  0.002206 (0.000279) \\
%     & \DTname\  &   0.280 \textbf{(0.005)} &  0.210 \textbf{(0.006)} &  0.001386 \textbf{(0.000117)} &  0.216 \textbf{(0.006)} &  0.188 \textbf{(0.007)} &  0.001682 \textbf{(0.000147)} \\
%     \hline
%     \multirow{7}{*}{\makecell[c]{Random \\ joint \\ velocity}}
%     & PopSAN  &   0.510 (0.025) &  0.224 (0.034) &  0.001589 (0.000658) &  0.189 (0.024) &  0.121 (0.045) &  0.003472 (0.001445) \\
%     & DT1~\cite{hao2020biologically}    &   0.510 (0.020) &  0.220 (0.032) &  0.003236 (0.000548) &  0.424 (0.029) &  0.281 (0.037) &  0.002692 (0.000998) \\
%     & DT2~\cite{kim2021spiking}     &   0.688 (0.065) &  0.203 (0.027) &  0.003163 (0.001565) &  0.522 (0.041) &  0.220 (0.038) &  0.002732 (0.000761) \\

%     & DET only   &   0.263 (0.039) &  0.294 (0.044) &  0.002583 (0.000636) &  0.353 (0.019) &  0.209 (0.017) &  0.003135 (0.001263) \\
%     & DTT only   &   0.522 (0.019) &  0.259 (0.017) &  0.002184 (0.000658) &  0.426 (0.025) &  0.252 (0.029) &  0.001921 (0.000564) \\
%     & \DTname\  &   0.267 \textbf{(0.008)} &  0.206 \textbf{(0.002)} &  0.001632 \textbf{(0.000129)} &  0.213 \textbf{(0.009)} &  0.190 \textbf{(0.005)} &  0.002005 \textbf{(0.000176)} \\
%     \hline
%     \multirow{7}{*}{\makecell[c]{GN}}
%     & PopSAN  &   0.572 (0.037) &  0.240 (0.018) &  0.004581 (0.002334) &  0.180 (0.033) &  0.120 (0.046) &  0.003148 (0.001121) \\
%     & DT1~\cite{hao2020biologically}    &   0.512 (0.018) &  0.214 (0.038) &  0.002012 (0.000676) &  0.633 \textbf{(0.018)} &  0.269 (0.025) &  0.002885 (0.001191) \\
%     & DT2~\cite{kim2021spiking}     &   0.718 (0.035) &  0.259 (0.029) &  0.002833 (0.001895) &  0.520 (0.043) &  0.232 (0.050) &  0.002148 (0.001345) \\

%     & DET only   &   0.323 (0.021) &  0.299 (0.049) &  0.003665 (0.001718) &  0.305 (0.029) &  0.169 (0.023) &  0.002684 (0.000812) \\
%     & DTT only   &   0.512 (0.029) &  0.244 (0.032) &  0.003522 (0.001996) &  0.412 (0.039) &  0.328 (0.047) &  0.003144 (0.000659) \\
%     & \DTname\  &   0.264 \textbf{(0.011)} &  0.200 \textbf{(0.004)} &  0.001400 \textbf{(0.000103)} &  0.204 \textbf{(0.018)} &  0.177 \textbf{(0.018)} &  0.002129 \textbf{(0.000300)} \\
%     \hline
%     \multirow{7}{*}{\makecell[c]{8-bit \\ Loihi \\ weight}}
%     & PopSAN  &   0.546 (0.011) &  0.275 (0.017) &  0.002569 (0.000322) &  0.225 (0.012) &  0.179 (0.013) &  0.002581 (0.000554) \\
%     & DT1~\cite{hao2020biologically}    &   0.542 (0.012) &  0.264 (0.012) &  0.003189 (0.000501) &  0.421 (0.032) &  0.257 (0.013) &  0.001184 (0.000510) \\
%     & DT2~\cite{kim2021spiking}     &   0.738 (0.015) &  0.220 (0.010) &  0.003680 (0.001048) &  0.545 (0.018) &  0.194 (0.012) &  0.003026 (0.000467) \\

%     & DET only   &   0.316 (0.014) &  0.236 (0.014) &  0.002292 (0.000345) &  0.346 (0.012) &  0.212 (0.020) &  0.002214 (0.000342) \\
%     & DTT only   &   0.554 (0.013) &  0.290 (0.014) &  0.001174 (0.000352) &  0.438 (0.013) &  0.294 (0.013) &  0.002763 (0.000278) \\
%     & \DTname\  &   0.270 \textbf{(0.005)} &  0.200 \textbf{(0.004)} &  0.001576 \textbf{(0.000073)} &  0.218 \textbf{(0.004)} &  0.199 \textbf{(0.004)} &  0.001722 \textbf{(0.000107)} \\
%     \hline
%     \multirow{7}{*}{\makecell[c]{GN \\ weight}}
%     & PopSAN  &   0.493 (0.042) &  0.295 (0.037) &  0.003726 (0.001479) &  0.190 (0.023) &  0.141 (0.025) &  0.005216 (0.003189) \\
%     & DT1~\cite{hao2020biologically}    &  0.482 (0.048) &  0.277 (0.025) &  0.004663 (0.001975) &  0.522 (0.069) &  0.287 (0.043) &  0.003540 (0.001846) \\
%     & DT2~\cite{kim2021spiking}     &   0.715 (0.038) &  0.286 (0.056) &  0.003431 (0.001297) &  0.486 (0.077) &  0.235 (0.053) &  0.004632 (0.001139) \\

%     & DET only   &   0.257 (0.045) &  0.215 (0.035) &  0.001036 (0.000911) &  0.394 (0.060) &  0.227 (0.035) &  0.003373 (0.001501) \\
%     & DTT only   &   0.518 (0.023) &  0.223 (0.053) &  0.003998 (0.002472) &  0.410 (0.041) &  0.342 (0.061) &  0.004025 (0.001540) \\
%     & \DTname\  &   0.265 \textbf{(0.010)} &  0.211 \textbf{(0.007)} &  0.001729 \textbf{(0.000226)} &  0.212 \textbf{(0.010)} &  0.206 \textbf{(0.011)} &  0.002773 \textbf{(0.000944)} \\
%     \hline
%     \multirow{7}{*}{\makecell[c]{30\% \\ Zero \\ weight}}
%     & PopSAN  &   0.510 (0.025) &  0.288 (0.030) &  0.005942 (0.003695) &  0.168 (0.045) &  0.137 (0.029) &  0.004893 (0.002866) \\
%     & DT1~\cite{hao2020biologically}    &   0.457 (0.073) &  0.307 (0.055) &  0.004043 (0.001355) &  0.406 (0.047) &  0.220 (0.024) &  0.003909 (0.002215) \\
%     & DT2~\cite{kim2021spiking}     &   0.685 (0.068) &  0.309 (0.079) &  0.002863 (0.001865) &  0.517 (0.046) &  0.236 (0.054) &  0.005426 (0.001933) \\

%     & DET only   &   0.252 (0.050) &  0.243 \textbf{(0.007)} &  0.001132 (0.000815) &  0.376 (0.042) &  0.232 (0.040) &  0.004387 (0.002515) \\
%     & DTT only   &   0.579 (0.038) &  0.332 (0.056) &  0.003538 (0.002012) &  0.487 (0.036) &  0.256 (0.025) &  0.003692 (0.001207) \\
%     & \DTname\  &   0.263 \textbf{(0.012)} &  0.213 (0.009) &  0.001883 \textbf{(0.000380)} &  0.204 \textbf{(0.018)} &  0.183 \textbf{(0.012)} &  0.002485 \textbf{(0.000656)} \\
    
%     \bottomrule
%   \end{tabular}
% \end{table}

% \begin{figure}[ht!]
% 	\centering
% 	\includegraphics [scale=0.15]{figures/T25_Ant_homeostasis.png}
% 	\vspace{-0.3cm}
% 	\caption{
% 		\bd{The changes of quantified homeostasis with respect to the base condition in Mujoco Ant-v3.(T=25)}
% % 		Firing rate evaluation test of different methods on different SNN models in success trails.
% 	}
% 	\label{fig:T25_Ant_h_changes}
% 	\vspace{-0.5cm}
% \end{figure}


% \begin{figure}[ht!]
% 	\centering
% 	\includegraphics [height=104mm,width=135mm ]{figures/half_homeostasis.png}
% 	\vspace{-0.3cm}
% 	\caption{
% 		\bd{The changes of quantified homeostasis with respect to the base condition in Mujoco Ant-v3.}
% % 		Firing rate evaluation test of different methods on different SNN models in success trails.
% 	}
% 	\label{fig:half_h_changes}
% 	\vspace{-0.5cm}
% \end{figure}


%%%%%%%%%%%%%%%%%%%%%%%%%%%%%%%%%%% Ant-v3 T=25 end %%%%%%%%%%%%%%%%%%%%%%%%%%%%%%%
