# Supplementary material for: Biologically Inspired Dynamic Thresholds for Spiking Neural Networks
Source: arXiv:2206.04426 source file (2023-06-19)
Supplement: Supplementary file 12 [file CC_HC_additional.tex]

%%%%%%%%%%%%%%%%%%%%%%%%%%%% random seed begin %%%%%%%%%%%%%%%%%%%%%%%%%%%%%%


% \begin{table}
% \vspace{-0.5cm}
% \centering
%  \caption{\tb{Random seed Quantitative performance of obstacle avoidance with dynamic obstacles.}}

%   \vspace{0.2cm}
%   \label{tab:0.2 Degraded environment mujoco}

%   \centering
%   \small
%   \setlength\tabcolsep{3pt}
%   \begin{tabular}{lll}
%     \toprule
     
%      & \multicolumn{1}{c}{\textbf{LIF}}     & \multicolumn{1}{c}{\textbf{SRM}}                \\
%     \cmidrule(r){2-2}
%     \cmidrule(r){3-3}
%      \textbf{Name}  & \makecell[c]{Reward$\uparrow$}      &  \makecell[c]{Reward$\uparrow$}      \\
%     \hline
%     random seed 1  & \makecell[c]{\%}      & \makecell[c]{\textbf{\%}}   \\

%     random seed 2  & \makecell[c]{\textbf{92.5\%}}         & \makecell[c]{\textbf{90.5\%}} \\
%     random seed 3  &  \makecell[c]{\%}    &  \makecell[c]{\%}    \\
%     % DT3~\cite{sengupta2019going}   & 49.93    & 19.27   & 63.5\%  & 51.35 & 19.23 & 52.5\%  \\
%     % \hline
%     random seed 4  & \makecell[c]{\%}    &  \makecell[c]{\%} \\
%     random seed 5  & \makecell[c]{\%}      &   \makecell[c]{\%}  \\
%     % \hline
%     \bottomrule
%   \end{tabular}
%   \vspace{-0.3cm}
% \end{table}


% \begin{table}
% \vspace{-0.3cm}
%     \caption{\tb{Random seed Quantitative performance of obstacle avoidance with degraded inputs.}}
%   \label{tab:0.2 Degraded inputs mujoco}
%   \centering
%   \scriptsize
%   \setlength\tabcolsep{4pt}
%   \begin{tabular}{llllllllllll}
%     \toprule
     
%      & & \multicolumn{1}{c}{\textbf{LIF}}     & \multicolumn{1}{c}{\textbf{SRM}}  & & & \multicolumn{1}{c}{\textbf{LIF}}     & \multicolumn{1}{c}{\textbf{SRM}}  & & & \multicolumn{1}{c}{\textbf{LIF}}     & \multicolumn{1}{c}{\textbf{SRM}}            \\
%     \cmidrule(r){3-3}
%     \cmidrule(r){4-4}
%     \cmidrule(r){7-7}
%     \cmidrule(r){8-8}
%     \cmidrule(r){11-11}
%     \cmidrule(r){12-12}
%       \textbf{Noise} & \textbf{Constant}  & \makecell[c]{Reward$\uparrow$}        &  \makecell[c]{Reward$\uparrow$}    &\textbf{ Noise} & \textbf{Constant}  & \makecell[c]{Reward$\uparrow$}        &  \makecell[c]{Reward$\uparrow$}    &\textbf{ Noise} & \textbf{Constant}  & \makecell[c]{Reward$\uparrow$}  &  \makecell[c]{Reward$\uparrow$} 
%       \\
%     \hline
%     \makecell[c]{\multirow{5}{*}{\makecell[c]{0.2}}}
%     & random seed 1  & \makecell[c]{\%}    & \makecell[c]{\%}   & \makecell[c]{\multirow{5}{*}{\makecell[c]{0.6}}}   & random seed 1  & \makecell[c]{\%}   & \makecell[c]{\%} &
%   \makecell[c]{\multirow{5}{*}{GN}} & 
%     random seed 1 & \makecell[c]{\%}   & \makecell[c]{\%}   \\
%     & random seed 2   & \textbf{\makecell[c]{90\%}}      & \makecell[c]{\textbf{79.5\%}}   & & random seed 2    & \textbf{\makecell[c]{84.5\%}}      & \textbf{\makecell[c]{83\%}} 
%     & & random seed 2    & \textbf{\makecell[c]{84.5\%}}       & \makecell[c]{\textbf{82.5\%}}\\
%     & random seed 3 & \makecell[c]{\%}   & \makecell[c]{\%}  & &  random seed 3  & \makecell[c]{\%}       &  \makecell[c]{\%} 
%     & & random seed 3  &   \makecell[c]{\%}    &   \makecell[c]{\%}   \\



%     & random seed 4  & \makecell[c]{\%}    & \makecell[c]{\%}    & & random seed 4  & \makecell[c]{\%}      & \makecell[c]{\%}    & & random seed 4  & \makecell[c]{\%}     & \makecell[c]{\%}   \\
%     & random seed 5  & \makecell[c]{\%}      & \makecell[c]{\%}  & & random seed 5  & \makecell[c]{\%}       & \makecell[c]{\%}    &  & random seed 5   & \makecell[c]{\%}      & \makecell[c]{\%} \\

%     \bottomrule
%   \end{tabular}
% \vspace{-0.3cm}
% \end{table}

% \begin{table}
% \vspace{-0.3cm}
%     \caption{\tb{Random seed Quantitative performance of obstacle avoidance with weight uncertainly.}}
%   \label{tab:0.2 Degraded inputs mujoco}
%   \centering
%   \scriptsize
%   \setlength\tabcolsep{4pt}
%   \begin{tabular}{llllllllllll}
%     \toprule
     
%      & & \multicolumn{1}{c}{\textbf{LIF}}     & \multicolumn{1}{c}{\textbf{SRM}}  & & & \multicolumn{1}{c}{\textbf{LIF}}     & \multicolumn{1}{c}{\textbf{SRM}}  & & & \multicolumn{1}{c}{\textbf{LIF}}     & \multicolumn{1}{c}{\textbf{SRM}}            \\
%     \cmidrule(r){3-3}
%     \cmidrule(r){4-4}
%     \cmidrule(r){7-7}
%     \cmidrule(r){8-8}
%     \cmidrule(r){11-11}
%     \cmidrule(r){12-12}
%       \textbf{Noise} & \textbf{Constant}  & \makecell[c]{Reward$\uparrow$}        &  \makecell[c]{Reward$\uparrow$}    &\textbf{ Noise} & \textbf{Constant}  & \makecell[c]{Reward$\uparrow$}        &  \makecell[c]{Reward$\uparrow$}    &\textbf{ Noise} & \textbf{Constant}  & \makecell[c]{Reward$\uparrow$}  &  \makecell[c]{Reward$\uparrow$} 
%       \\
%     \hline
%     \makecell[c]{\multirow{5}{*}{\makecell[c]{8-bit \\ Loihi \\ weight}}}
%     & random seed 1  & \makecell[c]{\%}    & \makecell[c]{\%}   & \makecell[c]{\multirow{5}{*}{\makecell[c]{GN \\ weight \\ (5 rounds)}}}   & random seed 1  & \makecell[c]{\%}   & \makecell[c]{\%} &
%   \makecell[c]{\multirow{5}{*}{\makecell[c]{$30\%$ \\ Zero \\ weight \\ (5 rounds)}}} & 
%     random seed 1 & \makecell[c]{\%}   & \makecell[c]{\%}   \\
%     & random seed 2   & \textbf{\makecell[c]{90\%}}      & \makecell[c]{\textbf{88.5\%}}     & & random seed 2     & \textbf{\makecell[c]{87.7\%}}      & \textbf{\makecell[c]{61.8\%}}      & & random seed 2    & \textbf{\makecell[c]{77.2\%}}       & \makecell[c]{\textbf{65.2\%}}  \\
%     & random seed 3 & \makecell[c]{\%}   & \makecell[c]{\%}  & &  random seed 3  & \makecell[c]{\%}       &  \makecell[c]{\%} 
%     & & random seed 3  &   \makecell[c]{\%}    &   \makecell[c]{\%}   \\

%     & random seed 4  & \makecell[c]{\%}    & \makecell[c]{\%}    & & random seed 4  & \makecell[c]{\%}      & \makecell[c]{\%}    & & random seed 4  & \makecell[c]{\%}     & \makecell[c]{\%}   \\
%     & random seed 5  & \makecell[c]{\%}      & \makecell[c]{\%}  & & random seed 5  & \makecell[c]{\%}       & \makecell[c]{\%}    &  & random seed 5   & \makecell[c]{\%}      & \makecell[c]{\%} \\

%     \bottomrule
%   \end{tabular}
% \vspace{-0.3cm}
% \end{table}

%%%%%%%%%%%%%%%%%%%%%%%%%%%% random seed end %%%%%%%%%%%%%%%%%%%%%%%%%%%%%%





%%%%%%%%%%%%%%%%%%%%%%%%%%%%%%%%%%% HalfCheetah-v3 T=25 %%%%%%%%%%%%%%%%%%%%%%%%%%%%%%%

% \begin{table}
% \vspace{-0.5cm}
% \centering
%   \caption{\tb{Quantitative performance of Mujoco HalfCheetah-v3. ($T=25$)}}

%   \vspace{0.2cm}
%   \label{tab:Degraded environment mujoco HC t25}

%   \centering
%   \small
%   \setlength\tabcolsep{2pt}
%   \begin{tabular}{lll}
%     \toprule
     
%      & \multicolumn{1}{c}{\textbf{LIF}}     & \multicolumn{1}{c}{\textbf{SRM}}                \\
%     \cmidrule(r){2-2}
%     \cmidrule(r){3-3}
%      \textbf{Name}  & \makecell[c]{Reward$\uparrow$}      &  \makecell[c]{Reward$\uparrow$}      \\
%     \hline
%     PopSAN  & \makecell[c]{11137 ($\sigma\mbox{-}70$)}      & \makecell[c]{11247 ($\sigma\mbox{-}132$)}   \\

%     DT1~\cite{hao2020biologically}   & \makecell[c]{6438 ($\sigma\mbox{-}102$)}     &   \makecell[c]{7001 ($\sigma\mbox{-}82$)} \\
%     DT2~\cite{kim2021spiking}  &  \makecell[c]{5523 ($\sigma\mbox{-}67$)}    &  \makecell[c]{5311 ($\sigma\mbox{-}113$)}    \\
%     % DT3~\cite{sengupta2019going}   & 49.93    & 19.27   & 63.5\%  & 51.35 & 19.23 & 52.5\%  \\
%     \hline
%     DET only  & \makecell[c]{9704 ($\sigma\mbox{-}125$)}    &  \makecell[c]{9619 ($\sigma\mbox{-}105$)} \\
%     DTT only  & \makecell[c]{10221 ($\sigma\mbox{-}57$)}      &   \makecell[c]{10563 ($\sigma\mbox{-}83$)}  \\
%     \hline
%     \DTname\   & \makecell[c]{\textbf{11209 ($\sigma\mbox{-}56$)}}         & \makecell[c]{\textbf{11956 ($\sigma\mbox{-}95$)}}  \\
%     \bottomrule
%   \end{tabular}
%   \vspace{-0.3cm}
% \end{table}
  




% \begin{table}
% \vspace{-0.3cm}
%     \caption{\tb{Quantitative performance of Mujoco HalfCheetah-v3 with degraded inputs. ($T=25$)}}
%   \label{tab:Degraded inputs mujoco HC t25}
%   \centering
%     % \scriptsize
%   \fontsize{7pt}{\baselineskip}\selectfont
%   \setlength\tabcolsep{4pt}
%   \begin{tabular}{llllllllllll}
%     \toprule
     
%      & & \multicolumn{1}{c}{\textbf{LIF}}     & \multicolumn{1}{c}{\textbf{SRM}}  & & & \multicolumn{1}{c}{\textbf{LIF}}     & \multicolumn{1}{c}{\textbf{SRM}}  & & & \multicolumn{1}{c}{\textbf{LIF}}     & \multicolumn{1}{c}{\textbf{SRM}}            \\
%     \cmidrule(r){3-3}
%     \cmidrule(r){4-4}
%     \cmidrule(r){7-7}
%     \cmidrule(r){8-8}
%     \cmidrule(r){11-11}
%     \cmidrule(r){12-12}
%       \textbf{Type} & \textbf{Name}  & \makecell[c]{Reward$\uparrow$}        &  \makecell[c]{Reward$\uparrow$}    &\textbf{ Type} & \textbf{Name}  & \makecell[c]{Reward$\uparrow$}        &  \makecell[c]{Reward$\uparrow$}    &\textbf{ Type} & \textbf{Name}  & \makecell[c]{Reward$\uparrow$}  &  \makecell[c]{Reward$\uparrow$} 
%       \\
%     \hline
%     \makecell[c]{\multirow{7}{*}{\makecell[c]{Random \\ joint \\ position}}}
%     & PopSAN  & \makecell[c]{7947 ($\sigma\mbox{-}253$)}    & \makecell[c]{7167 ($\sigma\mbox{-}197$)}   & \makecell[c]{\multirow{6}{*}{\makecell[c]{Random \\ joint \\ velocity}}}   & PopSAN  & \makecell[c]{7223 ($\sigma\mbox{-}165$)}   & \makecell[c]{6583 ($\sigma\mbox{-}168$)} &
%   \makecell[c]{\multirow{6}{*}{GN}} &
%     PopSAN & \makecell[c]{2393 ($\sigma\mbox{-}214$)}   & \makecell[c]{3494 ($\sigma\mbox{-}187$)}   \\
%     & DT1~\cite{hao2020biologically}   & \makecell[c]{3835 ($\sigma\mbox{-}248$)}     &  \makecell[c]{6792 ($\sigma\mbox{-}157$)}    & & DT1~\cite{hao2020biologically}     & \makecell[c]{3203 ($\sigma\mbox{-}148$)}       & \makecell[c]{3855 ($\sigma\mbox{-}202$)}     & & DT1~\cite{hao2020biologically}    & \makecell[c]{2773 ($\sigma\mbox{-}198$)}      &  \makecell[c]{2355 ($\sigma\mbox{-}120$)}   \\
%     & DT2~\cite{kim2021spiking} & \makecell[c]{3950 ($\sigma\mbox{-}192$)}   & \makecell[c]{3213 ($\sigma\mbox{-}230$)} & &  DT2~\cite{kim2021spiking}  & \makecell[c]{3506 ($\sigma\mbox{-}208$)}       &  \makecell[c]{2965 ($\sigma\mbox{-}241$)} 
%     & & DT2~\cite{kim2021spiking}  &   \makecell[c]{2281 ($\sigma\mbox{-}223$)}    &   \makecell[c]{2210 ($\sigma\mbox{-}251$)}   \\
%     \cline{2-4}
%     \cline{6-8}
%     \cline{10-12}
%     & DET only  & \makecell[c]{8051 ($\sigma\mbox{-}148$)}    & \makecell[c]{3502 ($\sigma\mbox{-}323$)}    & & DET only  & \makecell[c]{6498 ($\sigma\mbox{-}219$)}      & \makecell[c]{6435 ($\sigma\mbox{-}213$)}    & & DET only  & \makecell[c]{2807 ($\sigma\mbox{-}163$)}     & \makecell[c]{3061 ($\sigma\mbox{-}155$)}   \\
%     & DTT only  & \makecell[c]{6922 ($\sigma\mbox{-}202$)}      & \makecell[c]{7493 ($\sigma\mbox{-}182$)}  & & DTT only  & \makecell[c]{7363 ($\sigma\mbox{-}150$)}       & \makecell[c]{6762 ($\sigma\mbox{-}247$)}    &  & DTT only   & \makecell[c]{3281 ($\sigma\mbox{-}173$)}      & \makecell[c]{2855 ($\sigma\mbox{-}115$)} \\
%     \cline{2-4}
%     \cline{6-8}
%     \cline{10-12}
%     & \DTname\   & \makecell[c]{\textbf{8463 ($\sigma\mbox{-}130$)}}     & \makecell[c]{\textbf{7846 ($\sigma\mbox{-}70$)}}   & & \DTname\   & \makecell[c]{\textbf{8422 ($\sigma\mbox{-}94$)}}      & \makecell[c]{\textbf{7127 ($\sigma\mbox{-}131$)}} 
%     & & \DTname\   & \makecell[c]{\textbf{3965 ($\sigma\mbox{-}83$)}}       & \makecell[c]{\textbf{3852 ($\sigma\mbox{-}69$)}}\\
%     \bottomrule
%   \end{tabular}
% \vspace{-0.3cm}
% \end{table}


% \begin{table}
% \vspace{-0.3cm}
%     \caption{\tb{Quantitative performance of Mujoco HalfCheetah-v3 with weight uncertainly.}}
%   \label{tab:Weight pollution mujoco}
%   \centering
% %   \scriptsize
%   \fontsize{7pt}{\baselineskip}\selectfont
%   \setlength\tabcolsep{2.8pt}
%   \begin{tabular}{llllllllllll}
%     \toprule
     
%      & & \multicolumn{1}{c}{\textbf{LIF}}     & \multicolumn{1}{c}{\textbf{SRM}}  & & & \multicolumn{1}{c}{\textbf{LIF}}     & \multicolumn{1}{c}{\textbf{SRM}}  & & & \multicolumn{1}{c}{\textbf{LIF}}     & \multicolumn{1}{c}{\textbf{SRM}}            \\
%     \cmidrule(r){3-3}
%     \cmidrule(r){4-4}
%     \cmidrule(r){7-7}
%     \cmidrule(r){8-8}
%     \cmidrule(r){11-11}
%     \cmidrule(r){12-12}
%       \textbf{Noise} & \textbf{Name}  & \makecell[c]{Reward$\uparrow$}        &  \makecell[c]{Reward$\uparrow$}    &\textbf{ Noise} & \textbf{Name}  & \makecell[c]{Reward$\uparrow$}        &  \makecell[c]{Reward$\uparrow$}    &\textbf{ Noise} & \textbf{Name}  & \makecell[c]{Reward$\uparrow$}  &  \makecell[c]{Reward$\uparrow$} 
%       \\
%     \hline
%     \multirow{7}{*}{\makecell[c]{8-bit \\ Loihi \\ weight}}
%     & PopSAN  & \makecell[c]{10505 ($\sigma\mbox{-}690$)}         & \makecell[c]{10602 ($\sigma\mbox{-}984$)}   & \multirow{7}{*}{\makecell[c]{GN \\ weight}}
%     & PopSAN  & \makecell[c]{4640 ($\sigma\mbox{-}1320$)}  &  \makecell[c]{3583 ($\sigma\mbox{-}1288$)}   &
%     \multirow{7}{*}{\makecell[c]{ $30\%$ \\ Zero \\ weight}}
%     & PopSAN  & \makecell[c]{5020 ($\sigma\mbox{-}1206$)}        & \makecell[c]{3233 ($\sigma\mbox{-}1283$)}    \\
%     & DT1~\cite{hao2020biologically}   & \makecell[c]{}     &  \makecell[c]{}    & & DT1~\cite{hao2020biologically}     & \makecell[c]{}       & \makecell[c]{}     & & DT1~\cite{hao2020biologically}    & \makecell[c]{}      &  \makecell[c]{}   \\
%     & DT2~\cite{kim2021spiking} & \makecell[c]{}   & \makecell[c]{}  & &  DT2~\cite{kim2021spiking}  & \makecell[c]{}       &  \makecell[c]{} 
%     & & DT2~\cite{kim2021spiking}  &   \makecell[c]{}    &   \makecell[c]{}   \\
%     \cline{2-4}
%     \cline{6-8}
%     \cline{10-12}
%     & DET only  & \makecell[c]{}    & \makecell[c]{}    & & DET only  & \makecell[c]{}      & \makecell[c]{}    & & DET only  & \makecell[c]{}     & \makecell[c]{}   \\
%     & DTT only  & \makecell[c]{}      & \makecell[c]{}  & & DTT only  & \makecell[c]{}       & \makecell[c]{}    &  & DTT only   & \makecell[c]{}      & \makecell[c]{} \\
%     \cline{2-4}
%     \cline{6-8}
%     \cline{10-12}
%     & \DTname\   &  \makecell[c]{\textbf{10923} ($\sigma\mbox{-}698$)}      & \makecell[c]{\textbf{11877} ($\sigma\mbox{-}982$)}   & & \DTname\   & \makecell[c]{\textbf{6928} ($\sigma\mbox{-}1124$)}      & \makecell[c]{\textbf{8381} ($\sigma\mbox{-}1203$)} 
%     & & \DTname\   &  \makecell[c]{\textbf{6551} ($\sigma\mbox{-}1093$)}       & \makecell[c]{\textbf{5386} ($\sigma\mbox{-}1164$)}\\
%     \bottomrule
%   \end{tabular}
% \vspace{-0.3cm}
% \end{table}


% \begin{table}
% \vspace{-0.3cm}
%     \caption{\tb{Quantitative performance of Mujoco HalfCheetah-v3 with weight uncertainly. ($T=25$)}}
%   \label{tab:Weight pollution mujoco HC t25}
%   \centering
% %   \scriptsize
%   \fontsize{7pt}{\baselineskip}\selectfont
%   \setlength\tabcolsep{4pt}
%   \begin{tabular}{llllllllllll}
%     \toprule
     
%      & & \multicolumn{1}{c}{\textbf{LIF}}     & \multicolumn{1}{c}{\textbf{SRM}}  & & & \multicolumn{1}{c}{\textbf{LIF}}     & \multicolumn{1}{c}{\textbf{SRM}}  & & & \multicolumn{1}{c}{\textbf{LIF}}     & \multicolumn{1}{c}{\textbf{SRM}}            \\
%     \cmidrule(r){3-3}
%     \cmidrule(r){4-4}
%     \cmidrule(r){7-7}
%     \cmidrule(r){8-8}
%     \cmidrule(r){11-11}
%     \cmidrule(r){12-12}
%       \textbf{Type} & \textbf{Name}  & \makecell[c]{Reward$\uparrow$}        &  \makecell[c]{Reward$\uparrow$}    &\textbf{ Type} & \textbf{Name}  & \makecell[c]{Reward$\uparrow$}        &  \makecell[c]{Reward$\uparrow$}    &\textbf{ Type} & \textbf{Name}  & \makecell[c]{Reward$\uparrow$}  &  \makecell[c]{Reward$\uparrow$} 
%       \\
%     \hline
%     \multirow{7}{*}{\makecell[c]{8-bit \\ Loihi \\ weight}}
%     & PopSAN  & \makecell[c]{10926 ($\sigma\mbox{-}59$)}         & \makecell[c]{10850 ($\sigma\mbox{-}44$)}   & \multirow{7}{*}{\makecell[c]{GN \\ weight}}
%     & PopSAN  & \makecell[c]{4816 ($\sigma\mbox{-}583$)}  &  \makecell[c]{3597 ($\sigma\mbox{-}426$)}   &
%     \multirow{7}{*}{\makecell[c]{ $30\%$ \\ Zero \\ weight}}
%     & PopSAN  & \makecell[c]{5078 ($\sigma\mbox{-}1031$)}        & \makecell[c]{3304 ($\sigma\mbox{-}950$)}    \\
%     & DT1~\cite{hao2020biologically}   & \makecell[c]{5883 ($\sigma\mbox{-}102$)}     &  \makecell[c]{6420 ($\sigma\mbox{-}97$)}    & & DT1~\cite{hao2020biologically}     & \makecell[c]{4365 ($\sigma\mbox{-}466$)}       & \makecell[c]{4051 ($\sigma\mbox{-}760$)}     & & DT1~\cite{hao2020biologically}    & \makecell[c]{3927 ($\sigma\mbox{-}1406$)}      &  \makecell[c]{3484 ($\sigma\mbox{-}772$)}   \\
%     & DT2~\cite{kim2021spiking} & \makecell[c]{4301 ($\sigma\mbox{-}87$)}   & \makecell[c]{4636 ($\sigma\mbox{-}74$)}  & &  DT2~\cite{kim2021spiking}  & \makecell[c]{1402 ($\sigma\mbox{-}721$)}       &  \makecell[c]{1982 ($\sigma\mbox{-}993$)} 
%     & & DT2~\cite{kim2021spiking}  &   \makecell[c]{2713 ($\sigma\mbox{-}1352$)}    &   \makecell[c]{3002 ($\sigma\mbox{-}582$)}   \\
%     \cline{2-4}
%     \cline{6-8}
%     \cline{10-12}
%     & DET only  & \makecell[c]{9474 ($\sigma\mbox{-}137$)}    & \makecell[c]{9376 ($\sigma\mbox{-}82$)}    & & DET only  & \makecell[c]{5313 ($\sigma\mbox{-}801$)}      & \makecell[c]{5035 ($\sigma\mbox{-}652$)}    & & DET only  & \makecell[c]{4406 ($\sigma\mbox{-}822$)}     & \makecell[c]{4692 ($\sigma\mbox{-}515$)}   \\
%     & DTT only  & \makecell[c]{9968 ($\sigma\mbox{-}69$)}      & \makecell[c]{9645 ($\sigma\mbox{-}113$)}  & & DTT only  & \makecell[c]{4238 ($\sigma\mbox{-}468$)}       & \makecell[c]{6327 ($\sigma\mbox{-}403$)}    &  & DTT only   & \makecell[c]{3604 ($\sigma\mbox{-}662$)}      & \makecell[c]{3359 ($\sigma\mbox{-}705$)} \\
%     \cline{2-4}
%     \cline{6-8}
%     \cline{10-12}
%     & \DTname\   &  \makecell[c]{\textbf{10990 ($\sigma\mbox{-}61$)}}      & \makecell[c]{\textbf{11760 ($\sigma\mbox{-}68$)}}   & & \DTname\   & \makecell[c]{\textbf{6957 ($\sigma\mbox{-}429$)}}      & \makecell[c]{\textbf{8321 ($\sigma\mbox{-}352$)}} 
%     & & \DTname\   &  \makecell[c]{\textbf{6619 ($\sigma\mbox{-}712$)}}       & \makecell[c]{\textbf{5474 ($\sigma\mbox{-}388$)}}\\
%     \bottomrule
%   \end{tabular}
% \vspace{-0.3cm}
% \end{table}







%%%%%%%%%%%%%%%%%%%%%%% homeostasis %%%%%%%%%%%%%%%%%%%
% \begin{table}
%   \caption{The raw homeostasis measurements in the two statistical metrics and the corresponding changes with respect to the baseline condition in Mujoco HalfCheetah-v3. ($T=25$)}
% %   \caption{Firing rate evaluation test of different methods on different SNN models in successful trials (T=5)}
%   \label{SMtab:half-v3-t25}
%   \centering
%   \scriptsize
%   \setlength\tabcolsep{5pt}
%   \begin{tabular}{llllllll}
%     \toprule
     
%      & & \multicolumn{3}{c}{\textbf{LIF}}     & \multicolumn{3}{c}{\textbf{SRM}}                \\
%     \cmidrule(r){3-5}
%     \cmidrule(r){6-8}
%      \textbf{Type} & \textbf{Name}  & \makecell[c]{$\text{FR}_m (\Delta)$}        & \makecell[c]{$\text{FR}_{std}^m (\Delta)$}     & \makecell[c]{$\text{FR}_{std}^s (\Delta)$}         & \makecell[c]{$\text{FR}_m (\Delta)$}        & \makecell[c]{$\text{FR}_{std}^m (\Delta)$}     & \makecell[c]{$\text{FR}_{std}^s (\Delta)$}     \\ 
%     \hline
%     \multirow{7}{*}{\makecell[c]{baseline \\ condition}}
%     & PopSAN  & 0.436    & 0.230   & 0.001156    & 0.440  & 0.252   & 0.002217  \\
%     & DT1~\cite{hao2020biologically}   & 0.420 & 0.240 & 0.001158 & 0.470 & 0.247 & 0.001869 \\
%     & DT2~\cite{kim2021spiking}     & 0.676  & 0.290 & 0.000939 & 0.521 & 0.305 & 0.001785\\

%     & DET only   & 0.292 & 0.225 & 0.001237  & 0.341  & 0.253 & 0.001631\\
%     & DTT only & 0.635 & 0.257 & 0.002433  & 0.493 & 0.340 & 0.002722 \\
%     & \DTname\  & 0.251 & 0.192 & 0.001292 & 0.215 & 0.173 & 0.001074 \\
%     \hline
%     \multirow{7}{*}{\makecell[c]{Random \\ joint \\ position}}
%     & PopSAN  &   0.426 (0.010) &  0.238 (0.008) &  0.001381 (0.000225) &  0.458 (0.018) &  0.264 (0.012) &  0.003048 (0.000831) \\
%     & DT1~\cite{hao2020biologically}    &   0.440 (0.020) &   0.258 (0.018) &   0.001721 (0.000563) &  0.442 (0.028) &  0.268 (0.021) &  0.003632 (0.001763) \\
%     & DT2~\cite{kim2021spiking}     &   0.648 (0.028) &  0.272 (0.018) &  0.001348 (0.000409) &  0.501 (0.020) &  0.342 (0.037) &  0.002384 (0.000599) \\

%     & DET only   &   0.301 (0.009) &  0.236 (0.011) &  0.001464 (0.000227) &  0.359 (0.018) &  0.285 (0.032) &  0.002179 (0.000548) \\
%     & DTT only   &   0.630 (0.005) &  0.265 (0.008) &  0.002104 (0.000329) &  0.518 (0.025) &  0.372 (0.032) &  0.003438 (0.000716) \\
%     & \DTname\  &   0.247 \textbf{(0.004)} &  0.187 \textbf{(0.005)} &  0.001431 \textbf{(0.000139)} &  0.210 \textbf{(0.005)} &  0.163 \textbf{(0.010)} &  0.001242 \textbf{(0.000168)} \\
%     \hline
%     \multirow{7}{*}{\makecell[c]{Random \\ joint \\ velocity}}
%     & PopSAN  &   0.450 (0.014) &  0.239 (0.009) &  0.001425 (0.000269) &  0.474 (0.034) &  0.332 (0.080) &  0.002922 (0.000705) \\
%     & DT1~\cite{hao2020biologically}    &   0.387 (0.033) &  0.258 (0.018) &  0.002474 (0.001316) &  0.427 (0.043) &  0.268 (0.021) &  0.003572 (0.001703) \\
%     & DT2~\cite{kim2021spiking}     &   0.664 (0.012) &  0.261 (0.029) &  0.002582 (0.001643) &  0.487 (0.034) &  0.347 (0.042) &  0.002529 (0.000744) \\

%     & DET only   &   0.310 (0.018) &  0.235 (0.010) &  0.001582 (0.000345) &  0.368 (0.027) &  0.292 (0.039) &  0.002544 (0.000913) \\
%     & DTT only   &   0.627 (0.008) &  0.269 (0.012) &  0.001548 (0.000885) &  0.515 (0.022) &  0.370 (0.030) &  0.003282 (0.000560) \\
%     & \DTname\  &   0.245 \textbf{(0.006)} &  0.185 \textbf{(0.007)} &  0.001478 \textbf{(0.000186)} &  0.208 \textbf{(0.007)} &  0.183 \textbf{(0.010)} &  0.001305 \textbf{(0.000231)} \\
%     \hline
%     \multirow{7}{*}{\makecell[c]{GN}}
%     & PopSAN  &   0.423 (0.013) &  0.252 (0.022) &  0.001633 (0.000477) &  0.403 (0.037) &  0.236 (0.016) &  0.002574 (0.000357) \\
%     & DT1~\cite{hao2020biologically}    &   0.433 (0.013) &  0.221 (0.019) &  0.002061 (0.000903) &  0.552 (0.082) &  0.271 (0.024) &  0.003784 (0.001915) \\
%     & DT2~\cite{kim2021spiking}     &   0.642 (0.034) &  0.310 (0.020) &  0.001385 (0.000446) &  0.480 (0.041) &  0.373 (0.068) &  0.002833 (0.001048) \\

%     & DET only   &   0.281 (0.011) &  0.219 \textbf{(0.006)} &  0.001610 (0.000373) &  0.304 (0.037) &  0.290 (0.037) &  0.003082 (0.001451) \\
%     & DTT only   &   0.622 (0.013) &  0.274 (0.017) &  0.002762 (0.000329) &  0.453 (0.040) &  0.305 (0.035) &  0.002048 (0.000674) \\
%     & \DTname\  &   0.243 \textbf{(0.008)} &  0.184 (0.008) &  0.001512 \textbf{(0.000220)} &  0.226 \textbf{(0.011)} &  0.180 \textbf{(0.007)} &  0.001283 \textbf{(0.000209)} \\
%     \hline
%     \multirow{7}{*}{\makecell[c]{8-bit \\ Loihi \\ weight}}
%     & PopSAN  &   0.432 (0.004) &  0.224 (0.006) &  0.001310 (0.000154) &  0.452 (0.012) &  0.238 (0.014) &  0.001849 (0.000368) \\
%     & DT1~\cite{hao2020biologically}    &   0.427 (0.007) &  0.221 (0.019) &  0.001035 (0.000123) &  0.485 (0.015) &  0.259 (0.012) &  0.002363 (0.000494) \\
%     & DT2~\cite{kim2021spiking}     &   0.661 (0.015) &  0.278 (0.012) &  0.001174 (0.000235) &  0.535 (0.014) &  0.328 (0.023) &  0.001976 (0.000191) \\

%     & DET only   &   0.299 (0.007) &  0.234 (0.009) &  0.001379 (0.000142) &  0.351 (0.010) &  0.267 (0.014)  &  0.001275 (0.000356) \\
%     & DTT only   &   0.644 (0.009) &  0.242 (0.015) &  0.002210 (0.000223) &  0.506 (0.013) &  0.354 (0.014)  &  0.002894 (0.000172) \\
%     & \DTname\  &   0.250 \textbf{(0.001)} &  0.197 \textbf{(0.005)} &  0.001393 \textbf{(0.000101)} &  0.211 \textbf{(0.004)} &  0.178 \textbf{(0.005)} &  0.001169 \textbf{(0.000094)} \\
%     \hline
%     \multirow{7}{*}{\makecell[c]{GN \\ weight}}
%     & PopSAN  &   0.471 (0.035) &  0.211 (0.019) &  0.001637 (0.000481) &  0.479 (0.039) &  0.336 (0.084) &  0.003181 (0.000964) \\
%     & DT1~\cite{hao2020biologically}    &   0.433 \textbf{(0.013)} &   0.218 (0.022) &  0.000904 (0.000254) &  0.438 (0.032) &  0.302 (0.055) &  0.004041 (0.002172) \\
%     & DT2~\cite{kim2021spiking}     &   0.642 (0.034) &  0.320 (0.030) &  0.001683 (0.000744) &  0.492 (0.029) &  0.366 (0.061) &  0.004585 (0.002800) \\

%     & DET only   &   0.271 (0.021) &  0.238 (0.013) &  0.001720 (0.000483) &  0.369 (0.028) &  0.202 (0.051) &  0.003927 (0.002296) \\
%     & DTT only   &   0.607 (0.028) &  0.289 (0.032) &  0.003104 (0.000671) &  0.569 (0.076) &  0.301 (0.039) &  0.004273 (0.001551) \\
%     & \DTname\  &   0.264 \textbf{(0.013)} &  0.183 \textbf{(0.009)} &  0.001512 \textbf{(0.000220)} &  0.229 \textbf{(0.014)} &  0.182 \textbf{(0.009)} &  0.001199 \textbf{(0.000125)} \\
%     \hline
%     \multirow{7}{*}{\makecell[c]{30\% \\ Zero \\ weight}}
%     & PopSAN  &   0.493 (0.057) &  0.215 (0.015) &  0.001892 (0.000736) &  0.410 (0.030) &  0.292 (0.040) &  0.003237 (0.001020) \\
%     & DT1~\cite{hao2020biologically}    &   0.447 (0.027) &  0.258 (0.018) &  0.001859 (0.000701) &  0.424 (0.046) &  0.288 (0.041) &  0.000926 (0.000943) \\
%     & DT2~\cite{kim2021spiking}     &   0.655 (0.021) &  0.334 (0.044) &  0.001674 (0.000735) &  0.486 (0.035) &  0.251 (0.054) &  0.000896 (0.000889) \\

%     & DET only   &   0.273 (0.019) &  0.239 (0.014) &  0.001692 (0.000455) &  0.371 (0.030) &  0.216 (0.037) &  0.004106 (0.002475) \\
%     & DTT only   &   0.677 (0.042) &  0.305 (0.048) &  0.002976 (0.000543) &  0.426 (0.067) &  0.312 (0.028) &  0.001176 (0.001546) \\
%     & \DTname\  &   0.239 \textbf{(0.012)} &  0.181 \textbf{(0.011)} &  0.001642 \textbf{(0.000350)} &  0.221 \textbf{(0.006)} &  0.180 \textbf{(0.007)} &  0.001183 \textbf{(0.000109)} \\
    
%     \bottomrule
%   \end{tabular}
% \end{table}


% \begin{figure}[ht!]
% 	\centering
% 	\includegraphics [scale=0.15]{figures/T25_half_homeostasis.png}
% 	\vspace{-0.3cm}
% 	\caption{
% 		\bd{The changes of quantified homeostasis with respect to the base condition in Mujoco HalfCheetah-v3.(T=25)}
% % 		Firing rate evaluation test of different methods on different SNN models in success trails.
% 	}
% 	\label{fig:T25_half_h_changes}
% 	\vspace{-0.5cm}
% \end{figure}


%%%%%%%%%%%%%%%%%%%%%%%%%%%%%%%%%%% HalfCheetah-v3 T=25 end %%%%%%%%%%%%%%%%%%%%%%%%%%%%%%%
