# Supplementary material for: Biologically Inspired Dynamic Thresholds for Spiking Neural Networks
Source: arXiv:2206.04426 source file (2023-06-19)
Supplement: Supplementary file 13 [file OA_additional.tex]

\subsection*{Additional Quantitative Performance}
\label{SMsec:performance}
In this section, we provide additional experimental results related to obstacle avoidance performance. Specifically, we show the quantitative performance of all competing SNNs in static obstacle avoidance tasks. Besides the reported success rate (SR), we report the following two additional results, namely: Common routes percentage (CRP), the percentage of the successful routes that had the common start and goal positions across all competing SNNs to all successful trials of a specific SNN; b) Overtime percentage (OTP), the percentage of overtime trials to total trials (\ie 200 trials), where overtime is defined as the trial that the robot cannot reach the goal within 1000 steps but without touching any obstacle. 

\noindent
The quantitative performance of all competing SNNs in static obstacle avoidance tasks are shown in Table~\ref{SMtab:Sta_test}. The corresponding testing environment is shown in Figure~\ref{SMfig:env}(b), where we adopt the same 200 start-goal pairs as the ones used for testing SAN. The SRs of all competing SNNs are relatively the same which is ensured by grid search on all tunable hyperparameters. There is no overtime trial among all experiments. Since the lowest SRs are pretty high (\ie 96\% for LIF and 95\% for SRM), the CRPs are also pretty high. 

\noindent
Table~\ref{SMtab:Degraded environment}, ~\ref{SMtab:Degraded inputs}, and ~\ref{SMtab:Weight pollution} show the quantitative performance of all competing approaches in DO, DI, and weight uncertainty experiments, respectively. Since the lowest SRs lower than those obtained in static obstacle avoidance experiments, the CRPs reduce significantly. In terms of OTP, we witness high overtime trials in the `0.2' section of degraded inputs and the `GN weight' section of weight uncertainty. 
As discussed in the main paper, with the `0.2' setup, the three disturbed lasers generate more spikes than it is supposed to, making the robot more cautious. Thus, it slows down the speed of the robot, introducing more over time trials. As expected, adding GN Type to learned weights reduces the effectiveness avoidance policy. However, our approach gets the most negligible impact, offering the best SRs. 

\noindent
As discussed in the main paper, each robot state is encoded into 24 Poisson spike trains, and each spike train has $T$ timesteps. Due to the limited space, we only report the experimental results based on $T=5$ in the main paper. Here, we show the quantitative performance with $T=25$. Our approach still offers the best SRs across all experimental settings. Specifically, in the dynamic obstacle experiments (Table~\ref{SMtab:Degraded environment T=25}), our approach outperforms the runner-ups by a significant marge, 9.5\% with LIF and 12.5\% with SRM; As shown in Table~\ref{SMtab:Degraded inputs T=25}, the proposed \DTname\ improves the SRs of both LIF-based and SRM-based baseline model (i.e., SAN-NR) by at least 11.5\% and 18\%, respectively; Under the three weight uncertainty conditions (see Table~\ref{SMtab:Weight pollution T=25}), the proposed \DTname\ increases the SRs of the baseline model SAN-NR by at least 9.5\%, 14.2\%, and 14.8\%, respectively.

\noindent
Based on Table~\ref{SMtab:Sta_test} and Table~\ref{SMtab:Sta_test T=25}, compared to the SRs obtained with $T=5$ settings, $T=25$ settings only change the SRs slightly (\ie $\pm 0.5\%$), indicating that all competing SNNs are not sensitive to the $T$ value in static obstacle avoidance tasks. The observations also hold in the dynamic obstacle experiments with the two different $T$ value (Table~\ref{SMtab:Degraded environment} vs Table~\ref{SMtab:Degraded environment T=25}). However, We observe the SRs increases with larger $T$ value in the most degraded inputs and weight uncertainty experiments, especially in `GN weight' and `30\% zero weight' settings.

% \tb{T=25} Table~\ref{SMtab:Sta_test T=25}, Table~\ref{SMtab:Degraded environment T=25} T=25 Interference experiments.

% \tb{$\eta$ test} Table~\ref{SMtab:eta}
% \begin{table}
% \caption{Quantitative performance in dynamic obstacles scenes with different $\eta$.}
%   \vspace{0.2cm}
%   \label{SMtab:eta}
%   \centering
%   \small
%   \setlength\tabcolsep{2pt}
%   \begin{tabular}{lllllll}
%     \toprule
     
%      & \multicolumn{3}{c}{\textbf{LIF}}     & \multicolumn{3}{c}{\textbf{SRM}}                \\
%     \cmidrule(r){2-4}
%     \cmidrule(r){5-7}
%      \textbf{$\eta$}  & \makecell[c]{SR$\uparrow$}    &  \makecell[c]{AD(m)$\downarrow$}       & \makecell[c]{AS(m/s)$\uparrow$}        & \makecell[c]{SR$\uparrow$}    &  \makecell[c]{AD(m)$\downarrow$}       & \makecell[c]{AS(m/s)$\uparrow$} \\
%     \hline
%      0.01 & 92.5\% & & & 90.5\%   \\
%      0.05 & 89.5\%  & & & 86.5\% \\

%      0.50  & 87.5\% & & & 79\%\\
%      -0.01 & 91\% &  & &89\% \\
%      -0.50 & 0\%  &  & & 0\% \\
%     \bottomrule
%   \end{tabular}
% \end{table}
