# Supplementary material for: Biologically Inspired Dynamic Thresholds for Spiking Neural Networks
Source: arXiv:2206.04426 source file (2023-06-19)
Supplement: Supplementary file 14 [file OA_experimental_detials.tex]

% \subsection{Additional Experimental details}
\noindent
\label{SMsec:setting}
\bd{
In this section, we provide additional experimental details related to SNNs' inputs and training process in obstacle avoidance tasks. 
}
% In this section, we describe the network input spike train, the training method, settings of heuristic threshold methods, and Loihi weight settings.

\begin{figure}[h]
	\centering

	\includegraphics [height=37mm,width=85mm ]{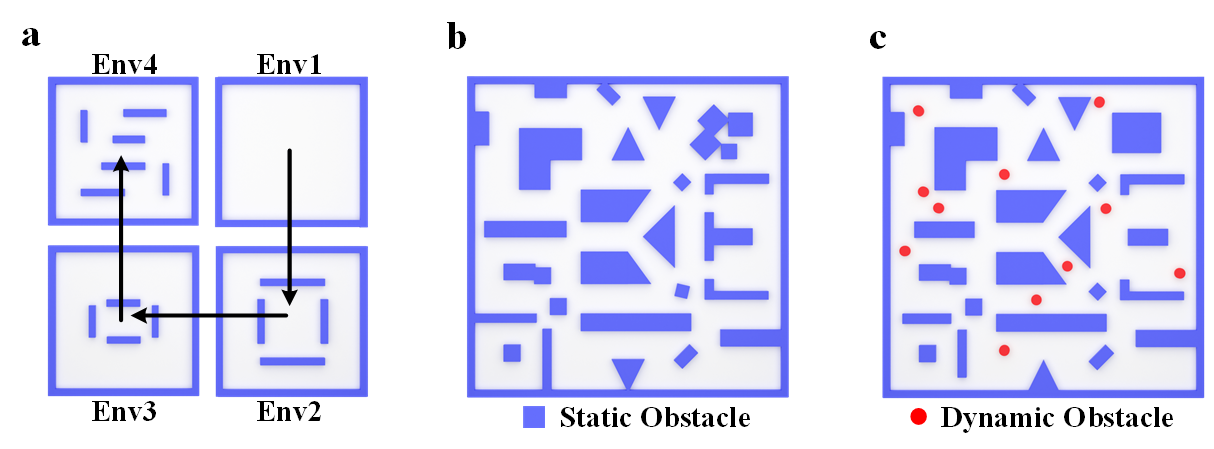}
	\vspace{-0.2cm}
	\caption{
	    \bd{\tb{Illustrations of training, static testing and dynamic testing environment.}
		(a) Four training environments. The training processes of all competing SNNs start from Env1 and end with Env4. (b) Static testing environment, where all obstacles are static. (c) Dynamic obstacle avoidance testing environment. Besides static obstacles, we insert $11$ dynamic obstacles. }
	}
	\label{SMfig:env}
	%\vspace{-0.2cm}
\end{figure}
