# Supplementary material for: Biologically Inspired Dynamic Thresholds for Spiking Neural Networks
Source: arXiv:2206.04426 source file (2023-06-19)
Supplement: Supplementary file 15 [file OA_homeostasis.tex]

% \subsection{Homeostatic experimental setup and raw data}
\subsection*{Additional Obstacle Avoidance Homeostasis Experimental Results}
\label{SMsec:homeostatic}

In the main manuscript, we show the changes of quantified homeostasis of all successful trials with respect to the base condition (\ie homeostasis obtained in the dynamic obstacle experiments) with $T=5$. In Table~\ref{SMtab:hom_success_5}, we provide the raw homeostasis measurements in the three metrics and the corresponding changes used for plotting the polar chart in the main paper. Furthermore, the changes related to failed trials are reported in Table~\ref{SMtab:hom_fail_5} and Figure~\ref{SMfig:fail_hom}. Please note the overtime trials are also counted as failed trials. In terms of $\Delta\text{FR}_m$ and $\Detla\text{FR}_{std}^m$, the measurements between successful and failed trials are relatively the same. However, we witness most failed trials have higher $\Delta\text{FR}_{std}^s$ values than successful trials, especially for the LIF-based SNNs.

\noindent
We also report the measured homeostasis and corresponding changes with $T=25$ in Table~\ref{SMtab:hom_success_25} and Table~\ref{SMtab:hom_fail_25}. The corresponding polar plots are shown in Figure~\ref{SMfig:T25_success_hom} and Figure~\ref{SMfig:T25_fail_hom}. The association between homeostasis and obstacle avoidance success rate still holds. As shown in Figure~\ref{SMfig:T25_success_hom} and Table~\ref{SMtab:hom_success_25}, our approach offers the lowest changes in the three metrics across all experimental settings, except for the $\Detla\text{FR}_{std}^m$ obtained in the SRM-based 8-bit Loihi weight experiment. Meanwhile, the proposed \DTname\ delivers the best obstacle avoidance SRs in all designed experimental conditions with $T=25$ (Table~\ref{SMtab:Degraded environment T=25},~\ref{SMtab:Degraded inputs T=25}, and~\ref{SMtab:Weight pollution T=25}). We observe a similar pattern between successful and failed trials like the one observed with $T=5$ that is: the $\Delta\text{FR}_m$ and $\Detla\text{FR}_{std}^m$ are relatively the same, but most failed trials have higher $\Delta\text{FR}_{std}^s$ value than the ones of the successful trials.

\begin{table}
  \caption{\bd{The raw homeostasis measurements of successful trials in the three statistical metrics and the corresponding changes with respect to the baseline condition. ($T=5$)}}
%   \caption{Firing rate evaluation test of different methods on different SNN models in successful trials ($T=5$)}
  \label{SMtab:hom_success_5}
  \centering
  \scriptsize
  \setlength\tabcolsep{5pt}
  \begin{tabular}{llllllll}
    \toprule
     
     & & \multicolumn{3}{c}{\textbf{LIF ($T=5$)}}     & \multicolumn{3}{c}{\textbf{SRM ($T=5$)}}                \\
    \cmidrule(r){3-5}
    \cmidrule(r){6-8}
     \textbf{Type} & \textbf{Name}  & \makecell[c]{$\text{FR}_m (\Delta)$}        & \makecell[c]{$\text{FR}_{std}^m (\Delta)$}     & \makecell[c]{$\text{FR}_{std}^s (\Delta)$}         & \makecell[c]{$\text{FR}_m (\Delta)$}        & \makecell[c]{$\text{FR}_{std}^m (\Delta)$}     & \makecell[c]{$\text{FR}_{std}^s (\Delta)$}     \\ 
    \hline
    \multirow{7}{*}{\makecell[c]{Dynamic \\ obstacle \\ (baseline \\ condition)}}
    & SAN  &0.523 &0.325  &0.000891  &0.278 &0.301  &0.000596   \\
    & SAN-NR  &0.515  &0.330  &0.001029   &0.487  & 0.309 &0.006853  \\
    & DT1~\cite{hao2020biologically}   &0.443   &0.325    &0.001738 &0.482   &0.310    &0.002942      \\
    & DT2~\cite{kim2021spiking}     &0.400   &0.345  &0.002136  &0.418  &0.309    &0.005873      \\

    & DET only   &0.508  &0.336    &0.001024  &0.380  &0.276    &0.002564 \\
    & DTT only & 0.456  & 0.320        &0.000902   &0.475   &0.294   &0.002284  \\
    & \DTname\  & 0.439   &  0.312    & 0.000916  &0.501   &0.298      &0.001759   \\
    \hline
    \multirow{7}{*}{\makecell[c]{0.2}}
    & SAN  &0.556 (0.033) &0.329 (0.004)  &0.000750 (0.000141)  &0.293 (0.015) &0.247 (0.054)  &0.000746 (0.000150)   \\
    & SAN-NR  &0.565 (0.050)  &0.326 (0.004)  &0.000738 (0.000291)   & 0.508 (0.021)  &0.333 (0.024)  &0.001069 (0.005784)    \\
    & DT1~\cite{hao2020biologically}    &0.479 (0.036)   &0.387 (0.062)    &0.000973 (0.000765)    &0.518 (0.036)   &0.348 (0.038)    &0.003993 (0.001051)   \\
    & DT2~\cite{kim2021spiking}     &0.412 (0.012)  &0.370 (0.025)    &0.001293 (0.000843)    &0.438 (0.020)  &0.325 (0.016)    &0.001709 (0.004164)    \\

    & DET only   &0.495 (0.013)  &0.353 (0.017)    &0.001523 (0.000499)  &0.380 (0.000)  &0.244 (0.032)    &0.003969 (0.001405)    \\
    & DTT only & 0.481 (0.025)  & 0.335 (0.015)        & 0.000768 (0.000134)  &0.420 (0.055)   &0.335 (0.041)         &0.002040 (0.000244)    \\
    & \DTname\  &0.444\textbf{ (0.005)}   &0.315\textbf{ (0.003)}      &0.000851\textbf{ (0.000065)}    &0.494\textbf{ (0.007)}   &0.310\textbf{ (0.012)}      &0.001884\textbf{ (0.000125)}  \\
    \hline
    \multirow{7}{*}{\makecell[c]{6.0}}
    & SAN  &0.564 (0.041) &0.342 (0.017)  &0.001454 (0.000563)  &0.275 (0.003) &0.306 (0.005)  &0.000747 (0.000151)   \\
    & SAN-NR  &0.558 (0.043)  &0.339 (0.009)  &0.001548 (0.000519)   &0.483 (0.004)  &0.306 (0.003)  &0.002533 (0.004320) \\
    & DT1~\cite{hao2020biologically}    &0.432 (0.011)   &0.318 (0.007)    &0.002862 (0.001124)   &0.471 (0.011)  & 0.315 (0.005)   &0.004224 (0.001282)   \\
    & DT2~\cite{kim2021spiking}     &0.407 (0.007)  &0.354 (0.009)    &0.003785 (0.001649)    &0.408 (0.010)  &0.320 (0.011)   &0.005417 (0.000456)  \\

    & DET only   &0.515 (0.007)  &0.374 (0.038)    &0.003088 (0.002064)  &0.377 (0.003)  &0.230 (0.046)    &0.003889 (0.001325)    \\
    & DTT only &0.450 (0.006)   & 0.325 (0.005)        &0.003057 (0.002155)   &0.403 (0.072)   &0.290 (0.004)     &0.002855 (0.000571)   \\
    & \DTname\  & 0.440\textbf{ (0.001)}  &0.317\textbf{ (0.005)}      &0.000960\textbf{ (0.000044)}   &0.501\textbf{ (0.000)}   &0.300\textbf{ (0.002)}     &0.001870\textbf{ (0.000111)}   \\
    \hline
    \multirow{7}{*}{\makecell[c]{GN}}
    & SAN  &0.534 (0.011) &0.310 (0.015)  &0.001416 (0.000525)  &0.287 (0.009) & 0.204 (0.097) &0.000727 (0.000131)  \\
    & SAN-NR  &0.527 (0.012)  &0.314 (0.016)  & 0.001622 (0.000593)  & 0.497 (0.010) &0.298 (0.011) & 0.007395 (0.000542)   \\
    & DT1~\cite{hao2020biologically}    & 0.451 (0.008)  &0.319 (0.006)    &0.000982 (0.000756)  & 0.502 (0.020)  &0.302 (0.008)    &0.004634 (0.001692) \\
    & DT2~\cite{kim2021spiking}     &0.405 (0.005)  &0.337 (0.008)    &0.001654 (0.000482)    &0.423 (0.005)  &0.283 (0.026)    &0.005578 (0.000295)   \\

    & DET only   & 0.502 (0.006) &0.361 (0.025)    &0.001228 (0.000204)  &0.390 (0.010)  &0.283 (0.007)    &0.002454 (0.000110)   \\
    & DTT only &0.445 (0.011)   &0.315 (0.005)         & 0.001453 (0.000551)  &0.390 (0.085)   & 0.308 (0.014)        &0.001968 (0.000316)  \\
    & \DTname\  & 0.443\textbf{ (0.004)}  & 0.307\textbf{ (0.005)}     &0.000880\textbf{ (0.000036)}   &0.500\textbf{ (0.001)}   &0.301\textbf{ (0.003)}    &0.001886\textbf{ (0.000127)}   \\
    \hline
    \multirow{7}{*}{\makecell[c]{8-bit \\ Loihi \\ weight}}
    & SAN  &0.520 (0.003) &0.319 (0.006)  &0.000988 (0.000097)  &0.288 (0.010) &0.314 (0.013)  &0.000731\textbf{ (0.000135)}   \\
    & SAN-NR  &0.513 (0.002)   & 0.334\textbf{ (0.004)}  & 0.001286 (0.000257)    & 0.479 (0.008) &0.315 (0.006) &0.005527 (0.001326)  \\
    & DT1~\cite{hao2020biologically}    &  0.437 (0.006)  & 0.319 (0.006)    & 0.001589 (0.000149)  &0.473 (0.009)  &0.325 (0.015)  &0.002084 (0.000858)     \\
    & DT2~\cite{kim2021spiking}      &0.407 (0.007)   &0.340 (0.005)     &0.001853 (0.000283)    & 0.425 (0.007) &0.316 (0.007)  &0.005638 (0.000235)    \\

    & DET only   & 0.505 (0.003)  & 0.341 (0.005)    &0.000868 (0.000156)   & 0.385 (0.005) &0.285 (0.009)    &0.002185 (0.000379)    \\
    & DTT only & 0.446 (0.010)  & 0.325 (0.005)        & 0.000787 (0.000115)  & 0.460 (0.015)  &0.301 (0.007)   &0.002436 (0.000152)   \\
    & \DTname\  & 0.439\textbf{ (0.000)}  & 0.308\textbf{ (0.004)}     & 0.000932\textbf{ (0.000016)}  &0.500\textbf{ (0.001)}    &0.293\textbf{ (0.005)}      &0.001570 (0.000189) \\
    \hline
    \multirow{7}{*}{\makecell[c]{GN \\ weight \\  (5 rounds)}}
    & SAN  &0.501 (0.022) &0.338 (0.013)  &0.001192 (0.000301)  & - & - & -  \\
    & SAN-NR  &0.490 (0.025)  &0.338 (0.008)  &0.001281 (0.000252)   &0.498 (0.011)  &0.326 (0.017)  &0.004461 (0.002392)    \\
    & DT1~\cite{hao2020biologically}    & 0.407 (0.036)  &0.349 (0.024)    &0.001902 (0.000164)  &0.487 (0.005)   &0.319 (0.009)    &0.003573 (0.000631)     \\
    & DT2~\cite{kim2021spiking}     &0.391 (0.009)  &0.335 (0.010)    & 0.001356 (0.000780)   &0.410 (0.008)  &0.291 (0.018)    & 0.010002 (0.004129)   \\

    & DET only   &0.516 (0.008)  &0.375 (0.039)    &0.002225 (0.001201)  &0.399 (0.019)  &0.212 (0.064)    &0.003675 (0.001111)    \\
    & DTT only &0.467 (0.011)   & 0.327 (0.007)        &0.001244 (0.000342)   &0.387 (0.088)   &  0.301 (0.007)  & 0.002387 (0.000103)  \\
    & \DTname\  &0.444\textbf{ (0.005)}   & 0.318\textbf{ (0.006)}     &0.001013\textbf{ (0.000097)} &0.498\textbf{ (0.003)}   &0.299\textbf{ (0.001)}      &0.001602\textbf{ (0.000157)} \\
    \hline
    \multirow{7}{*}{\makecell[c]{30\% \\ Zero \\ weight\\ (5 rounds)}}
    & SAN  &0.448 (0.075) &0.321\textbf{ (0.004)}  &0.001490 (0.000599)  &- & - & -   \\
    & SAN-NR  &0.454 (0.061)  &0.335 (0.005)  &0.001399 (0.000370)   &0.470 (0.017)  &0.331 (0.022)  &0.009941 (0.003088)  \\
    & DT1~\cite{hao2020biologically}    & 0.387 (0.056)  &0.313 (0.012)    &0.002045 (0.000307)  & 0.456 (0.026)  &0.334 (0.024)    &0.005103 (0.002161)    \\
    & DT2~\cite{kim2021spiking}     &0.377 (0.023)  &0.358 (0.013)    &0.001834 (0.000302)    &0.403 (0.015)  &0.332 (0.023)    &0.003469 (0.002404)   \\

    & DET only   &0.520 (0.012)  &0.387 (0.051)    &0.002582 (0.001558)  &0.356 (0.024)  &0.235 (0.041)    &0.005036 (0.002472)   \\
    & DTT only & 0.470 (0.014)  & 0.337 (0.017)        & 0.002551 (0.001649)  &0.394 (0.081)   &0.274 (0.020)         &0.003706 (0.001422) \\
    & \DTname\  &0.444\textbf{ (0.005) }  & 0.316\textbf{ (0.004)}     &0.000993\textbf{ (0.000077)}   &0.497\textbf{ (0.004)}   &0.318\textbf{ (0.020)}      &0.003855\textbf{ (0.002096)}    \\
    
    \bottomrule
  \end{tabular}
\end{table}

\begin{table}
  \caption{The raw homeostasis measurements of successful trials in the three statistical metrics and the corresponding changes with respect to the baseline condition. ($T=25$)}
  \label{SMtab:hom_success_25}
  \centering
  \scriptsize
  \setlength\tabcolsep{5pt}
  \begin{tabular}{llllllll}
    \toprule
     
     & & \multicolumn{3}{c}{\textbf{LIF ($T=25$)}}     & \multicolumn{3}{c}{\textbf{SRM ($T=25$)}}                \\
    \cmidrule(r){3-5}
    \cmidrule(r){6-8}
     \textbf{Type} & \textbf{Name}  & \makecell[c]{$\text{FR}_m (\Delta)$}        & \makecell[c]{$\text{FR}_{std}^m (\Delta)$}     & \makecell[c]{$\text{FR}_{std}^s (\Delta)$}         & \makecell[c]{$\text{FR}_m (\Delta)$}        & \makecell[c]{$\text{FR}_{std}^m (\Delta)$}     & \makecell[c]{$\text{FR}_{std}^s (\Delta)$}     \\ 
    \hline
    \multirow{7}{*}{\makecell[c]{Dynamic \\ obstacle \\(baseline \\condition)}}
    & SAN  &  0.524  & 0.325  &  0.002098  & 0.285  & 0.306  & 0.001504    \\
    & SAN-NR  & 0.515   & 0.331  & 0.001440  & 0.488   & 0.312  &  0.003486 \\
    & DT1~\cite{hao2020biologically}    & 0.447  & 0.324  &0.002155  & 0.485   & 0.319  & 0.002473 \\
    & DT2~\cite{kim2021spiking}     & 0.401  & 0.347  & 0.002470 & 0.420  &  0.314 & 0.005771\\

    & DET only   & 0.509  & 0.336  & 0.001206  & 0.384  & 0.279  & 0.002483\\
    & DTT only &  0.449  & 0.317   & 0.001736  & 0.475  & 0.301  & 0.002515    \\
    & \DTname\ & 0.439   & 0.311  & 0.001035  & 0.501  & 0.301  & 0.002394\\
    \hline
    \multirow{7}{*}{\makecell[c]{0.2}}
    & SAN  & 0.556 (0.032) & 0.330 (0.005)  & 0.000798 (0.001300)  & 0.294 (0.009) &  0.245 (0.061) & 0.001004 (0.000500)  \\
    & SAN-NR  &  0.566 (0.051)  & 0.326 (0.005)  & 0.000768 (0.000670)  & 0.536 (0.048)  &  0.351 (0.039) & 0.001224 (0.002260) \\
    & DT1~\cite{hao2020biologically}    & 0.481 (0.034) & 0.387 (0.063)  & 0.001097 (0.001060)   & 0.517 (0.032)  & 0.344 (0.025) & 0.003823 (0.001350) \\
    & DT2~\cite{kim2021spiking}     & 0.415 (0.014)  & 0.370 (0.023)   & 0.001662 (0.000810)  & 0.438 (0.018)  & 0.326 (0.012)  & 0.001781 (0.003990) \\

    & DET only   &0.496 (0.013)  &  0.353 (0.017) & 0.001424 (0.000218)  &  0.380 (0.004) & 0.246 (0.033)  &  0.003362 (0.000879) \\
    & DTT only &  0.485 (0.036)  & 0.336 (0.019)  & 0.000972 (0.000760)  & 0.420 (0.055)  & 0.335 (0.034)  &  0.003116 (0.000601) \\
    & \DTname\  & 0.444\textbf{ (0.005)} & 0.314\textbf{ (0.003)}   & 0.001104\textbf{ (0.000069)}  & 0.494\textbf{ (0.007)}  &  0.310\textbf{ (0.010)} &  0.002238\textbf{ (0.000160)}\\
    \hline
    \multirow{7}{*}{\makecell[c]{6.0}}
    & SAN  & 0.558 (0.034) & 0.341 (0.016)  & 0.001415 (0.000683)  & 0.275 (0.010)  & 0.303 (0.003)  & 0.000839 (0.000665) \\
    & SAN-NR  &0.550 (0.035)  & 0.340 (0.009)  & 0.001165 (0.000275)  & 0.484 (0.004)  & 0.306 (0.006)  &  0.003828 (0.000342)  \\
    & DT1~\cite{hao2020biologically}    &0.433 (0.014) & 0.319\textbf{ (0.005)}  & 0.002449 (0.000294)  & 0.471 (0.014)  &  0.315 (0.004) & 0.003621 (0.001148)\\
    & DT2~\cite{kim2021spiking}    & 0.406 (0.005)  & 0.353 (0.006)  & 0.003206 (0.000736)  & 0.406 (0.014)  &  0.320 (0.006) & 0.005094 (0.000667) \\

    & DET only   &0.516 (0.007)  &0.374 (0.038)   & 0.003172 (0.001966)  & 0.377 (0.007)  & 0.241 (0.038)  & 0.003248 (0.000765) \\
    & DTT only & 0.450 (0.001)  &  0.327 (0.010) & 0.002744 (0.001008)  & 0.413 (0.062)  & 0.289 (0.012)  &  0.002742 (0.000227)\\
    & \DTname\  &0.440\textbf{ (0.001)}  & 0.316\textbf{ (0.005)}  &  0.001247\textbf{ (0.000212)} & 0.501\textbf{ (0.000)}  & 0.300\textbf{ (0.001)}  &0.002092\textbf{ (0.000302)} \\
    \hline
    \multirow{7}{*}{\makecell[c]{GN}}
    & SAN  & 0.538 (0.014)  & 0.311 (0.014)  & 0.002522 (0.000424)  & 0.288\textbf{ (0.003)}  & 0.209 (0.097)  & 0.000883 (0.000621) \\
    & SAN-NR  & 0.530 (0.015)   & 0.318 (0.013)  &  0.003055 (0.001615) &0.503 (0.015)   & 0.299 (0.013)  & 0.005029 (0.001543)\\
    & DT1~\cite{hao2020biologically}    &0.452 (0.005)  & 0.319\textbf{ (0.005)}  &  0.001408 (0.000747) & 0.502 (0.017)  &0.302 (0.017)   &  0.004470 (0.001997)\\
    & DT2~\cite{kim2021spiking}     & 0.405\textbf{ (0.004)}  & 0.336 (0.011)  & 0.002005 (0.000465)  & 0.423\textbf{ (0.003)}  &0.283 (0.031)  &0.005235 (0.000536) \\

    & DET only   & 0.500 (0.009) & 0.367 (0.031)  & 0.001424 (0.000218)  & 0.392 (0.008)   & 0.286 (0.007)  & 0.003130 (0.000647) \\
    & DTT only & 0.445 (0.004)   &  0.311 (0.006) & 0.001260 (0.000476)  & 0.401 (0.074)  & 0.310 (0.009)  & 0.001795 (0.000720) \\
    & \DTname\  & 0.443\textbf{ (0.004)} &  0.306\textbf{ (0.005)}  & 0.001085\textbf{ (0.000050)}  & 0.498\textbf{ (0.003)}  &  0.301\textbf{ (0.000)}  &  0.001962\textbf{ (0.000432)} \\
    \hline
    \multirow{7}{*}{\makecell[c]{8-bit \\ Loihi \\ weight}}
    & SAN  & 0.519 (0.005)   &  0.319 (0.006) & 0.001106 (0.000992)  & 0.290 (0.005)  & 0.315 (0.009)  & 0.000961 (0.000543) \\
    & SAN-NR  & 0.510 (0.005)   & 0.336 (0.005)  & 0.001153 (0.000287)  & 0.478 (0.010)  &  0.317 (0.005) &  0.005220 (0.001734) \\
    & DT1~\cite{hao2020biologically}    & 0.435 (0.012) & 0.318 (0.006)  & 0.001467 (0.000688)  & 0.472 (0.013)  & 0.327 (0.008)  & 0.001854 (0.000619)\\
    & DT2~\cite{kim2021spiking}     & 0.411 (0.010)  & 0.339 (0.008)  &  0.001802 (0.000668) & 0.428 (0.008)  &  0.317\textbf{ (0.003)} &0.005032 (0.000739) \\

    & DET only   & 0.504 (0.005) & 0.341 (0.005)  & 0.000924 (0.000282)  & 0.387 (0.003)  & 0.288 (0.009)  & 0.002816 (0.000333) \\
    & DTT only & 0.446 (0.003)   & 0.327 (0.010)  & 0.001302 (0.000434)  & 0.462 (0.013)   &  0.303 (0.002)  & 0.002038 (0.000477) \\
    & \DTname\  & 0.439\textbf{ (0.000)} & 0.308\textbf{ (0.003)}  & 0.001107\textbf{ (0.000072)} &  0.502\textbf{ (0.001)}  & 0.297 (0.004) & 0.002164\textbf{ (0.000230)} \\
    \hline
    \multirow{7}{*}{\makecell[c]{GN \\ weight \\  (5 rounds)}}
    & SAN  & 0.503 (0.021)  & 0.340 (0.015)  & 0.001241 (0.000857)  &  - &  - &  -\\
    & SAN-NR  & 0.488 (0.027)   & 0.340 (0.009)  & 0.001796 (0.000356)  & 0.499 (0.011)   & 0.328 (0.016)  & 0.004204 (0.000718) \\
    & DT1~\cite{hao2020biologically}    & 0.413 (0.034)  &0.346 (0.022)   & 0.002318 (0.000163)  & 0.491 (0.006)  & 0.320\textbf{ (0.001)}   &  0.003065 (0.000592)\\
    & DT2~\cite{kim2021spiking}     & 0.390 (0.011) & 0.336 (0.011)  &  0.001382 (0.001088) & 0.411 (0.007)  & 0.292 (0.017)  &0.008895 (0.003124)  \\

    & DET only   & 0.516 (0.007)  & 0.372 (0.036)  & 0.002643 (0.001437)  & 0.397 (0.013)  & 0.218 (0.061)  & 0.003384 (0.000901) \\
    & DTT only & 0.467 (0.018)  & 0.328 (0.011)  & 0.001352 (0.000384)  & 0.393 (0.082)  &  0.303 (0.002)  & 0.003581 (0.001066) \\
    & \DTname\  & 0.444\textbf{ (0.005)} & 0.318\textbf{ (0.007)}  & 0.001163\textbf{ (0.000128)}  & 0.498\textbf{ (0.003)}  & 0.300\textbf{ (0.001)}  & 0.001923\textbf{ (0.000471)}\\
    \hline
    \multirow{7}{*}{\makecell[c]{30\% \\ Zero \\ weight\\ (5 rounds)}}
    & SAN  & 0.443 (0.081) & 0.320\textbf{ (0.005)}  & 0.000862 (0.001236)  & -  &-   & -\\
    & SAN-NR  &0.457 (0.058)    & 0.338 (0.007)   & 0.002461 (0.001021)  & 0.472 (0.016)  &  0.332 (0.020)  &  0.009380 (0.005894)\\
    & DT1~\cite{hao2020biologically}    & 0.388 (0.059) & 0.312 (0.012)  & 0.001257 (0.000898)  & 0.456 (0.029)  & 0.334\textbf{ (0.015)} & 0.005820 (0.003347) \\
    & DT2~\cite{kim2021spiking}     &0.372 (0.029)  &  0.359 (0.012) & 0.001930 (0.000540)  &  0.403 (0.017) & 0.332 (0.018)  & 0.003060 (0.002711) \\

    & DET only   &0.524 (0.015)  & 0.368 (0.032)  &  0.002974 (0.001786) & 0.360 (0.024)  & 0.245 (0.034)  & 0.004378 (0.001895) \\
    & DTT only & 0.472 (0.023)  & 0.334 (0.017)  &  0.002013 (0.000277) & 0.402 (0.073)  & 0.280 (0.021) &0.004420 (0.001905) \\
    & \DTname\  & 0.446\textbf{ (0.007)} & 0.316\textbf{ (0.005)}  &  0.001502\textbf{ (0.000467)} & 0.488\textbf{ (0.013)}  &  0.316\textbf{ (0.015)} &0.004638\textbf{ (0.002244)} \\

    \bottomrule
  \end{tabular}
\end{table}
