# Supplementary material for: Biologically Inspired Dynamic Thresholds for Spiking Neural Networks
Source: arXiv:2206.04426 source file (2023-06-19)
Supplement: Supplementary file 17 [file rebuttal1.tex]

% \textbf{The experiments are restricted to the robot and control tasks. It would be better to include more tasks such as tasks in computer vision.}


% In principle, the proposed BDETT may be applied to tasks solved with an SNN. We assess the method on three tasks under 19 different experimental setups, including normal and degraded conditions. The proposed BDETT has been tested with two different SNN models, i.e., LIF and SRM.

% Nevertheless, we conducted additional experiments on image classification. To this end, we adopted the SCNN model~\cite{wu2018spatio} and trained on the MNIST dataset. Following the experimental setup of~\cite{wu2018spatio}, each pixel of an MNIST image is encoded into 30 Poisson spikes as inputs to SCNN for both training and testing.

% Similar to our experimental setup for robotic control tasks, we also designed two different degraded conditions: degraded inputs and weight uncertainty.

% \textbf{Adversarial samples as degraded inputs}: to test the generalization on degraded inputs we use existing adversarial attack methods to generate relevant degraded inputs for the image classification tasks.

% \begin{itemize}
%     % \vspace{-0.1cm}
%     \item `FGSM $\epsilon = x$': Fast gradient sign method (FGSM)~\cite{goodfellow2014explaining} with $\epsilon = x$;
    
%     \item `PGD $iter_\epsilon=x\ iter_{num}=y$: projected gradient descent (PGD)~\cite{madry2017towards}, with iteration epsilon of $x$ and iteration number of $y$ for each attack step.
% \end{itemize}

% \textbf{Weight uncertainty}: we also evaluate the robustness to internal weight uncertainty as follows.


% \begin{itemize}
%     % \vspace{-0.1cm}
%     \item `GN$(0, x)$': adding Gaussian noise (GN) with zero mean and standard deviation of $x$ to all synaptic weights;
    
%     \item `$x\%$ zero weight': for the synaptic weights between every two adjacent layers, we randomly set $x\%$ of them to 0;
    
% \end{itemize}

% Directly applying the proposed approach without any changes to image classification in degraded conditions compares favorably across all experimental settings and in terms of generalization. With stronger degradations, the top 1 classification accuracy of both baseline and our approach decreases, but the proposed method is less affected, validating BDETT for this vision task.

% \begin{table}[hb]
% \caption{ }
%   \label{SMtab}
%   \centering
%   \renewcommand\arraystretch{2}
% %   \setlength\tabcolsep{5pt}
% \begin{tabular}{llll}
% \hline
% \textbf{Experimental setup}                                                              & \textbf{Threshold Type} & \textbf{LIF-based SCNN} & \textbf{SRM-based SCNN} \\
% \hline
% \multirow{2}{*}{Original}                                                                & Static Threshold        & 99.42\%                 & 99.13\%                 \\
%                                                                                          & BDETT                   & \textbf{99.45\%}        & \textbf{99.15\%}        \\
% \multirow{2}{*}{\makecell[c]{FGSM \\ $\epsilon$ = 0.20}}
%   & Static Threshold        & 66.33\%                 & 56.85\%                 \\
%                                                                                          & BDETT                   & \textbf{69.14\%}        & \textbf{57.01\%}        \\
% \multirow{2}{*}{\makecell[c]{PGD \\ $iter_\epsilon$ = 0.01 \\ $iter_{num}$=20}}
% & Static Threshold        & 84.31\%                 & 67.53\%                 \\
%                                                                                          & BDETT                   & \textbf{85.74\%}        & \textbf{68.06\%}        \\
% \multirow{2}{*}{GN(0, 0.3)}                                                              & Static Threshold        & 81.98\%                 & 78.24\%                 \\
%                                                                                          & BDETT                   & \textbf{85.09\%}        & \textbf{78.68\%}        \\
% \multirow{2}{*}{GN(0, 0.5)}                                                              & Static Threshold        & 39.84\%                 & 45.32\%                 \\
%                                                                                          & BDETT                   & \textbf{47.74\%}        & \textbf{46.34\%}        \\
% \multirow{2}{*}{20\% zero weight}                                                        & Static Threshold        & 90.52\%                 & 95.10\%                 \\
%                                                                                          & BDETT                   & \textbf{96.37\%}        & \textbf{96.59\%}        \\
% \multirow{2}{*}{30\% zero weight}                                                        & Static Threshold        & 84.37\%                 & 89.75\%                 \\
%                                                                                          & BDETT                   & \textbf{90.68\%}        & \textbf{91.02\%}      \\
       
%       \hline
% \end{tabular}
% \end{table}



% \textbf{Since the authors claim in the methods section that the two dynamic threshold mechanisms can help each other achieve optimal settings. Thus, more sufficient evidence needs to be provided to support this viewpoint.}

In the section ``Interaction of DET and DTT" of our main paper, we illustrate the interaction between DET and DTT with two examples. Here, we provide additional experimental evidence of the interaction of DET and DTT. Without loss of generality, we conduct the experiments by using spiking actor network (SAN) as the host SNN for a robot obstacle avoidance task.

% \subsection*{Interaction between DET and DTT}
Interaction DET/DTT with low potential fluctuations.

\begin{itemize}
    \item \textbf{Experimental setup}: We randomly chose a timestamp and recorded all postsynaptic membrane potentials and spiking thresholds of the host SNN. Then, for each layer, we randomly selected $X$ neurons based on the binomial distribution with a probability of $0.5$. The chosen neurons were added random positive noise, generated based on a normal distribution $\mathcal N(0.2,0.05)$. The mean of 0.2 is around 20\% of the average of the recorded membrane potentials. To reduce the impact of the randomness, we did 5-round tests and reported the average and standard deviation of the obtained DETs and DTTs. The average number of selected neurons of these 5-round tests of each layer, $\mu(X)$, is also reported. 
    
    \item \textbf{Experimental thesis}: We expect DET increases as the noise increases the membrane potential. DTT should remain at a relatively constant threshold (\emph{i.e.}, $a + 1$) as the preceding rate of depolarization caused by the noise is close to 0.
    
    \item \textbf{Experimental result}: The layerwise mean, $\mu$, and standard deviation, $\sigma$, of the 5-round DETs and DTTs with and without added noise are reported in Table~\ref{tab:low}, aligning well with the experimental thesis. $\Delta$ is the absolute value of the difference between original and add noise.

    
\end{itemize}

\begin{table}[hb]
\caption{Interaction DET/DTT with low potential fluctuations. }
  \label{tab:low}
  \centering
  \renewcommand\arraystretch{2}
%   \setlength\tabcolsep{5pt}
\begin{tabular}{lllll}
\hline
                             & \textbf{$\mu(X)$}       & \textbf{original ($\mu$ / $\sigma$)} & \textbf{add noise ($\mu$ / $\sigma$)} & \makecell[c]{\textbf{$\Delta$}} \\
\hline
layer 1 DET & \multirow{2}{*}{130.4}        & 1.4950 / 0.0051        & 1.5143 / 0.0066     & \makecell[c]{0.0193 / 0.0015}     \\
layer 1 DTT &                               & 0.0570 / 0.0064        & 0.0571 / 0.0063    & \makecell[c]{0.0001 / 0.0001}    \\
\hline
layer 2 DET & \multirow{2}{*}{128.4}        & 2.1548 / 0.0120        & 2.1745 / 0.0111    & \makecell[c]{0.0197 / 0.0009}    \\
layer 2 DTT &                               & 0.2725 / 0.0154        & 0.2724 / 0.0152    & \makecell[c]{0.0001 / 0.0002 }   \\
\hline
layer 3 DET & \multirow{2}{*}{126.6}        & 3.3528 / 0.0788        & 3.3720 / 0.0777   & \makecell[c]{0.0192 / 0.0011}     \\
layer 3 DTT &                               & 0.4549 / 0.0033        & 0.4549 / 0.0033   & \makecell[c]{0.0000 / 0.0000 }    \\
\hline
\end{tabular}
\end{table}


% \begin{table}[hb]
% \caption{Interaction DET/DTT with low potential fluctuations. }
%   \label{tab:low}
%   \centering
%   \renewcommand\arraystretch{2}
% %   \setlength\tabcolsep{5pt}
% \begin{tabular}{lllll}
% \hline
%                              & \textbf{$\mu(X)$}       & \textbf{original ($\mu$ / $\sigma$)} & \textbf{add noise ($\mu$ / $\sigma$)} & \makecell[c]{\textbf{$\Delta$}} \\
% \hline
% layer 1 DET & \multirow{2}{*}{130.4}        & 1.4950 / 0.0051        & 1.5143 / 0.0066     & \makecell[c]{-0.0193/-0.0015}     \\
% layer 1 DTT &                               & 0.0570 / 0.0064        & 0.0571 / 0.0063    & \makecell[c]{-0.0001/0.0001}    \\
% \hline
% layer 2 DET & \multirow{2}{*}{128.4}        & 2.1548 / 0.0120        & 2.1745 / 0.0111    & \makecell[c]{-0.0197/0.0009}    \\
% layer 2 DTT &                               & 0.2725 / 0.0154        & 0.2724 / 0.0152    & \makecell[c]{0.0001/0.0002 }   \\
% \hline
% layer 3 DET & \multirow{2}{*}{126.6}        & 3.3528 / 0.0788        & 3.3720 / 0.0777   & \makecell[c]{-0.0192/0.0011}     \\
% layer 3 DTT &                               & 0.4549 / 0.0033        & 0.4549 / 0.0033   & \makecell[c]{0.0000/0.0000 }    \\
% \hline
% \end{tabular}
% \end{table}

Interaction DET/DTT with fast membrane potential drop.


\begin{itemize}
    \item \textbf{Experimental setup}: We adopted the same binomial distribution as in the first experiment and randomly selected $X$ neurons of the host SNN. To mimic fast membrane potential drops from $t$ to $t+1$, we added random negative membrane potentials with a larger magnitude than the first experiment, which was generated by sampling a normal distribution $\mathcal N(-2.0, 0.5)$.
    
    \item \textbf{Experimental thesis}: In this scenario, even though DET decreases with the reduced membrane potential, we expect DTT to increase faster, and BDETT to increase the overall threshold.
    
    \item \textbf{Experimental result}: The layerwise mean and STD of the 5-round $X$ DETs, DTTs, and BDETTs with and without fast membrane potential drop are shown in Table~\ref{tab:fast}. Again, the findings align with the experimental thesis.

    
\end{itemize}


\begin{table}[ht]
\caption{Interaction DET/DTT with fast membrane potential drop }
  \label{tab:fast}
  \centering
  \renewcommand\arraystretch{2}
%   \setlength\tabcolsep{5pt}
\begin{tabular}{lllll}
\hline
                             & \textbf{$\mu(X)$}       & \textbf{original ($\mu$ / $\sigma$)} & \textbf{fast potential drop ($\mu$ / $\sigma$)} & \makecell[c]{\textbf{$\Delta$}}\\
\hline
layer 1 DET & \multirow{3}{*}{128.2}        & 1.4919 / 0.0089        & \makecell[c]{1.4032 / 0.0106 }   & \makecell[c]{0.0887 / 0.0017} \\
layer 1 DTT &                               & 0.0579 / 0.0044        & \makecell[c]{1.0115 / 0.0251 }   &  \makecell[c]{0.9536 / 0.0207}  \\
layer 1 BDETT &                               & 0.7749 / 0.0039        & \makecell[c]{1.2074 / 0.0124}  & \makecell[c]{0.4325 / 0.0085} \\
\hline
layer 2 DET & \multirow{3}{*}{124.8}        & 2.1865 / 0.0292        & \makecell[c]{2.0348 / 0.0514 }    &  \makecell[c]{0.1517 / 0.0222} \\
layer 2 DTT &                               & 0.2863 / 0.0053        & \makecell[c]{1.1938 / 0.0332}     &  \makecell[c]{0.9075 / 0.0279} \\
layer 2 BDETT &                               & 1.2364 / 0.0148        & \makecell[c]{1.6143 / 0.0293}    & \makecell[c]{0.3779 / 0.0145}   \\
\hline
layer 3 DET & \multirow{3}{*}{130.4}        & 3.6456 / 0.1114        & \makecell[c]{3.3802 / 0.1298}    &  \makecell[c]{0.2654 / 0.0184}  \\
layer 3 DTT &                               & 0.4479 / 0.0141        & \makecell[c]{1.3337 / 0.0307}   &  \makecell[c]{0.8858 / 0.0166}   \\
layer 3 BDETT &                               & 2.0468 / 0.0610        & \makecell[c]{2.3570 / 0.0574}    &  \makecell[c]{0.3102 / 0.0036}  \\
\hline
\end{tabular}
\end{table}




% \begin{table}[ht]
% \caption{Interaction DET/DTT with fast membrane potential drop }
%   \label{tab:fast}
%   \centering
%   \renewcommand\arraystretch{2}
% %   \setlength\tabcolsep{5pt}
% \begin{tabular}{lllll}
% \hline
%                              & \textbf{$\mu(X)$}       & \textbf{original ($\mu$ / $\sigma$)} & \textbf{fast potential drop ($\mu$ / $\sigma$)} & \makecell[c]{\textbf{$\Delta$}}\\
% \hline
% layer 1 DET & \multirow{3}{*}{128.2}        & 1.4919 / 0.0089        & \makecell[c]{1.4032 / 0.0106 }   & \makecell[c]{0.0887/-0.0017} \\
% layer 1 DTT &                               & 0.0579 / 0.0044        & \makecell[c]{1.0115 / 0.0251 }   &  \makecell[c]{-0.9536/-0.0207}  \\
% layer 1 BDETT &                               & 0.7749 / 0.0039        & \makecell[c]{1.2074 / 0.0124}  & \makecell[c]{-0.4325/-0.0085} \\
% \hline
% layer 2 DET & \multirow{3}{*}{124.8}        & 2.1865 / 0.0292        & \makecell[c]{2.0348 / 0.0514 }    &  \makecell[c]{0.1517/-0.0222} \\
% layer 2 DTT &                               & 0.2863 / 0.0053        & \makecell[c]{1.1938 / 0.0332}     &  \makecell[c]{-0.9075/-0.0279} \\
% layer 2 BDETT &                               & 1.2364 / 0.0148        & \makecell[c]{1.6143 / 0.0293}    & \makecell[c]{-0.3779 / -0.0145}   \\
% \hline
% layer 3 DET & \multirow{3}{*}{130.4}        & 3.6456 / 0.1114        & \makecell[c]{3.3802 / 0.1298}    &  \makecell[c]{0.2654 / -0.0184}  \\
% layer 3 DTT &                               & 0.4479 / 0.0141        & \makecell[c]{1.3337 / 0.0307}   &  \makecell[c]{-0.8858 / -0.0166}   \\
% layer 3 BDETT &                               & 2.0468 / 0.0610        & \makecell[c]{2.3570 / 0.0574}    &  \makecell[c]{-0.3102 /0.0036}  \\
% \hline
% \end{tabular}
% \end{table}
