# Supplementary material for: Biologically Inspired Dynamic Thresholds for Spiking Neural Networks
Source: arXiv:2206.04426 source file (2023-06-19)
Supplement: Supplementary file 18 [file rebuttal2.tex]

The computational complexity of the proposed BDETT is bounded by the computational complexity of calculating the mean, maximum, and minimum, i.e., Eqs. 3, 4, and 6. Therefore, the upper bound of estimating BDETT complexity, $\Theta_i^l(t+1)$, is $O(n)$, where $n$ is the number of neurons on the $l$-th layer. The baseline methods, DT1 and DT2, are bounded by the summation operations and offer the same upper bound, $O(n)$; see Eqs. 8 and 9 in Supplementary Note 2.

We report the layer-wise running time with PyTorch 1.2 on an i7-7700 CPU and NVIDIA GTX 1080Ti GPU. As we can see the running time of the proposed BDETT for the testing network is 1.36 ms.
\begin{table}[ht]
\caption{Layer-wise running time.}
  \label{tab:run_time}
  \centering
  \renewcommand\arraystretch{2}
%   \setlength\tabcolsep{5pt}
\begin{tabular}{llllll}
\hline
         & \textbf{\makecell[c]{Layer 1 \\ (256 neurons)}} & \textbf{\makecell[c]{Layer 2 \\ (256 neurons)}} & \textbf{\makecell[c]{Layer 3 \\ (256 neurons)}} & \textbf{\makecell[c]{Layer 4 \\ (2 neurons)}} & \textbf{Total} \\
\hline
DET (ms) & 0.18        & 0.19        & 0.19      & 0.18        & 0.74      \\
DTT (ms) & 0.11        & 0.11        & 0.11      & 0.10        & 0.43      \\
BDETT (ms) &  0.34     & 0.35        & 0.35      & 0.32        & 1.36      \\
\hline
\end{tabular}
\end{table}

% \textbf{Memory complexity}

% To evaluate BDETT, $\Theta_i^l(t+1)$, we need to evaluate $V_m^l(t)$, $V_{\theta}^l(t)$, and $\mu(\Theta_i^l(t))$. Therefore, the upper bound of the memory complexity is $O(n)$, where $n$ is the number of neurons on the $l$-th layer. The lower bound is $O(1)$.

% DT1 and DT2 offer the same memory complexity.
